# Supplementary material for: Numerical investigations of the fluid-structure interaction of a NACA0012 airfoil based on large-eddy simulations
Source: arXiv:1807.01574 source file (2018-07-04)
Supplement: Supplementary file 1 [file appendix_phy_fund.tex]

\par When a relative velocity is present in a system composed of fluid and body, aerodynamic forces, i$.$e$.$, pressure (normal to the body) and skin friction (tangential to the body) forces, are generated. These are affected by the geometry of the body and the characteristics of the flow, for instance, if the boundary layer is detached or if separation bubbles are formed. Moreover, the fluid properties such as density, viscosity, speed and compressibility also influence the magnitude of these forces.
\par In aeroelasticity, i$.$e$.$, study of the influence of the aerodynamic forces on elastic bodies, two components of the force and one component of the moment that act on a body have a major effect: the lift and drag forces and the pitching moment. The former is perpendicular to the direction of motion, while the drag force is in the direction of the motion. The latter is the moment about an axis perpendicular to both the direction of motion and the lift vector.
\par Due to the effect of aeroelastic instabilities, a structure can suffer excessive deformations and fail. This is mainly caused by an increase in the relative flow speed, which leads to a raise in the aerodynamic forces, while the material and geometry dependent structural stiffness remains constant. The major problem of the dynamic aerolastic instability is flutter, which is characterized by self-sustained oscillations that either maintain or grow the oscillation amplitude.

\section{Aerodynamic properties}
\label{sec:aerodynamic_properties}
\par The aerodynamic performance of different structures is frequently compared by the aerodynamic coefficients, which are non-dimensional numbers that are proportional to the pressure, shear stress and the forces generated by these stresses.
\par Four coefficients are mainly utilized: the pressure coefficient $C_p$, the skin friction coefficient $C_f$, the drag coefficient $C_D$ and the lift coefficient $C_L$ (see \mbox{Eqs.\ (\ref{eq:pressure_coefficient}) through (\ref{eq:lift_coefficient})}). The former is a result of the fluid static pressure variation caused by the interaction between flow and body contour. The skin friction coefficient is a consequence of the fluid viscosity and the body surface roughness, which are responsible for the creation of a wall shear stress. The drag and lift coefficients are influenced by respectively the drag and lift forces.
%\begin{eqnarray}
%\label{eq:pressure_coefficient}
%C_D&=&\frac{2\,(p-p_\infty)}{\rho_f\,u_{in,\,1}^2}	\\
%\label{eq:skin_friction_coefficient}
%C_f&=&\frac{2\,\tau_w}{\rho_f\,u_{in,\,1}^2}	\\
%\label{drag_coefficient}
%C_D&=&\frac{2\,F_D}{\rho_f\,S\,u_{in,\,1}^2}	\\
%\label{eq:lift_coefficient}
%C_L&=&\frac{2\,F_L}{\rho_f\,S\,u_{in,\,1}^2}
%\end{eqnarray}
%\par $p$, $p_\infty$ and $u_{in,\,1}$ are the static pressure at the point at which the pressure coefficient is evaluated and the free stream static pressure and velocity, respectively. $\rho_f$, $\tau_w$, $F_D$, $F_L$ and $S$ are respectively the fluid density, the wall shear stress, the drag and lift forces and the reference are. The latter is a function of the chord length $c$ and the span-wise length $L_3$, according to Eq.\ (\ref{eq:reference_area}):
%\begin{equation}
%S=c\,L_3 \label{eq:reference_area}
%\end{equation}

\section{Aeroelastic properties}
\par The influence of the aerodynamic forces on bodies is studied according to the frequency and amplitude of the oscillations. The dimensionless Strouhal number $St$, which characterizes the flow, is utilized in order to enable a comparison between the numerical and experimental results. This is calculated conform Eq.\ (\ref{eq:strouhal_number}):
\begin{equation}
St=\frac{fc}{u_{in,\,1}}.
\label{eq:strouhal_number}
\end{equation} 
\par $c$ and $f$ represent the characteristic length, i$.$e$.$, the chord length, and the vortex shedding frequency. The latter can be estimated by the utilization of a Fourier transform in the time dependent translational and rotational displacements. This transform represent the frequency domain of the original signal, i$.$e$.$, it decomposes a function of time into frequencies.  
\par When a system has pitch and plunge degrees of freedom and the vortex shedding frequency $f$ achieves the critical flutter frequency, the amplitude of vibration increases exponentially and the flutter phenomenon occurs. This critical frequency lies between the two natural frequencies at zero airspeed, i$.$e$.$, the natural frequency of the body in each degree of freedom, that is, in the pitch and plunge degrees of freedom (see Fung \cite{Fung_2002}).
\par Besides the flutter phenomenon, the fluid-structure interaction between body and flow is also characterized by other aeroelastic instabilities, such as limit-cycle oscillations (LCO). These are caused by the presence of complex structural and/or aerodynamic nonlinearities, which can limit the amplitude of oscillation even when the free stream velocity is higher than the critical speed calculated by linear aeroleastic theories, such as the theory presented in the work of Theodorsen et al.\ \cite{Theodorsen_1935}. The structural nonlinearity is due to material and geometrical nonlinearities, caused respectively by plastic deformations and distortions, for example. The aerodynamic one results from compressibility and viscous effects and are greatly influenced by the Reynolds number (see \mbox{Ramesh et al.\ \cite{Ramesh_2015})}.
\par Since the simulated NACA0012 is rigid and submitted to an incompressible flow, only the nonlinear aerodynamic effects due to the viscosity are relevant, such as the separation of the laminar boundary layer, either in the form of  trailing edge separation or in the form of a laminar separation bubble. These can influence the fluid-structure interaction and lead to self-sustained oscillations in the form of limit-cycle oscillations even for speeds higher than the critical one, as occurred in the experiments performed by Poirel et al.\ \cite{Poirel_2008} of an elastically mounted NACA0012 airfoil with pitch and plunge degrees of freedom at a range of Reynolds number of $4.5{\cdot}10^4\leq Re \leq 1.3{\cdot}10^5$.

\subsection{Added mass effect}
\label{subsec:added_mass_effect}
\par Added mass is the additional inertia added to a system composed of a fluid and a body, which is submitted to a relative velocity. The deflection of the fluid due to the presence of the body generates additional fluid forces, which act on the surfaces in contact with the flow. This added mass acts as an extra mass on the structural degrees of freedom at the coupling interface and has destabilizing effects on loose coupled algorithms due to their explicit nature. Moreover, the effect of this mass varies also with the time discretization methods utilized by the structural and fluid subproblems (see \mbox{Förster et al.\ \cite{Foerster_2007})}.
\par The relation between the mass of the body and the mass of the displaced fluid (see \mbox{Eq.\ \ref{eq:mass_ratio})} indicates if the added mass effect must be considered.  The higher this relation, the smaller the effect of the added mass and therefore sequentially staggered schemes (loose coupling) are numerically stable and can be utilized (see Causin et al.\ \cite{Causin_2005}).
\begin{equation}
\label{eq:mass_ratio}
m^*=\frac{m^{body}}{m^{fluid}_{disp}}
\end{equation}
\par Song et al.\ \cite{Song_2013} investigated the influence of the added mass effect on stiff plate structures of different materials utilizing a partitioned approach based on a loose coupling algorithm. The case with $m^*=10$ exhibited no convergence problems, while under-relaxation factors were used in the case with $m^*=1$ in order to guarantee the convergence of the solution. Therefore, the influence of the added mass effect for $m^*=10$ was negligible, while this effect was responsible for numerical difficulties for the $m^*=1$ case.  
\par In the present work, the mass ratio between airfoil and displaced fluid is $m^*=720$. Therefore, a loose coupling method ($n_{FSI}=1$) is utilized due to its numerical stability and lower required computational time (compared to strong coupling approaches).
