# Supplementary material for: Numerical investigations of the fluid-structure interaction of a NACA0012 airfoil based on large-eddy simulations
Source: arXiv:1807.01574 source file (2018-07-04)
Supplement: Supplementary file 4 [file appendix_3.tex]

\par The algorithm utilized for the estimation of displacements, as well as the added mass effect and the coupling method are thoroughly analyzed. Since the utilization of the estimation of displacements together with a loosely coupled algorithm requires the smallest computational time, the studies primarily aim at the analysis of the accuracy of this method through a comparison with other algorithms. Thereby, the best compromise between accuracy and numerical effort can be determined and further utilized for the FSI simulations.

\section{Investigation of the estimation of displacements}\markboth{APPENDIX E.$\quad$PREL. STUD. FSI COUP.}{E.1$\quad$INV. OF THE EST. OF DISP.}
\label{subsec:investigation_estimation_displacement}

\par The linear extrapolation of the displacements is implemented in order to improve the convergence properties and therefore to reduce the required computational time. Two strong coupled simulations of the fluid-structure interaction between NACA0012 airfoil and flow are executed for the $m{-}L_3^{min}{-}y_{max}^+$ mesh utilizing the mapping strategy 4. The FSI is computed for two degrees of freedom (pitch and plunge) with linear and  torsional stiffnesses of $k_{l,\,2}=144\,\text{N}{\cdot}\text{m}^{-1}$ and $k_{t,\,3}=0.3832\,\text{N}{\cdot}\text{m}{\cdot}\text{rad}^{-1}$, respectively. Moreover, the chord Reynolds number is $Re=30{,}000$, the FSI convergence criterion is $\epsilon_{FSI,\,disp}<1{\cdot}10^{-6}$ and the computation runs until a dimensionless time of $t^*=4.47$ is achieved. Further properties of these simulations are summarized in Table \ref{table:comp_est_disp}:
\begin{table}[H]
	\centering
	\begin{tabular}{p{3cm} p{2.7cm} p{2.5cm} p{3cm} p{2cm}}
		\hline
		\multicolumn{1}{c}{\multirow{3}{*}{\centering{\bf{Mesh}}}} & \centering{\bf{Estimation of displacement}} & \centering{\bf{Maximal iteration number}} & \centering{\bf{Maximal number of sub-iterations}} & \centering{\bf{Time step size (s)}}\tabularnewline \hline
		\centering{$m{-}L_3^{min}{-}y^{+}_{max}$} & \centering{Yes} & \centering{$10{,}000$} & \centering{20} & \centering{$1\cdot10^{-5}$} \tabularnewline
		\centering{$m{-}L_3^{min}{-}y^+_{max}$} & \centering{No} & \centering{$14{,}286$} &\centering{20} & \centering{$7\cdot10^{-6}$} \tabularnewline			
		\hline	
	\end{tabular}
	\caption{\label{table:comp_est_disp}Simulation properties of the test cases aimed at the study of the advantages achieved by the  utilization of the prediction of the displacements.}
\end{table}
\par The simulation without prediction of the displacements requires a smaller time step, otherwise the computation of the FSI case diverges since the utilization of 20 sub-iterations is not enough to obtain a converged result for each time step.  Therefore, in order to achieve the same dimensionless time step, this simulation requires also the calculation of a greater number of iterations, increasing the necessary numerical effort.
\begin{figure}[H]
	\centering
	\subfigure[Simulation with estimation of displacement.]{\includegraphics[width=0.495\textwidth]{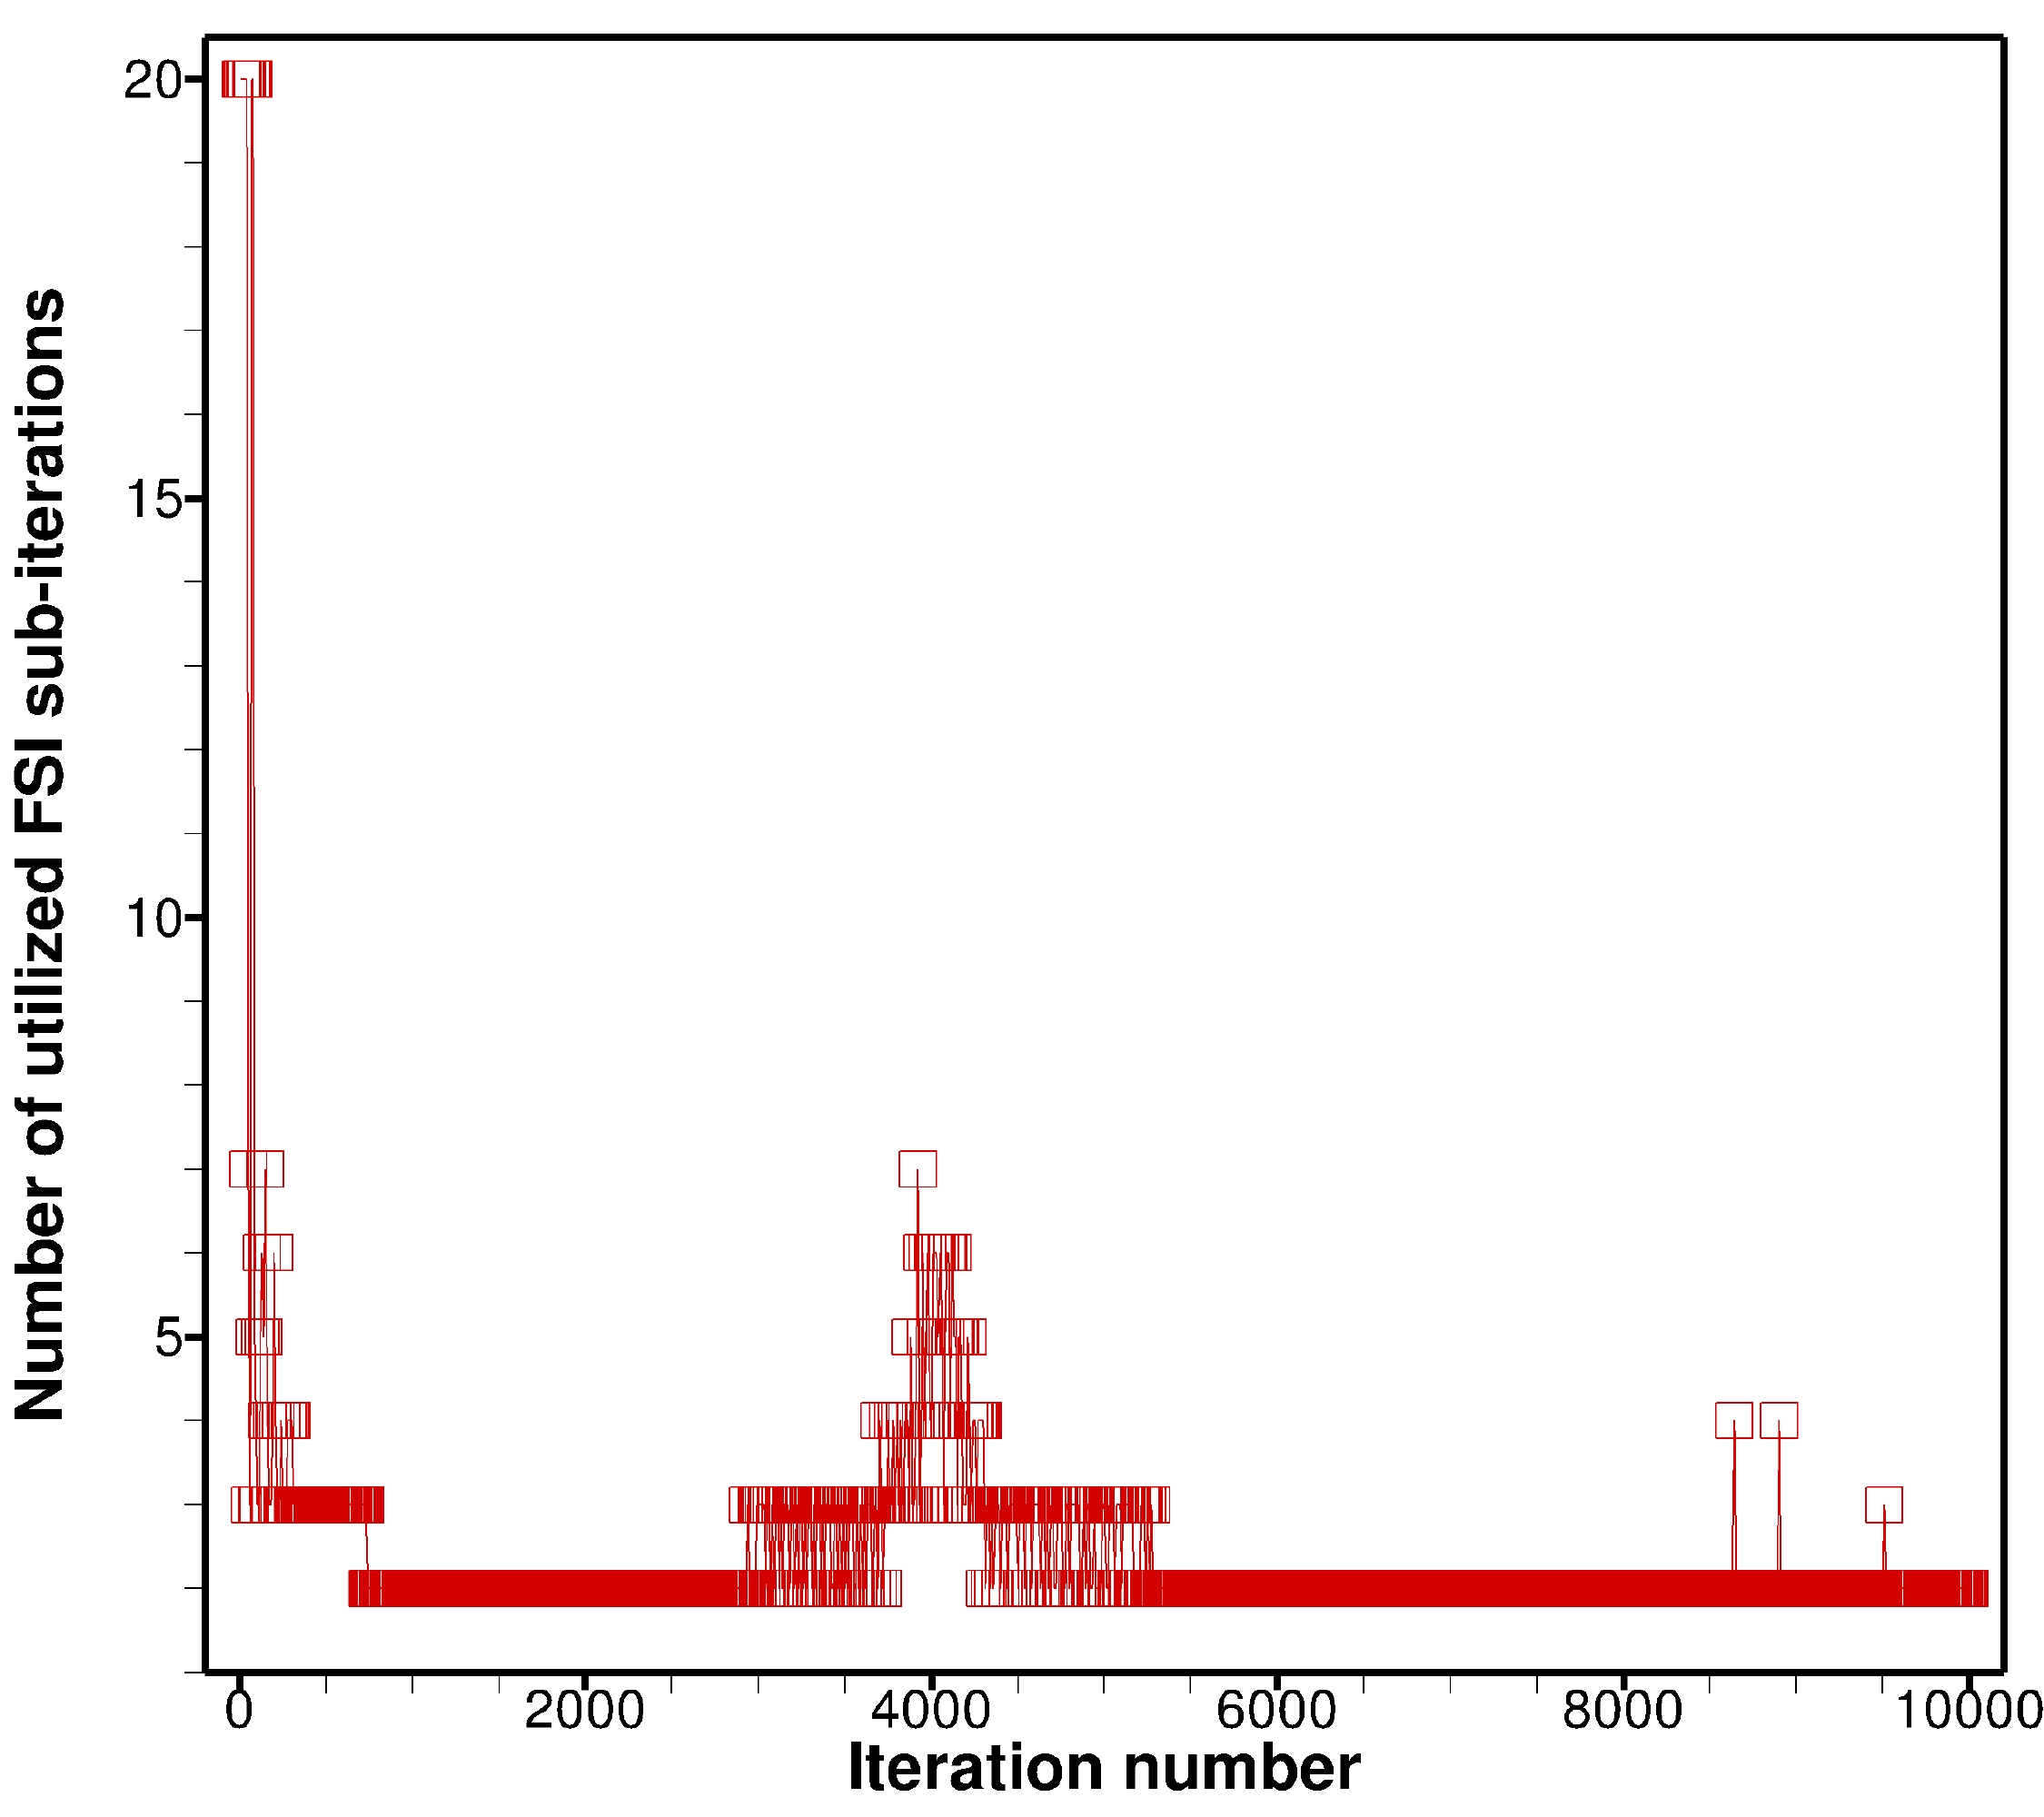} \label{fig:used_iterout_est_disp}}\hfill
	\subfigure[Simulation without estimation of displacement.]{\includegraphics[width=0.495\textwidth]{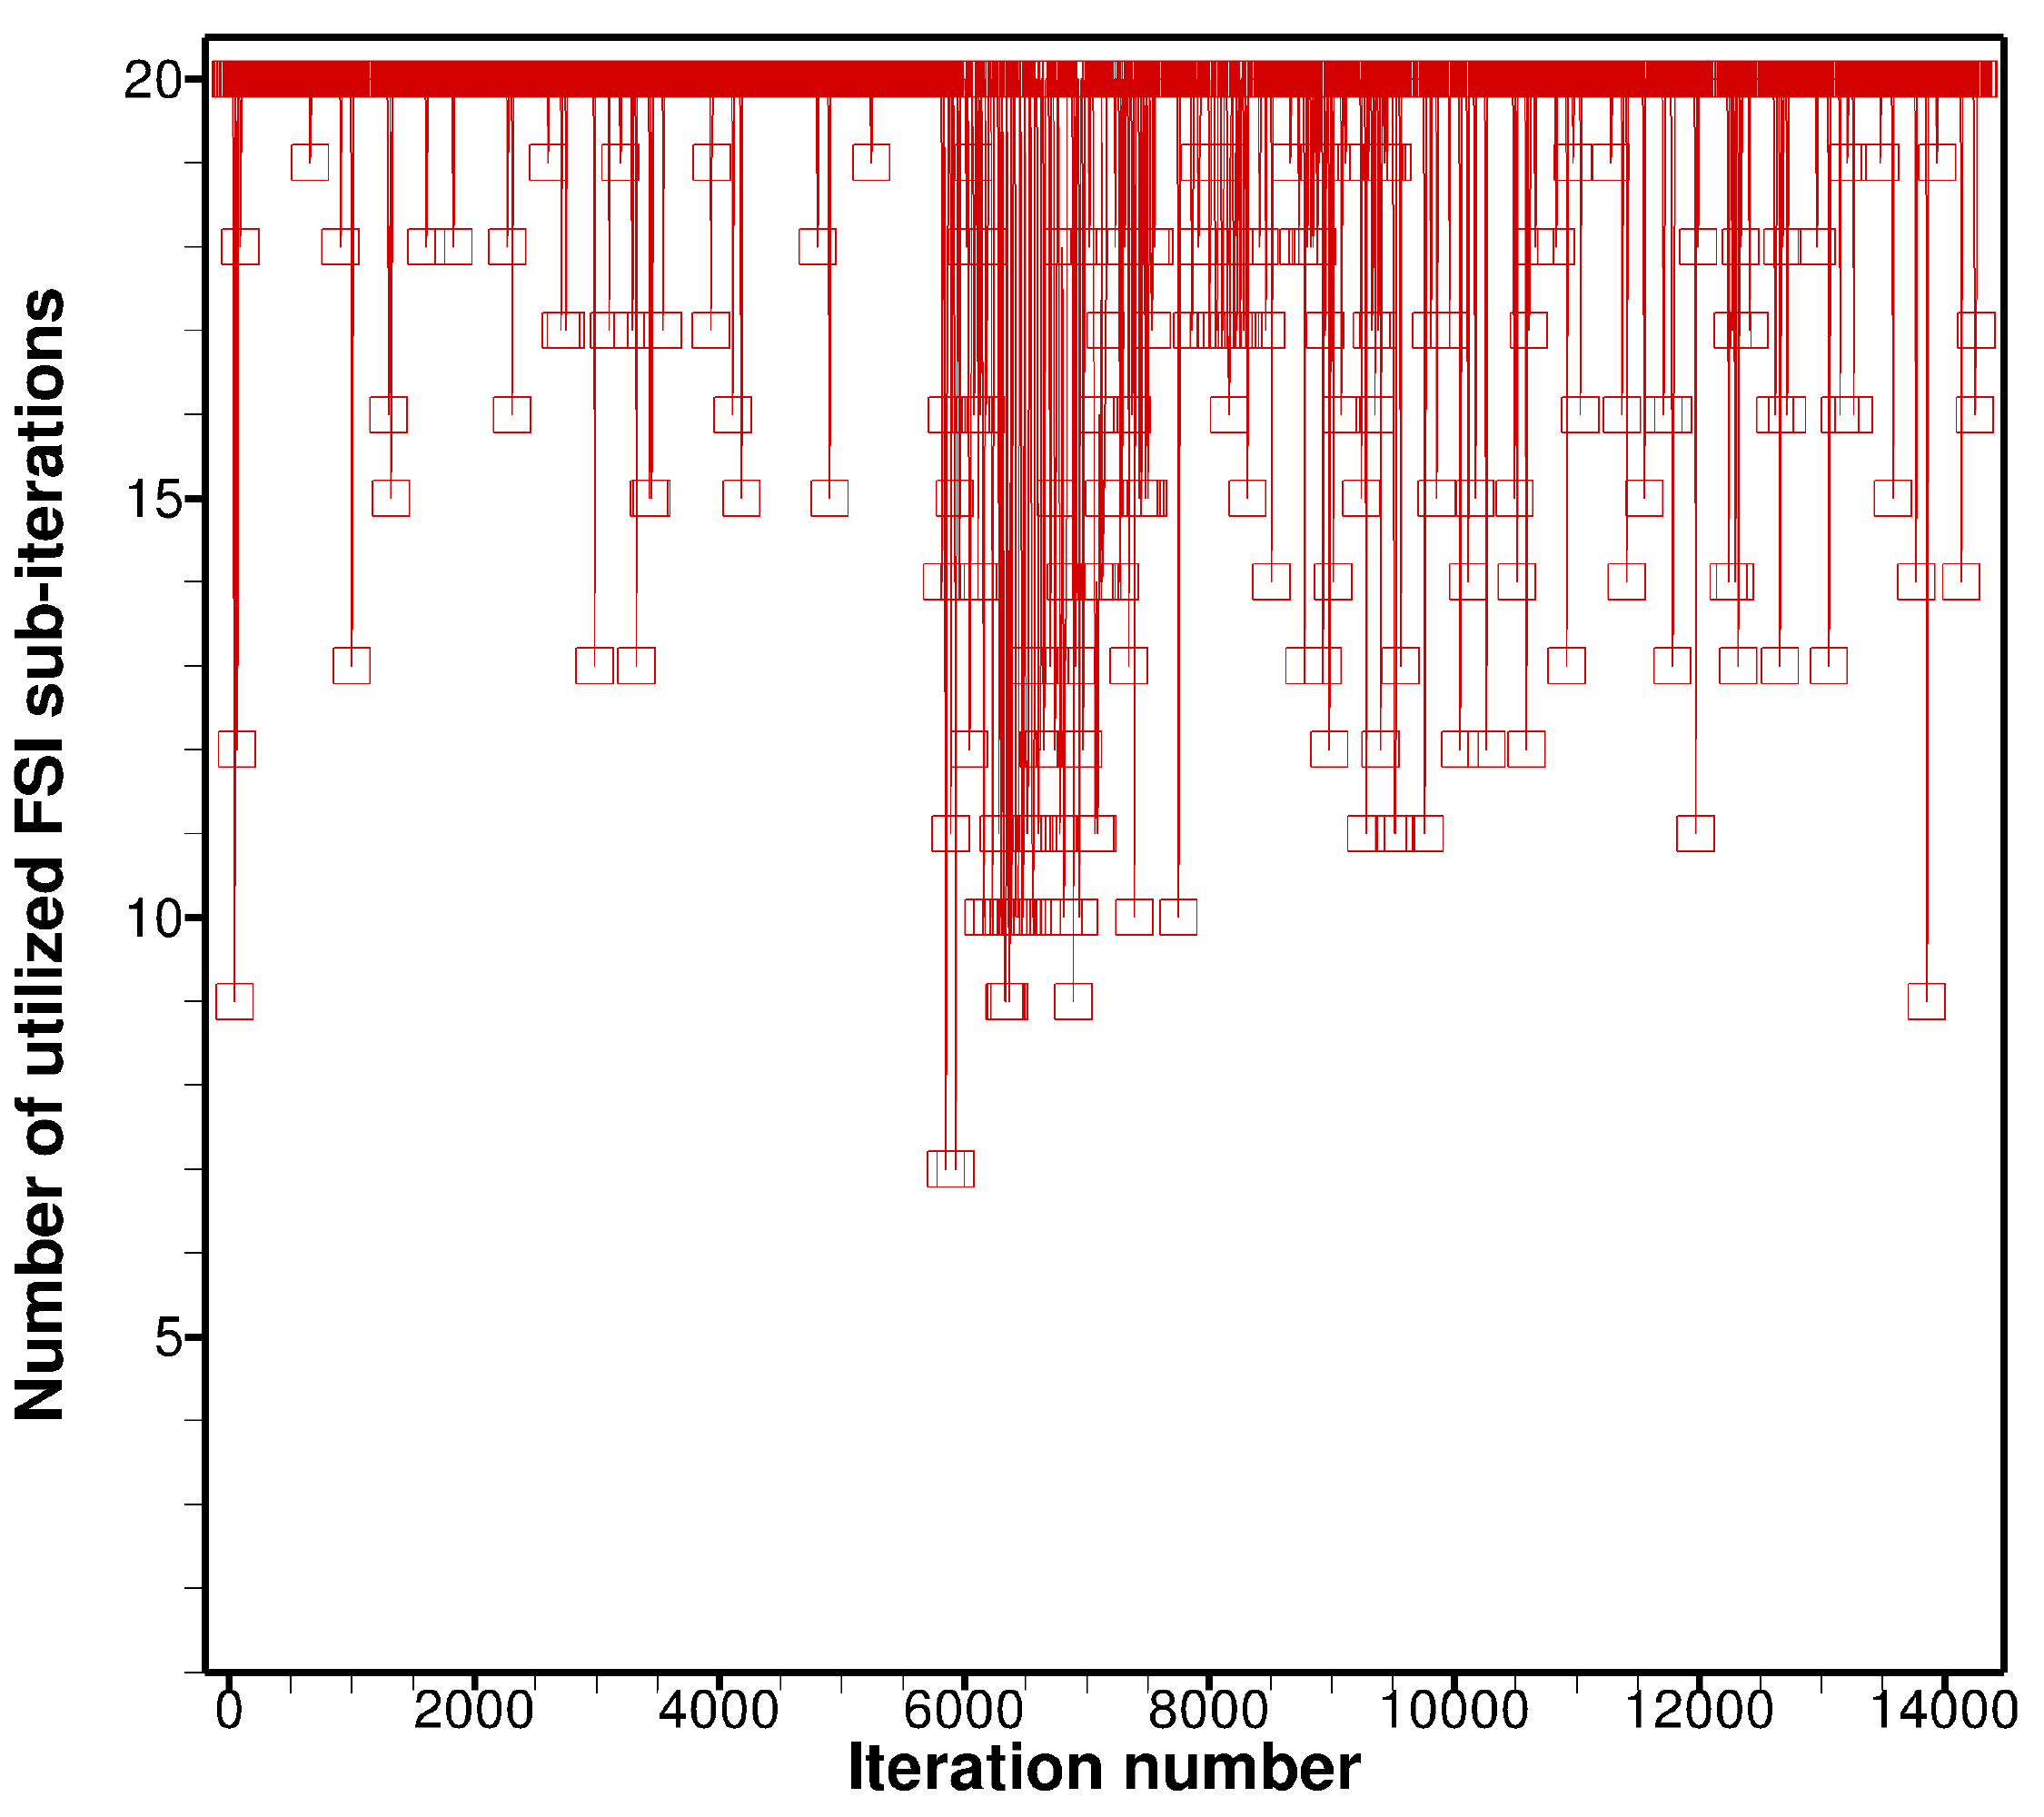}\label{fig:used_iterout_no_est_disp}}\hfill
	\caption{FSI sub-iterations for the test cases with and without the prediction of the displacements.}
	\label{fig:used_iterout_comparison}
\end{figure}
\begin{figure}[H]
	\centering
	\subfigure[Simulation with estimation of displacement.]{\includegraphics[width=0.495\textwidth]{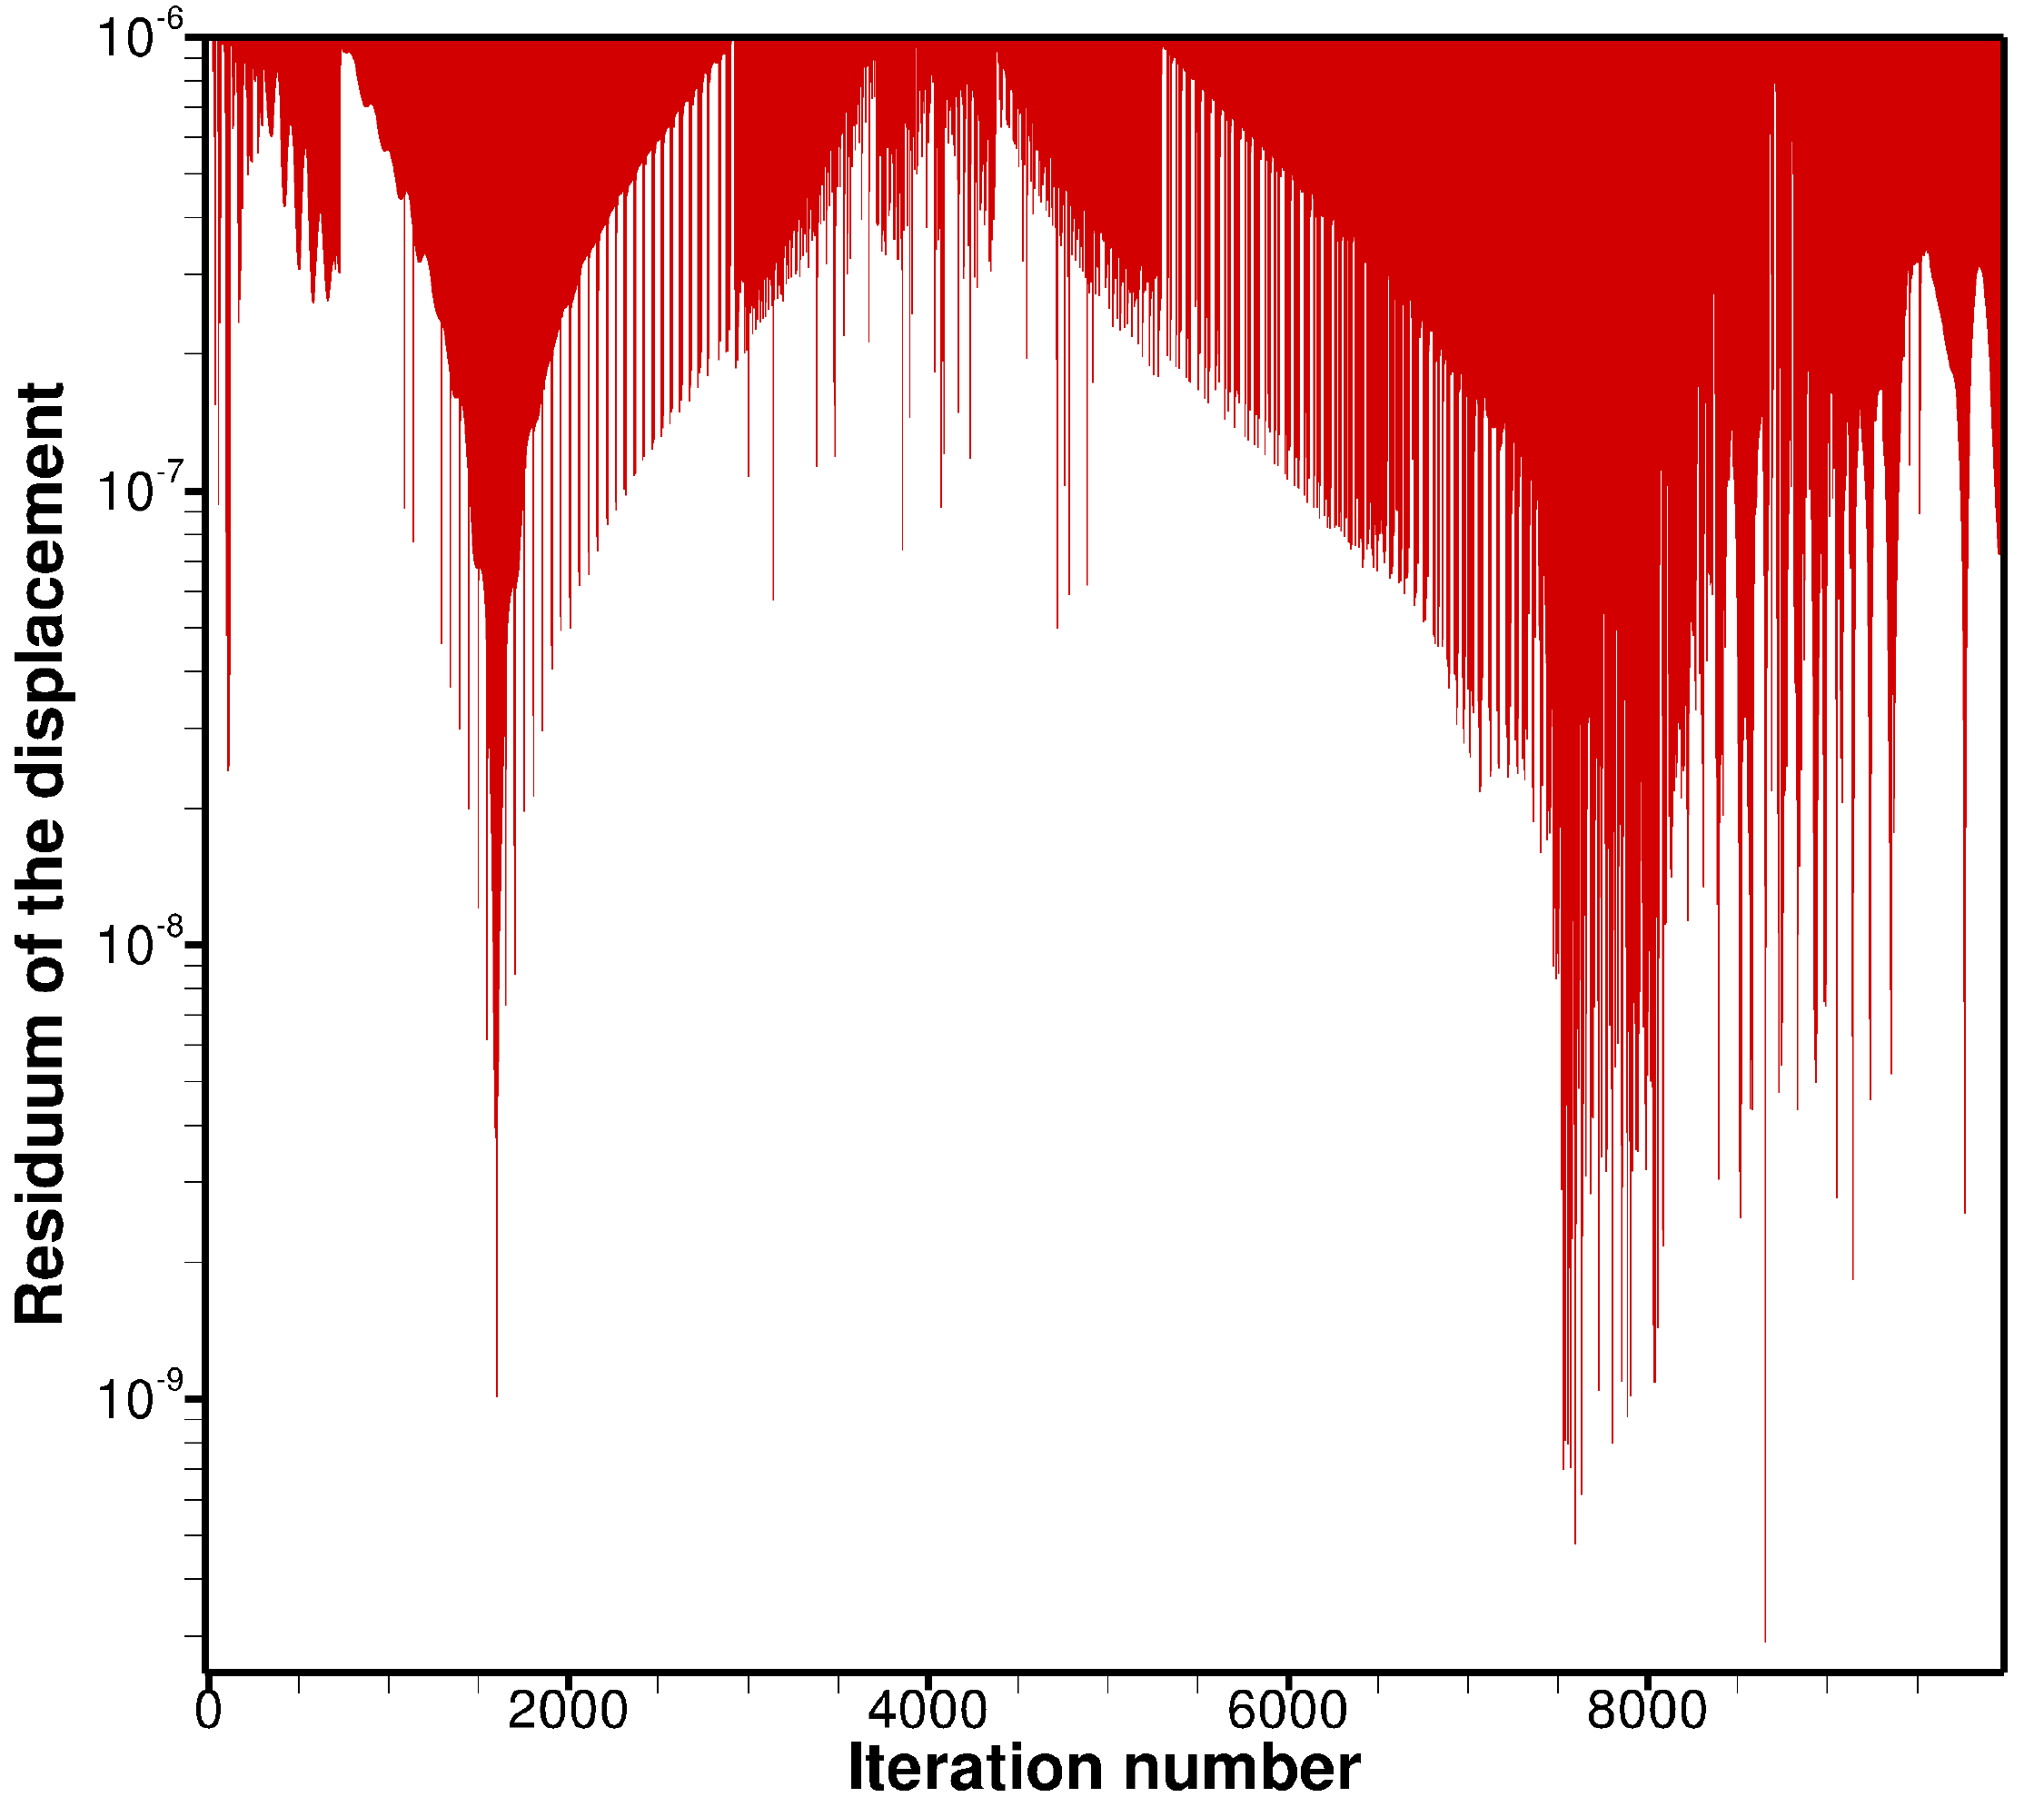} \label{fig:residuum_convergence_est_disp}}\hfill
	\subfigure[Simulation without estimation of displacement.]{\includegraphics[width=0.495\textwidth]{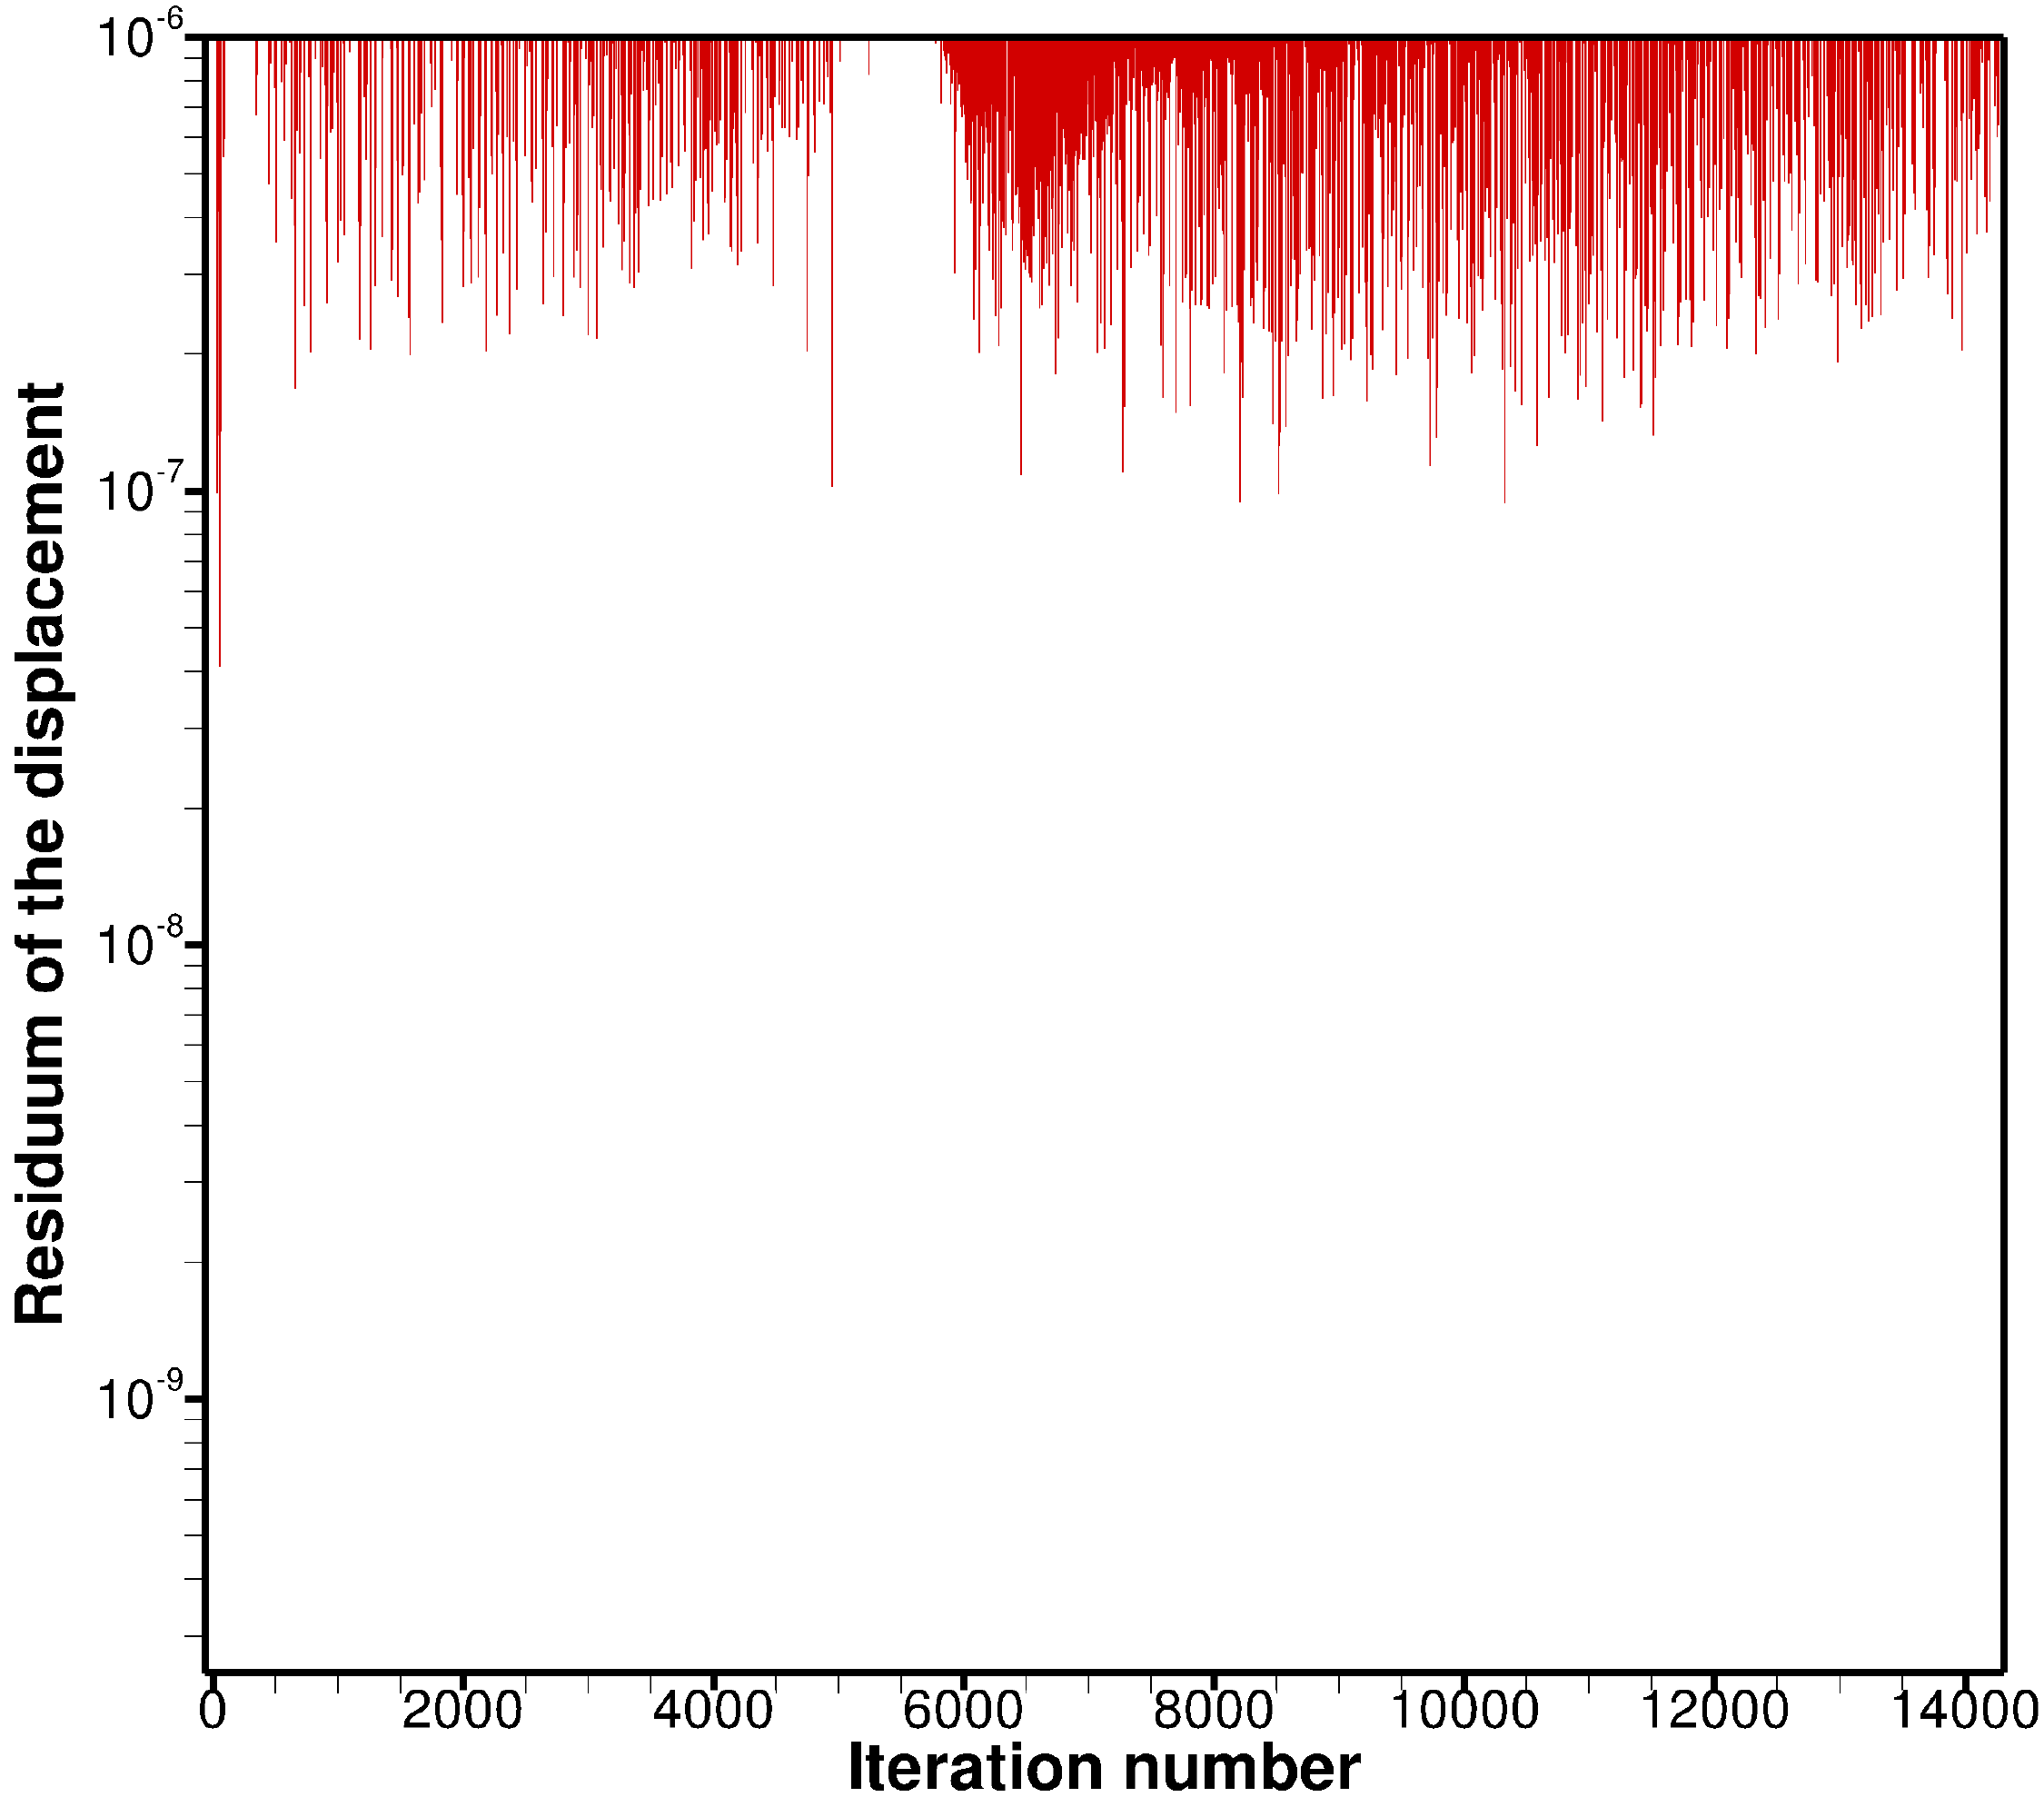}\label{fig:residuum_convergence_no_est_disp}}\hfill
	\caption{Achievement of the FSI convergence criterion $\epsilon_{FSI,\,disp}<1{\cdot}10^{-6}$ for the test cases with and without estimation of the displacements.}
	\label{fig:residuum_convergence_comparison}
\end{figure}
\par After the initialization phase, the simulation that utilizes the estimation of displacements generally requires the calculation of only two sub-iterations in order to converge, while the simulation that does not predict the displacements computes frequently all twenty sub-iterations without always achieving the convergence criterion, as illustrated in Figs.\ \ref{fig:used_iterout_comparison} and \ref{fig:residuum_convergence_comparison}. Although the convergence criterion is $\epsilon_{FSI,\,disp}<1{\cdot}10^{-6}$, many time steps of the simulations with the prediction of the displacements achieve residua in the order of magnitude of $\epsilon_{FSI,\,disp}\leq\mathcal{O}(10^{-7})$. This occurs, since the previous sub-iteration $n_{FSI}$ has not yet achieved the convergence criterion, while the current sub-iteration $n_{FSI}+1$ achieves it and also reduces the residuum of displacement up to three orders of magnitude. 
\par Furthermore, since the Fig.\ \ref{fig:residuum_convergence_comparison} does not show in detail the residuum of displacement at each sub-iteration, this is meticulously illustrated in Fig.\ \ref{fig:residuum_comparison} for the last five time steps of each simulation. These once again indicate that although all twenty sub-iterations are computed, the FSI convergence criterion is not achieved for the simulations without the estimation of displacements, resulting in a lost of accuracy.
\begin{figure}[H]
	\centering
	\subfigure[Simulation with estimation of displacement (\mbox{$9{,}996\leq n\leq10{,}000$}).]{\includegraphics[width=0.48\textwidth]{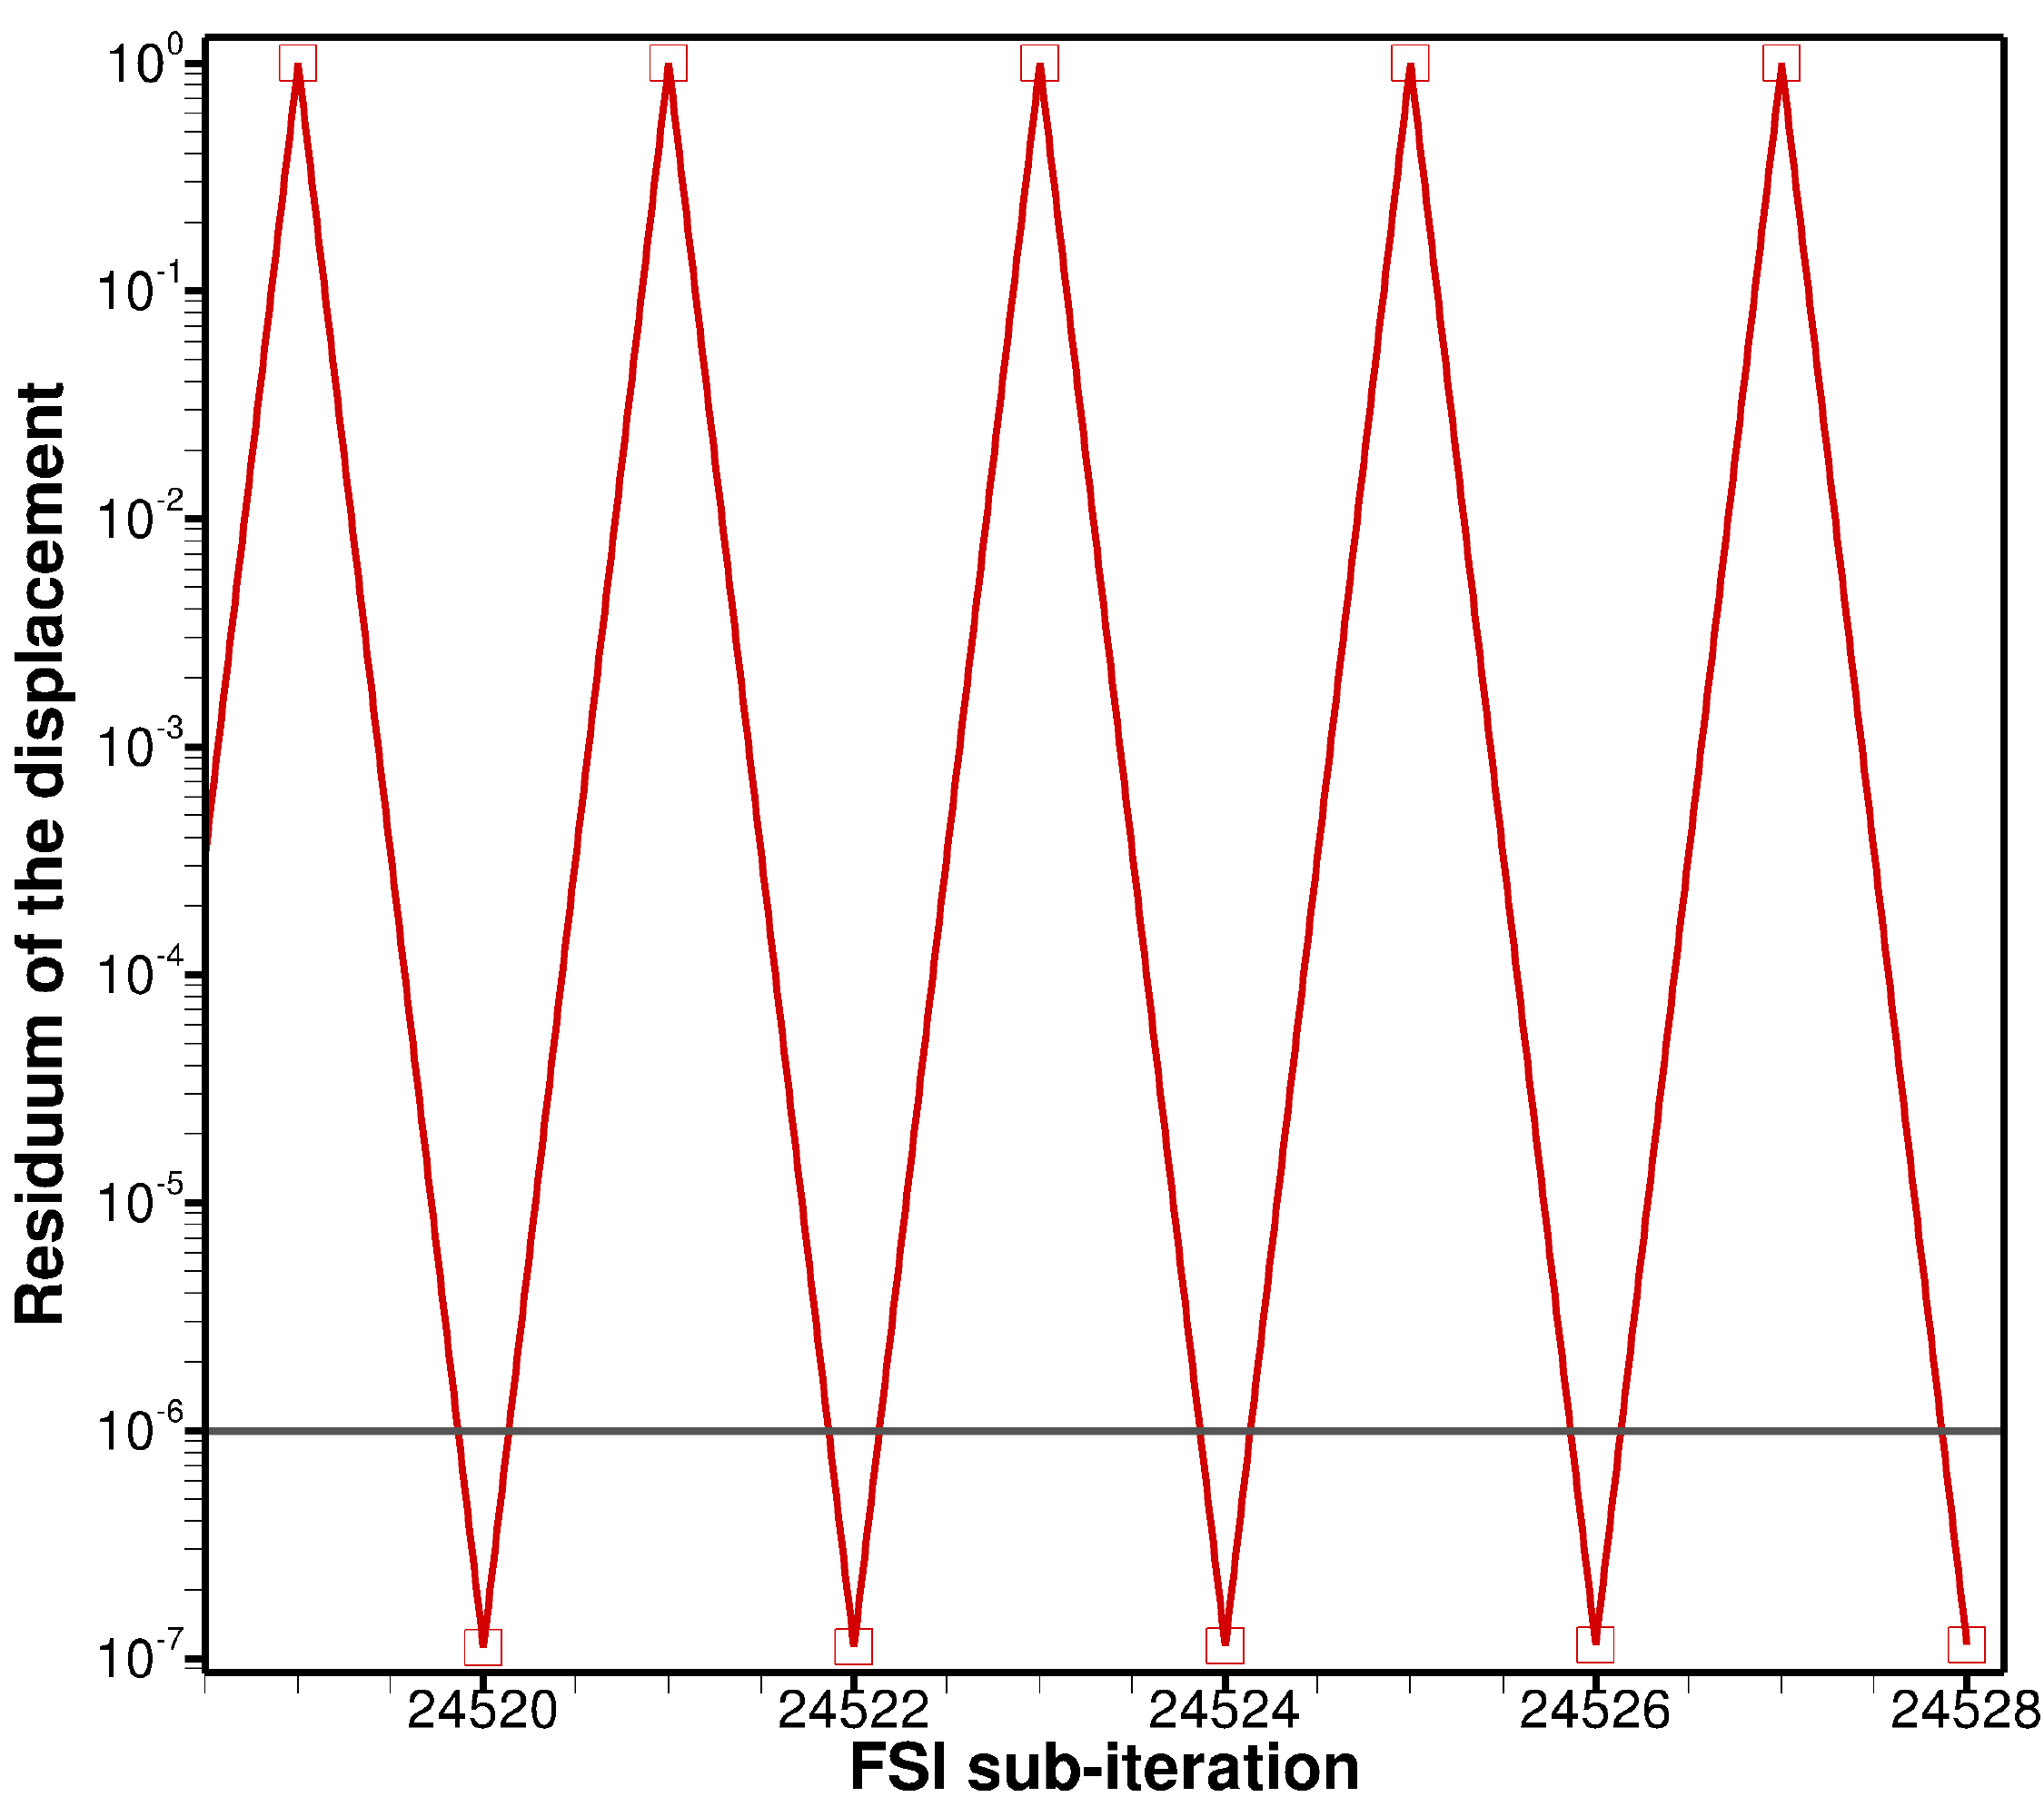} \label{fig:residuum_est_disp}}\hfill
	\subfigure[Simulation without estimation of displacement (\mbox{$14{,}282\leq n\leq14{,}286$}).]{\includegraphics[width=0.48\textwidth]{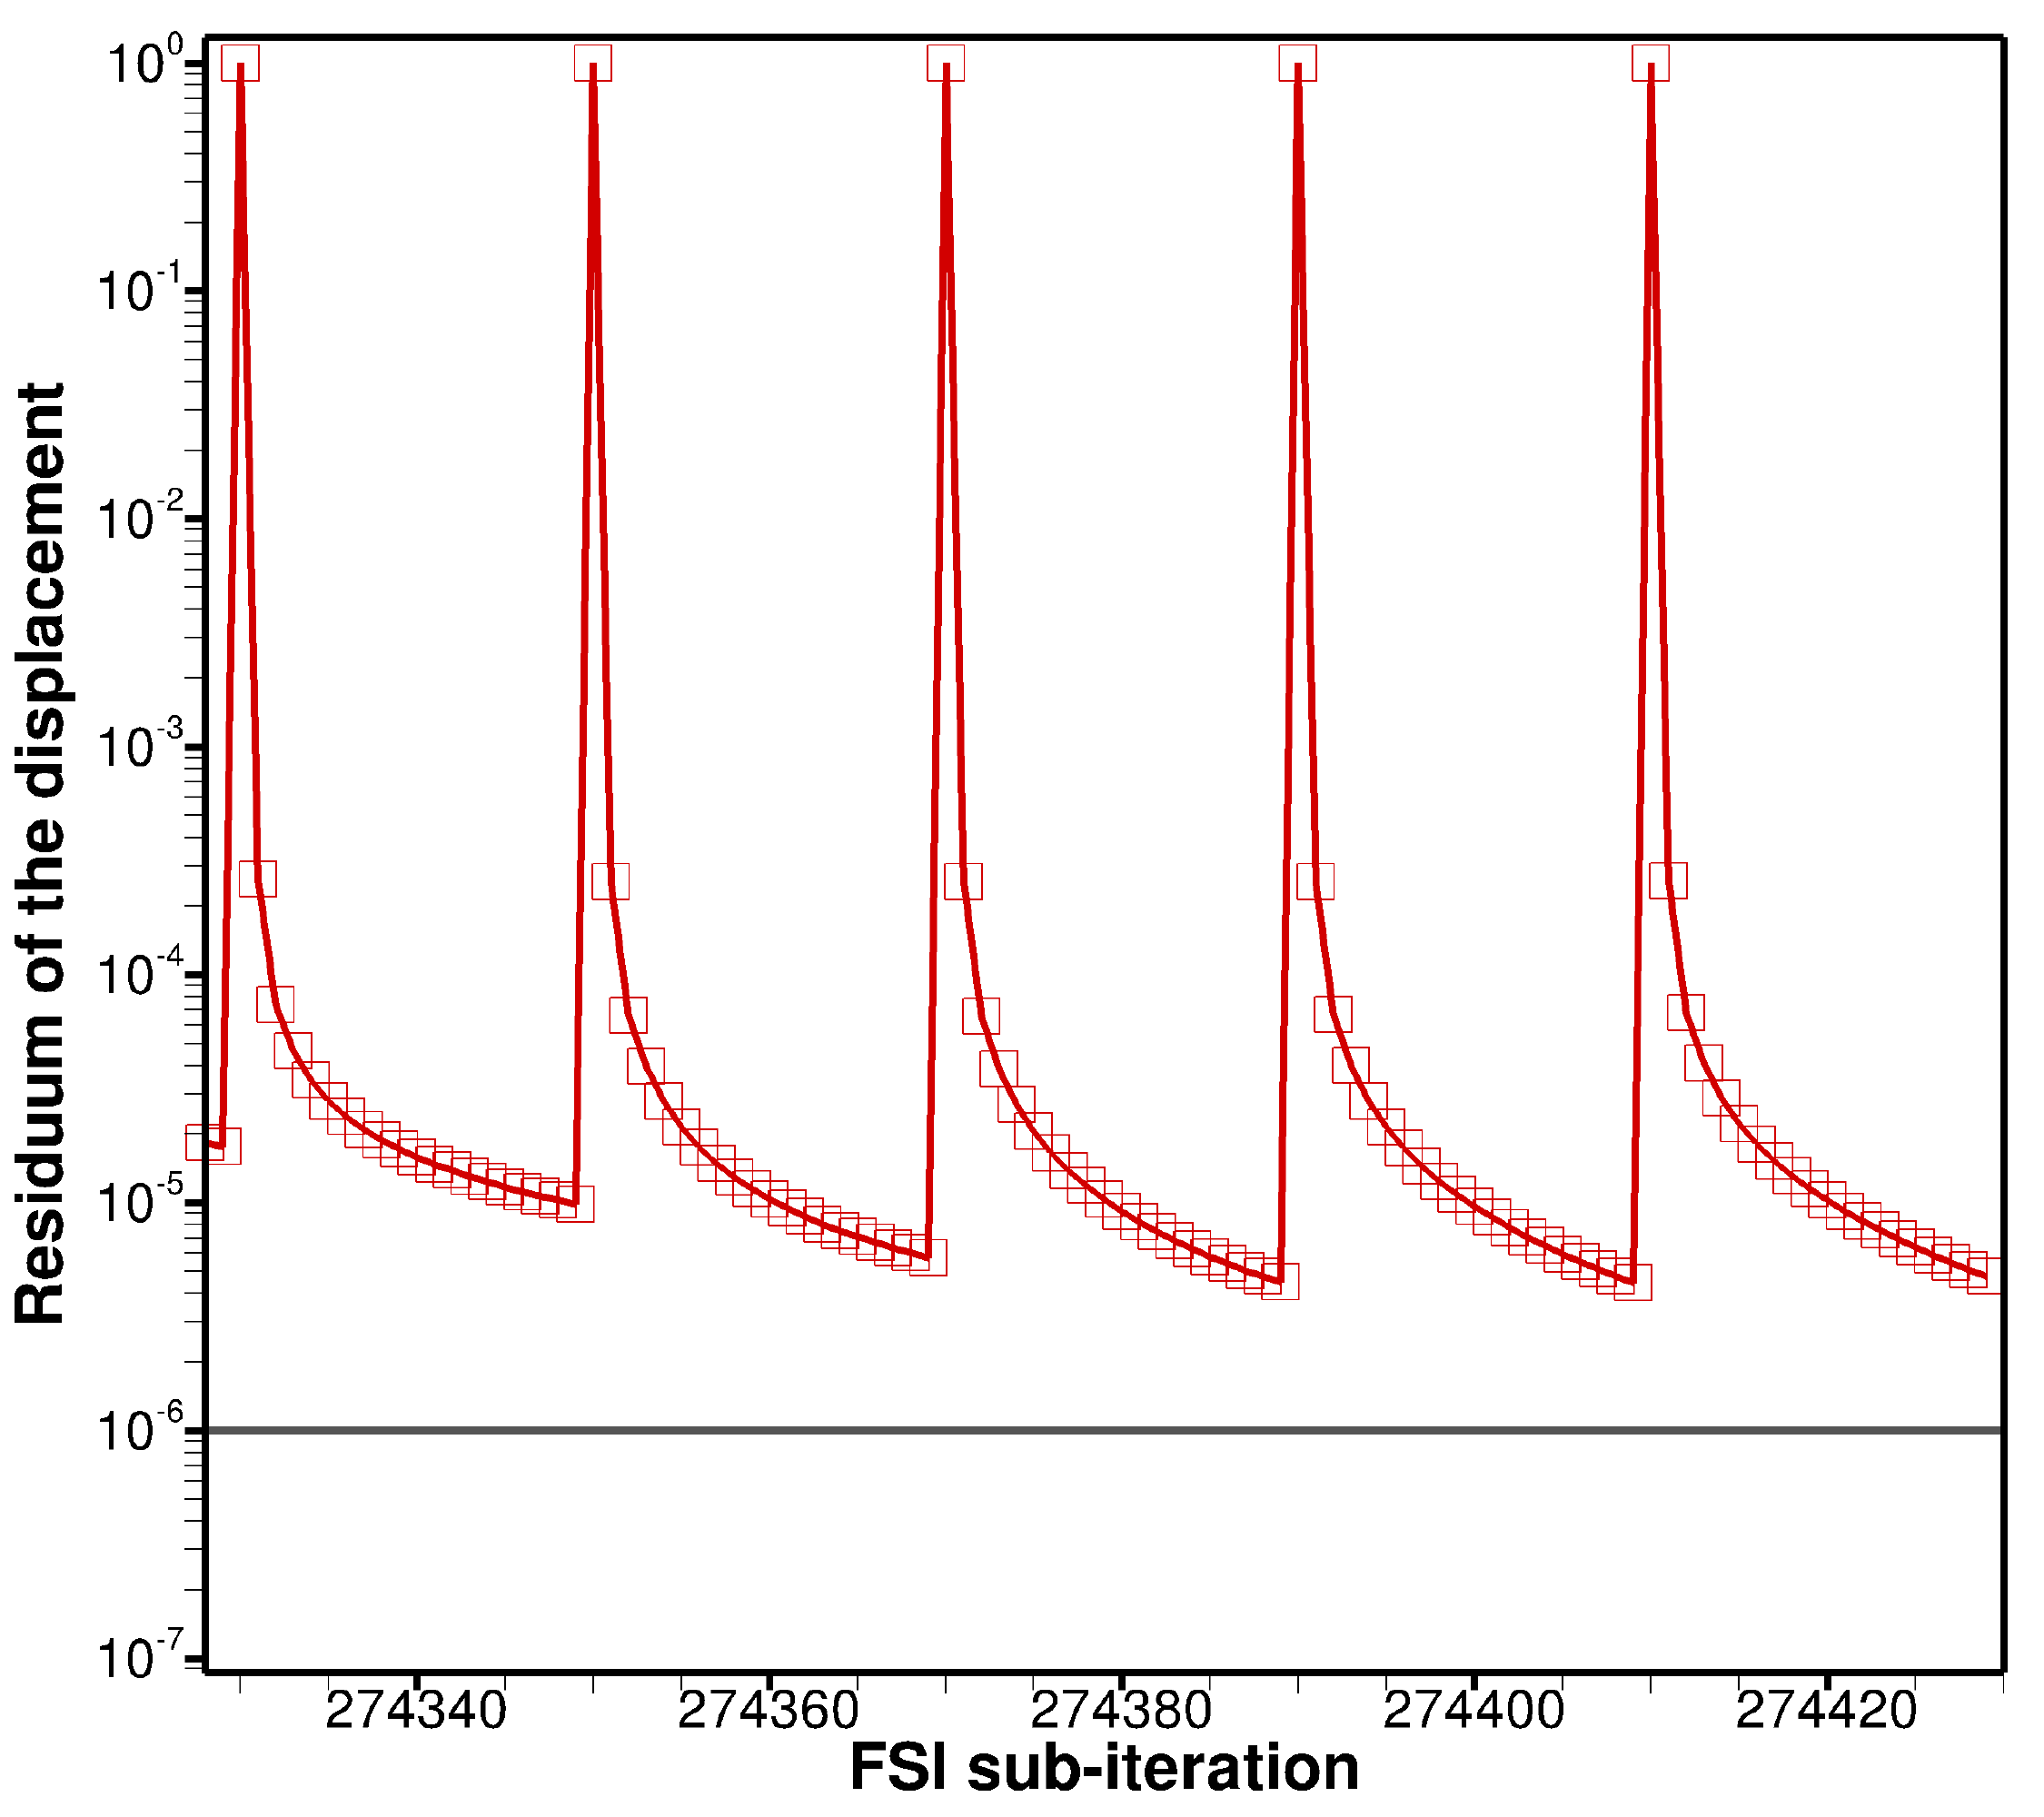}\label{fig:residuum_no_est_disp}}\hfill
	\caption{Residuum of displacement and force in the $x_3$-direction at the last five time steps of the simulations with and without estimation of displacement.}
	\label{fig:residuum_comparison}
\end{figure}
\par The accuracy of both methods can be analyzed according to the lift forces $F_3$, which should not be produced since the symmetric NACA0012 airfoil is at an incidence of $\alpha=0^\circ$. Table \ref{table:comp_forces_est_disp} illustrates the time-averaged lift force for the cases with and without estimation of displacement. 
\begin{table}[H]
	\centering
	\begin{tabular}{p{3cm} p{3cm} p{5cm}}
		\hline
		\multirow{2}{3cm}{\centering{\bf{Estimation of displacement}}} &  \multicolumn{2}{c}{\bf{Time-averaged lift force ($\text{kg}{\cdot}\text{m}{\cdot}\text{s}^{-1})$}} \tabularnewline \cline{2-3}
		 & \centering{\bf{Mean}} & \centering{\bf{Standard deviation}} \tabularnewline\hline
		 \centering{Yes} & \centering{$3.343{\cdot}10^{-7}$}&\centering{$4.341{\cdot}10^{-7}$} \tabularnewline
		 \centering{No} & \centering{$1.306{\cdot}10^{-7}$}&\centering{$6.226{\cdot}10^{-6}$} \tabularnewline
		\hline	
	\end{tabular}
	\caption{\label{table:comp_forces_est_disp}Time-averaged lift forces of the cases with and without the prediction of the displacements.}
\end{table}
\par Although the mean value of the time-averaged lift forces is slightly higher for the case utilizing the estimation of displacement, the standard deviation is one order of magnitude lower. Then, the calculations that utilize this prediction present a smaller dispersion of the data, as shown in Fig.\ \ref{fig:lift_comparison}. Therefore, the forces at each time step tend to be closer to the mean value. Hence, the algorithm that predicts the displacements leads to a greater accuracy.
\begin{figure}[H]
	\centering
	\subfigure[Simulation with estimation of displacement.]{\includegraphics[width=0.495\textwidth]{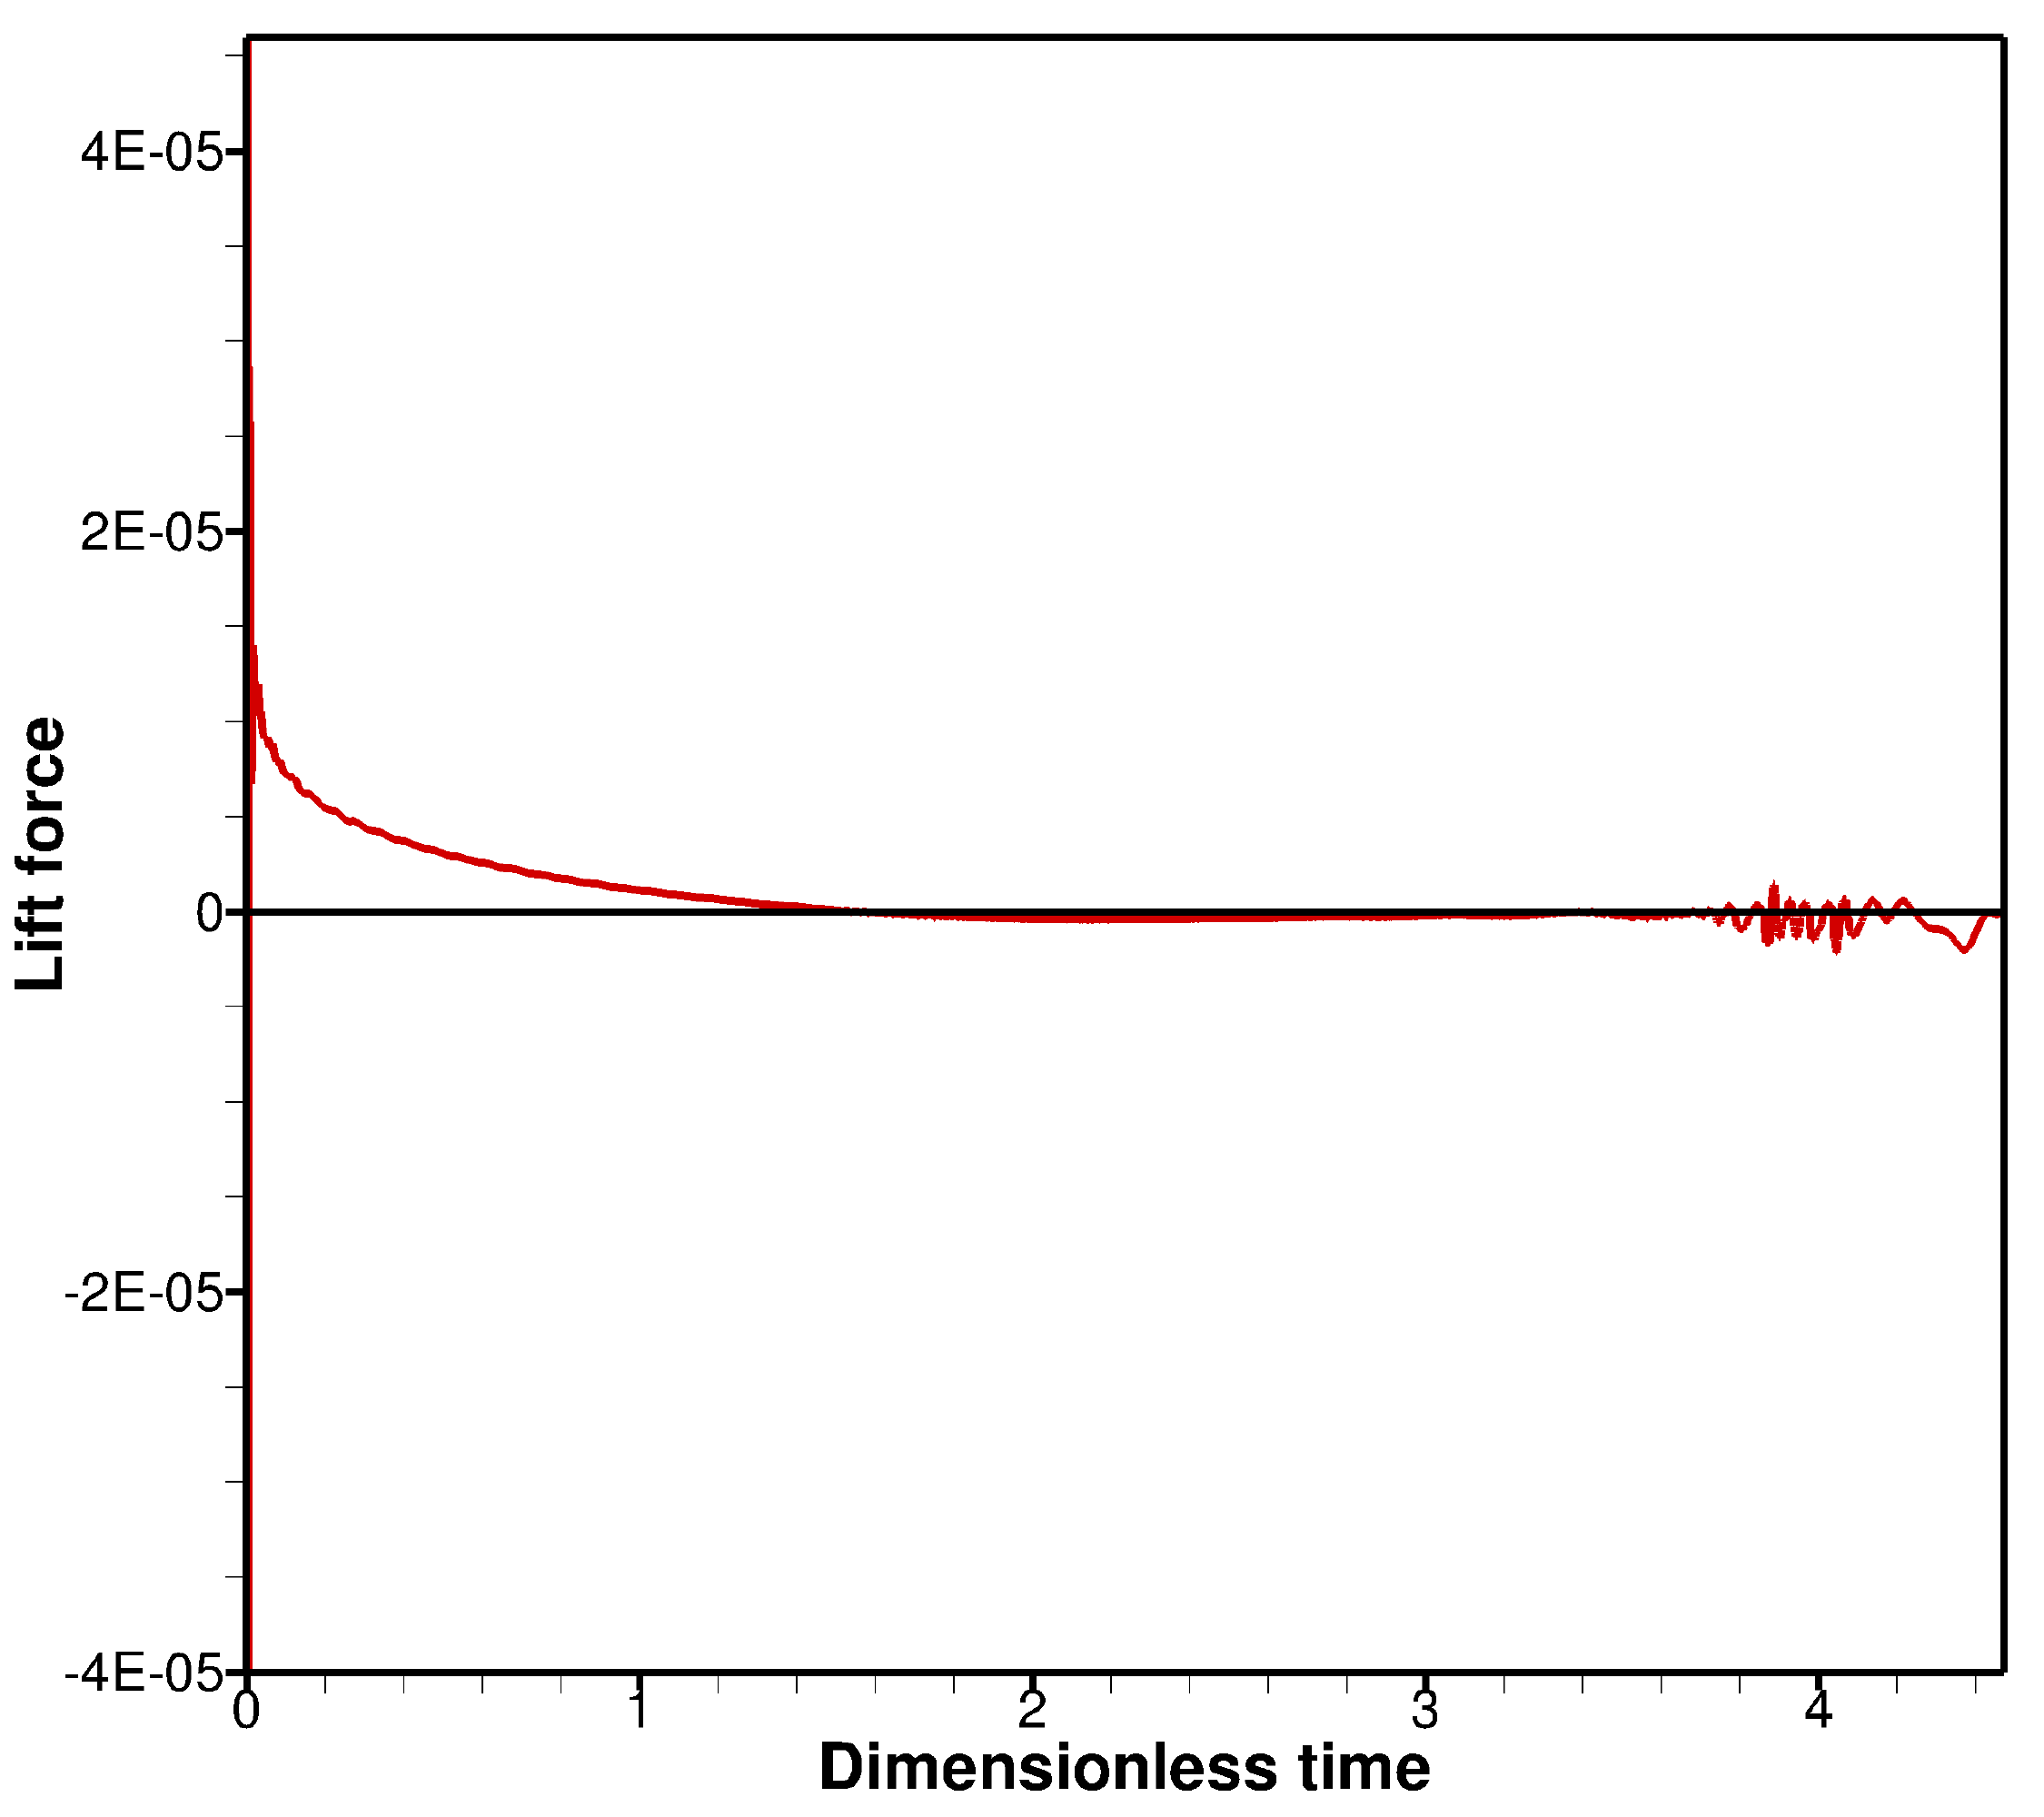} \label{fig:lift_est_disp}}\hfill
	\subfigure[Simulation without estimation of displacement.]{\includegraphics[width=0.495\textwidth]{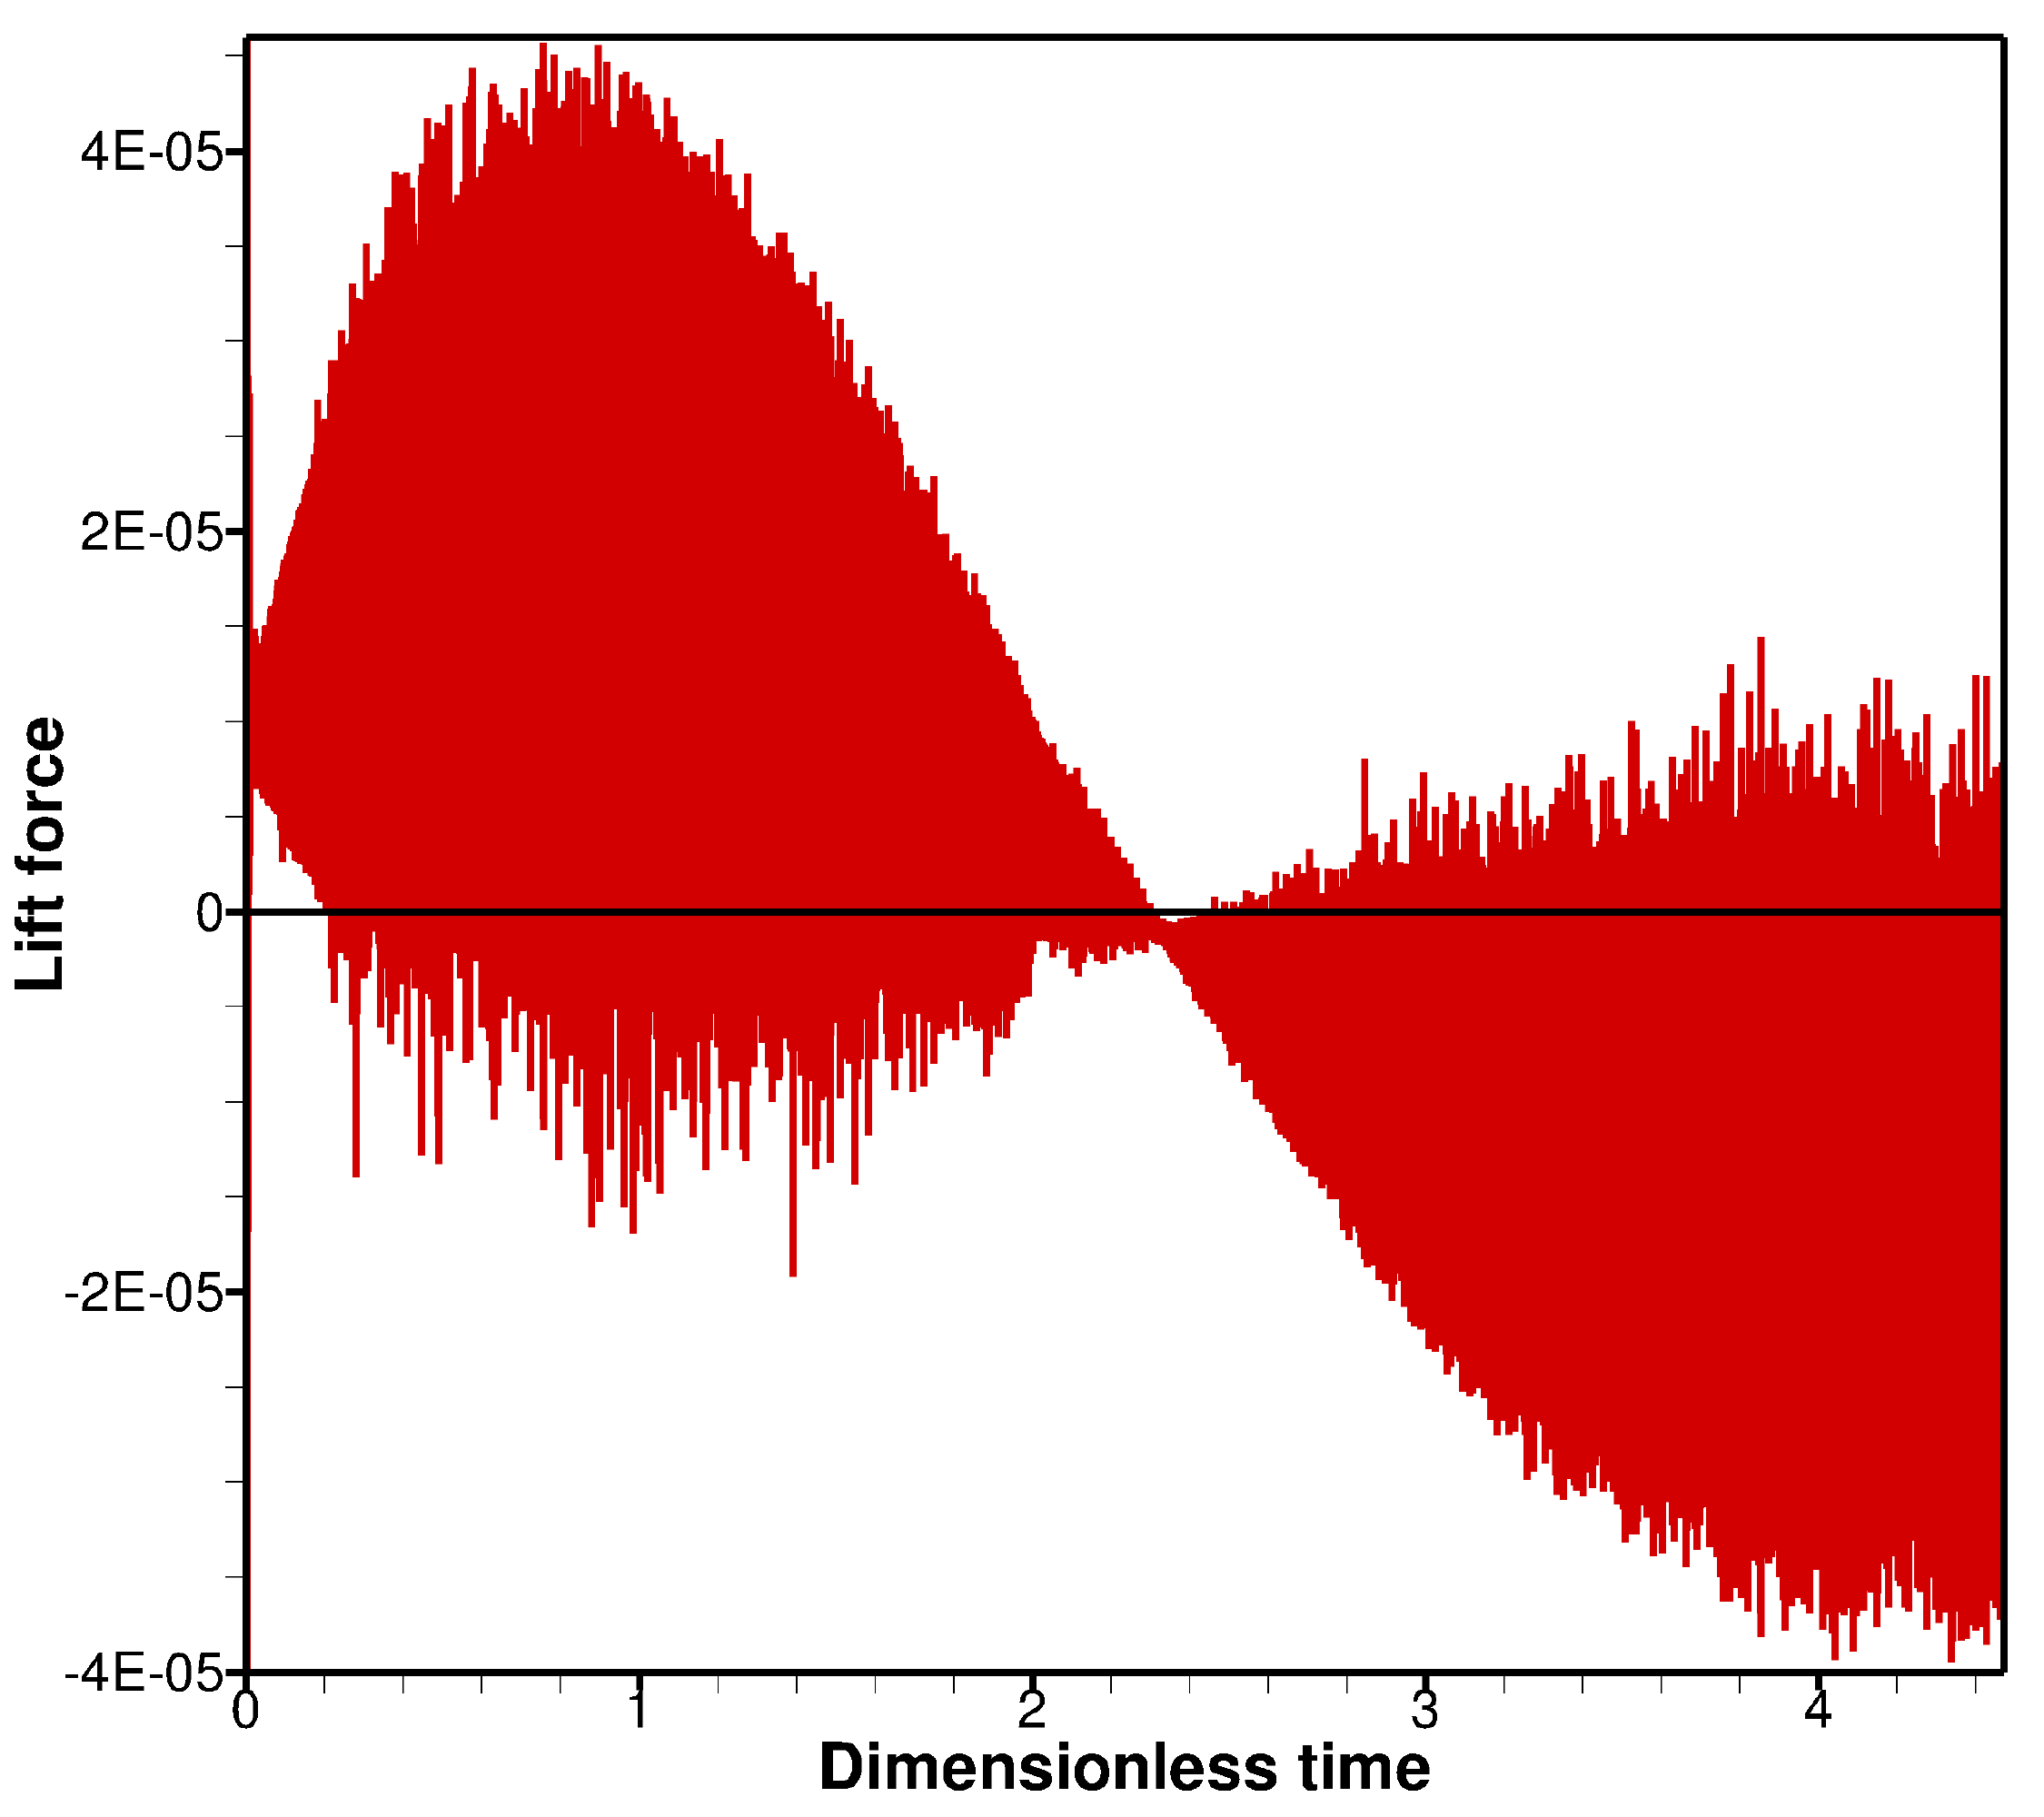}\label{fig:lift_no_est_disp}}\hfill
	\caption{Lift forces for the test cases with and without the prediction of the displacements.}
	\label{fig:lift_comparison}
\end{figure}
\par Finally, the simulation of the fluid-structure interaction with the prediction of the displacements is also approximately $6.7$ times faster, since it requires the computation of less sub-iterations in order to converge. Thus, the estimation of displacements is applied for all simulations in order to enable a faster convergence of the FSI solution and consequently save computational time.

\section{Investigation of the added mass effect}
\label{subsec:added_mass_effect}\markboth{APPENDIX E.$\quad$PREL. STUD. FSI COUP.}{E.1$\quad$INV. OF THE ADDED MASS EFFECT}
\par Added mass is the additional inertia added to a system composed of a fluid and a body, which is submitted to a relative velocity. The deflection of the fluid due to the presence of the body generates additional fluid forces, which act on the surfaces in contact with the flow. This added mass acts as an extra mass on the structural degrees of freedom at the coupling interface and has destabilizing effects on loose coupled algorithms due to their explicit nature. Moreover, the effect of this mass varies also with the time discretization methods utilized by the structural and fluid subproblems (see \mbox{Förster et al.\ \cite{Foerster_2007})}.
\par The relation between the mass of the body and the mass of the displaced fluid \mbox{(see Eq.\ \ref{eq:mass_ratio})} indicates if the added mass effect must be considered.  The higher this relation, the smaller the effect of the added mass and therefore sequentially staggered schemes (loose coupling) are numerically stable and can be utilized (see Causin et al.\ \cite{Causin_2005}).
\begin{equation}
\label{eq:mass_ratio}
m^*=\frac{m^{body}}{m^{fluid}_{disp}}
\end{equation}
\par Song et al.\ \cite{Song_2013} investigated the influence of the added mass effect on stiff plate structures of different materials utilizing a partitioned approach based on a loose coupling algorithm. The case with $m^*=10$ exhibited no convergence problems, while under-relaxation factors were used in the case with $m^*=1$ in order to guarantee the convergence of the solution. Therefore, the influence of the added mass effect for $m^*=10$ was negligible, while this effect was responsible for numerical difficulties for the $m^*=1$ case.  
\par In the present work, the mass ratio between airfoil and displaced fluid is $m^*=720$. Therefore, a loose coupling method ($n_{FSI}=1$) can be utilized due to its numerical stability and lower required computational time (compared to strong coupling approaches). 
\markboth{APPENDIX E.$\quad$PREL. STUD. FSI COUP.}{E.2$\quad$INV. OF THE COUP. ALG.}
\section{Investigation of the coupling algorithm}\markboth{APPENDIX E.$\quad$PREL. STUD. FSI COUP.}{E.2$\quad$INV. OF THE COUP. ALG.}
\label{subsec:investigation_coupling_algorithm}

\par Although the added mass effect is negligible for the NACA0012 FSI test cases (see Appendix \ref{subsec:added_mass_effect}), the accuracy of the loose coupling algorithm is tested through a comparison between the airfoil responses computed with both explicit and implicit coupling approaches. Three simulations with two degrees of freedom (pitch and plunge) are performed with the $m{-}L_3^{min}{-}y_{max}^+$ mesh, the mapping strategy 4 (see Appendix \ref{subsubsec:study_mapping_strategy}), the TFI re-meshing method and the prediction of displacements until a dimensionless time of $t^*=1564.5$ is achieved. The simulated Reynolds number is $Re=30{,}000$ and the utilized linear and torsional stiffnesses are  $k_{l,\,2}=144\,\text{N}{\cdot}\text{m}^{-1}$ and $k_{t,\,3}=0.3832\text{N}\,\text{m}{\cdot}\text{rad}^{-1}$, respectively.
\par The properties of the simulations are summarized in Table \ref{table:comp_FSI_coupling}, regarding that a test case that solves the fluid domain with an implicit coupling algorithm for the first \mbox{$n=100{,}000$} times steps and afterwards with an explicit algorithm is also computed.
\begin{table}[H]
	\centering
	\begin{tabular}{p{2.8cm} p{4.1cm} p{2.0cm} p{3cm} p{1.8cm}}
		\hline
		\multicolumn{1}{c}{\multirow{3}{*}{\centering{\bf{Mesh}}}} & \multicolumn{1}{c}{\multirow{3}{*}{\centering{\bf{Coupling algorithm}}}} & \centering{\bf{Maximal iteration number}} & \centering{\bf{Maximal number of FSI sub-iterations}} & \centering{\bf{Time step size (s)}}\tabularnewline \hline
		\centering{$m{-}L_3^{min}-y^{+}_{max}$} & \centering{Loose} & \centering{$3{,}500{,}000$} & \centering{1} & \centering{$1\cdot10^{-5}$} \tabularnewline \hline
		\centering{$m{-}L_3^{min}{-}y^+_{max}$} & \centering{Strong} & \centering{$3{,}500{,}000$} &\centering{20} & \centering{$1\cdot10^{-5}$} \tabularnewline \hline
		\multicolumn{1}{c}{\multirow{2}{*}{\centering{$m{-}L_3^{min}{-}y^+_{max}$}}} & \centering{Strong for $n\leq100{,}000$} & \centering{$100{,}000$} & \multicolumn{1}{c}{\centering{20}} & \multicolumn{1}{c}{\multirow{2}{*}{\centering{$1\cdot10^{-5}$}}} \tabularnewline	\cline{2-4}
		& \centering{Loose for $n>100{,}000$} & \centering{$3{,}500{,}000$} & \centering{1} & \tabularnewline
		\hline	
	\end{tabular}
	\caption{\label{table:comp_FSI_coupling}Simulation properties of the test cases aimed at the comparison of the coupling algorithms.}
\end{table}
\par The maximal number of sub-iterations is set to $n_{FSI}=20$ for the cases with strong coupling, since this is sufficient and necessary to achieve the convergence criterion of all computed time steps, especially during the initialization phase. After this phase, however, only two sub-iterations are in general utilized by the FSI solver (see Section \ref{subsec:investigation_estimation_displacement}), due to the fact that the convergence criterion is achieved before all sub-iterations are performed.
\par The airfoil structural responses in the form of translational displacements in the \mbox{$x_2$-direction} and rotational displacements about the $x_3$-axis are illustrated in Fig.\ \ref{fig:displacements_coupling_investigation} as a function of the time. Since the fluid movement is chaotic, a direct comparison of the displacements achieved by the different coupling algorithms is not possible. Therefore, only the oscillation amplitudes are studied and compared.
\par All simulated coupling algorithms are characterized by the achievement of the same maximal amplitude of oscillation, regarding the plunge and pitch degrees of freedom. For instance, these values are \mbox{$X_2=1.8{\cdot}10^{-4}\,\text{m}$} and \mbox{$\varphi_3=0.33^\circ$} for the translational and rotational motions, respectively. Although the various coupling algorithms require different initialization times in order to achieve a limit-cycle oscillation, the amplitudes of these oscillations are also the same for all coupling approaches, that is, \mbox{$X_{2,\,LCO}=1.8{\cdot}10^{-4}\,\text{m}$} and \mbox{$\varphi_{3,\,LCO}=0.0135^\circ$}.
\begin{figure}[H]
	\centering
	\subfigure[Loose coupling algorithm: Translational displacement $X_2$.]{\includegraphics[width=0.48\textwidth]{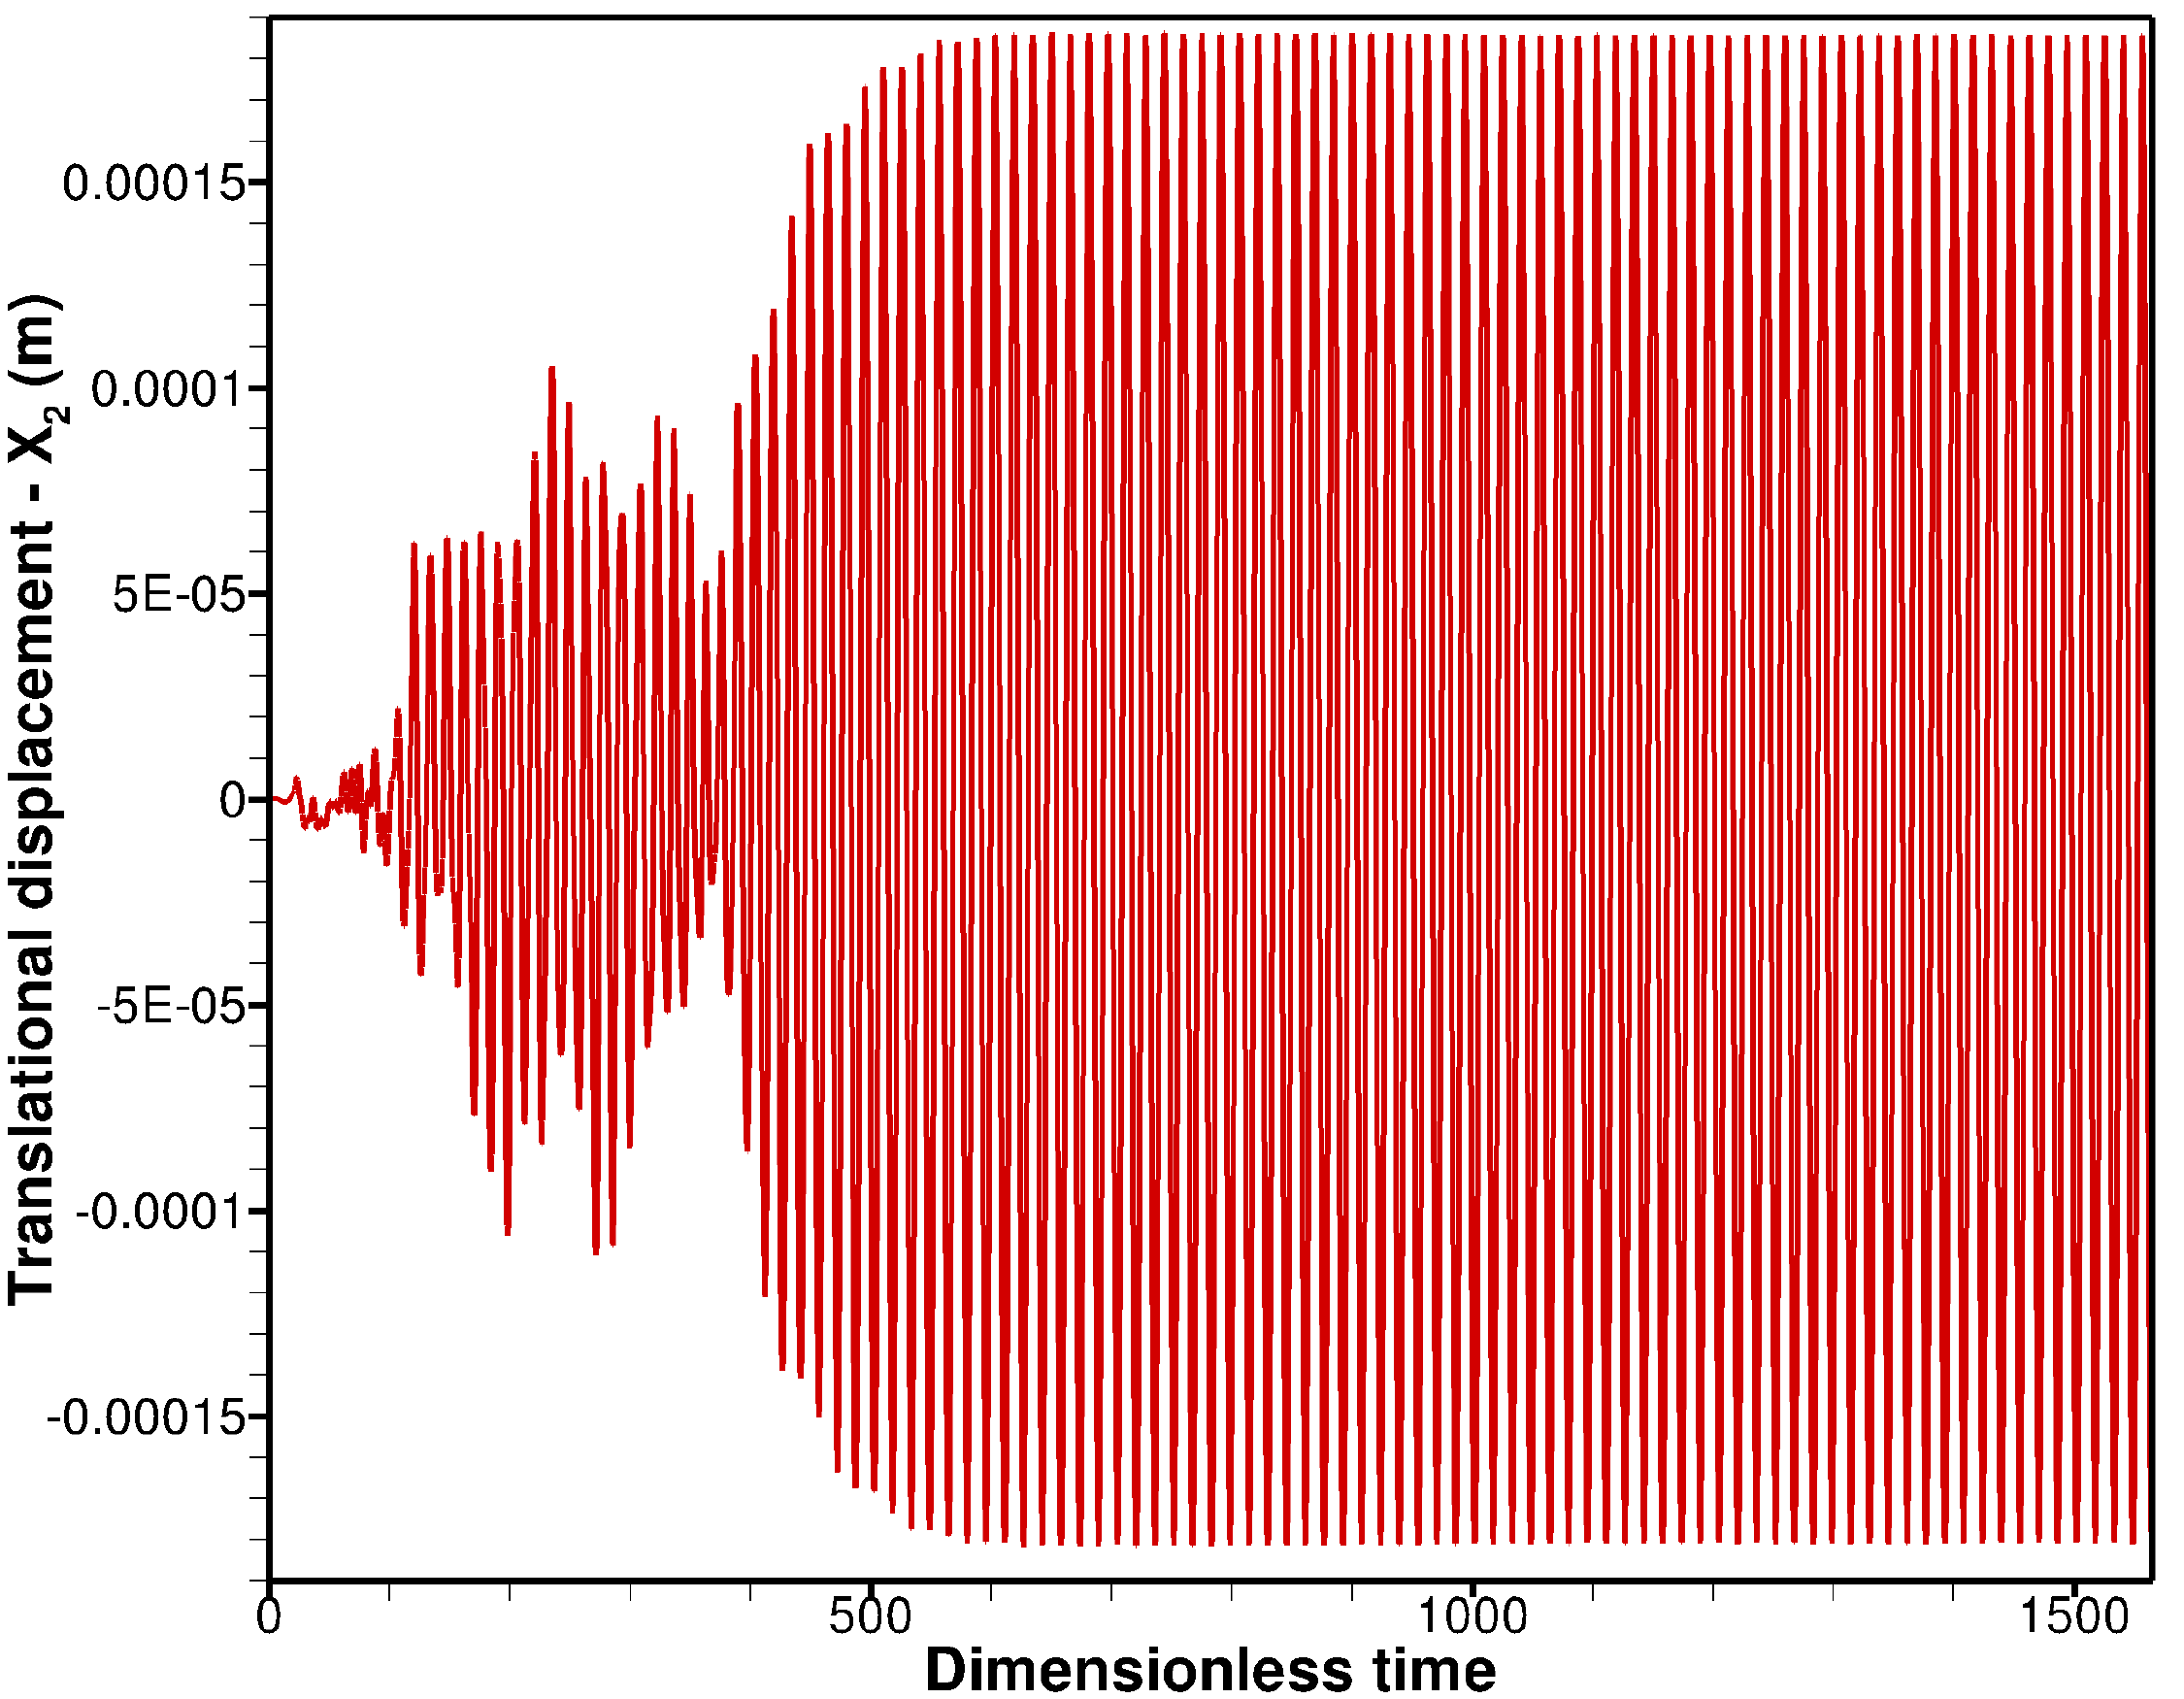} \label{fig:frequenciess_translation}}\hfill
	\subfigure[Loose coupling algorithm: Rotational displacement $\varphi_3$.]{\includegraphics[width=0.48\textwidth]{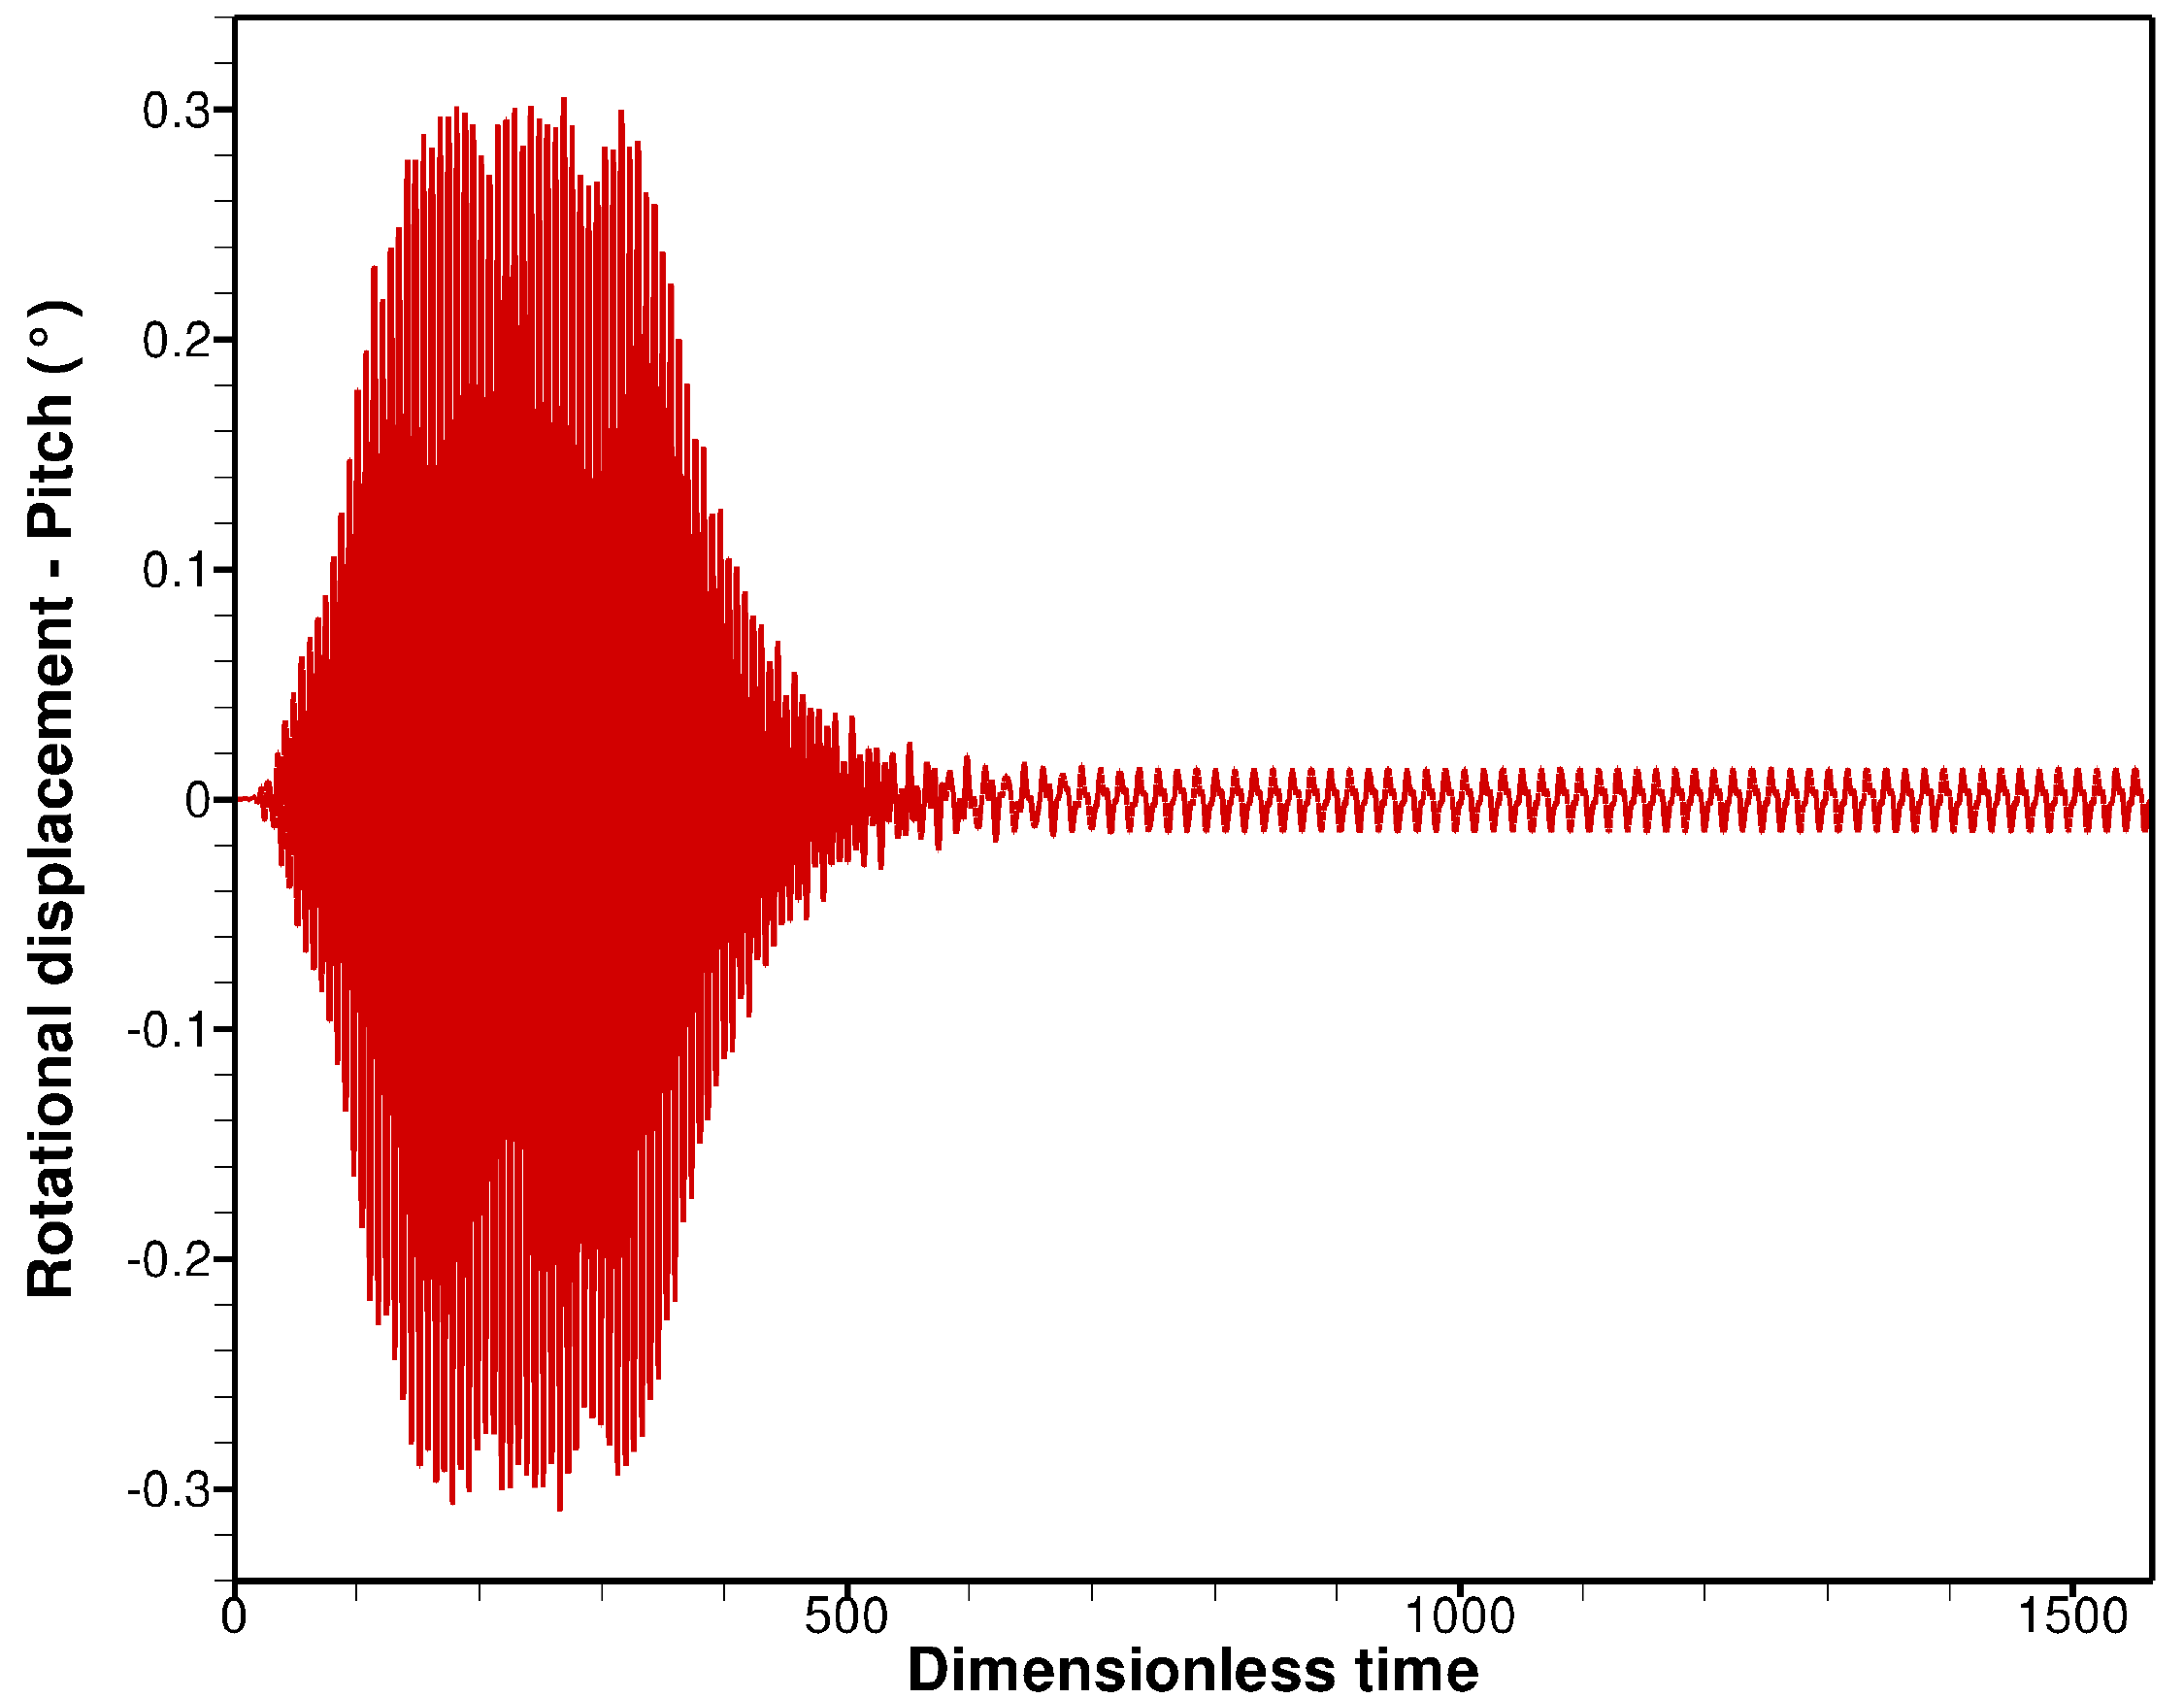}\label{fig:frequencies_rsotation}}\hfill
	\centering
	\subfigure[Strong coupling algorithm for $t\leq1\,s$ and loose coupling algorithm for $t>1\,s$: Translational displacement $X_2$.]{\includegraphics[width=0.48\textwidth]{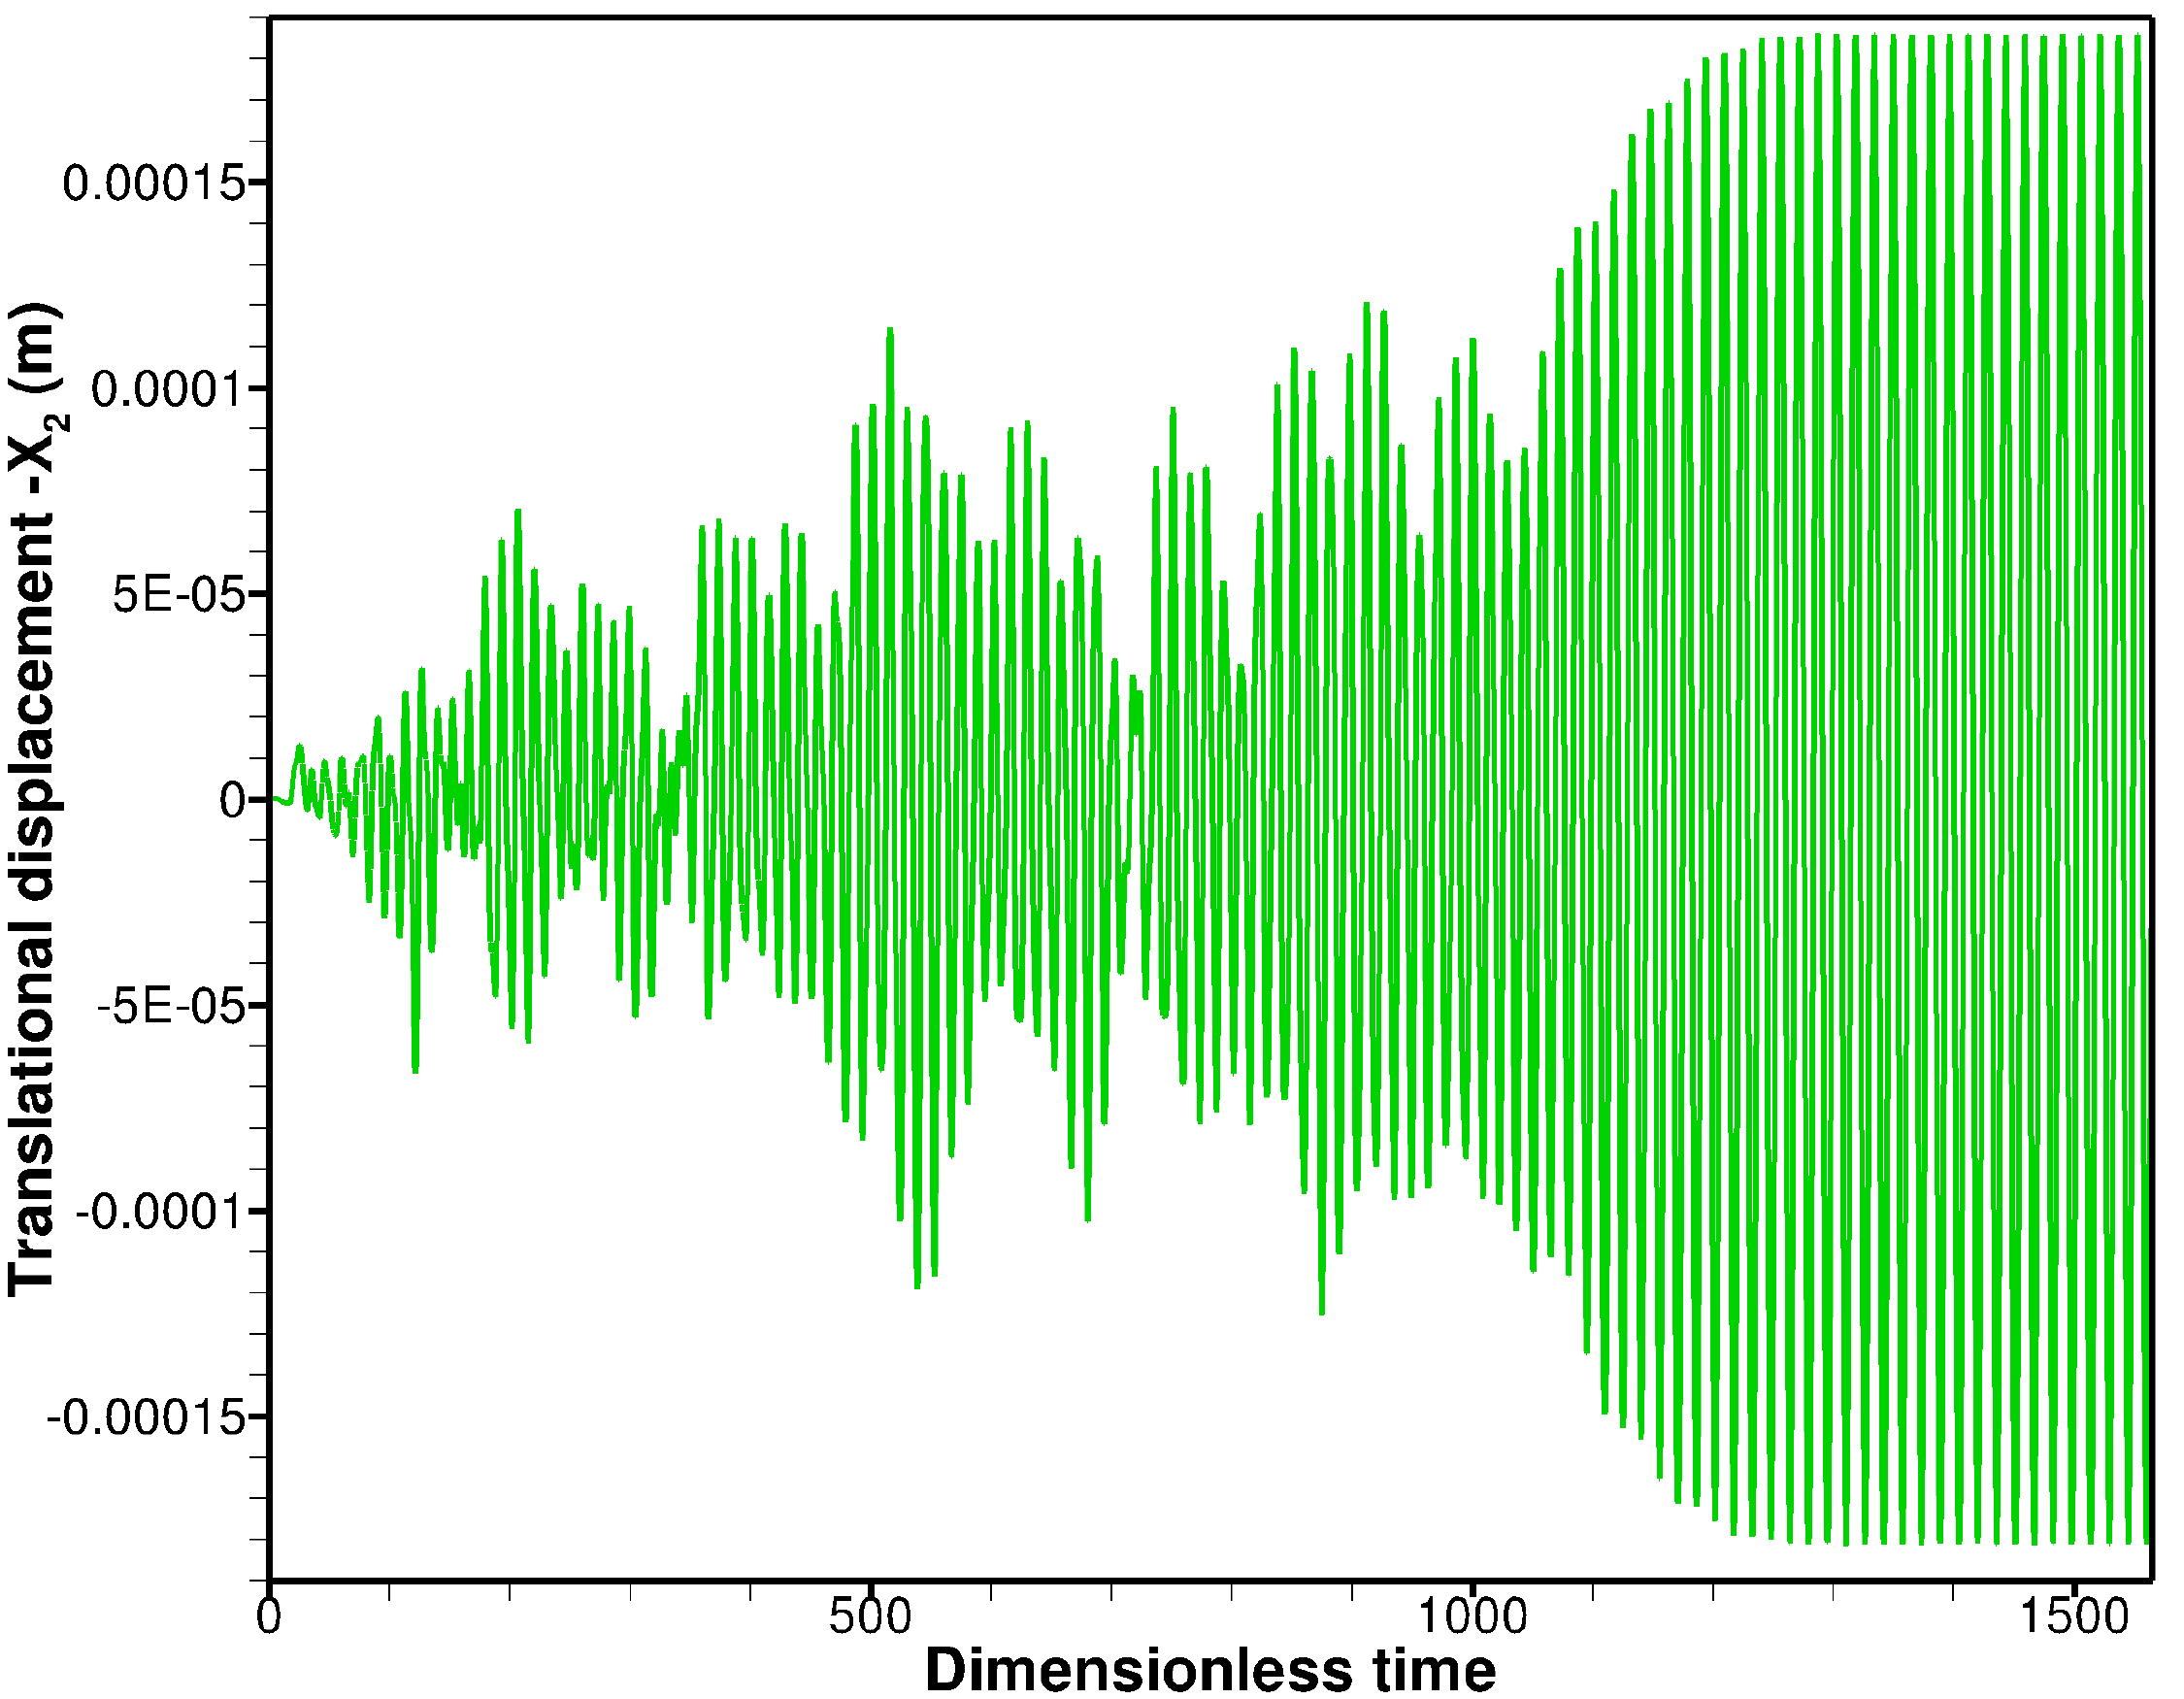} \label{fig:frequencies_translatison}}\hfill
	\subfigure[Strong coupling algorithm for $t\leq1\,s$ and loose coupling algorithm for $t>1\,s$: Rotational displacement $\varphi_3$.]{\includegraphics[width=0.48\textwidth]{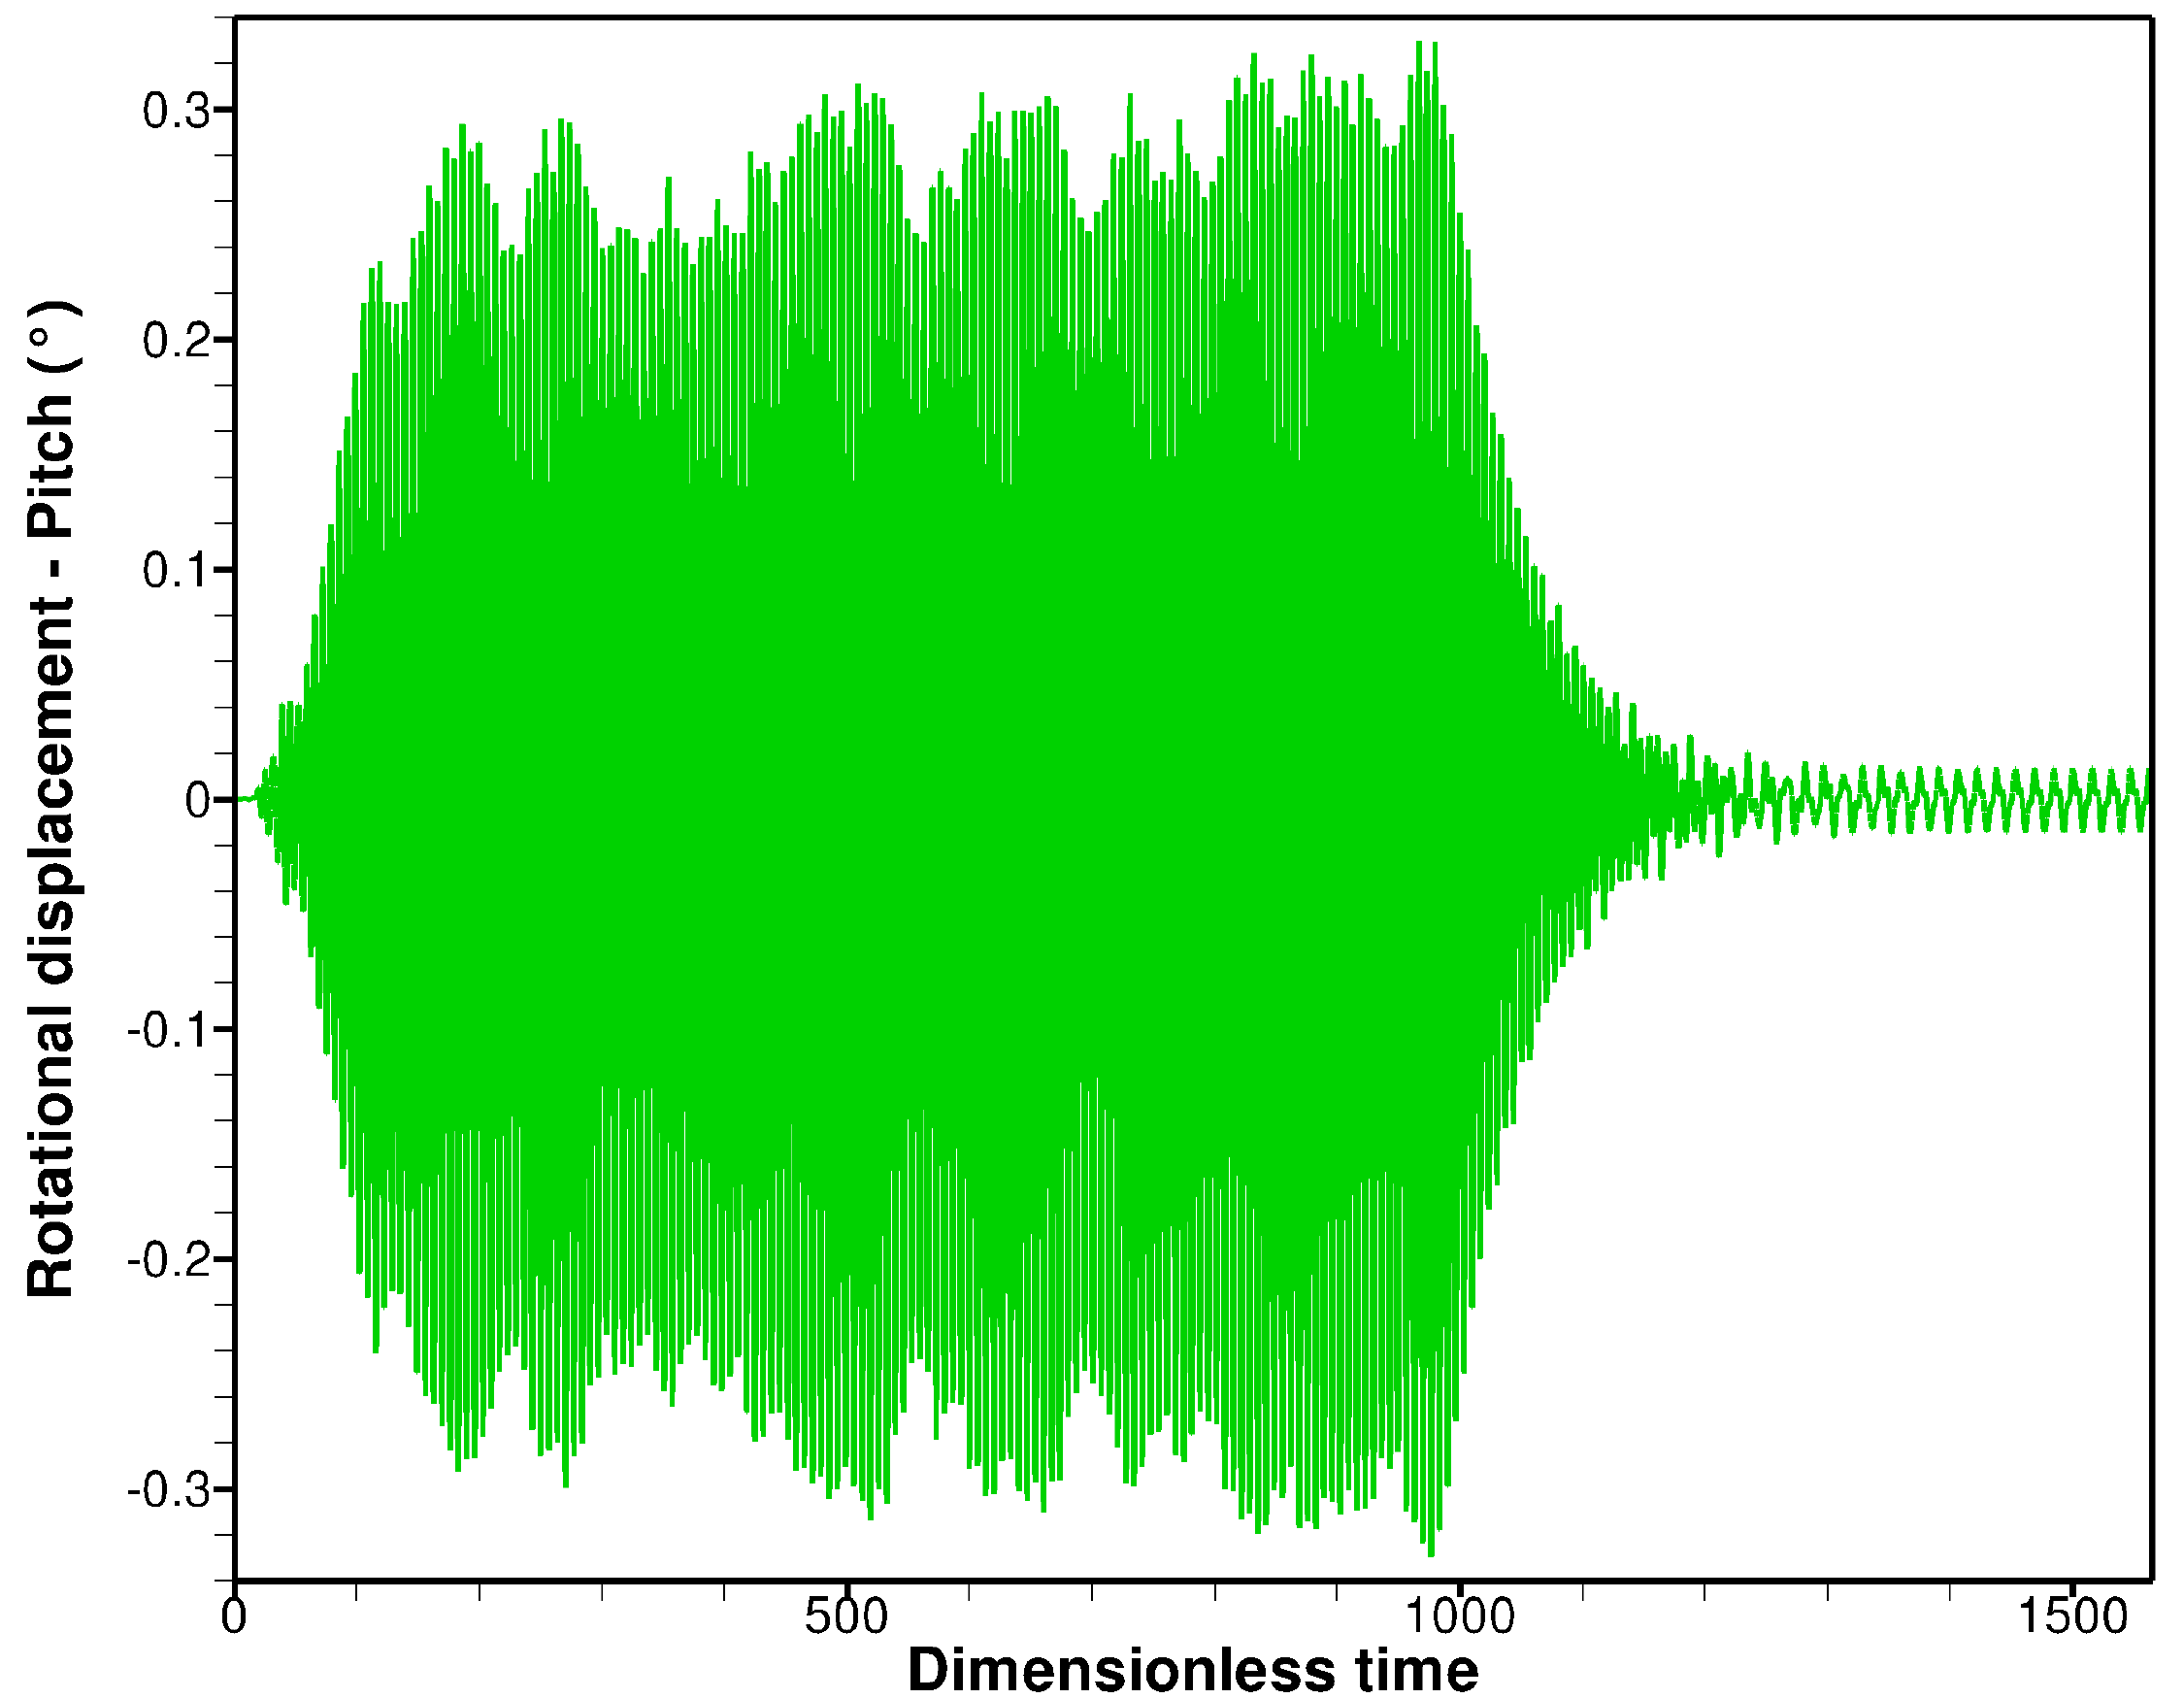} \label{fig:frequencies_translatiosn}}\hfill
\end{figure}
\begin{figure}[H]
	\subfigure[Strong coupling algorithm: Translational displacement $X_2$.]{\includegraphics[width=0.48\textwidth]{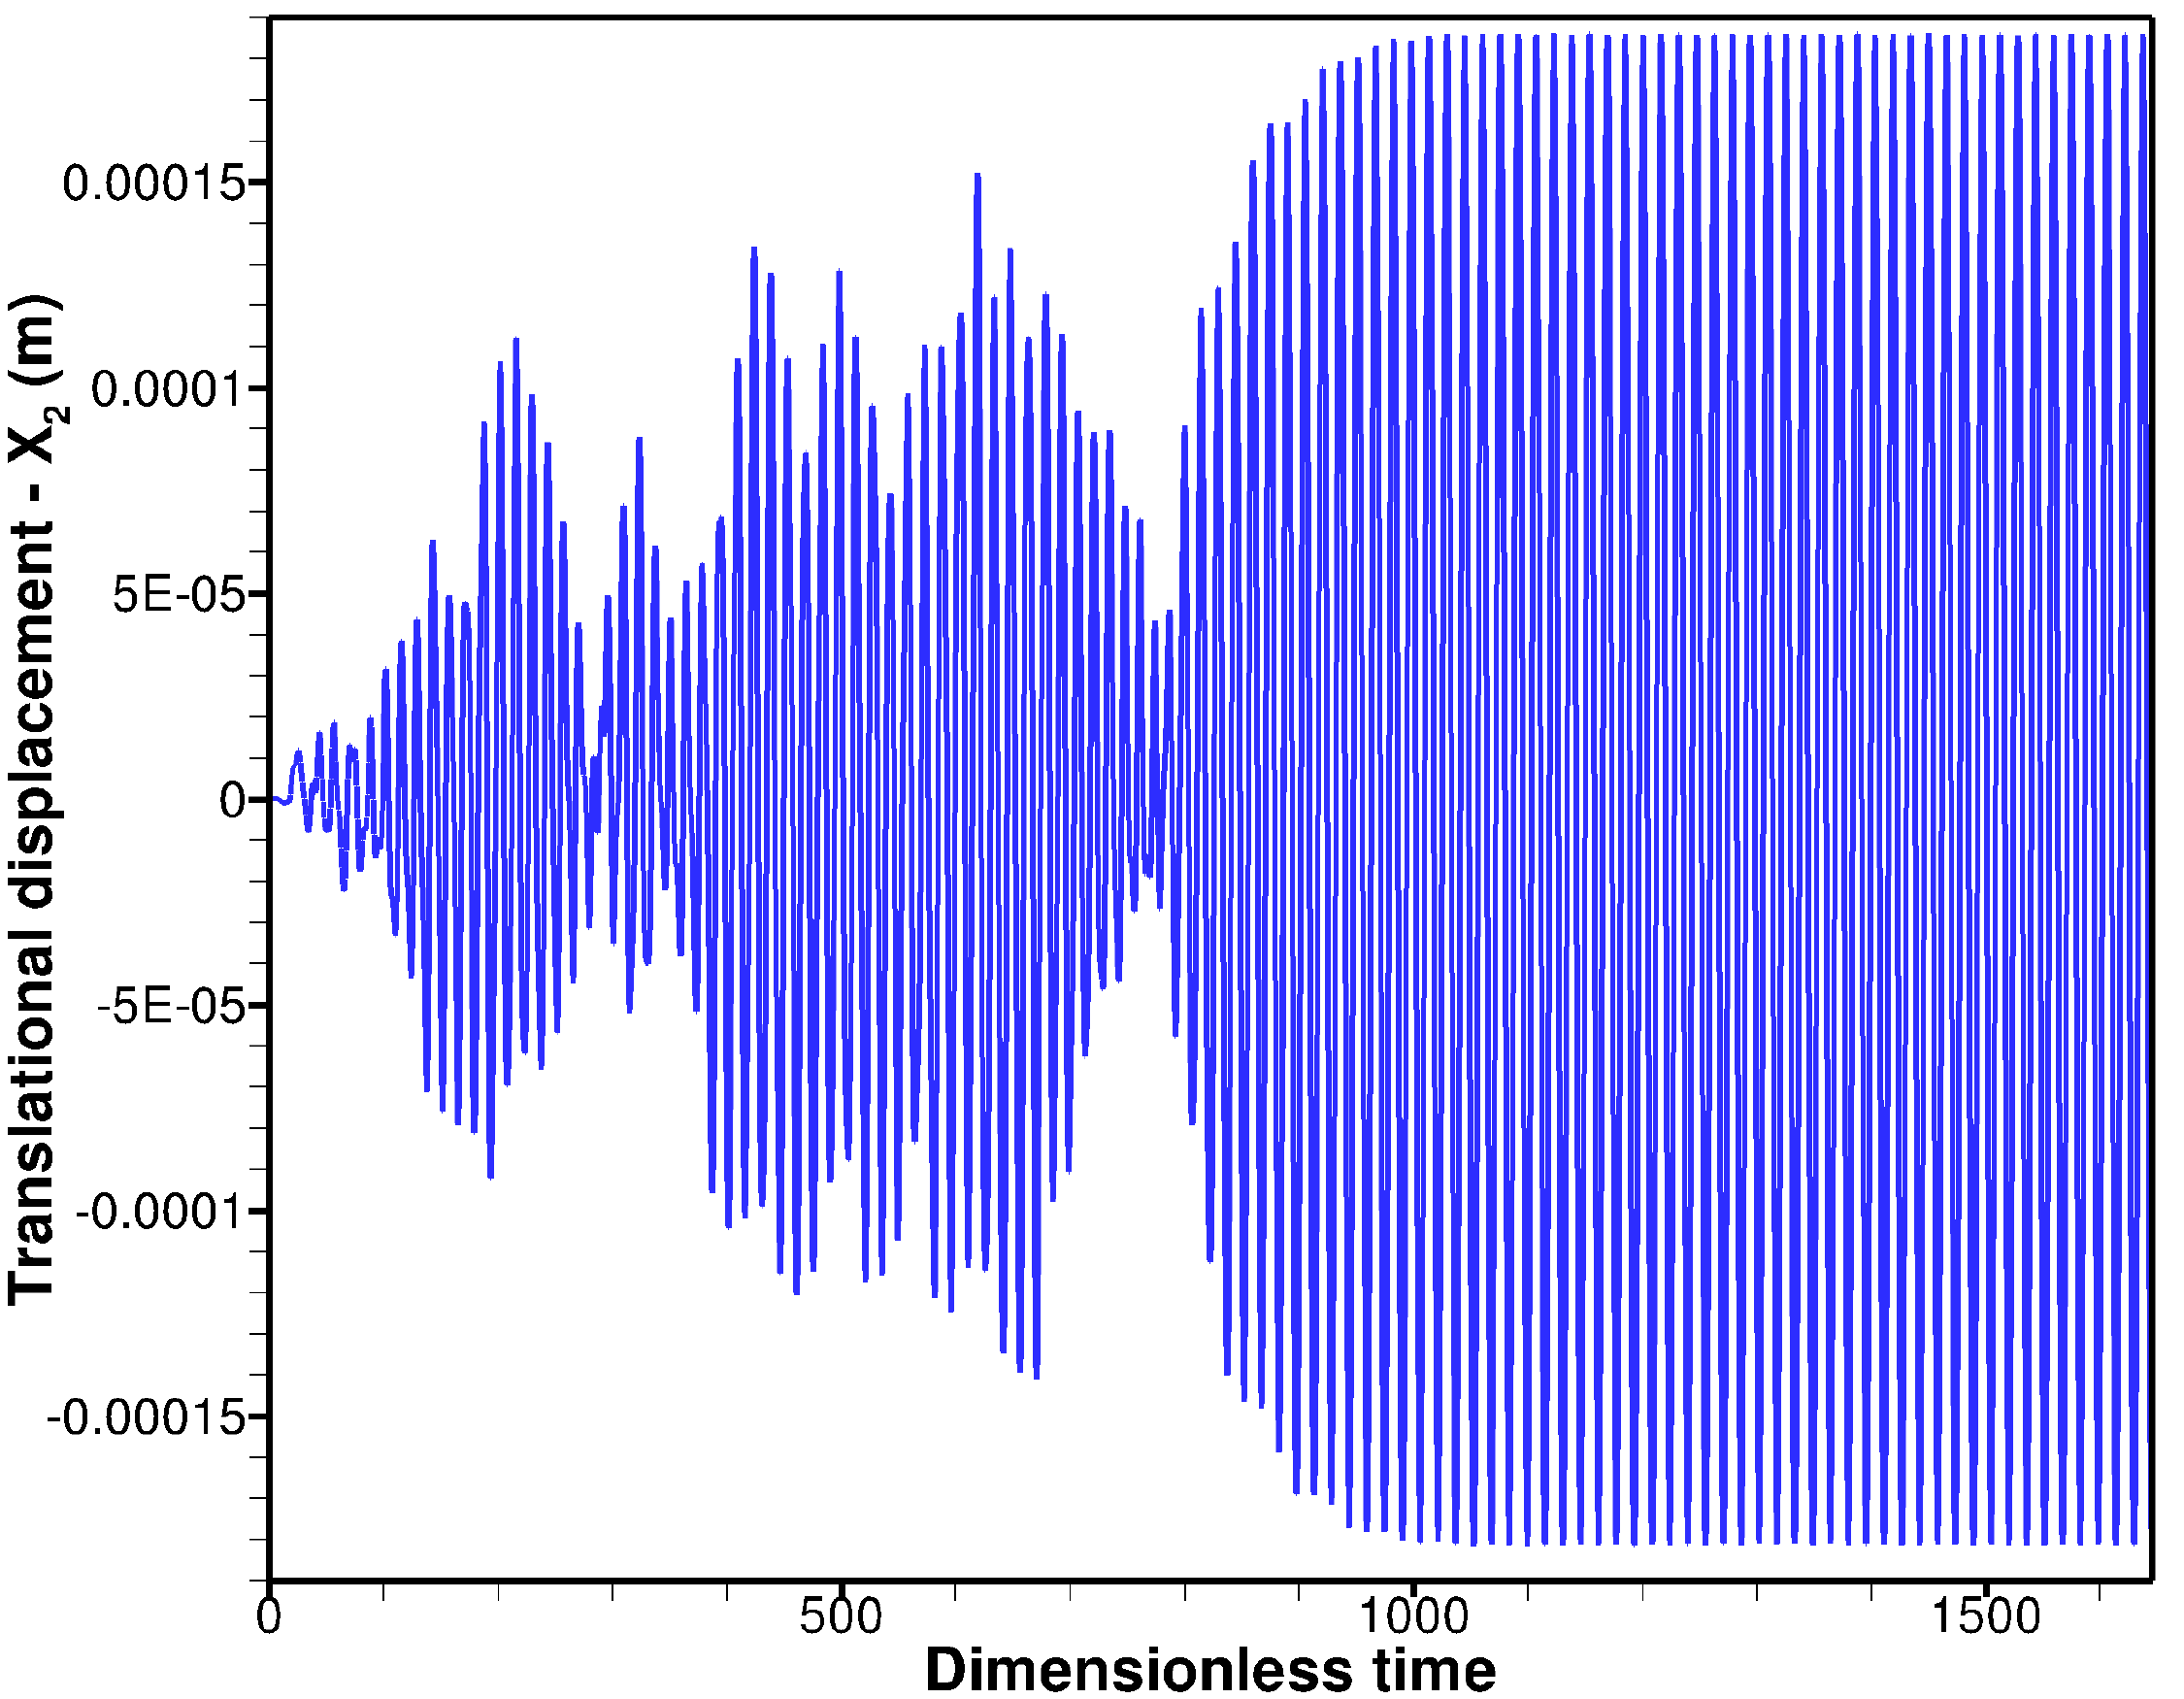} \label{fig:frequencies_translatsiosn}}\hfill
	\subfigure[Strong coupling algorithm: Rotational displacement $\varphi_3$.]{\includegraphics[width=0.48\textwidth]{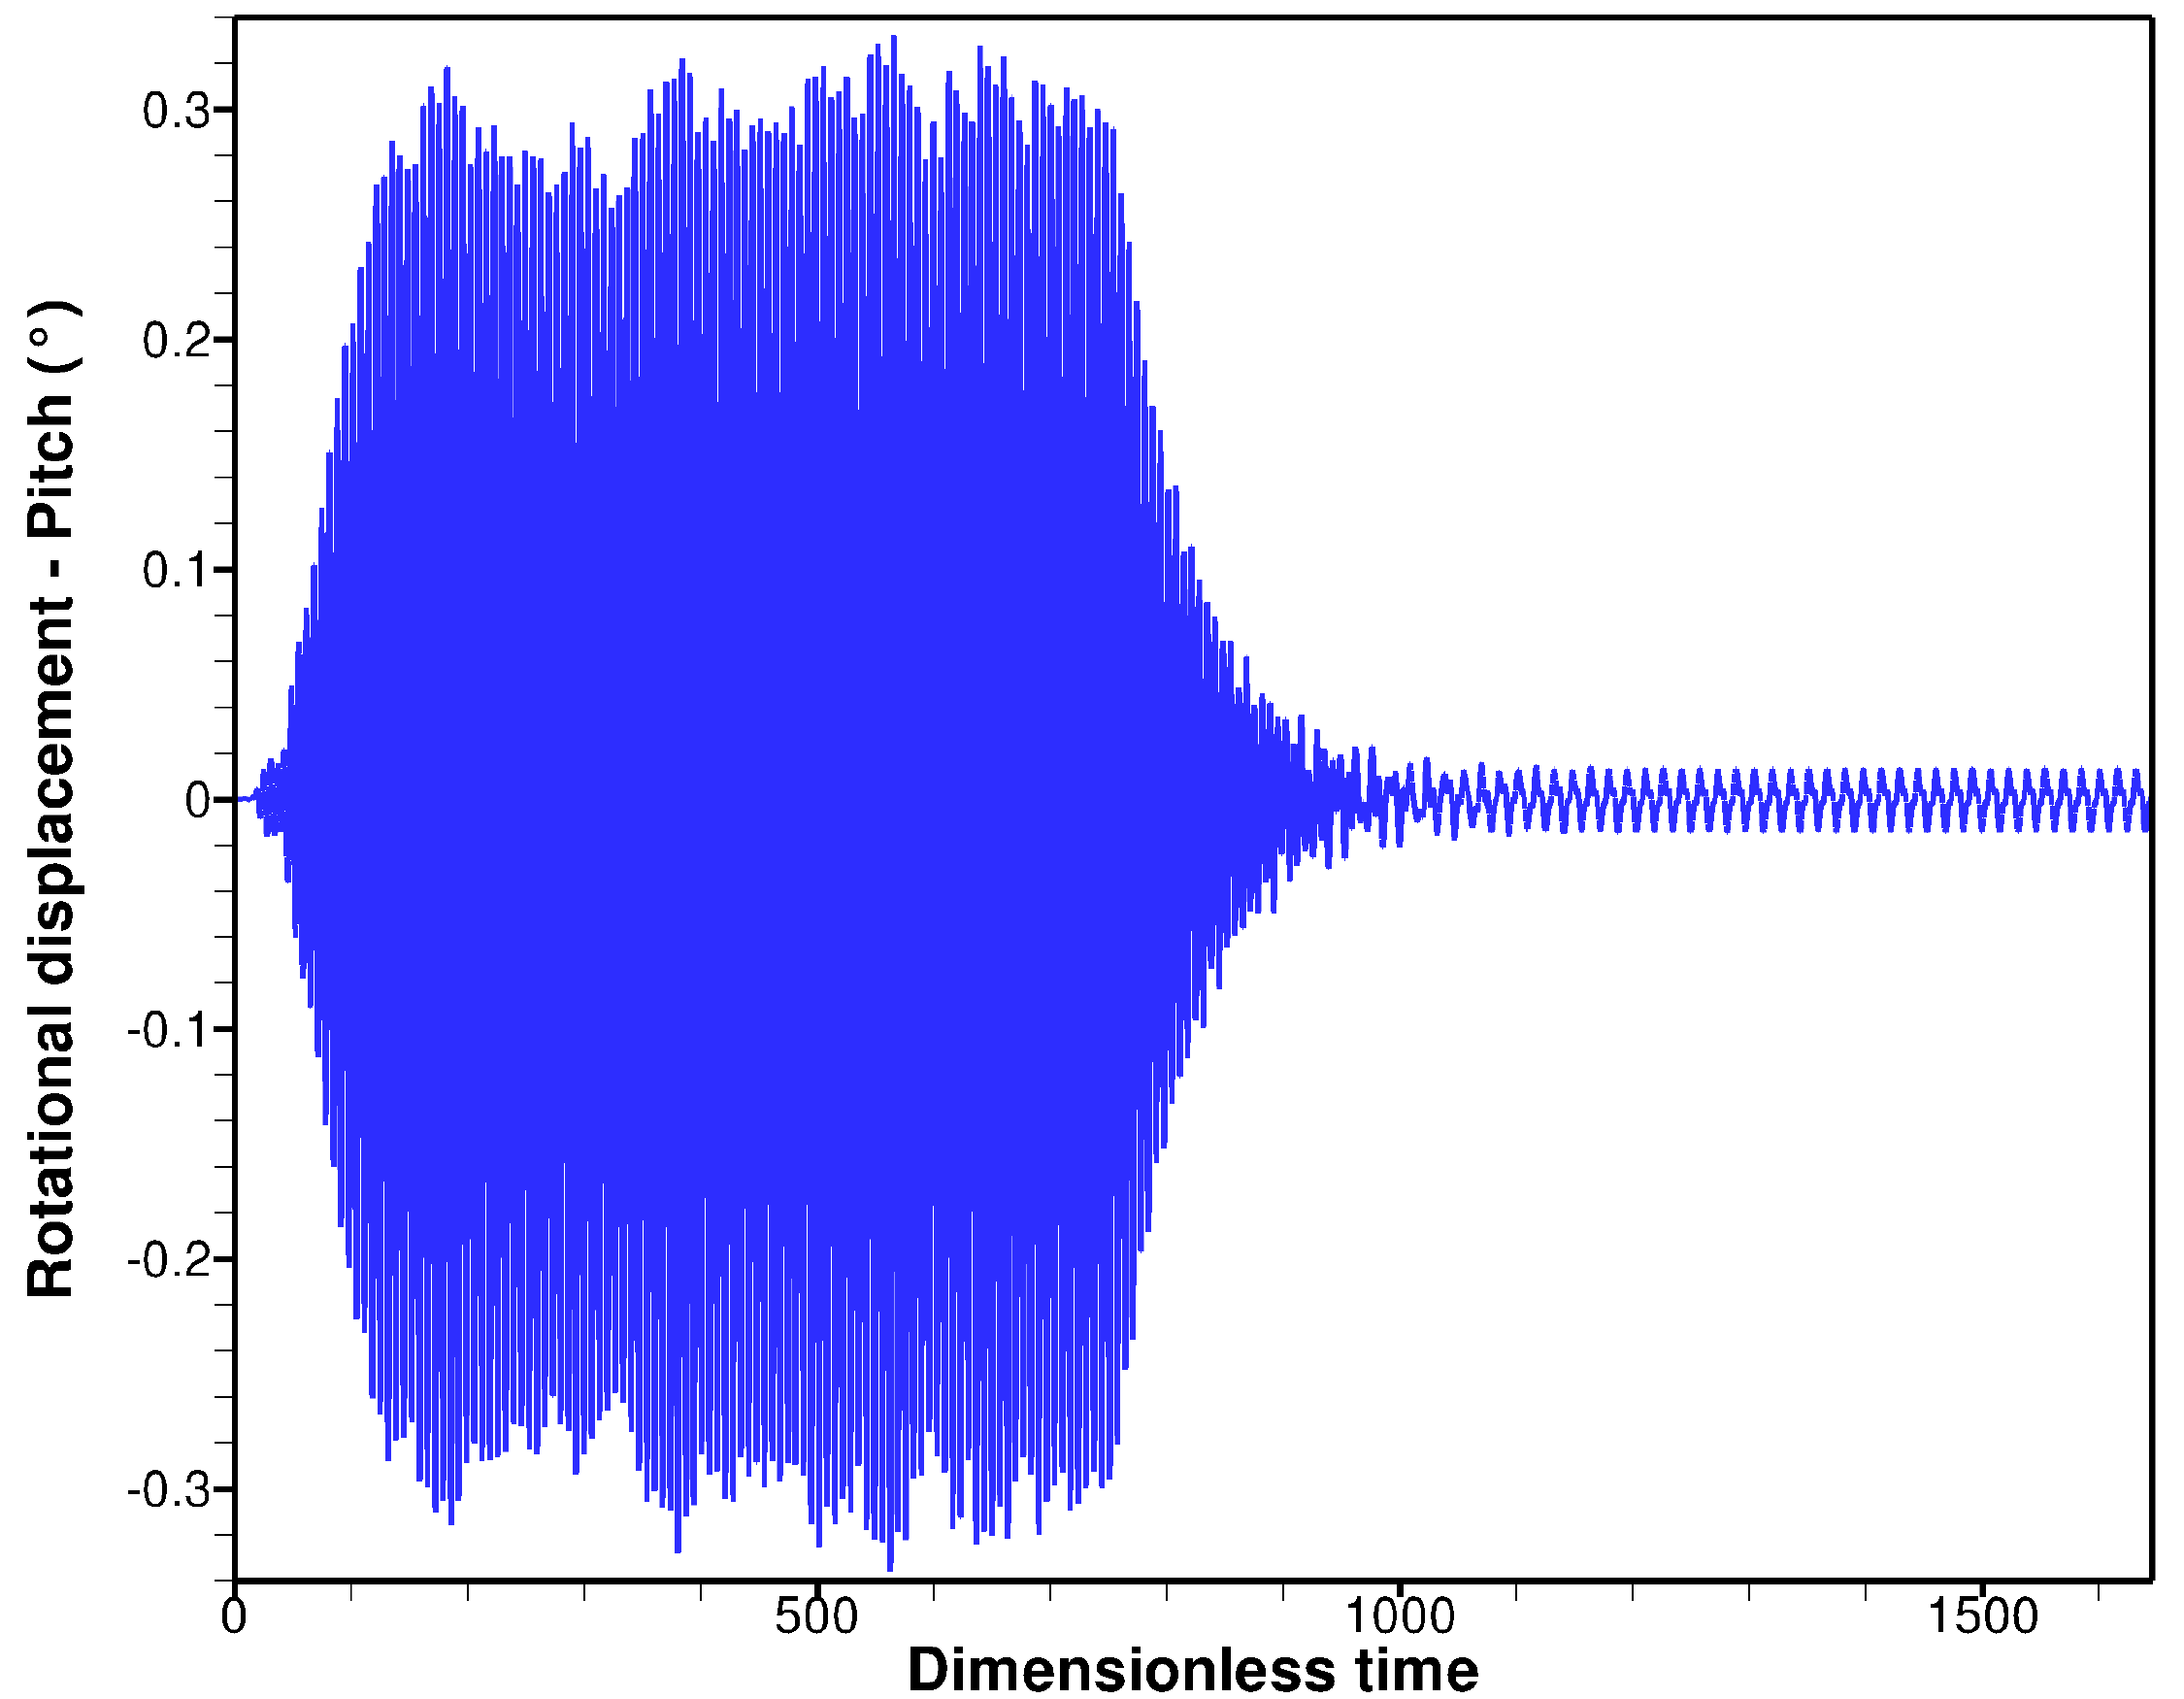} \label{fig:frequencies_stranslation}}\hfill
	\caption{Comparison of the coupling algorithms: Translational ($X_2$) and rotational ($\varphi_3$) displacements.}
	\label{fig:displacements_coupling_investigation}
\end{figure}
\par Since the amplitudes achieved with the loose coupling algorithm are in a good agreement with the ones achieved with both other simulated test cases, this coupling does not influence the computation of the fluid domain and therefore is applicable to further simulate the fluid structure interaction between the NACA0012 airfoil and the flow. This result is expected, since this FSI is characterized by a negligible added mass effect (see \mbox{Appendix \ref{subsec:added_mass_effect}).} Nevertheless, the frequencies generated by the fluid-structure interaction are also investigated.
\par In order to analyze the frequency domain, a Fourier transform with a Hamming window is carried out, considering that the independent variable is the time $t$ and that the dependent variables are the plunge and pitch displacements, i$.$e$.$, respectively $X_2$ and $\varphi_3$. The latter are utilized as parameters for the Fourier transform since these generate more distinct peaks in the frequency domain, when compared to the lift and drag forces, facilitating the comparison of the coupling algorithms. The frequency domain of the translational and rotational displacements are illustrated in Fig.\ \ref{fig:frequencies_displacements_coupling}, regarding that the amplitudes are normalized in relation to the maximal value. The frequency domain of the simulation characterized by the utilization of both loose and strong coupling algorithms is not displayed since only unclear frequency peaks are formed due to the fact that this test case requires a longer initialization time and therefore not enough data regarding the fully developed state is available. 
\par The frequencies of the three peaks characterized by the highest amplitudes are described in \mbox{Table \ref{table:frequencies_coupling}} for both strong and loose coupling algorithms. The origin of the generated frequencies and their physical or numerical meaning are not investigated, since these test cases aim only at the comparison of the coupling algorithms. Since only minor deviations are present in the frequencies generated by both coupling algorithms, it is confirmed that the coupling method does not influence the calculation of the coupled problem. 
\par Finally, the computational time of all simulations are compared, according to \mbox{Table \ref{table:compt_time_coupling}}. The loose coupling algorithm requires about $85\%$ and $56\%$ of the computational time of respectively the test case characterized by the utilization of both couplings and the one applying solely the loose coupling algorithm. Since it is also proven that the explicit coupling is accurate, this is utilized for the further investigations of the fluid-structure interaction.
\begin{figure}[H]
	\centering
	\subfigure[Loose coupling.]{\includegraphics[width=0.48\textwidth]{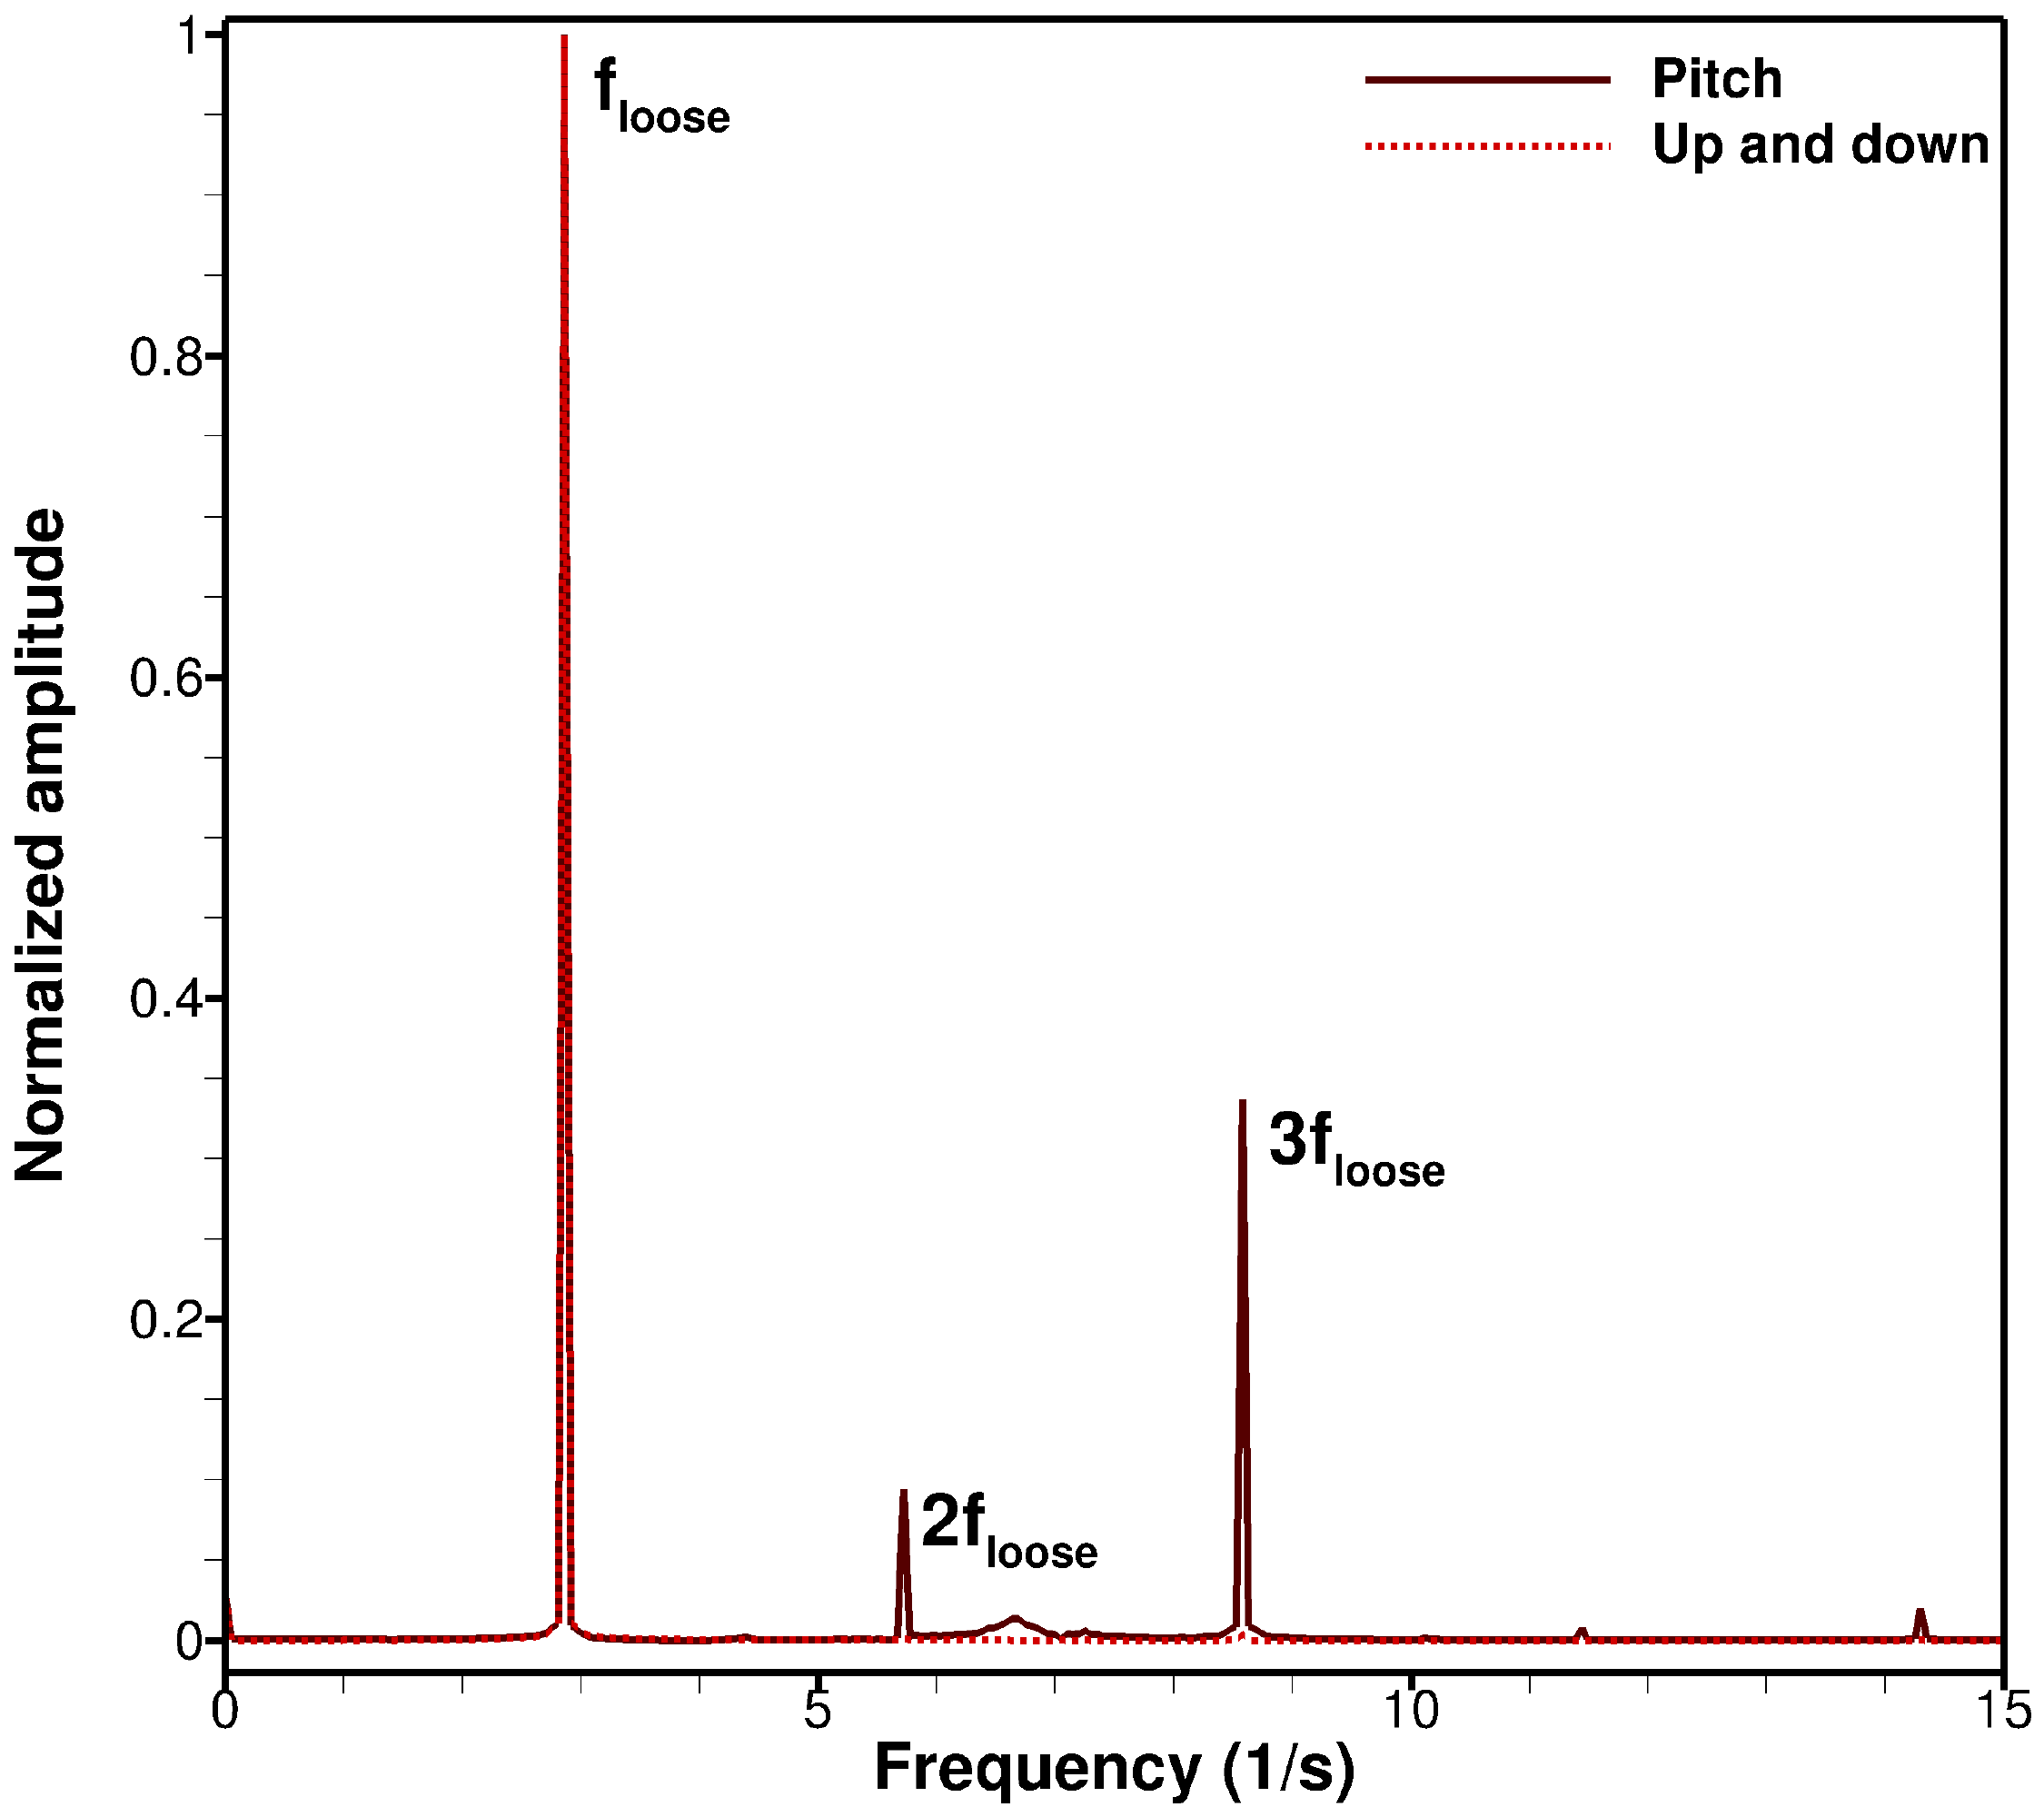} \label{fig:frequencies_loose}}\hfill
	\subfigure[Strong coupling. BLABLA]{\includegraphics[width=0.48\textwidth]{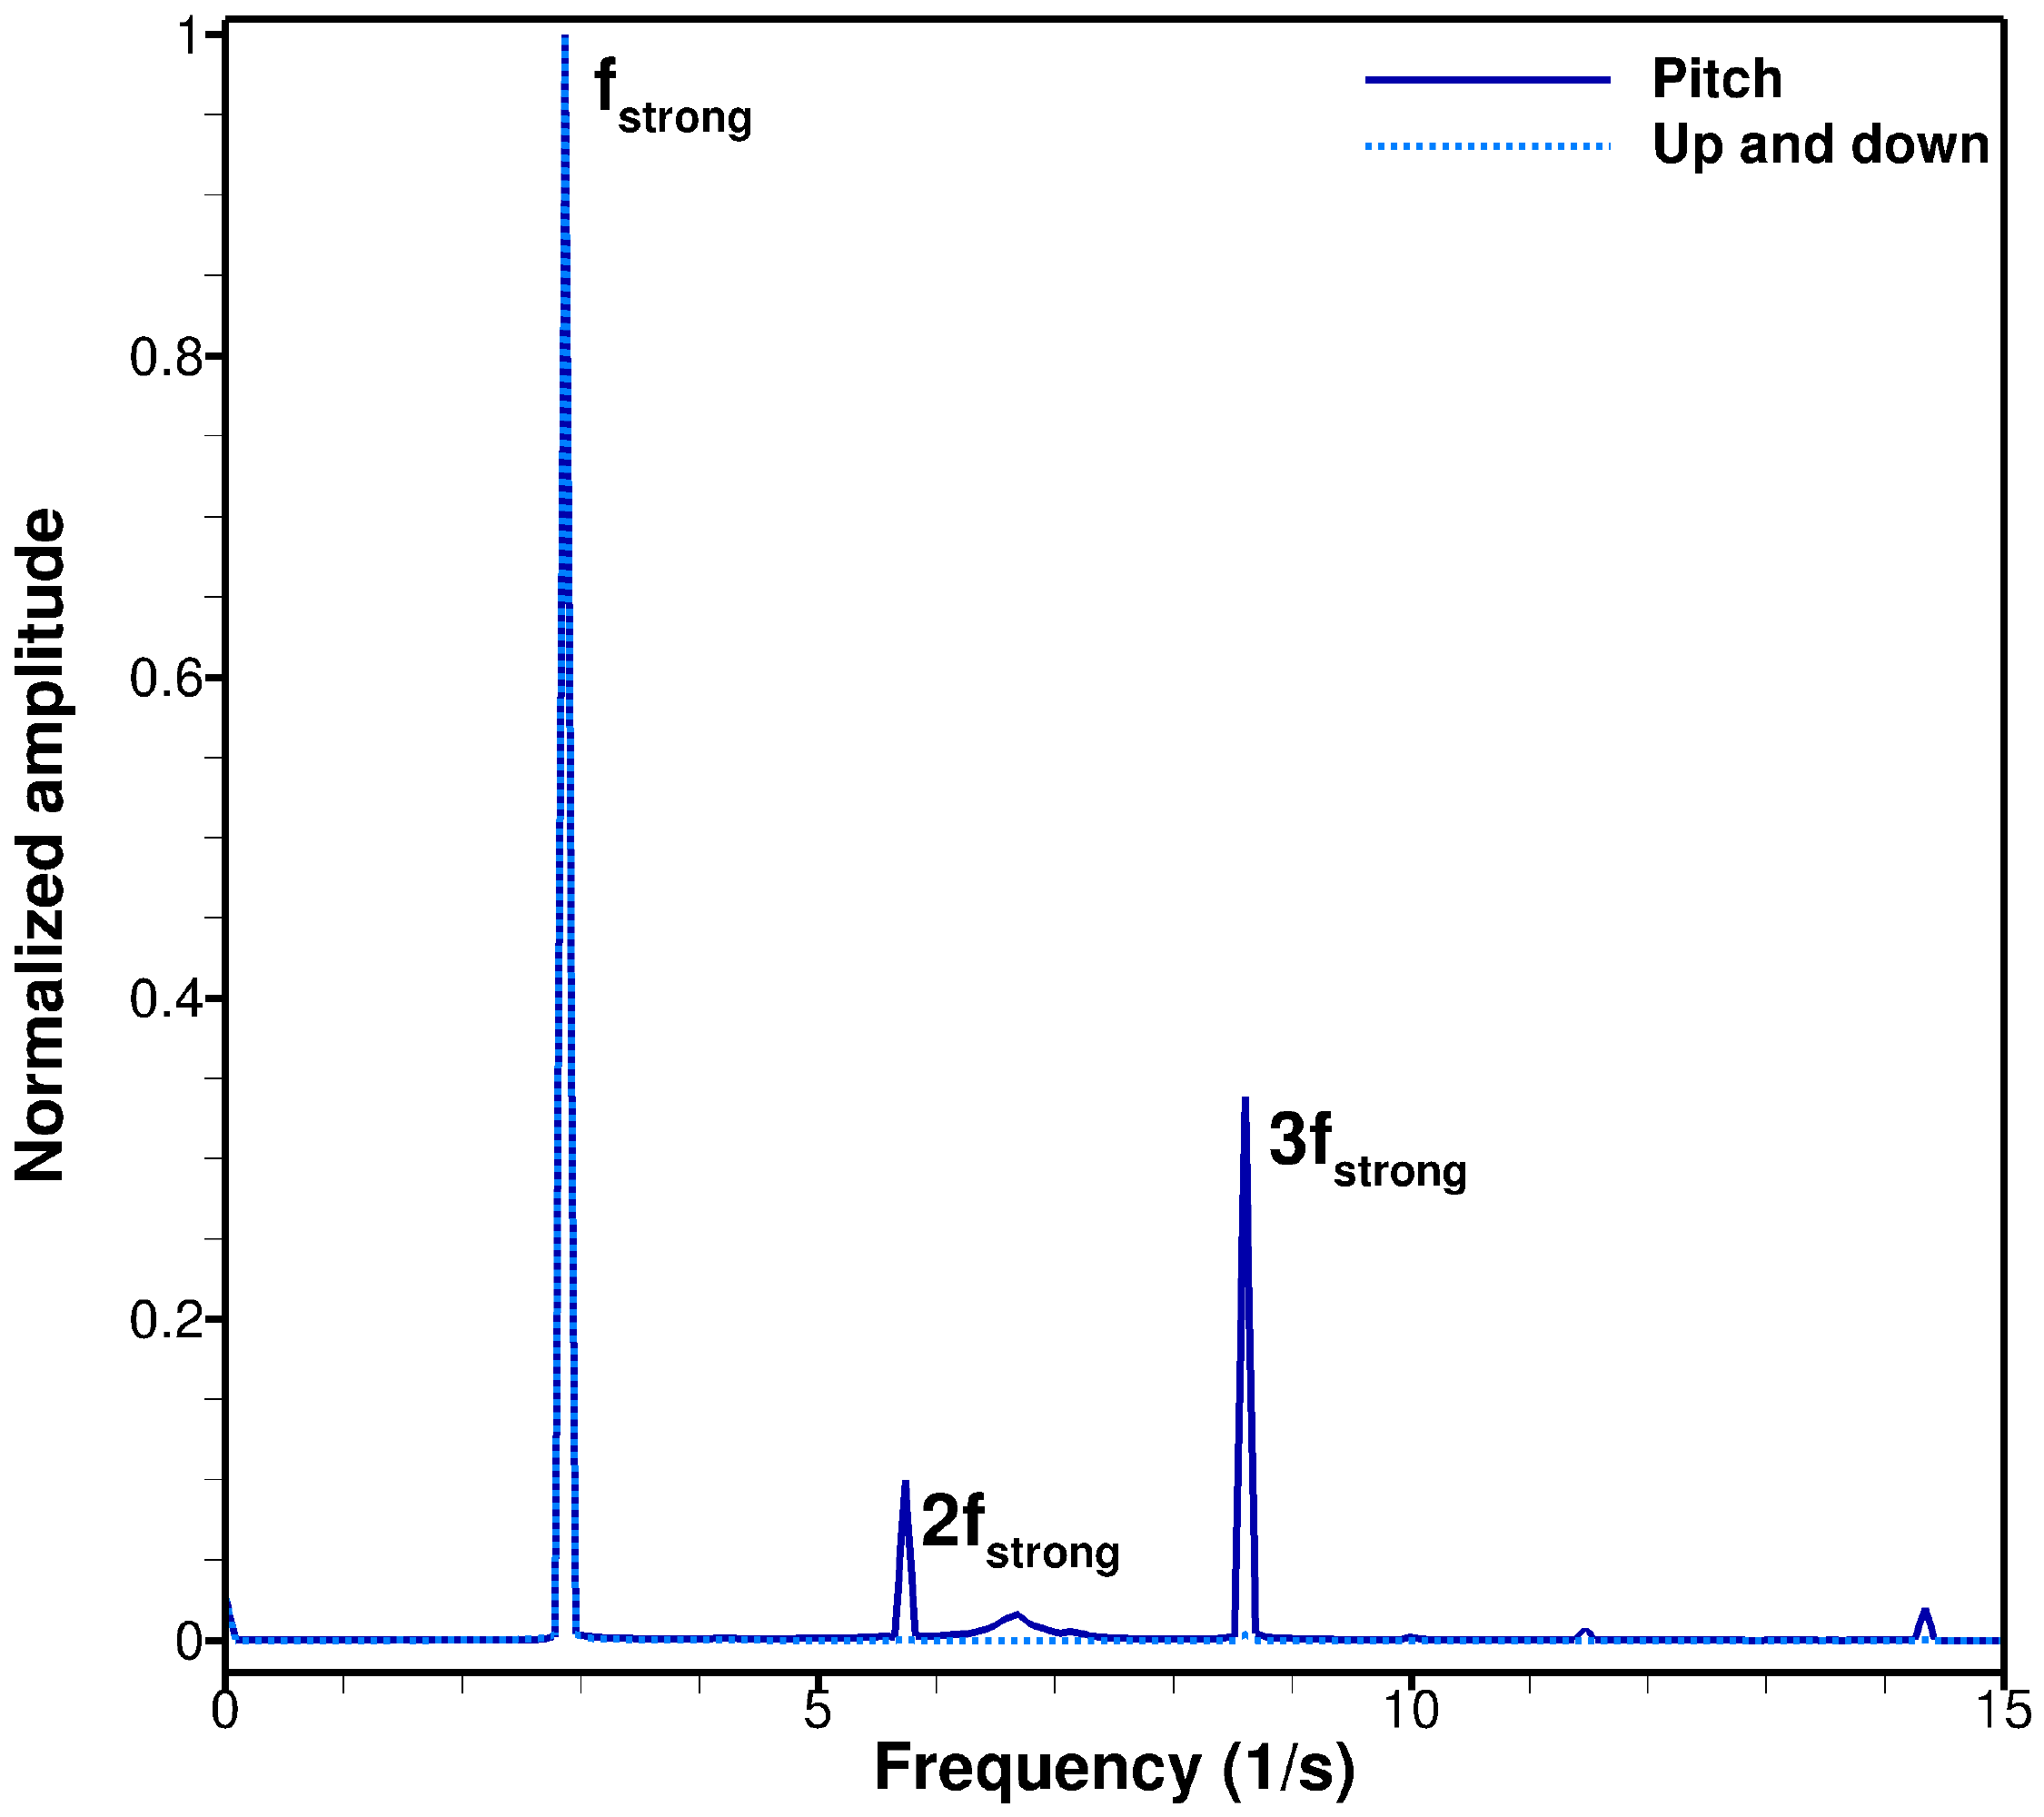}\label{fig:frequencies_strong}}\hfill
	\caption{Frequency domain of the plunge ($X_2$) and pitch ($\varphi_3$) displacements.}
	\label{fig:frequencies_displacements_coupling}
\end{figure}
\begin{table}[H]
	\centering
	\begin{tabular}{p{2cm} p{3cm} p{3cm} p{3cm}}
		\hline
		\centering{\bf{FSI coupling}} & \centering{\bf{Frequency $f_1$ ($\text{Hz}$)}} & \centering{\bf{Frequency $f_2$ ($\text{Hz}$)}} &  \centering{\bf{Frequency $f_3$ ($\text{Hz}$)}} \tabularnewline \hline
		\centering{Strong} & \centering{2.886} & \centering{5.772} & \centering{8.658} \tabularnewline
		\centering{Loose} & \centering{2.859} & \centering{5.719} & \centering{8.580} \tabularnewline		
		\hline	
	\end{tabular}
	\caption{\label{table:frequencies_coupling}Characteristic frequencies: Simulations with different coupling schemes.}
\end{table}
\begin{table}[H]
	\centering
	\begin{tabular}{p{4.2cm} p{5cm}}
		\hline
		\centering{\bf{FSI coupling}} & \centering{\bf{Computational time (d)}} \tabularnewline \hline
		\centering{Loose} &  \centering{23.07} \tabularnewline	
		\centering{Strong for $n\leq100{,}000$} & \multicolumn{1}{c}{\multirow{2}{*}{{$27.05$}}} \tabularnewline	
		\centering{Loose for $n>100{,}000$} & \tabularnewline
		\centering{Strong} & \centering{$41.23$} \tabularnewline
		\hline	
	\end{tabular}
	\caption{\label{table:compt_time_coupling}Computational times: Simulations with different coupling schemes.}
\end{table}
