# Supplementary material for: Numerical investigations of the fluid-structure interaction of a NACA0012 airfoil based on large-eddy simulations
Source: arXiv:1807.01574 source file (2018-07-04)
Supplement: Supplementary file 5 [file appendix_tfi_idw_tfi.tex]

\par In order to analyze the available re-meshing algorithms regarding cases characterized by great airfoil displacements and rotations, firstly a system configuration that causes these structural responses must be established. Since great airfoil displacements occur when the vortex shedding frequency stays between the natural frequencies of the degrees of freedom (see Fung \cite{Fung_2002}), the frequencies generated by the flow of various system configurations are primarily investigated. Afterwards, the natural frequencies of the plunge and pitch degrees of freedom are adjusted through the alteration of the linear and torsional stiffnesses, aiming at the creation of a natural frequency interval which contains the previously investigated flow frequencies. The established configuration is then tested in order to assure that great structural responses in the form of translational and rotational displacements are present. Finally, the greatest achieved airfoil displacements are gradually applied as boundary conditions in a setup that includes solely the NACA0012 without the surrounding fluid, aiming at the analysis of the available re-meshing algorithms.

\section{Analysis of the frequency domain}\markboth{APPENDIX F.$\quad$INV. MSH. ADP.: GREAT ROT. AND DISP.}{F.1$\quad$AN. FREQ. DOMAIN}
\label{sec:flow_frequencies_re_meshing}  

\par A brief analysis of the frequencies generated by the flow is carried out aiming only at the recognition of a rough flow frequency interval and not the thorough investigation of its physical meaning. Thereto, a variety of system configurations are analyzed, considering only the stiffnesses of the physically available springs (see \mbox{Appendix \ref{appendix_experimental_setup})}. While the torsional stiffness \mbox{$k_{t\,3,\,eq}=0.3832\,N{\cdot}m{\cdot}rad^{-1}$} is maintained constant for all simulations, the investigated linear stiffnesses are:
\begin{eqnarray}
\nonumber
k_{l\,2,\,eq}=40\,N{\cdot}m^{-1},\quad\;\, k_{l\,2,\,eq}=50\,N{\cdot}m^{-1},\quad\;\, k_{l\,2,\,eq}=60\,N{\cdot}m^{-1},\;\;\\\nonumber k_{l\,2,\,eq}=70\,N{\cdot}m^{-1},\quad\;\,
k_{l\,2,\,eq}=80\,N{\cdot}m^{-1},\quad\;\, k_{l\,2,\,eq}=92\,N{\cdot}m^{-1},\;\;\\\nonumber k_{l\,2,\,eq}=104\,N{\cdot}m^{-1},\quad k_{l\,2,\,eq}=114\,N{\cdot}m^{-1},\quad
k_{l\,2,\,eq}=124\,N{\cdot}m^{-1},\\ k_{l\,2,\,eq}=134\,N{\cdot}m^{-1},\quad
k_{l\,2,\,eq}=144\,N{\cdot}m^{-1}.\quad\quad\quad\quad\quad\quad\quad\quad\quad\quad
\label{eq:analyzed_stiffnesses}
\end{eqnarray}
\par These coupled simulations are carried for the $m{-}L_3^{min}{-}y_{max}^+$ mesh applying an explicit coupling algorithm at a chord Reynolds number of $Re=30{,}000$. The applied time step size is $\Delta t=1{\cdot}10^{-5}\,s$ and the simulations run until a dimensionless time step of $t^*=1564$ is achieved. The transfinite interpolation re-meshing method is applied due to the low required computational time. Later on, TFI proves to be the best algorithm, since only small translational and rotational displacements are available, i$.$e$.$, \mbox{$|X_2^{max}|=1.86{\cdot}10^{-4}\,m$} and \mbox{$|\varphi_3^{max}|=0.34^\circ$}. This structural response of the airfoil is shown in Fig.\ \ref{fig:disp_kl_124} for the case with a linear stiffness of \mbox{$k_{l\,2,\,eq}=124\,N{\cdot}m^{-1}$}. Although the flow is computed until $t=35\,s$, only the time range $0\,s\leq t\leq17\,s$ is illustrated since a limit-cycle oscillation (LCO) starts at $t\approx13\,s$. All other simulated cases also develop a LCO after different initialization times. However, these are not illustrated in the current work for the sake of brevity.
\begin{figure}[H]
	\centering
	\subfigure[Translational displacements in the $x_2$-direction.]{\includegraphics[width=0.495\textwidth]{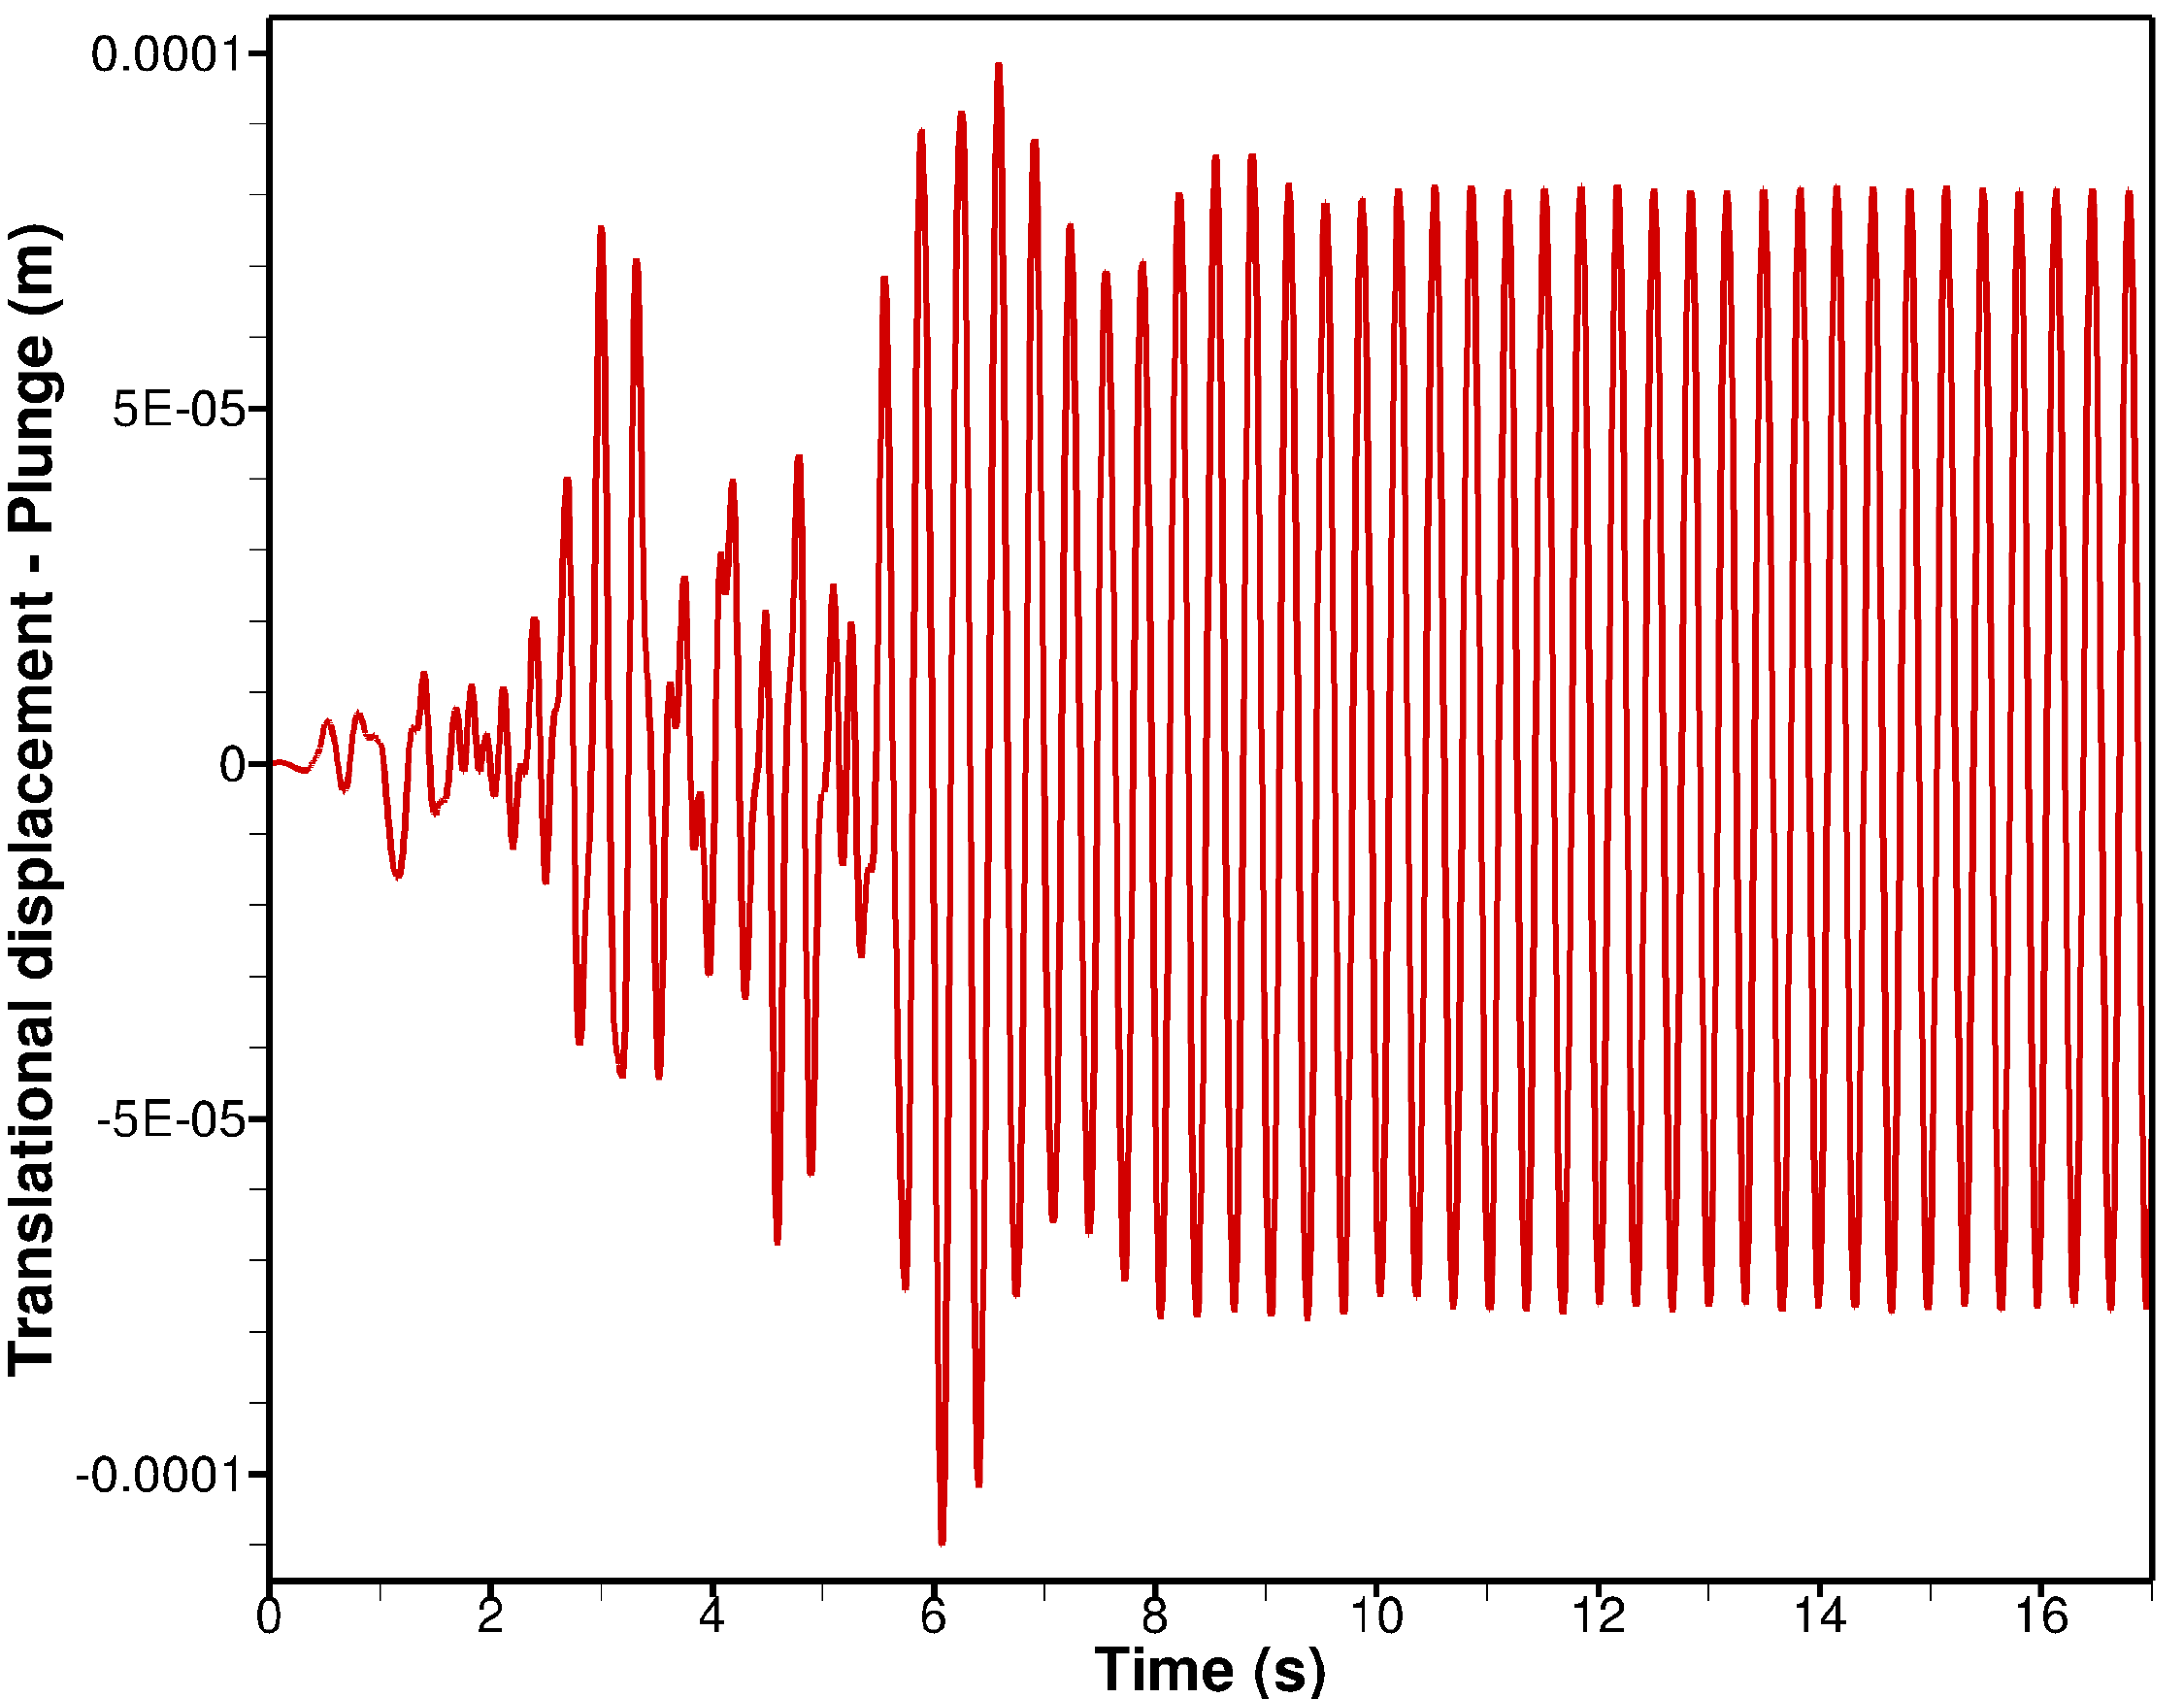} \label{fig:trans_disp_kl_124}}\hfill
	\subfigure[Rotational displacement about the $x_3$-axis.]{\includegraphics[width=0.495\textwidth]{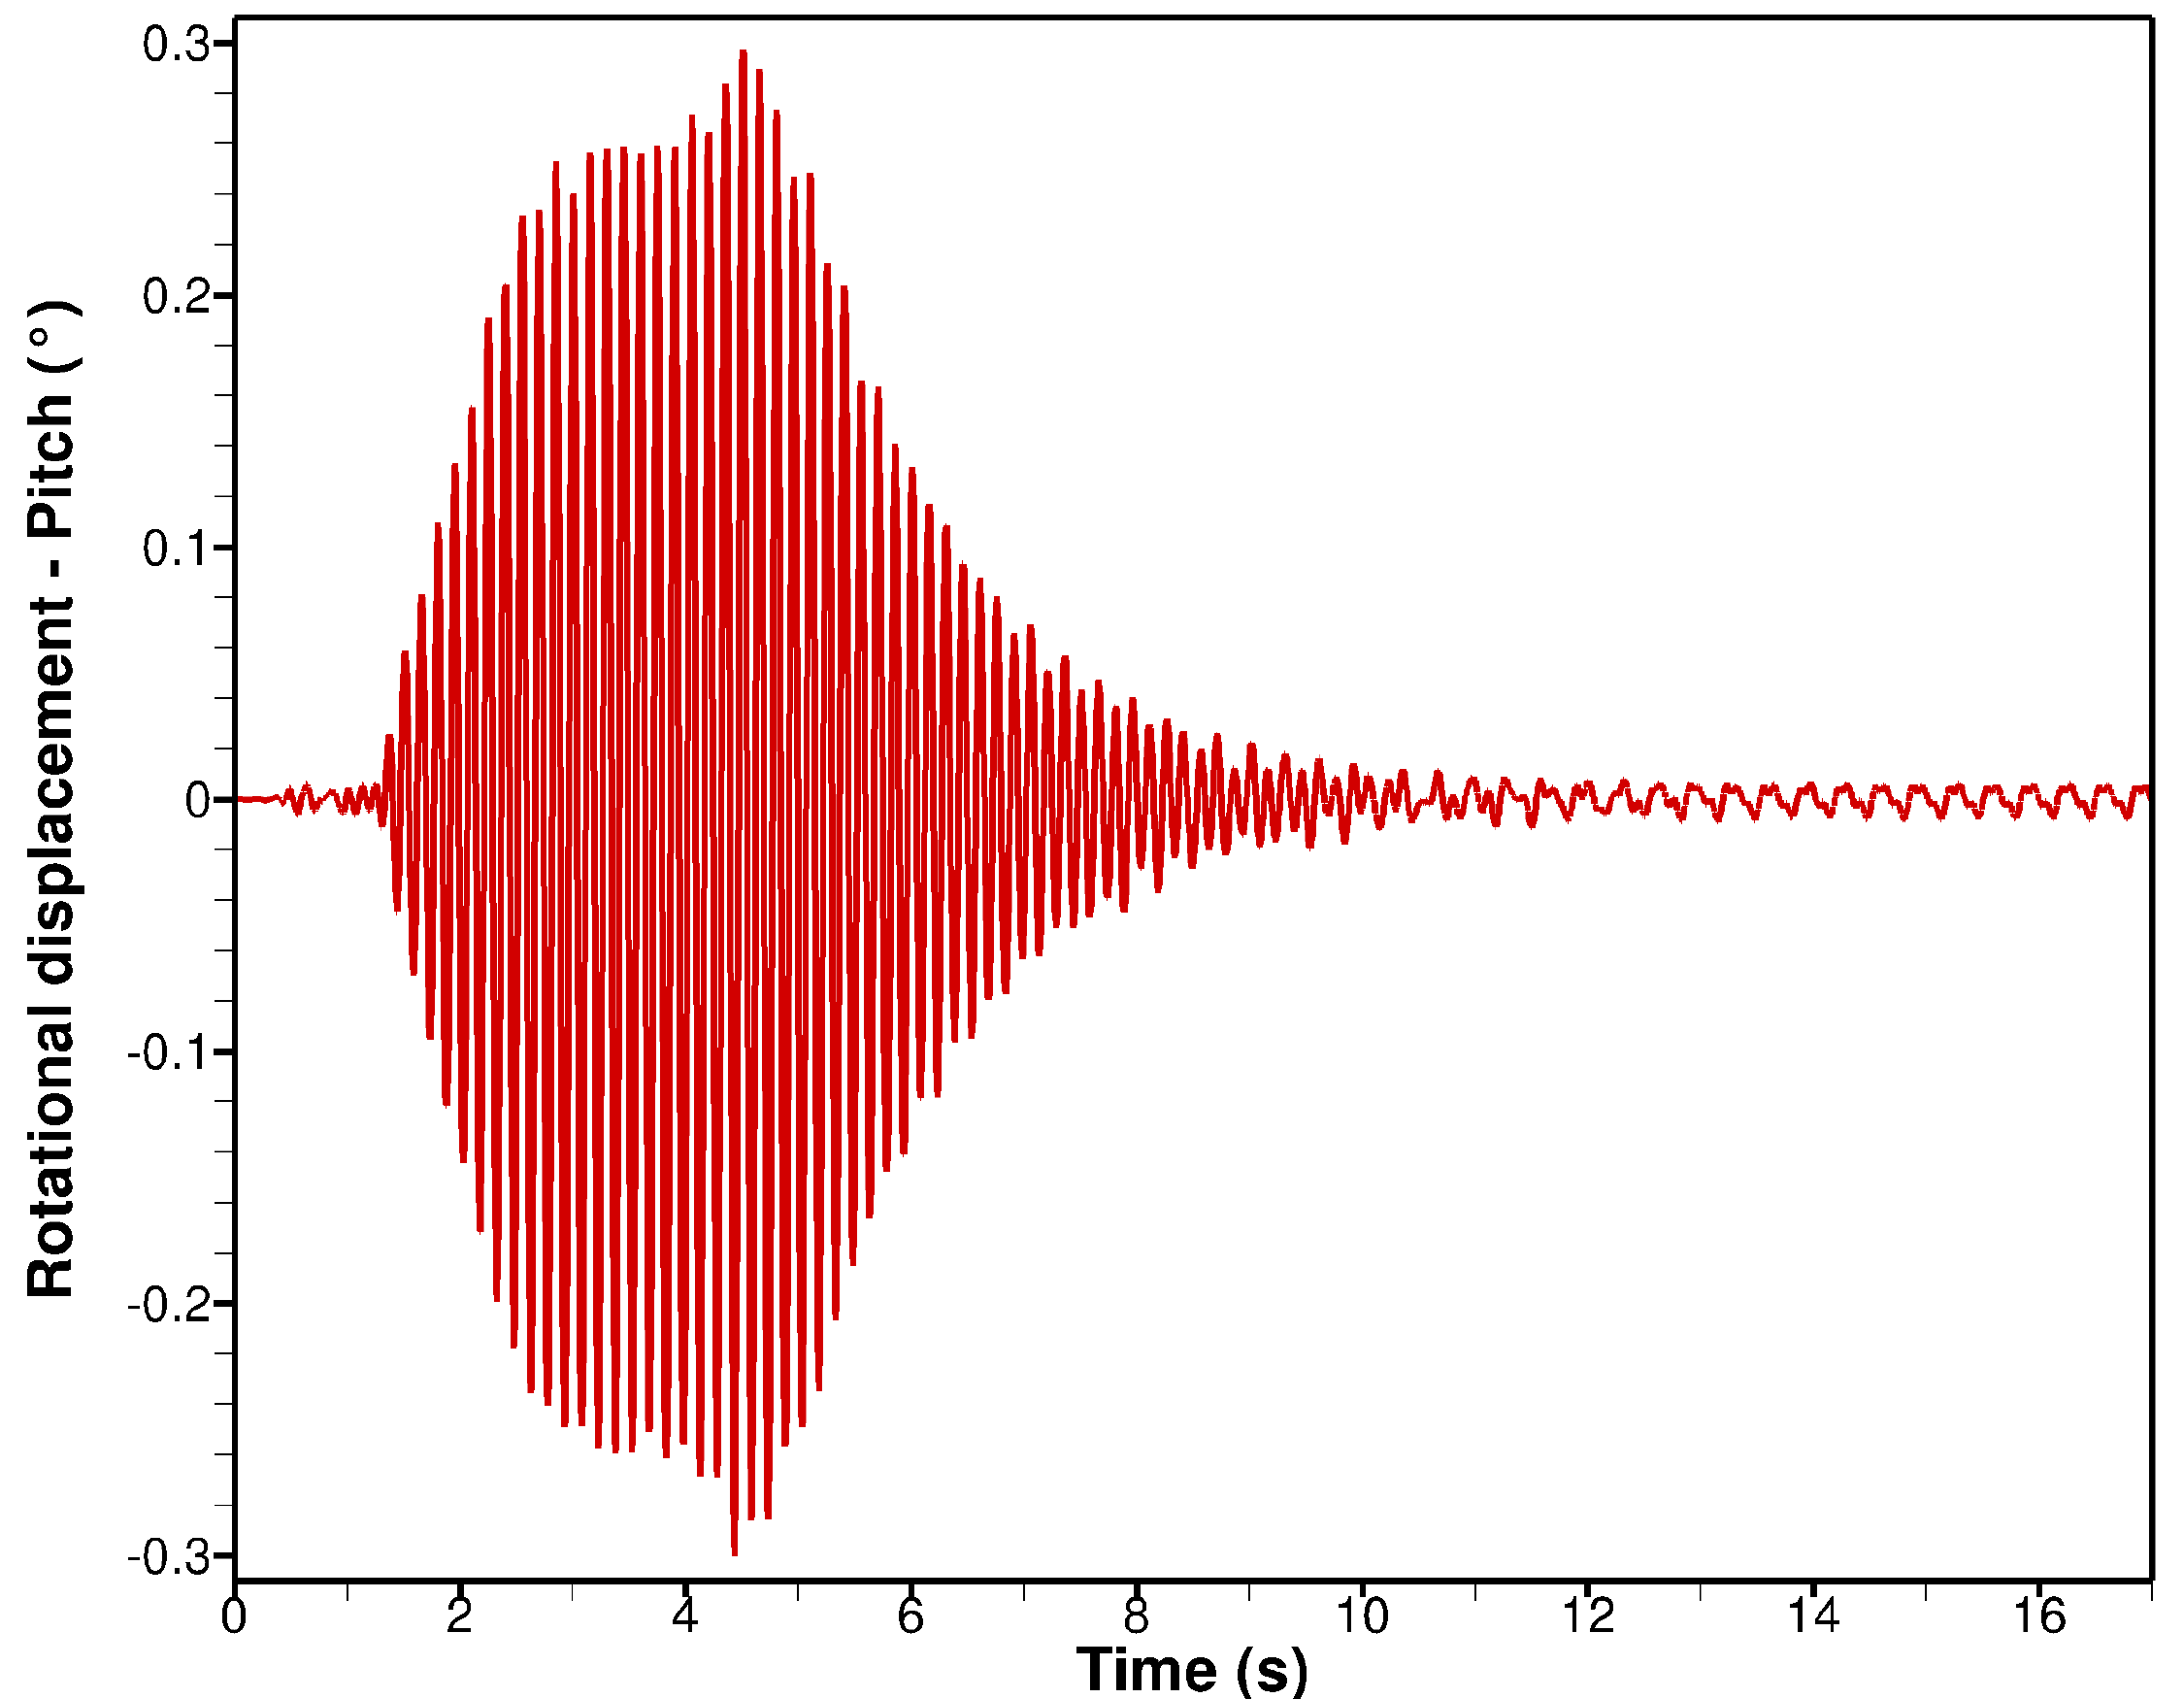}\label{fig:rot_disp_kl_124}}\hfill
	\caption{Airfoil displacements of the system characterized by the linear and torsional stiffnesses $k_{l\,2,\,eq}=124\,N{\cdot}m^{-1}$ and \mbox{$k_{t\,3,\,eq}=0.3832\,N{\cdot}m{\cdot}rad^{-1}$}, respectively.}
	\label{fig:disp_kl_124}
\end{figure}
\par The frequencies generated by the translational displacement of the airfoil are acquired through the application of a Fourier transform with a Hamming window. This utilizes the time $t$ as the independent variable and the translational displacement $X_2$ as the dependent variable. The achieved frequencies are then illustrated in Fig.\ \ref{fig:frequencies_all_kl} for the test cases with \mbox{$k_{l\,2,\,eq}=50\,N{\cdot}m^{-1}$}, \mbox{$k_{l\,2,\,eq}=60\,N{\cdot}m^{-1}$}, \mbox{$k_{l\,2,\,eq}=92\,N{\cdot}m^{-1}$}, \mbox{$k_{l\,2,\,eq}=104\,N{\cdot}m^{-1}$}, \mbox{$k_{l\,2,\,eq}=124\,N{\cdot}m^{-1}$} and \mbox{$k_{l\,2,\,eq}=144\,N{\cdot}m^{-1}$}, regarding that the amplitudes are normalized in relation to the maximal amplitude achieved by each case. The frequency domain of the simulations characterized by the linear stiffnesses \mbox{$k_{l\,2,\,eq}=40\,N{\cdot}m^{-1}$}, \mbox{$k_{l\,2,\,eq}=70\,N{\cdot}m^{-1}$}, \mbox{$k_{l\,2,\,eq}=80\,N{\cdot}m^{-1}$}, \mbox{$k_{l\,2,\,eq}=114\,N{\cdot}m^{-1}$} and \mbox{$k_{l\,2,\,eq}=134\,N{\cdot}m^{-1}$} are not illustrated in the present work since these require longer initialization times in order to reach a fully developed state and therefore only unclear frequency peaks are available.
\par The frequency spectrum of all test cases are characterized by the formation of a distinct peak located at the frequency interval of \mbox{$2.86\leq f_{X_{2}}\leq 3.03$}, which may be related to the vortex shedding frequency. Therefore, the spring parameters are afterwards adapted in order to provide an interval of the natural frequencies, in which these frequencies are contained. This aims at the achievement of a test case characterized by great airfoil displacements.
\begin{figure}[H]
	\centering
	\subfigure[$k_{l\,2,\,eq}={\left[104,124,144\right]}\,N{\cdot}m^{-1}$.]{\includegraphics[width=0.49\textwidth]{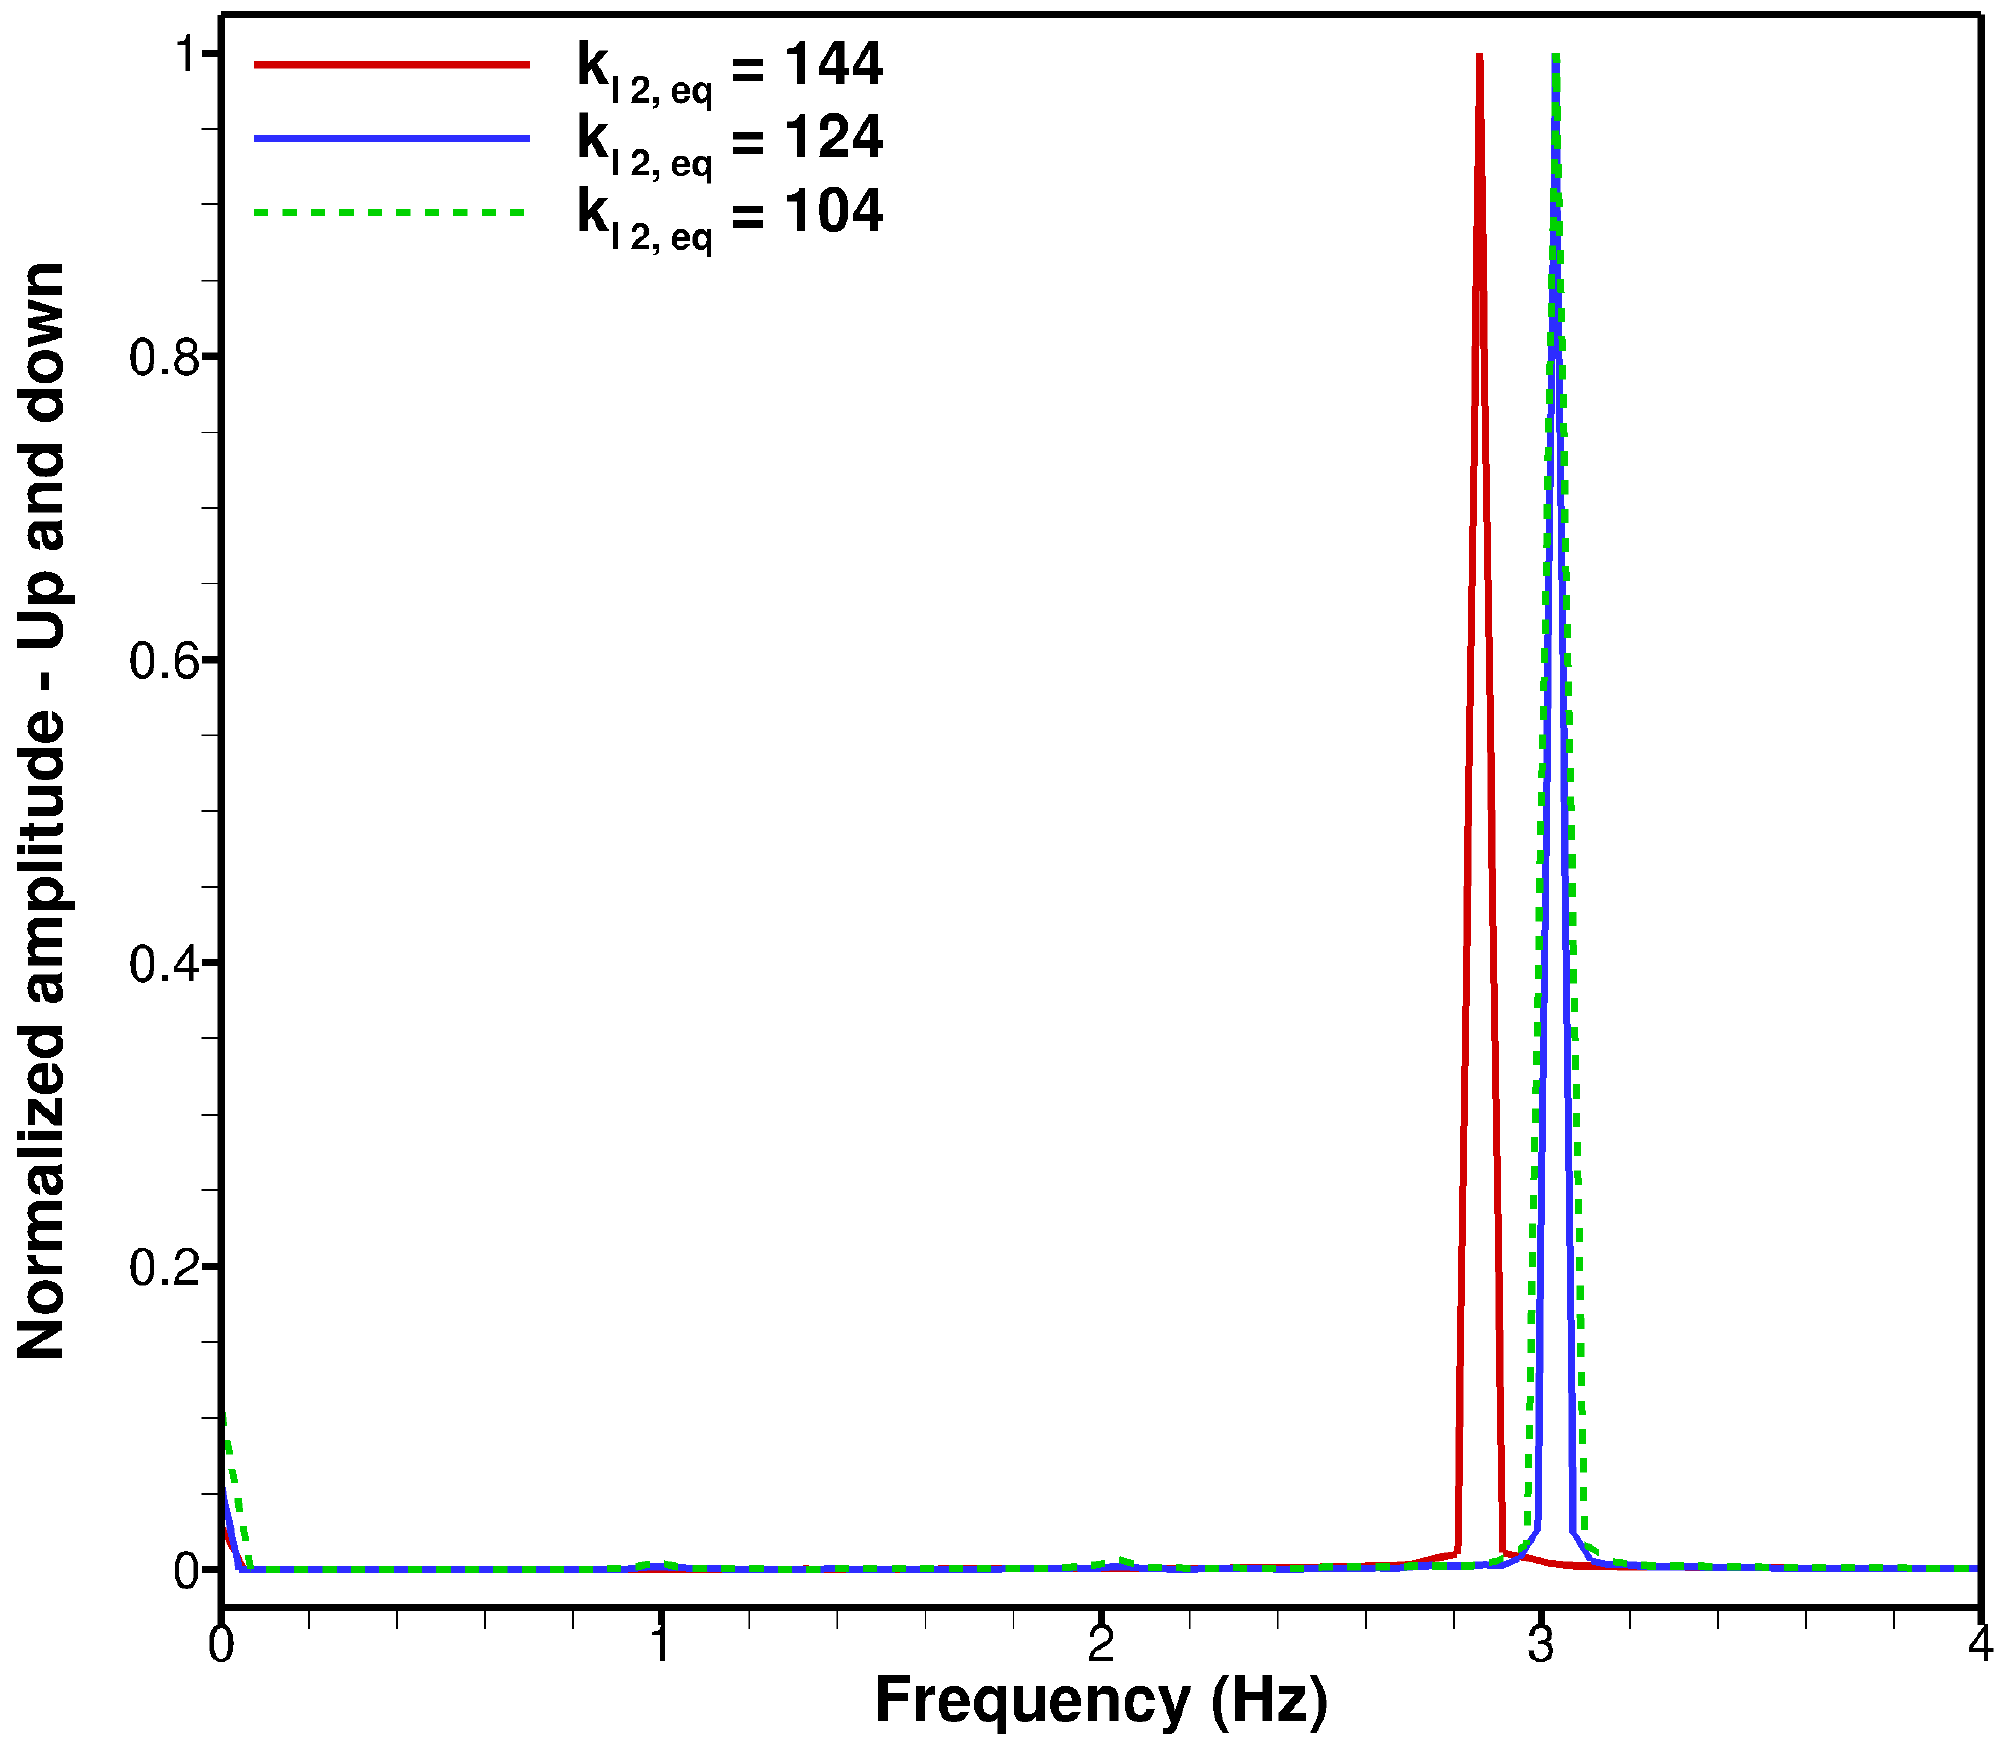} \label{fig:frequencies_high_high_kl}}\hfill
	\subfigure[$k_{l\,2,\,eq}={\left[50,60,92\right]}\,N{\cdot}m^{-1}$.]{\includegraphics[width=0.49\textwidth]{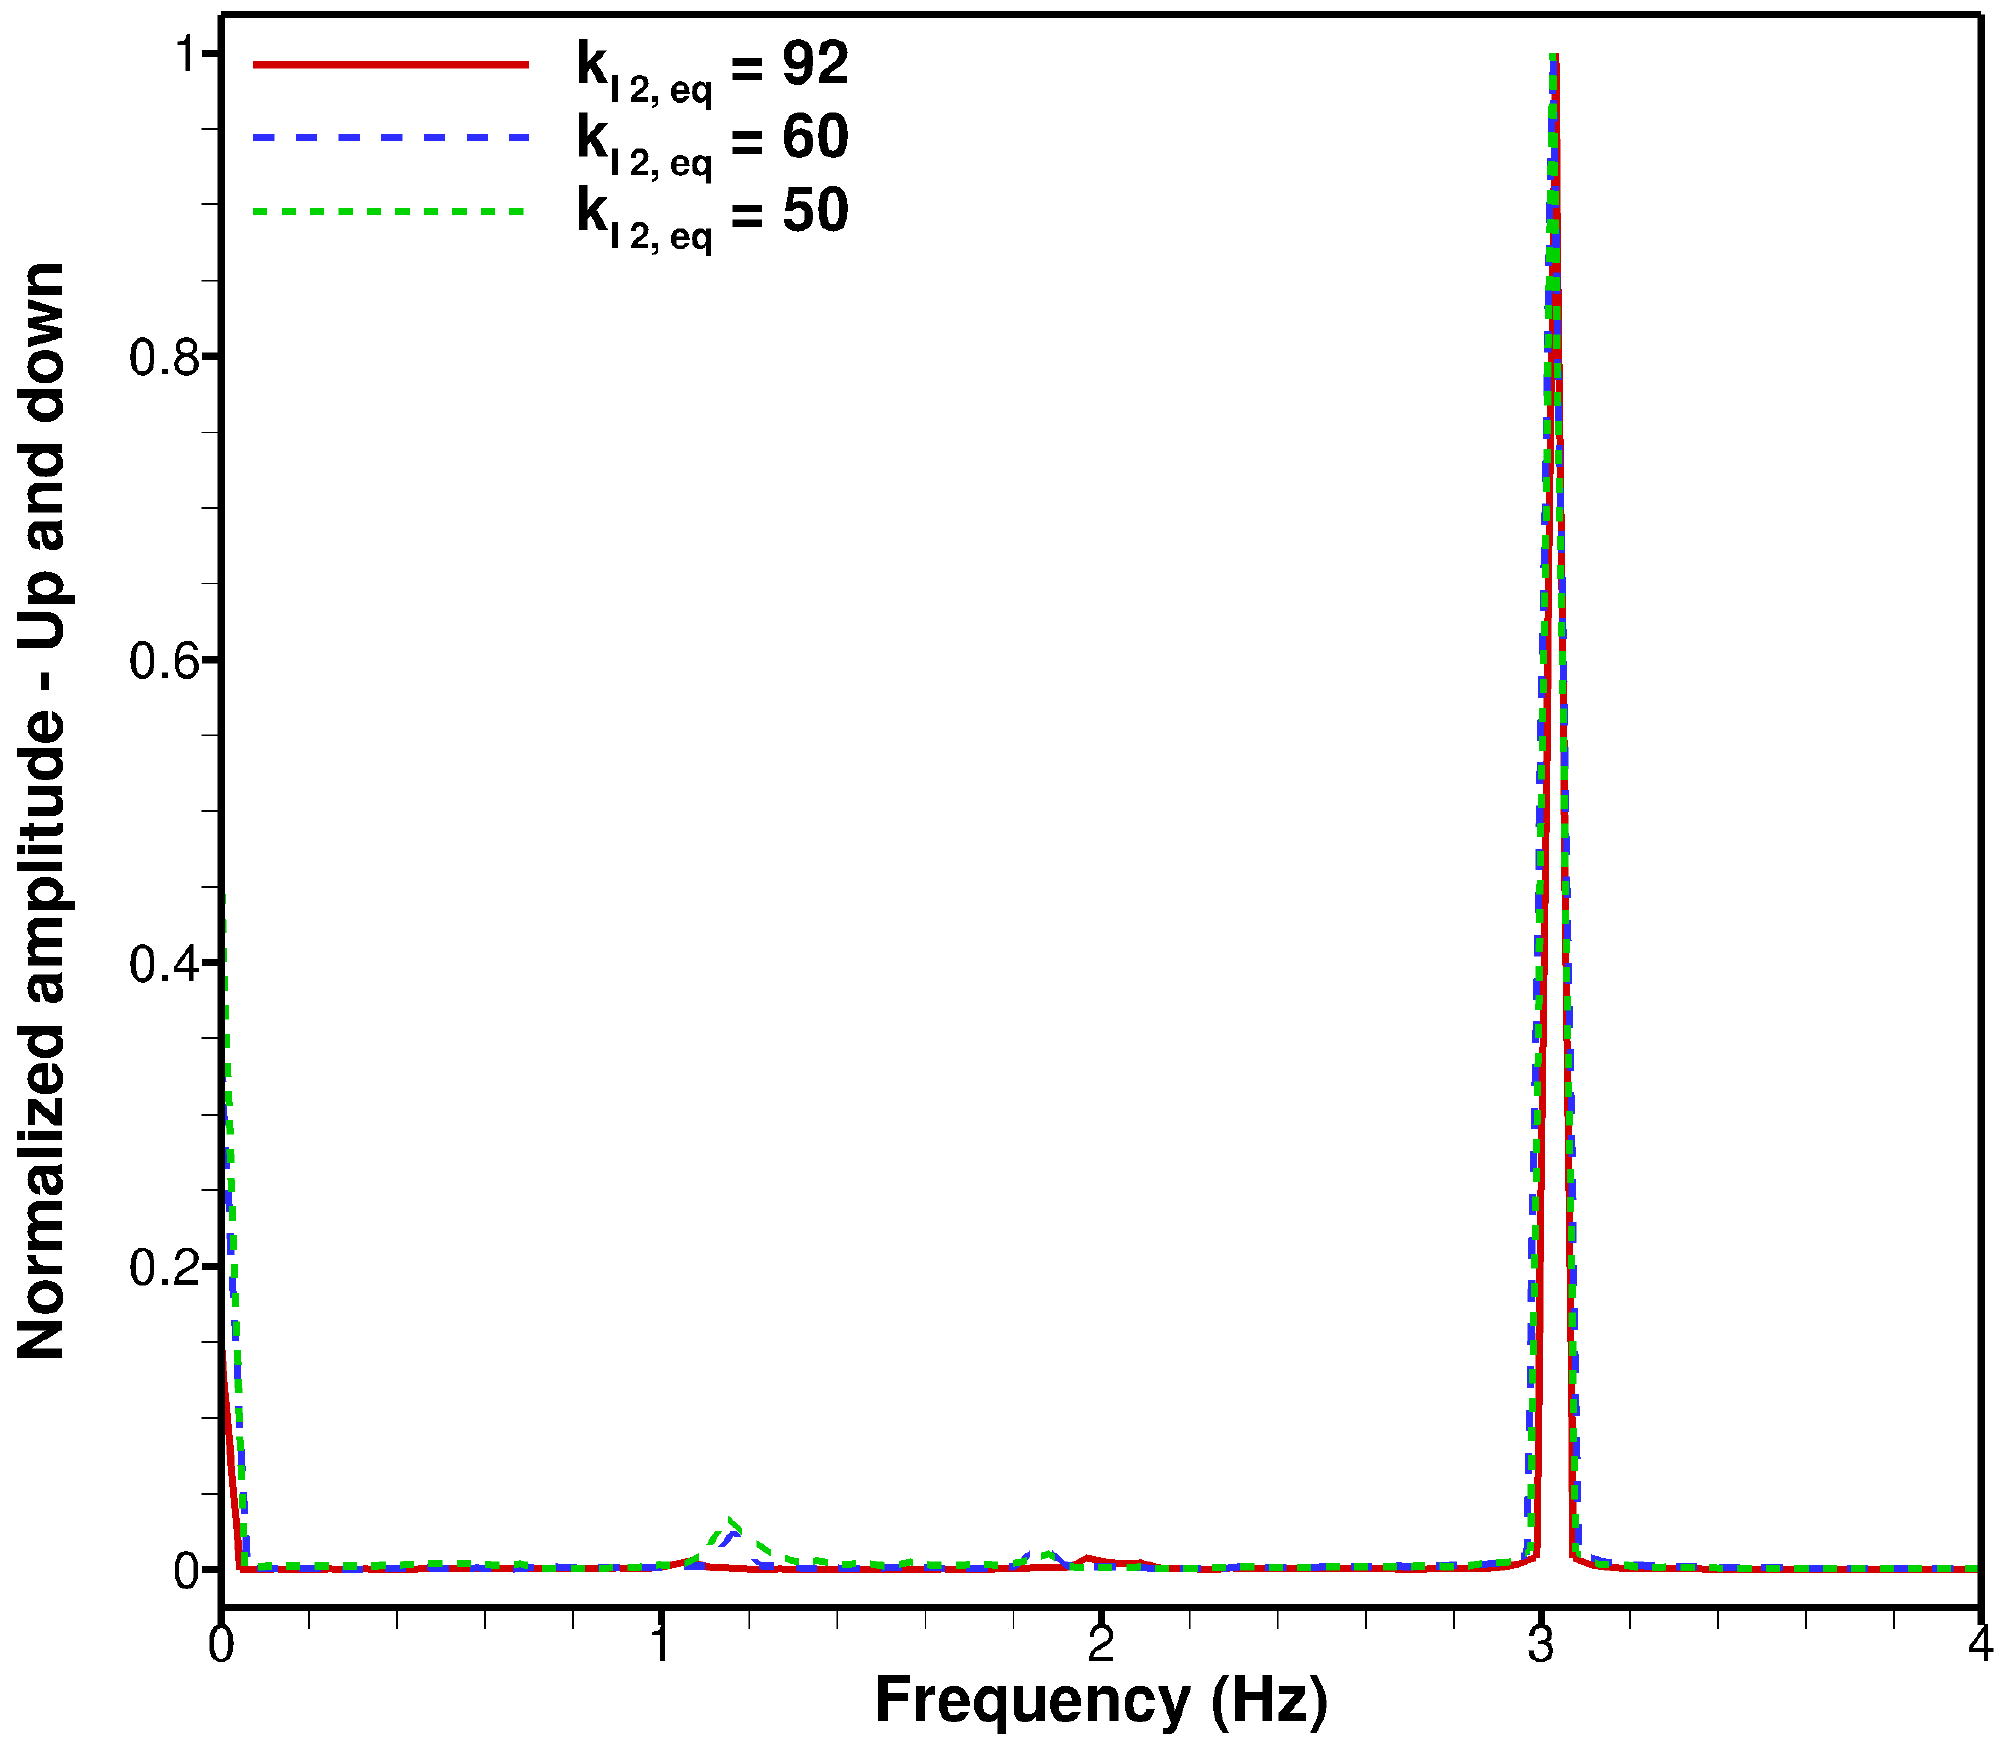}\label{fig:oifrsequencies_high_kl}}\hfill
	\caption{Frequency domain of the translational displacement for various system configurations: constant torsional stiffness of \mbox{$k_{t\,3,\,eq}=0.3832\,N{\cdot}m{\cdot}rad^{-1}$} and varying linear stiffnesses.}
	\label{fig:frequencies_all_kl}
\end{figure}

\markboth{APPENDIX F.$\quad$INV. MSH. ADP.}{F.2$\quad$TEST CASE: GREAT AIR. DISP.}
\section{Test case: Great airfoil displacements}\markboth{APPENDIX F.$\quad$INV. MSH. ADP.}{F.2$\quad$TEST CASE: GREAT AIR. DISP.}
\label{sec:case_great_airfoil_disp}

\par The linear and torsional stiffnesses of the system are adapted and set to respectively \mbox{$k_{l\,2,\,eq}={3}\,N{\cdot}m^{-1}$} and \mbox{$k_{t\,3,\,eq}=0.005\,N{\cdot}m{\cdot}rad^{-1}$}. This airfoil configuration ensures that the flow frequencies with the highest generated amplitudes (see \mbox{Appendix \ref{sec:flow_frequencies_re_meshing})} are contained within the interval created by the the natural frequencies of the pitch and plunge degrees of freedom, as stated in \mbox{Table \ref{table:frequencies_natural_flow}:} 
\begin{table}[H]
	\centering
	\begin{tabular}{p{4cm} p{5cm} p{5cm}}
		\hline
		\multirow{2}{4cm}{\centering{\bf{Flow frequencies interval ($1{\cdot}s^{-1}$)}}} &  \multicolumn{2}{c}{\bf{Natural frequencies ($1{\cdot}s^{-1}$)}} \tabularnewline \cline{2-3}
		& \centering{\bf{$X_2$ DOF}} & \centering{\bf{$\varphi_3$ DOF}} \tabularnewline\hline
		\multicolumn{1}{c}{\multirow{2}{*}{\centering{$2.86\leq f_{X_{2}}\leq 3.03$}}} & \multicolumn{1}{c}{\multirow{2}{*}{\centering{$\omega_{n,\,X_{2}}=\sqrt{\frac{k_{l\,2,\,eq}}{m_{tot}}}=2.6346$}}} & \multicolumn{1}{c}{\multirow{2}{*}{\centering{$\omega_{n,\,\varphi_{3}}=\sqrt{\frac{k_{t\,3,\,eq}}{J_{tot,\,33}^{CM}}}=5.0357$}}} \tabularnewline
		& &  \tabularnewline
		\hline	
	\end{tabular}
	\caption{\label{table:frequencies_natural_flow}Flow and natural frequencies.}
\end{table}
\par The simulation is performed for a Reynolds number of $Re=30{,}000$ with a time step size of $\Delta t=1{\cdot}10{-5}\,s$ and utilizing a loose coupling algorithm, as well as the TFI re-meshing method. The latter is utilized in order to achieve a reasonable computational time and enables only a rough analysis of the order of magnitude of the structural response, as illustrated in Fig.\ \ref{fig:disp_flutter_tfi}:
\begin{figure}[H]
	\centering
	\subfigure[Translational displacements in the $x_2$-direction.]{\includegraphics[width=0.48\textwidth]{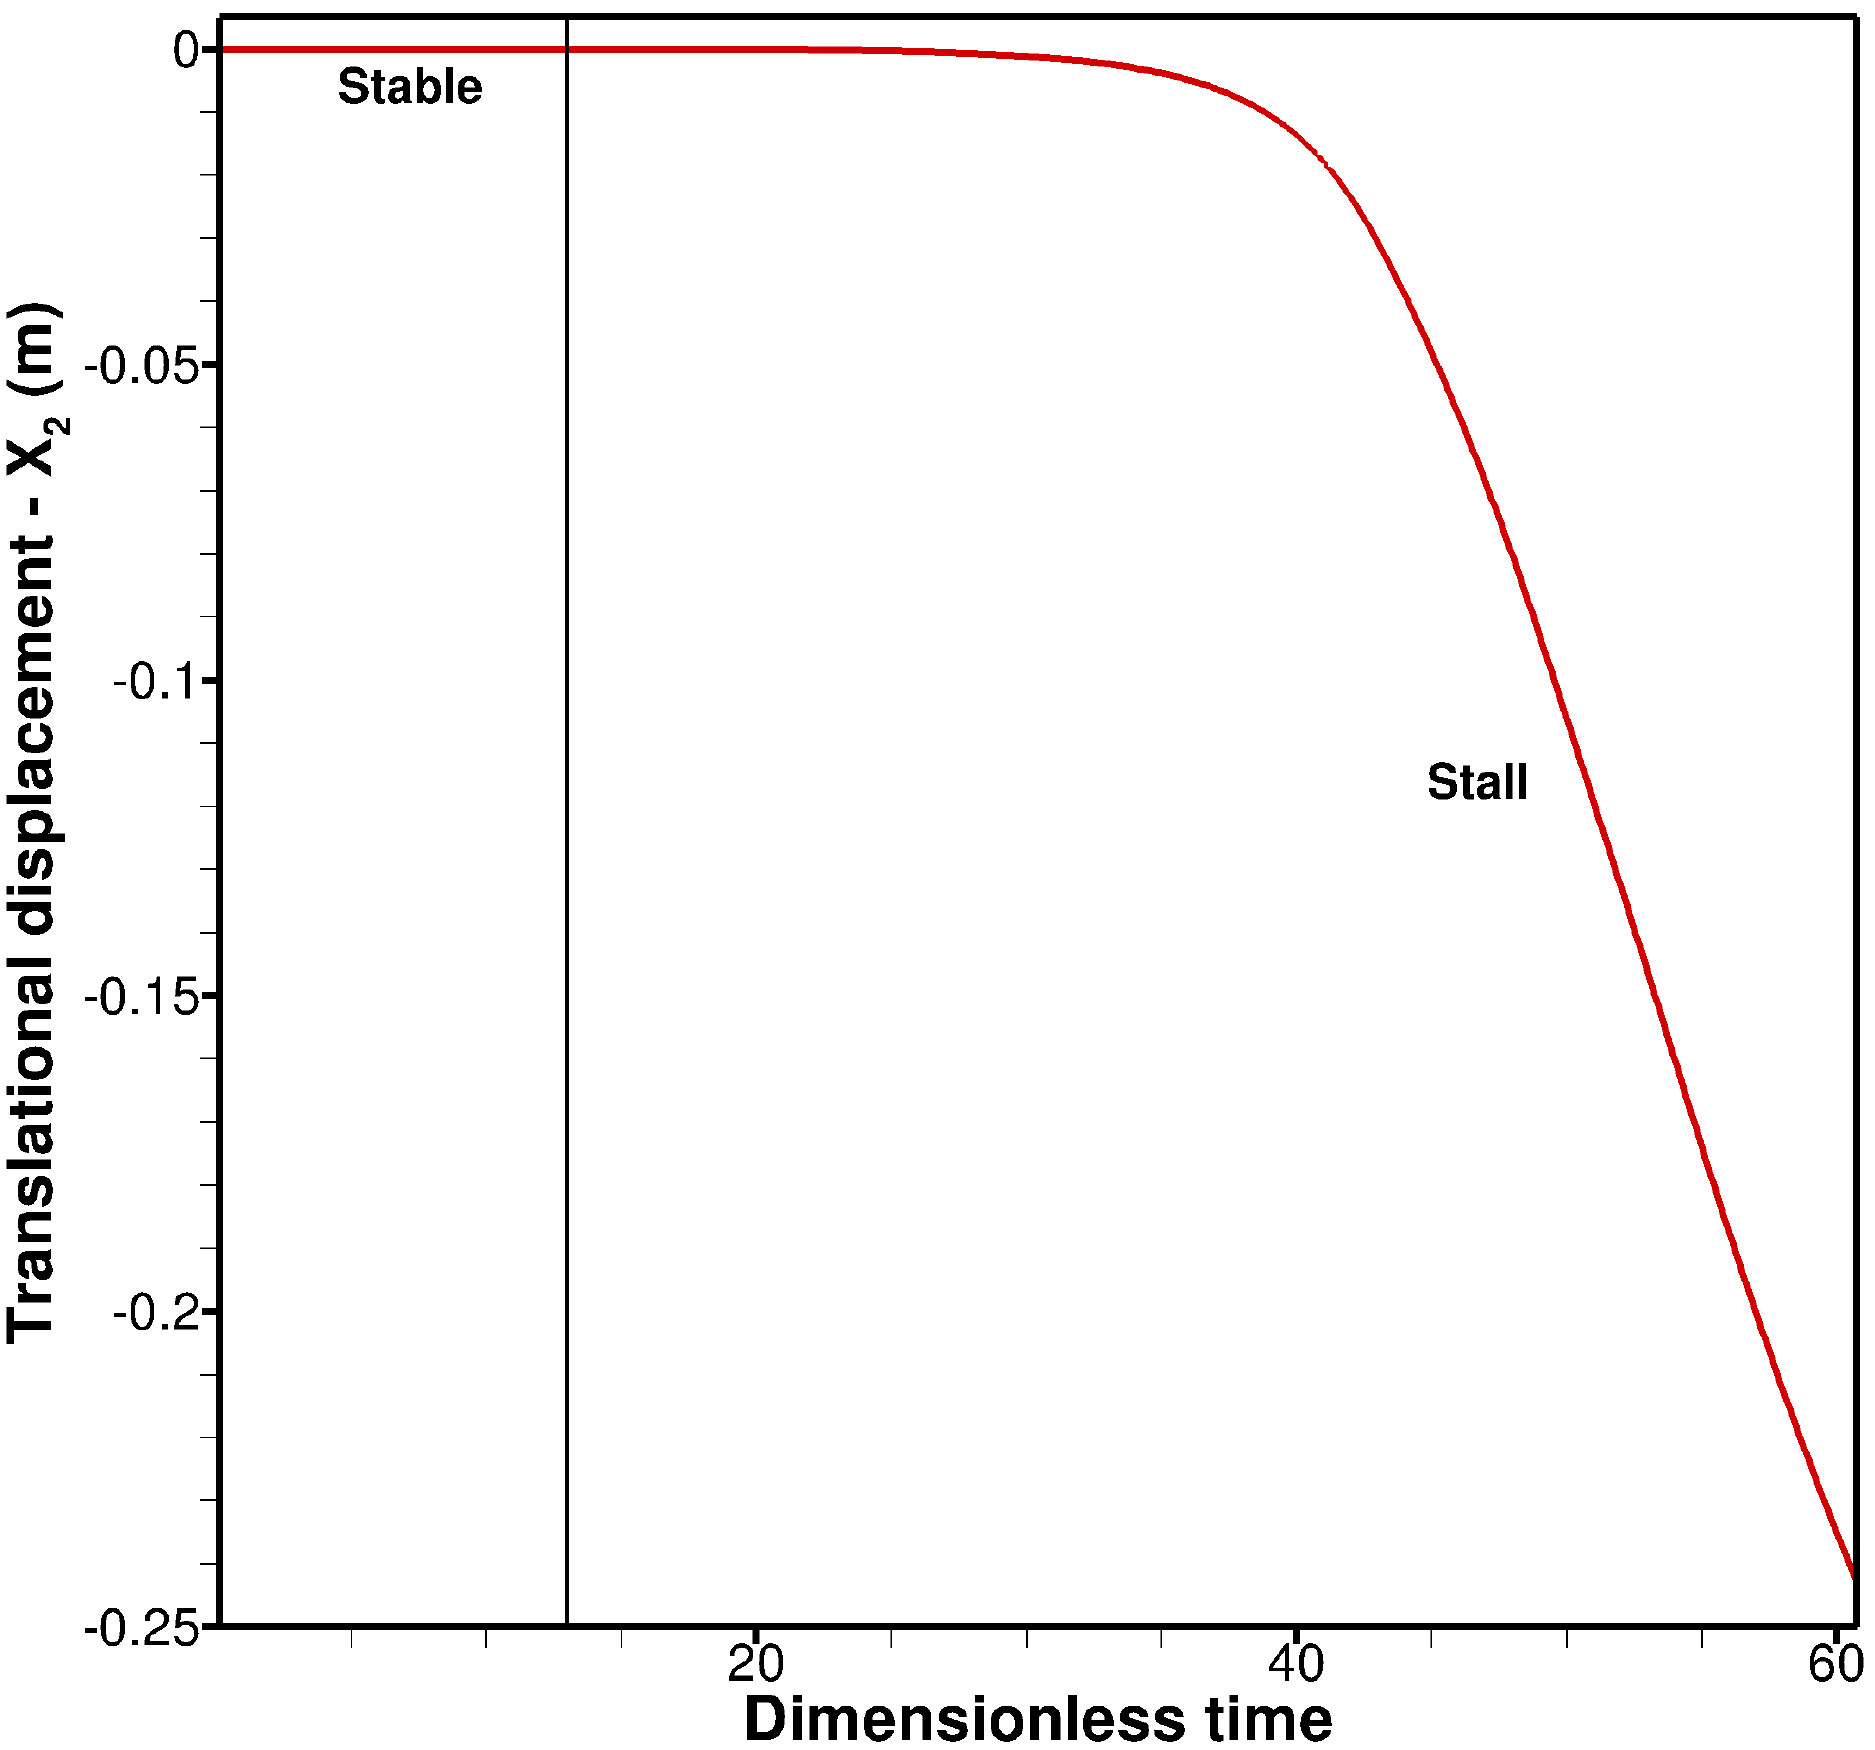} \label{fig:trans_disp_flutter_tfi}}\hfill
	\subfigure[Rotational displacements about the $x_3$-axis.]{\includegraphics[width=0.48\textwidth]{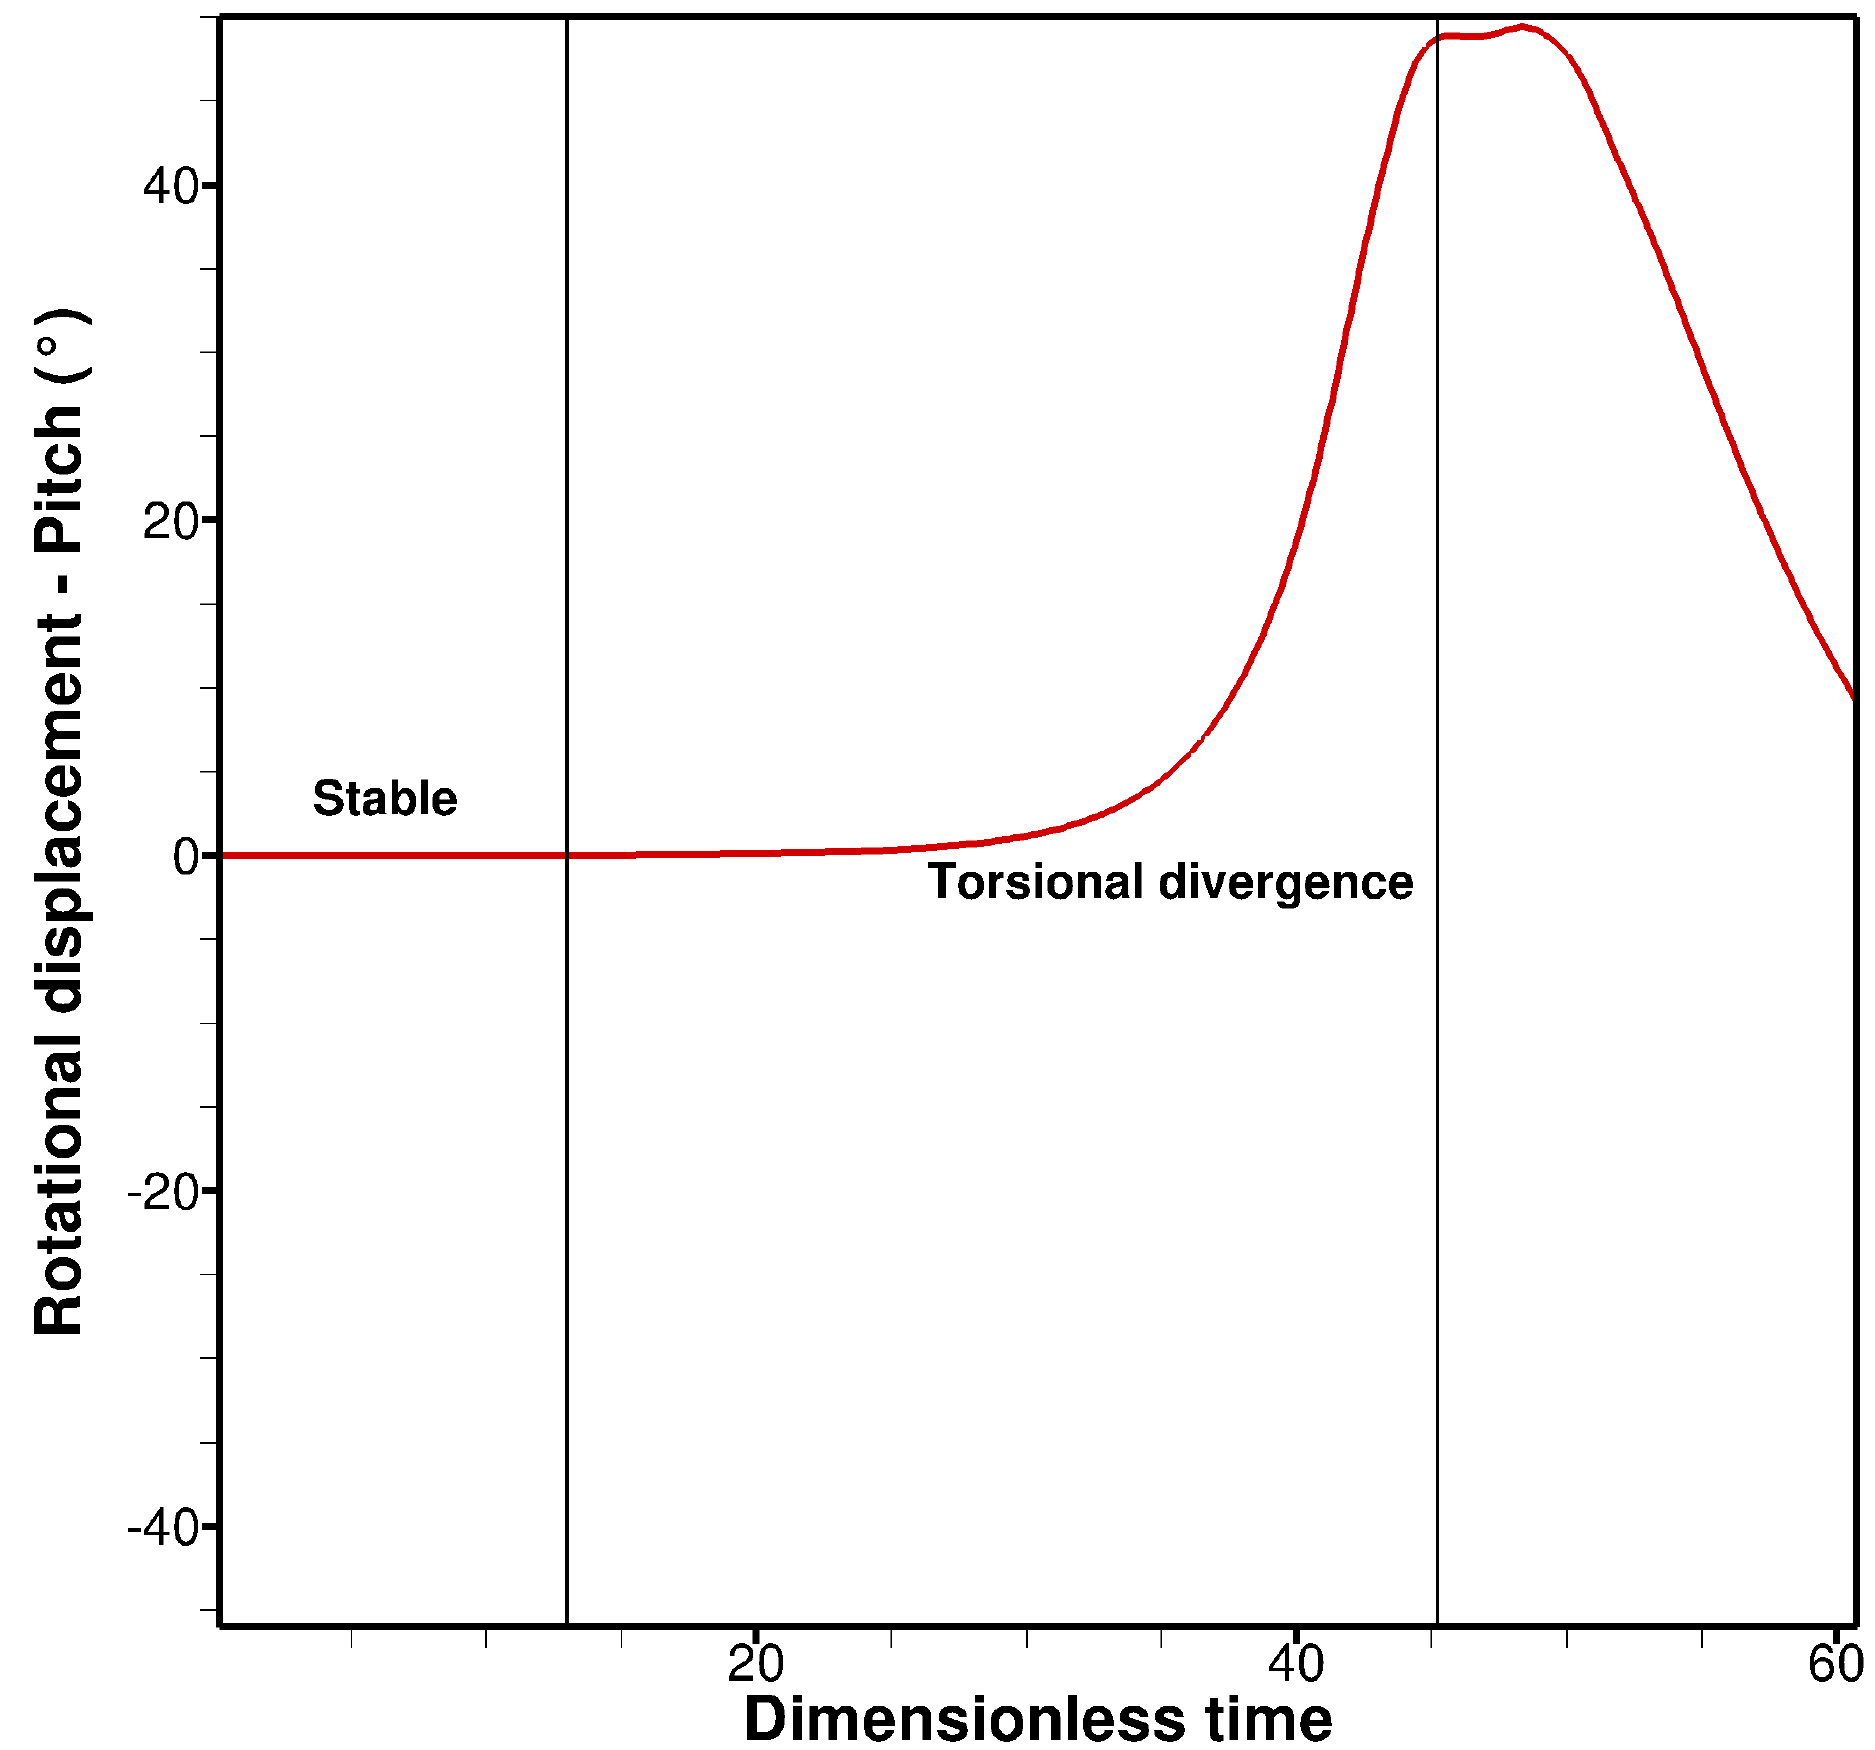}\label{fig:rot_disp_flutter_tfi}}\hfill
	\caption{Airfoil response to the flow: system characterized by linear and torsional stiffnesses of respectively \mbox{$k_{l\,2,\,eq}={3}\,N{\cdot}m^{-1}$} and \mbox{$k_{t\,3,\,eq}=0.005\,N{\cdot}m{\cdot}rad^{-1}$}.}
	\label{fig:disp_flutter_tfi}
\end{figure}  
\par The achieved results present maximal translational and rotational displacements of respectively $|X_2|=0.2875\,m$ and $\varphi_3=49.42^\circ$, regarding that the simulation diverges after the computation of $n=160{,}000$ time steps. The mesh quality is then investigated at this time step, in order to thoroughly evaluate the divergence cause. Figure \ref{fig:mesh_flutter_tfi} illustrates the adapted mesh, regarding that Fig.\ \ref{fig:mesh_overall_flutter_tfi} displays only one out of two mesh lines in the $\xi$ and $\eta$ axes for the front domain, and one out of two mesh lines in the $\xi$-axis for the wake domain.
\begin{figure}[H]
	\centering
	\subfigure[Adapted mesh - Overall view.]{\includegraphics[width=0.49\textwidth]{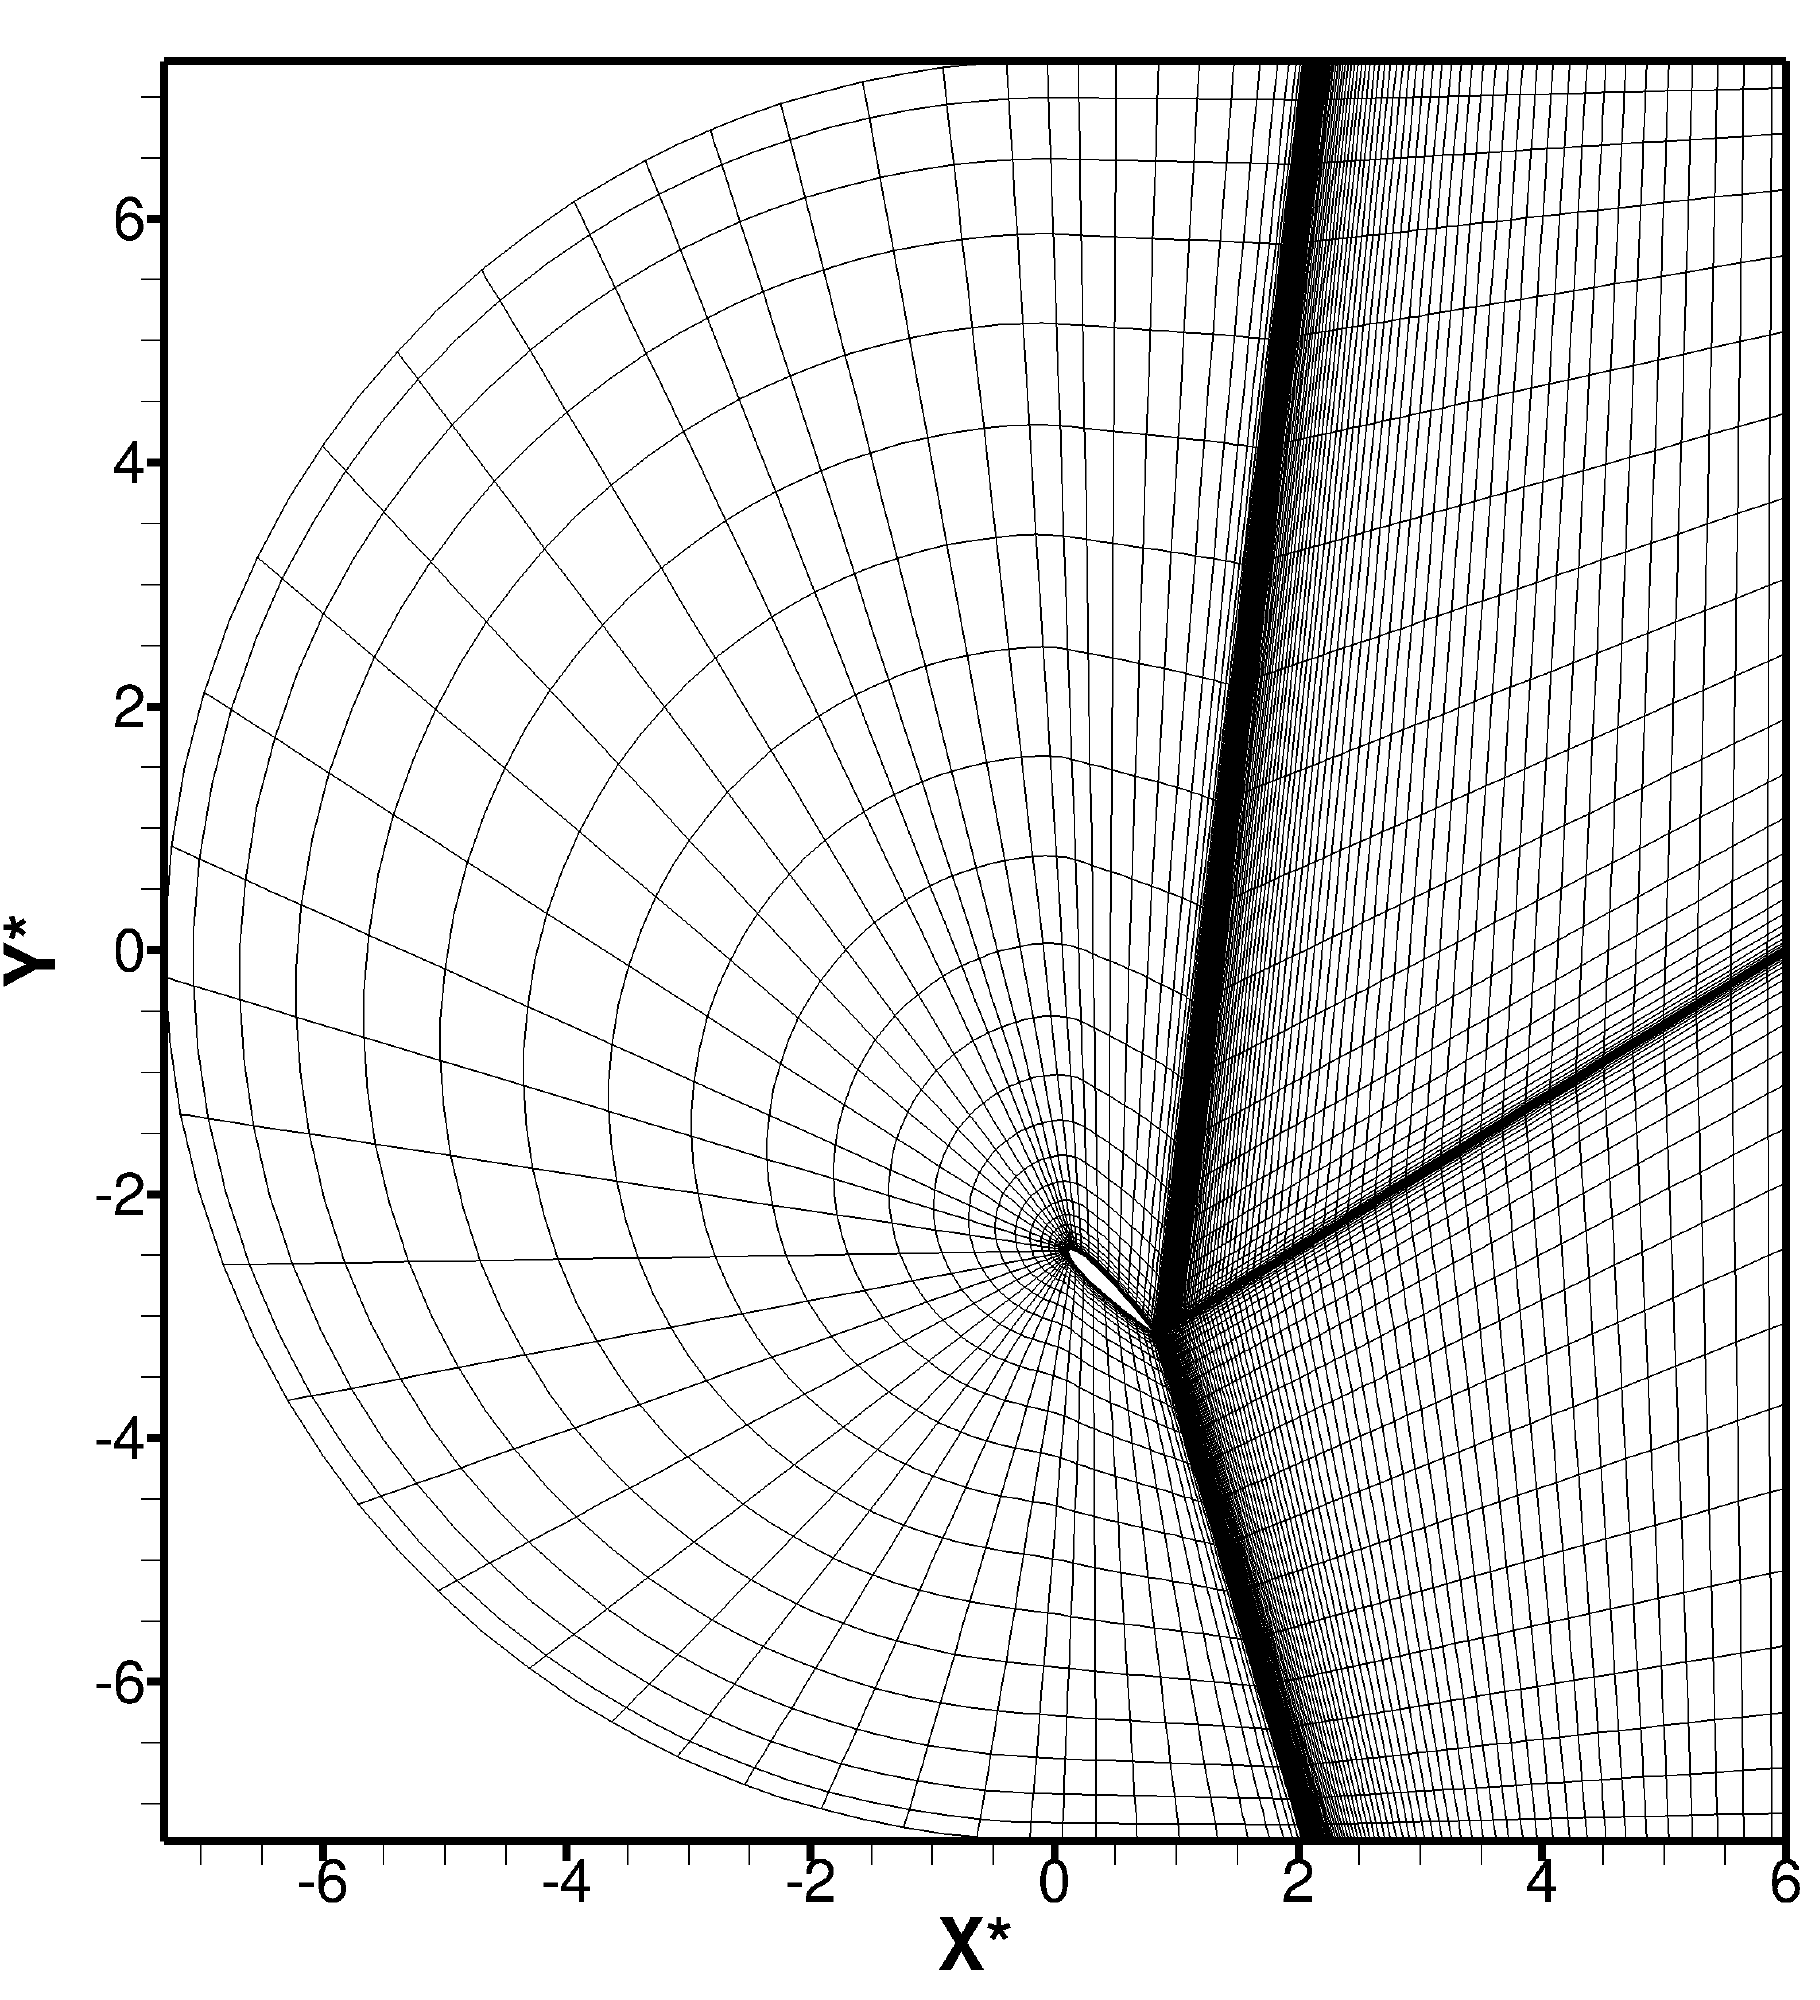} \label{fig:mesh_overall_flutter_tfi}}\hfill
	\subfigure[Adapted mesh: Focus on the trailing edge.]{\includegraphics[width=0.49\textwidth]{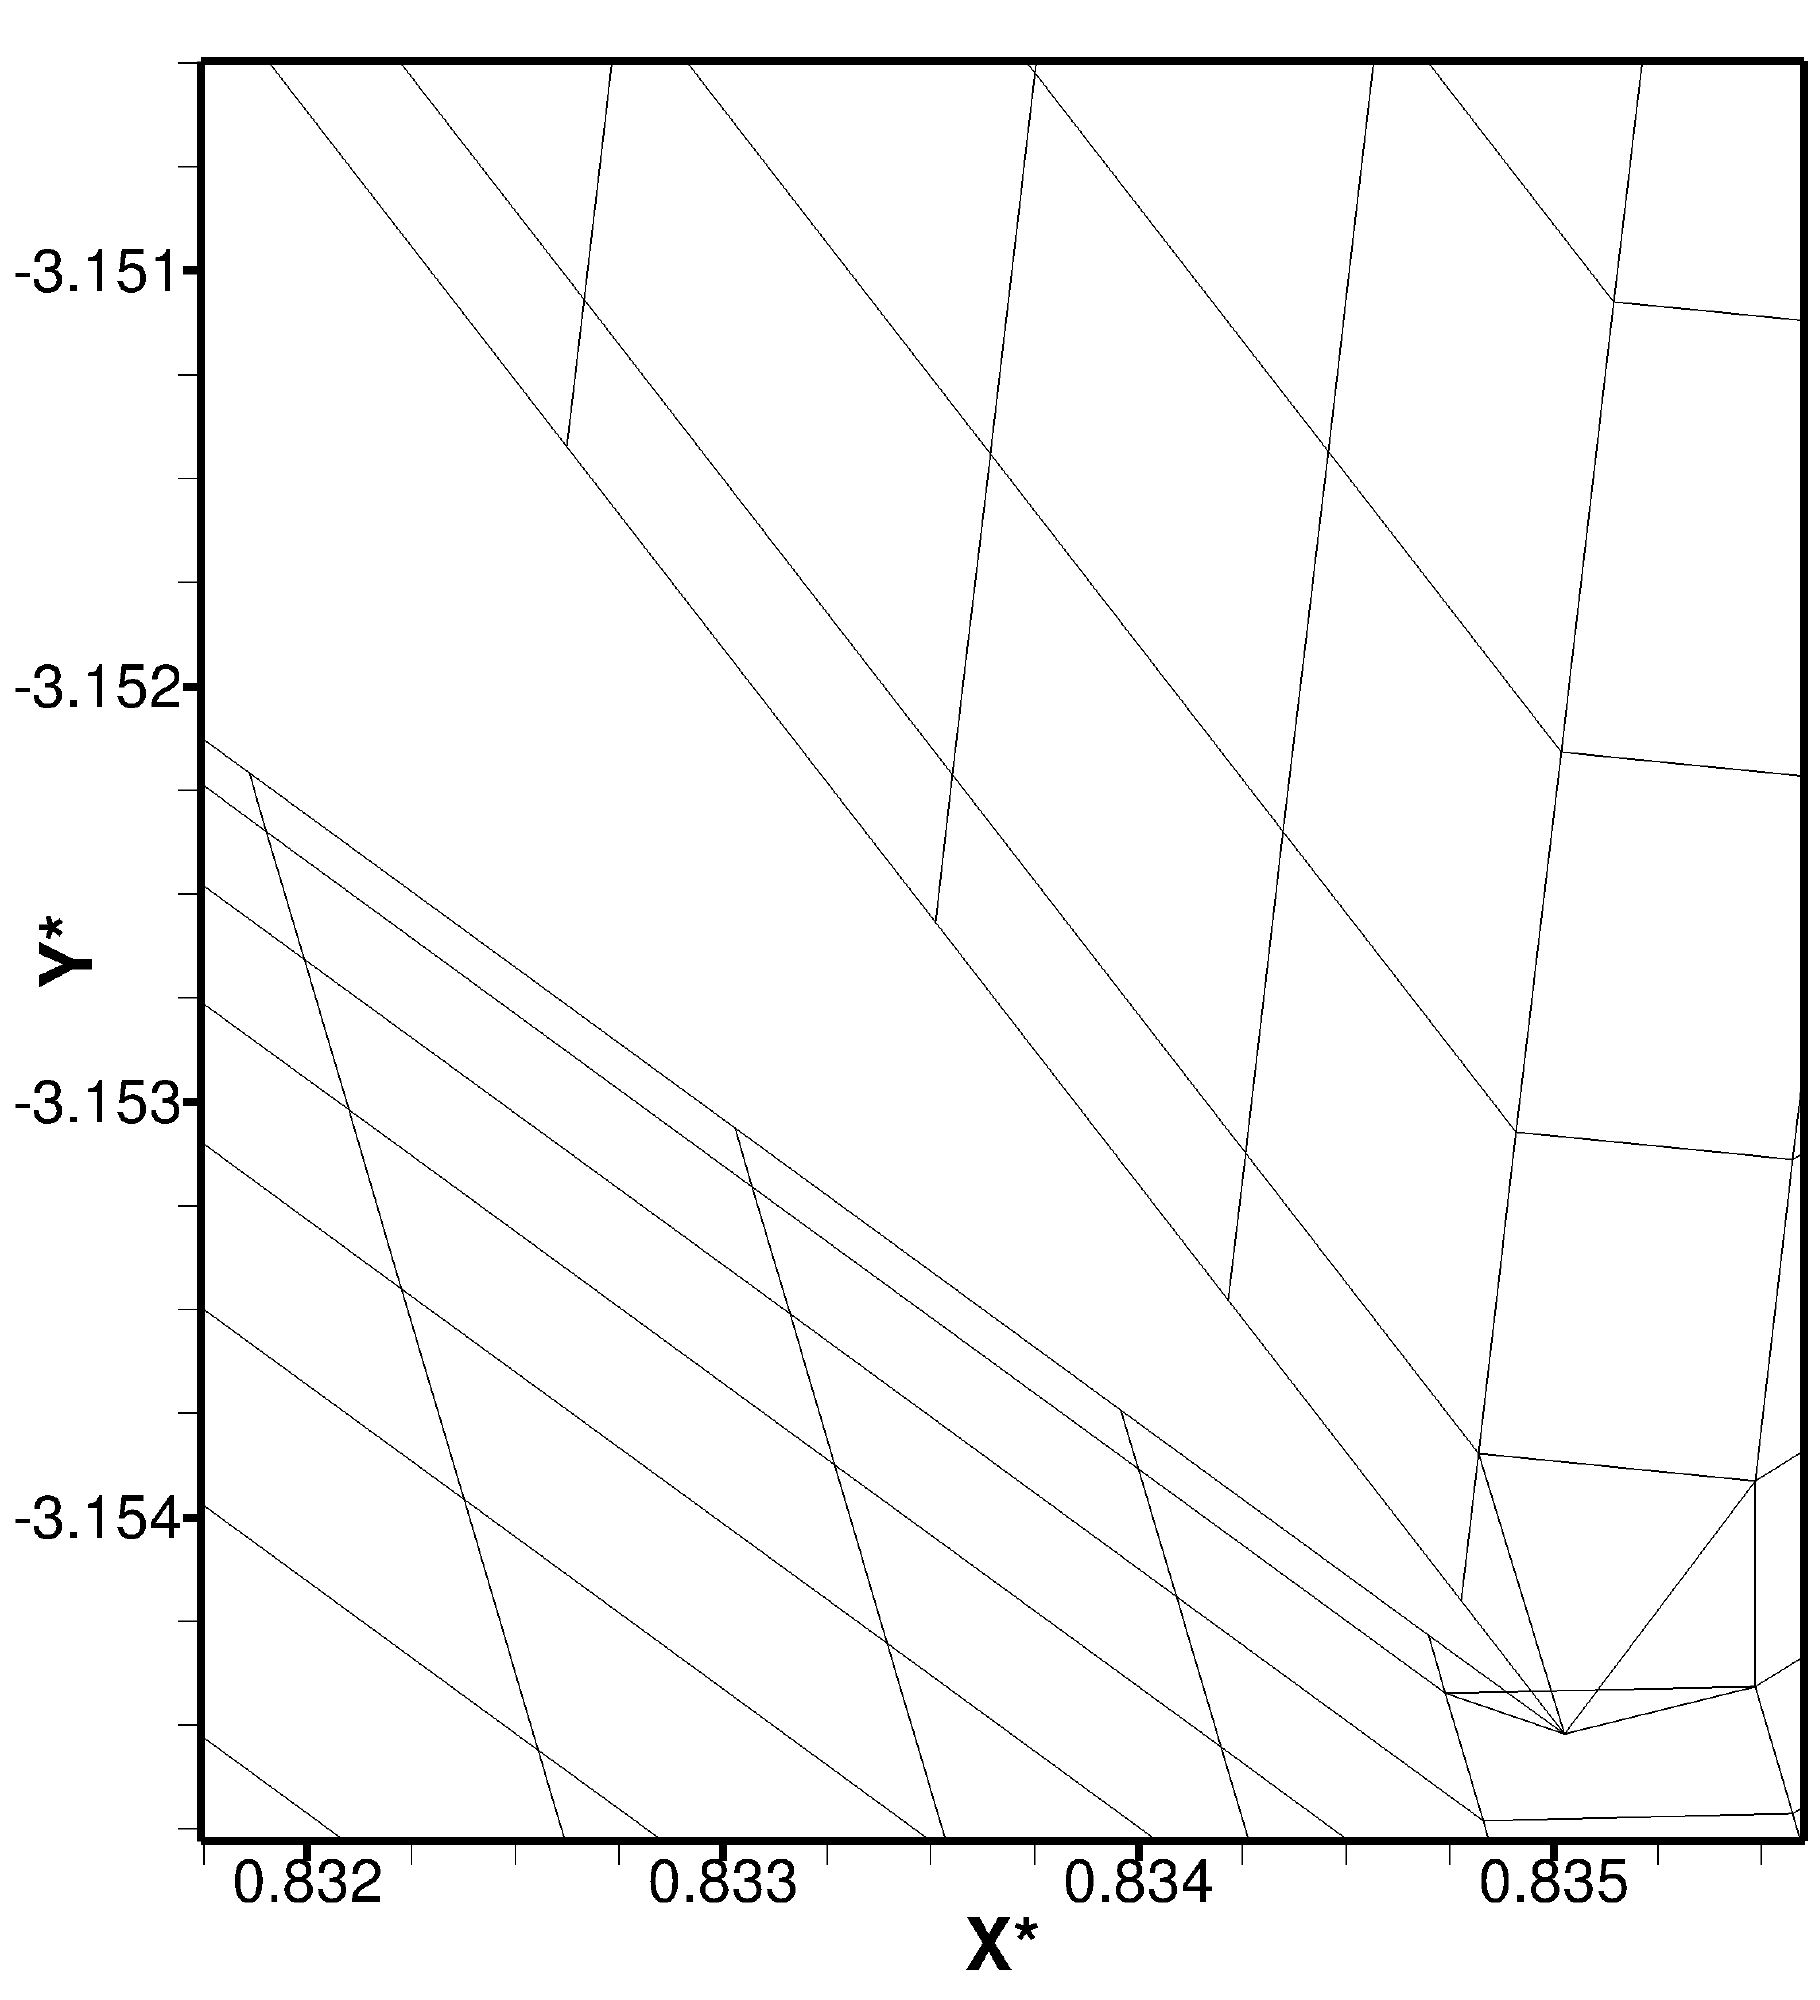}\label{fig:mesh_zoom_flutter_tfi}}\hfill
\end{figure}
\begin{figure}[H]
	\centering
	\subfigure[Mesh skew quality metric: Focus on the airfoil.]{\includegraphics[width=0.49\textwidth]{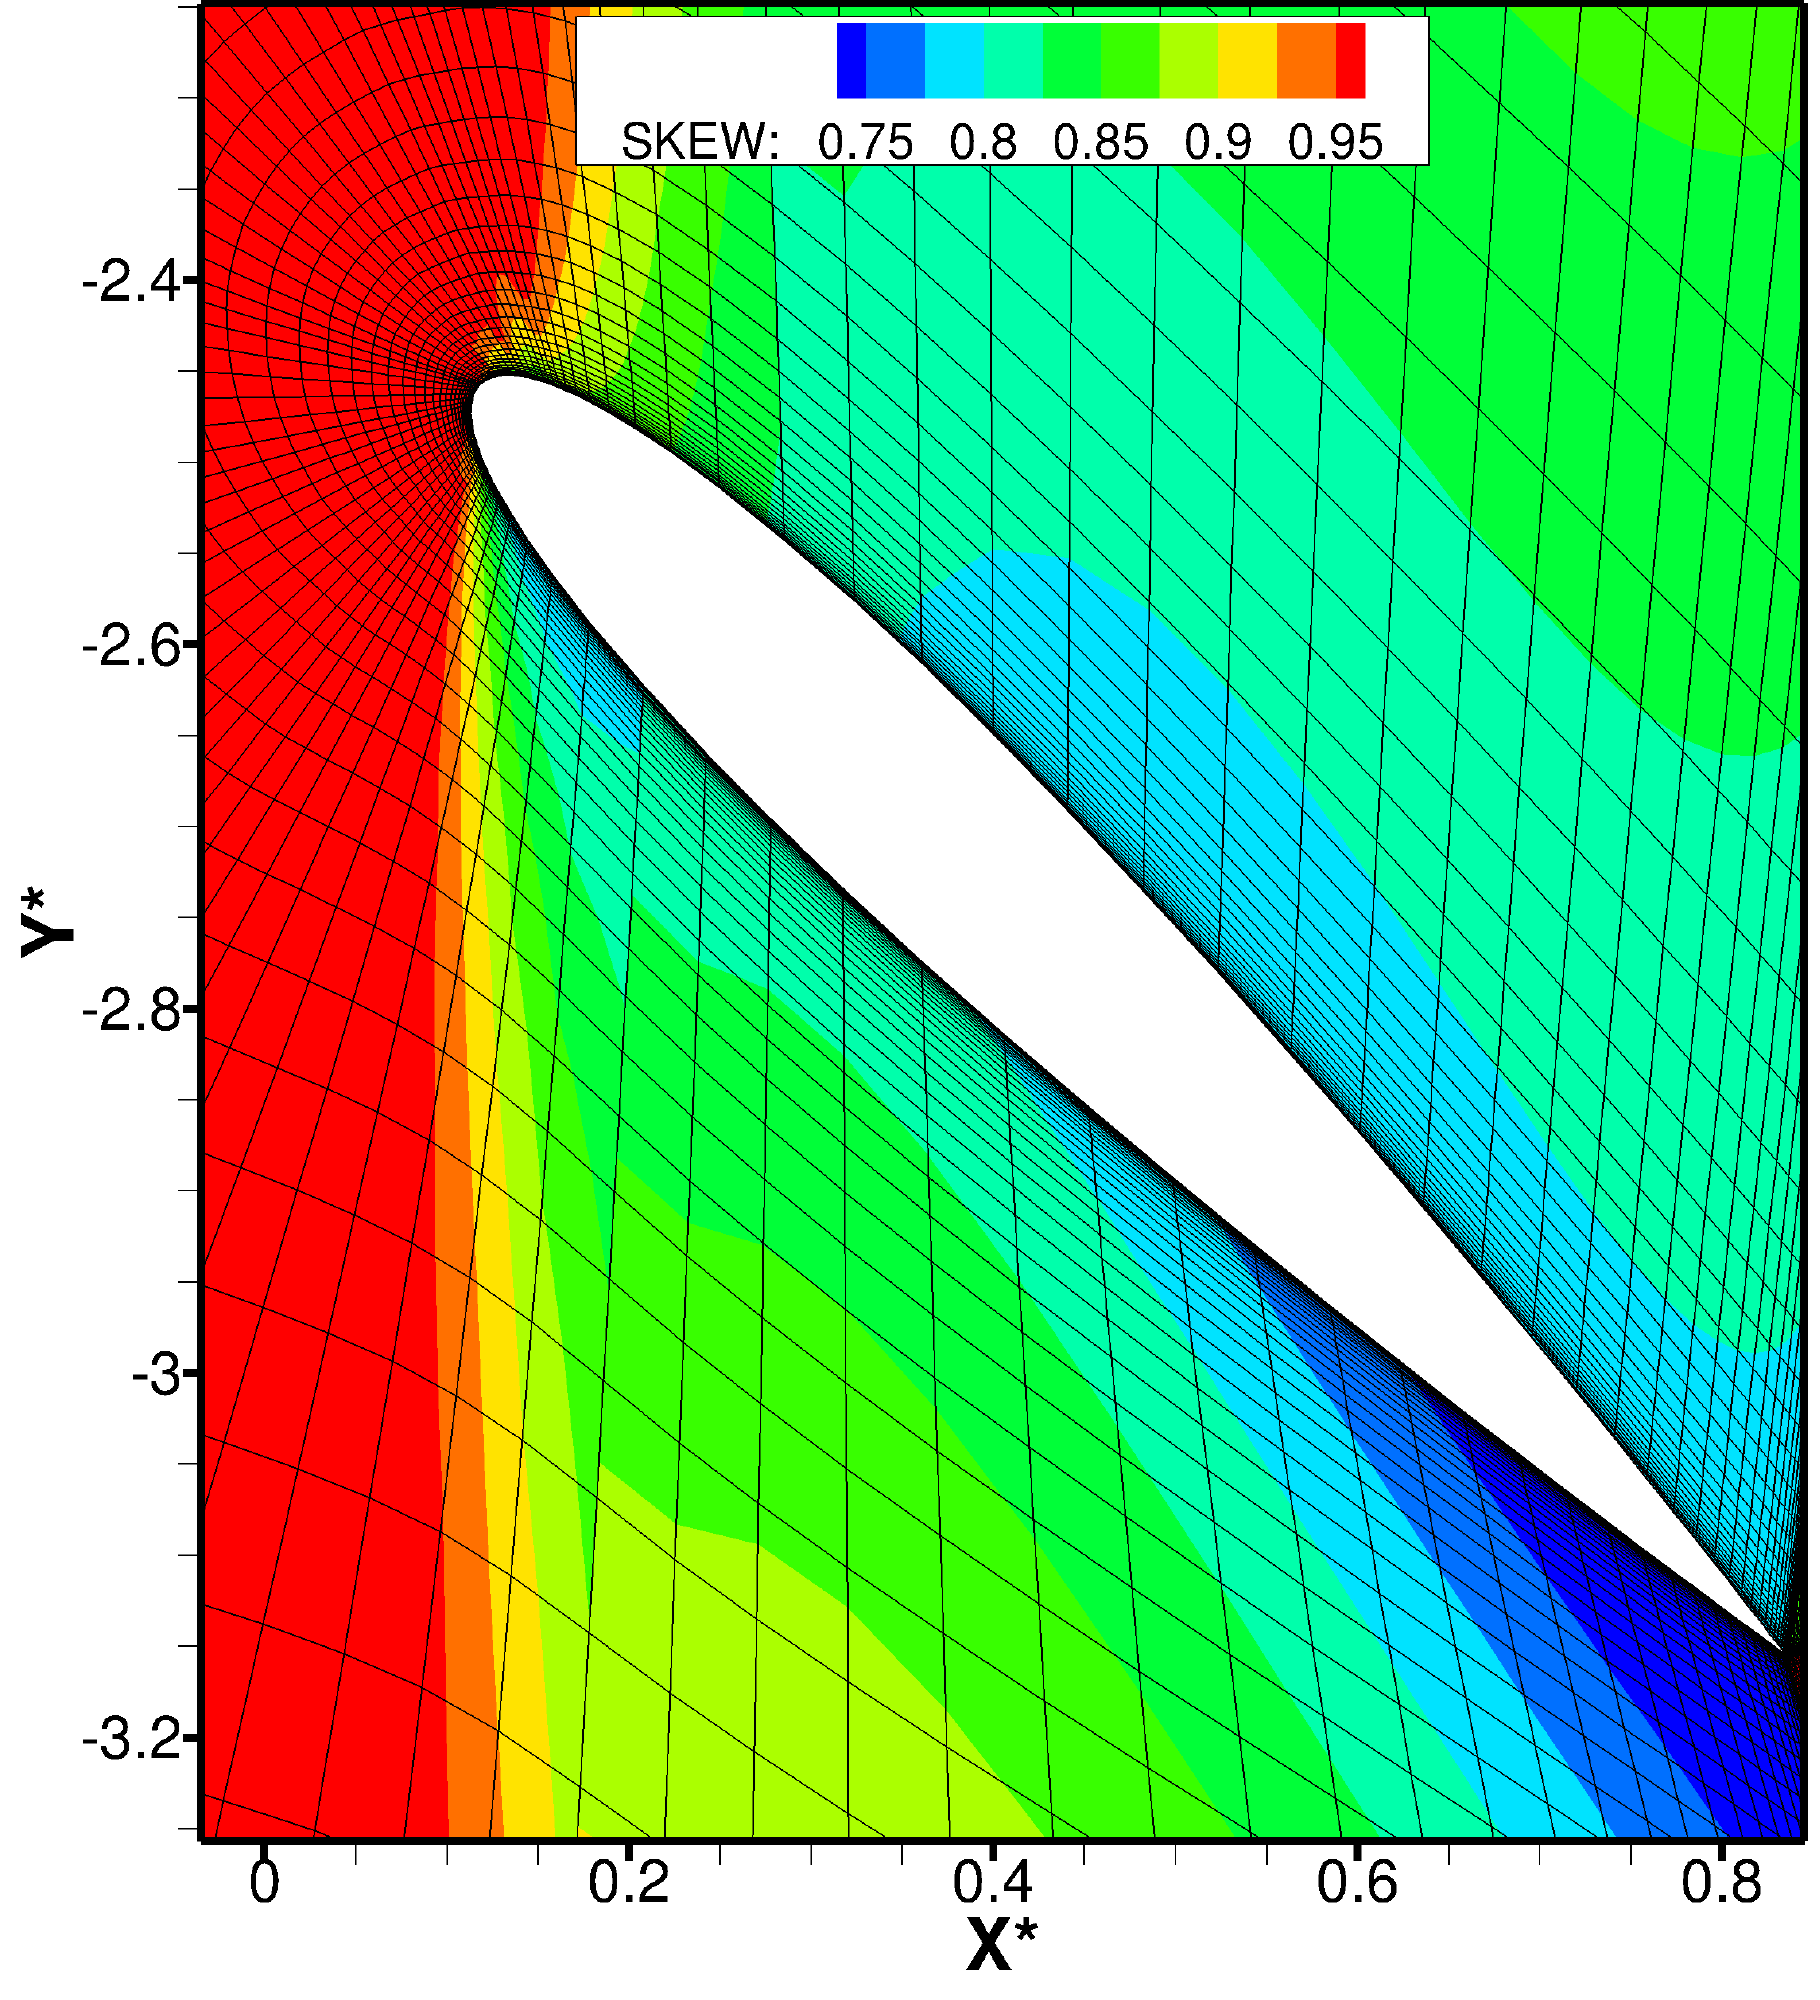}\label{fig:mesh_skew_flutter_tfi}}\hfill
	\caption{Coupled problem with TFI algorithm: Adapted mesh and grid quality at \mbox{$n=160{,}000$}.}
	\label{fig:mesh_flutter_tfi}
\end{figure}
\par The TFI mesh adaption yields the formation of cells that are not orthogonal to the boundaries, specially near the airfoil trailing edge, which leads to a loss in accuracy. The further away from the airfoil, the less the cell orthogonality is affected. Although the skew quality metric (see \mbox{Sen et al.\ \cite{Sen_2017})} indicates a reduction of the mesh quality, this is not the cause of the divergence. For instance, the skew varies between \mbox{$0.993\leq f_{skew}\leq 1$} for the undeformed mesh, i$.$e$.$, \mbox{$m{-}L_3^{min}{-}y^+_{max}$}, and between \mbox{$0.717\leq f_{skew}\leq 1$} for the deformed mesh at \mbox{$n=160{,}000$}, regarding that $f_{skew}=1$ indicates a perfect orthogonality of \mbox{the cells.} 
\par Furthermore, degenerated cells with crossovers are formed at the trailing edge of the airfoil, as well as first cells with different heights (see Fig.\ \ref{fig:mesh_zoom_flutter_tfi}). The latter is the leading cause of the divergence, since the utilized time step size is fixed at $\Delta t=5{\cdot}10^{-5}\,s$, while the first cell height is not maintained at $\Delta y^{first\,cell}=5{\cdot}10^{-5}\,m$. Indeed, this height decreases up to about $\Delta y^{first\,cell}=1.8{\cdot}10^{-5}\,m$, which would require much smaller time step sizes in order to obtain a converged solution.
\par Due to the fact, that the alteration of the first cell height is the main cause of the numerical difficulties and these are primarily yield by the translational displacement, the available re-meshing methods as well as their parameters are studied only in relation to the displacement $X_2$.  
\markboth{APPENDIX F.$\quad$INV. MSH. ADP.}{F.2$\quad$EVAL. OF THE RE-MESHING METHODS} 
\section{Evaluation of the re-meshing methods}\markboth{APPENDIX F.$\quad$INV. MSH. ADP.}{F.2$\quad$EVAL. OF THE RE-MESHING METHODS}
\label{sec:re_meshing_parameters_properties}
\par Various simulations utilizing distinct mesh adaption algorithms, as well as various re-meshing parameters are performed in order to establish the method that provides the greater accuracy while requiring the smallest computational time. These test cases are simulated considering only a translational displacement of $X_2=0.3\,m$, which is slightly greater than the maximal translational displacement achieved by the coupled simulation (see Appendix \ref{sec:case_great_airfoil_disp}), since the rotational displacement is not considered. The latter is not thoroughly studied, since it was proved that the orthogonality maintenance does not represent the main issue to the re-meshing algorithm for angles up to $\varphi_3=49.42^\circ$. 
\par The translational displacement of $X_2=0.3\,m$ is applied gradually as a boundary condition according to Eq.\ (\ref{eq:disp_func}), regarding that $A=0.3\,m$. This procedure must be undertaken, since the re-meshing algorithms adapt the mesh also in relation to the last time step. A total of $n=1{,}000$ time steps are computed with a time step size of \mbox{$\Delta t=1{\cdot}10^{-3}\,s$}. The fluid domain is not solved and therefore the required computational time represents only the time needed to adapt the mesh in relation to the new boundaries.  
\begin{equation}
\label{eq:disp_func}
X_{2,\,mesh\,adapt.}=A\,t
\end{equation}
\par The results achieved for all test cases are summarized in Table \ref{table:comp_re_meshing_algorithms}, regarding that the TFI, IDW and hybrid IDW-TFI re-meshing algorithms are examined and that the first cell height $\Delta y^{first\,cell}$ is indicated as $H$ for the sake of simplicity. Although it is already known that the former algorithm is not applicable for this test case (see \mbox{Appendix \ref{sec:case_great_airfoil_disp})}, this is also computed in order to enable a comparison of the required computational time and the mesh quality. The weighting function utilized to realize the interpolation of the IDW and IDW-TFI methods (see Section \ref{subsubsec:idw_tfi}), can be adapted according to the parameters $\alpha_{fxd}$ and $\alpha_{mv}$, regarding that their increase lead to a stiffer mesh adaption (see \mbox{Sen et al.\ \cite{Sen_2017})}. The former describes the adaption of the fixed boundaries, i$.$e$.$, inlet, outlet, symmetry, periodic and no-slip wall boundary utilized to define the form of the airfoil. The latter describes the adaption of the moving boundaries, that is, the airfoil wall boundary submitted to the fluid-structure interaction.
\begin{table}[H]
	\centering
	\begin{tabular}{p{2.3cm} p{2.3cm} p{3cm} p{3cm} p{2.5cm}}
		\hline
		\multicolumn{2}{c}{\bf{Re-meshing}} & \multicolumn{1}{c}{\multirow{2}{3cm}{\centering{\bf{Computational time (h)}}}} & \multicolumn{1}{c}{\multirow{2}{3cm}{\centering{\bf{Skew}}}} & \multicolumn{1}{c}{\multirow{2}{2.5cm}{\centering{\bf{First cell height (m)}}}} \tabularnewline\cline{1-2}
		\centering{\bf{Method}} & \centering{\bf{Parameters}} & & \tabularnewline \hline
		\multicolumn{1}{c}{\multirow{2}{*}{\centering{TFI}}} & \multicolumn{1}{c}{\multirow{2}{*}{\centering{-}}} & \multicolumn{1}{c}{\multirow{2}{*}{\centering{0.020}}} & \multicolumn{1}{c}{\multirow{2}{*}{\centering{$f_{skew}\geq0.86186$}}} & \centering{$H\geq2.8{\cdot}10^{-5}$ $H\leq 7.0{\cdot}10^{-5}$} \tabularnewline
		\multicolumn{1}{c}{\multirow{2}{*}{\centering{IDW}}} & \centering{$\alpha_{fxd}=0.1$ $\alpha_{mv}=0.3$} & \multicolumn{1}{c}{\multirow{2}{*}{\centering{9.639}}} &  \multicolumn{1}{c}{\multirow{2}{*}{\centering{$f_{skew}\geq0.59465$}}} & \multicolumn{1}{c}{\multirow{2}{*}{\centering{$H=5.0{\cdot}10^{-5}$}}} \tabularnewline
		\multicolumn{1}{c}{\multirow{2}{*}{\centering{IDW-TFI}}} & \centering{$\alpha_{fxd}=0.05$ $\alpha_{mv}=0.3$} & \multicolumn{1}{c}{\multirow{2}{*}{\centering{3.035}}} & \multicolumn{1}{c}{\multirow{2}{*}{\centering{$f_{skew}\geq0.59467$}}} & \multicolumn{1}{c}{\multirow{2}{*}{\centering{$H=5.0{\cdot}10^{-5}$}}} \tabularnewline
		\multicolumn{1}{c}{\multirow{2}{*}{\centering{IDW-TFI}}} & \centering{$\alpha_{fxd}=0.1$ $\alpha_{mv}=0.3$} & \multicolumn{1}{c}{\multirow{2}{*}{\centering{3.030}}} & \multicolumn{1}{c}{\multirow{2}{*}{\centering{$f_{skew}\geq0.59465$}}} & \multicolumn{1}{c}{\multirow{2}{*}{\centering{$H=5.0{\cdot}10^{-5}$}}} \tabularnewline
		\multicolumn{1}{c}{\multirow{2}{*}{\centering{IDW-TFI}}} & \centering{$\alpha_{fxd}=0.13$ $\alpha_{mv}=0.3$} & \multicolumn{1}{c}{\multirow{2}{*}{\centering{3.031}}} & \multicolumn{1}{c}{\multirow{2}{*}{\centering{$f_{skew}\geq0.59461$}}} & \multicolumn{1}{c}{\multirow{2}{*}{\centering{$H=5.0{\cdot}10^{-5}$}}} \tabularnewline
		\multicolumn{1}{c}{\multirow{2}{*}{\centering{IDW-TFI}}} & \centering{$\alpha_{fxd}=0.15$ $\alpha_{mv}=0.3$} & \multicolumn{1}{c}{\multirow{2}{*}{\centering{3.053}}} & \multicolumn{1}{c}{\multirow{2}{*}{\centering{$f_{skew}\geq0.59454$}}} & \multicolumn{1}{c}{\multirow{2}{*}{\centering{$H=5.0{\cdot}10^{-5}$}}} \tabularnewline
		\multicolumn{1}{c}{\multirow{2}{*}{\centering{IDW-TFI}}} & \centering{$\alpha_{fxd}=0.2$ $\alpha_{mv}=0.3$} & \multicolumn{1}{c}{\multirow{2}{*}{\centering{3.034}}} & \multicolumn{1}{c}{\multirow{2}{*}{\centering{$f_{skew}\geq0.59413$}}} & \multicolumn{1}{c}{\multirow{2}{*}{\centering{$H=5.0{\cdot}10^{-5}$}}} \tabularnewline
	\end{tabular}
\end{table}	
\begin{table}[H]
	\centering
	\begin{tabular}{p{2.3cm} p{2.3cm} p{3cm} p{3cm} p{2.5cm}}
		\multicolumn{1}{c}{\multirow{2}{2.3cm}{\centering{IDW-TFI}}} & \centering{$\alpha_{fxd}=0.5$ $\alpha_{mv}=0.3$} & \multicolumn{1}{c}{\multirow{2}{3cm}{\centering{3.032}}} & \multicolumn{1}{c}{\multirow{2}{3cm}{\centering{$f_{skew}\geq0.55951$}}} & \multicolumn{1}{c}{\multirow{2}{2.5cm}{\centering{$H=5.0{\cdot}10^{-5}$}}} \tabularnewline
		\multicolumn{1}{c}{\multirow{2}{*}{\centering{IDW-TFI}}} & \centering{$\alpha_{fxd}=0.1$ $\alpha_{mv}=0.1$} & \multicolumn{1}{c}{\multirow{2}{*}{\centering{3.033}}} & \multicolumn{1}{c}{\multirow{2}{*}{\centering{$f_{skew}\geq0.59872$}}} & \multicolumn{1}{c}{\multirow{2}{*}{\centering{$H=5.0{\cdot}10^{-5}$}}} \tabularnewline
		\multicolumn{1}{c}{\multirow{2}{*}{\centering{IDW-TFI}}} & \centering{$\alpha_{fxd}=0.13$ $\alpha_{mv}=0.1$} & \multicolumn{1}{c}{\multirow{2}{*}{\centering{3.069}}} & \multicolumn{1}{c}{\multirow{2}{*}{\centering{$f_{skew}\geq0.59868$}}} & \multicolumn{1}{c}{\multirow{2}{*}{\centering{$H=5.0{\cdot}10^{-5}$}}} \tabularnewline
		\multicolumn{1}{c}{\multirow{2}{*}{\centering{IDW-TFI}}} & \centering{$\alpha_{fxd}=0.13$ $\alpha_{mv}=0.5$} & \multicolumn{1}{c}{\multirow{2}{*}{\centering{3.031}}} & \multicolumn{1}{c}{\multirow{2}{*}{\centering{$f_{skew}\geq0.56227$}}} & \multicolumn{1}{c}{\multirow{2}{*}{\centering{$H=5.0{\cdot}10^{-5}$}}} \tabularnewline
		\hline
	\end{tabular}
	\caption{\label{table:comp_re_meshing_algorithms}Comparison of the re-meshing algorithms: Translational displacement of \mbox{$X_2=0.3\,m$}.}
\end{table}
\par The smallest computational time is achieved utilizing the TFI algorithm, which adapted mesh is illustrated in Fig.\ \ref{fig:mesh_tfi_re_meshing} for the considered displacement, regarding that one out ot two mesh lines is displayed for both the $\xi$-axis on the front domain and the $\eta$-axis on the whole fluid domain. Although this method generates the best mesh orthogonality, this measure of the mesh quality is only not deeply affected due to the fact that no airfoil rotation is present. The first cell height is not maintained, varying between $2.8{\cdot}10^{-5}\,m\leq \Delta y^{first\,cell}\leq 7.0{\cdot}10^{-5}\,m$ for the control volumes located on the airfoil surface,\break regarding a initial value of $\Delta y^{first\,cell}= 5.0{\cdot}10^{-5}\,m$. The cell height is also not maintained at the fixed boundaries, i$.$e$.$, the control volumes located at the bottom of the fluid domain are larger than the ones located at the top. Moreover, degenerated cells are created at the\break trailing edge. Therefore, the utilization of this adaptation method always leads to numerical difficulties if great displacements are available, even if no rotation is present.
\begin{figure}[H]
	\centering
	\subfigure[Adapted mesh - Overall view.]{\includegraphics[width=0.49\textwidth]{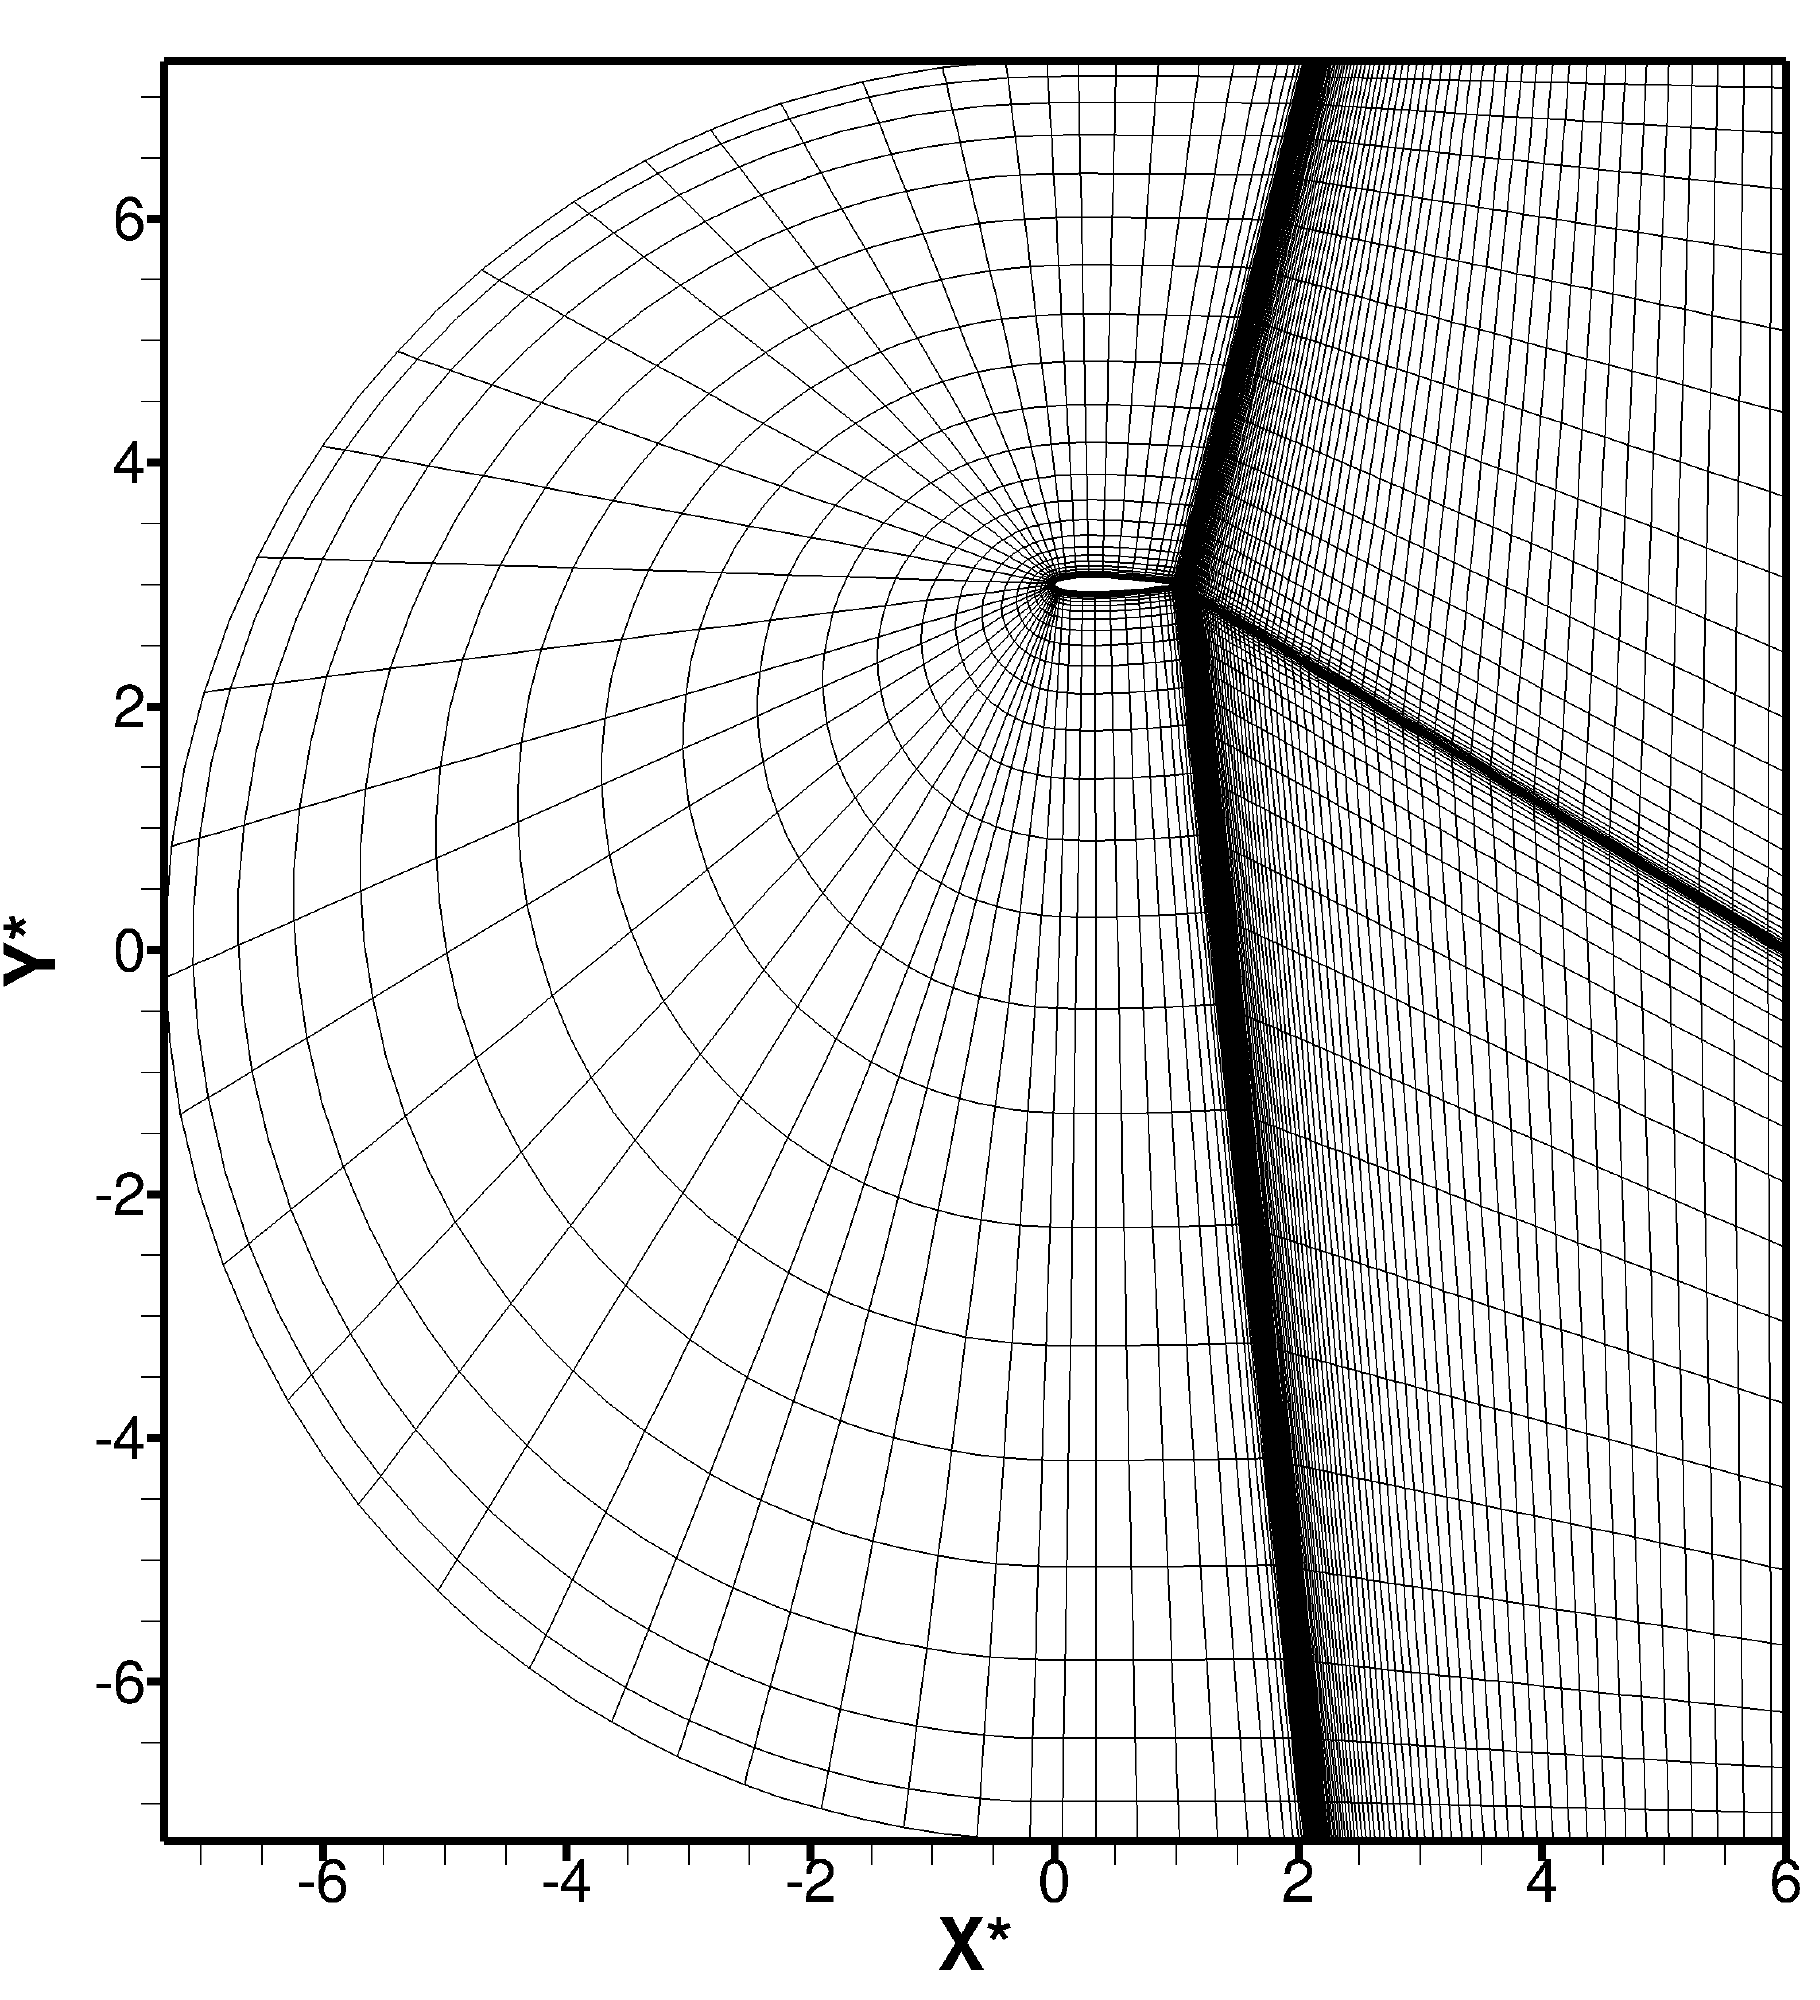} \label{fig:mesh_overall_tfi_re_meshing}}\hfill
	\subfigure[Adapted mesh - Focus on the trailing edge.]{\includegraphics[width=0.49\textwidth]{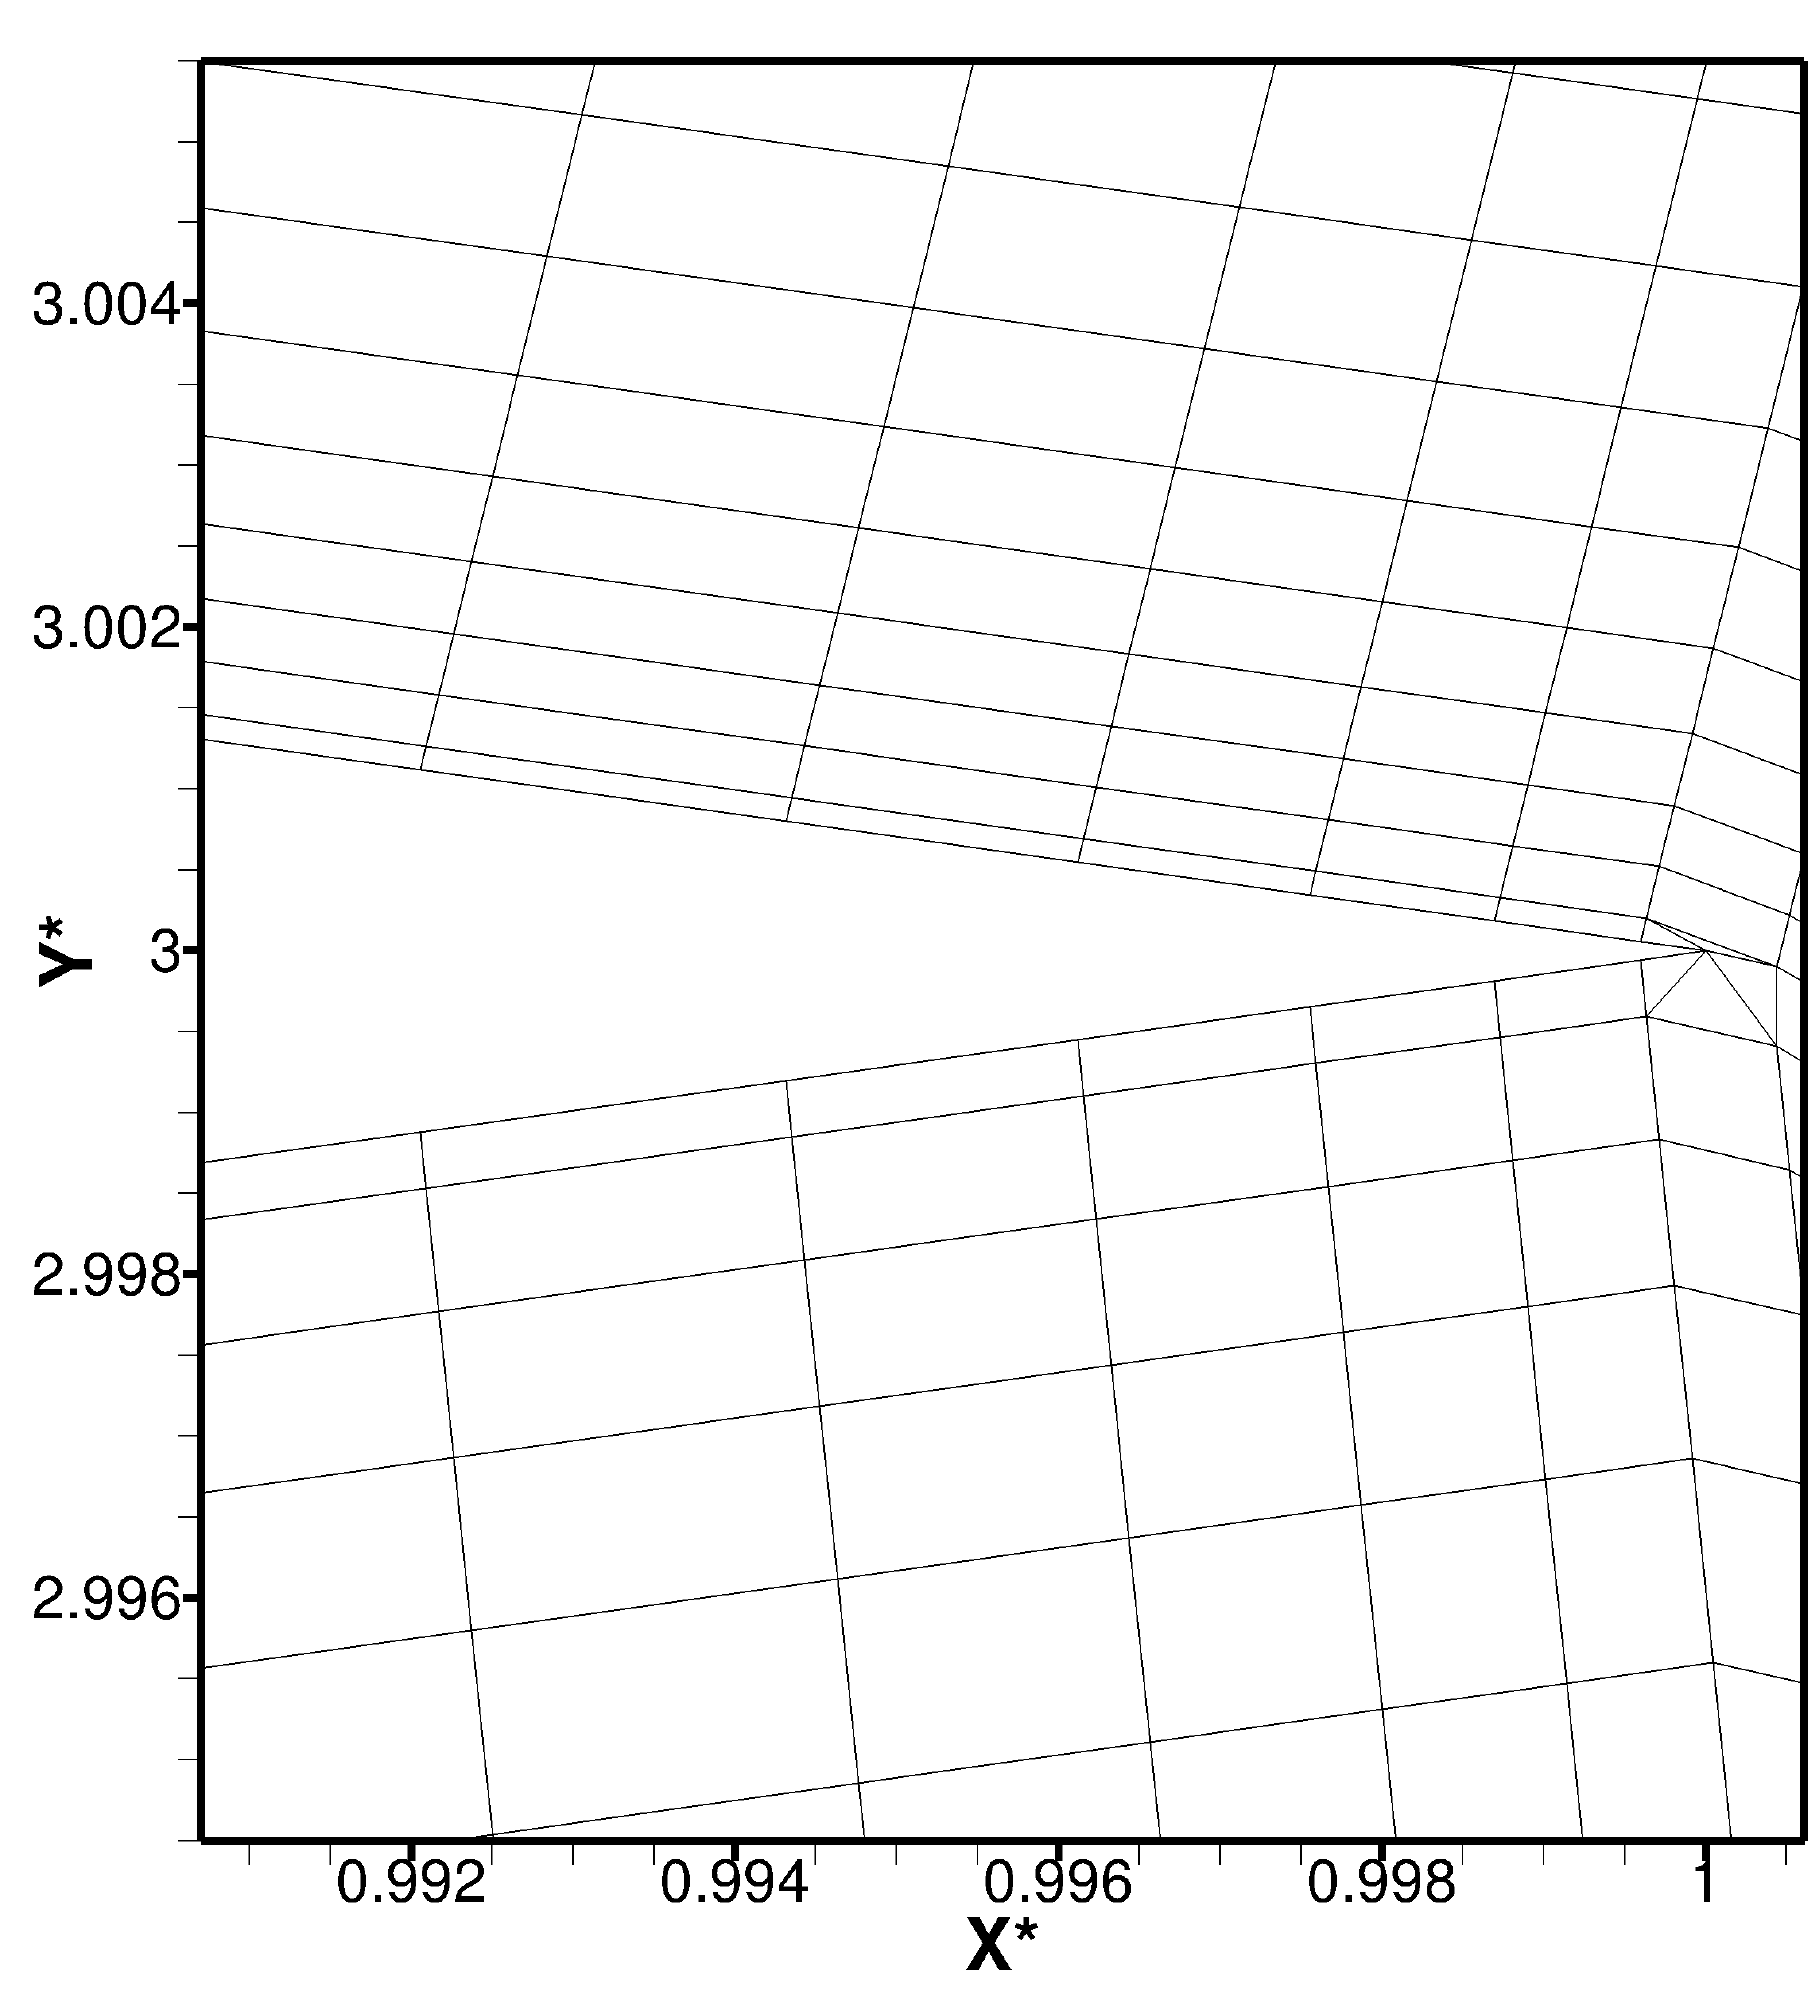} \label{fig:mesh_trailing_edge_tfi_re_meshing}}\hfill
	\caption{TFI algorithm: Mesh adaption considering a translational displacement of \mbox{$X_2=0.3\,m$}.}
	\label{fig:mesh_tfi_re_meshing}
\end{figure}
\par The IDW  and hybrid IDW-TFI methods are characterized by the maintenance of the first cell height, i$.$e$.$, $\Delta y^{first\,cell}=5{\cdot}10^{-5}\,m$. Since the required computational time of the former method is about 3.2 and 481.9 times higher than the hybrid IDW-TFI and TFI algorithms while the achieved mesh quality is exactly the same of the hybrid method, this is not considered for further studies.
\par Nine different combinations of the parameters that determine the weighting function of the fixed and the movable boundaries, i$.$e$.$, $\alpha_{fxd}$ and $\alpha_{mv}$, are investigated for the hybrid IDW-TFI algorithm. Since the best mesh quality is achieved for the parameters $\alpha_{fxd}=\alpha_{mv}=0.1$, the mesh adapted utilizing them is illustrated in Fig.\ \ref{fig:mesh_idw_tfi_re_meshing}: 
\begin{figure}[H]
	\centering
	\subfigure[Adapted mesh - Overall view.]{\includegraphics[width=0.49\textwidth]{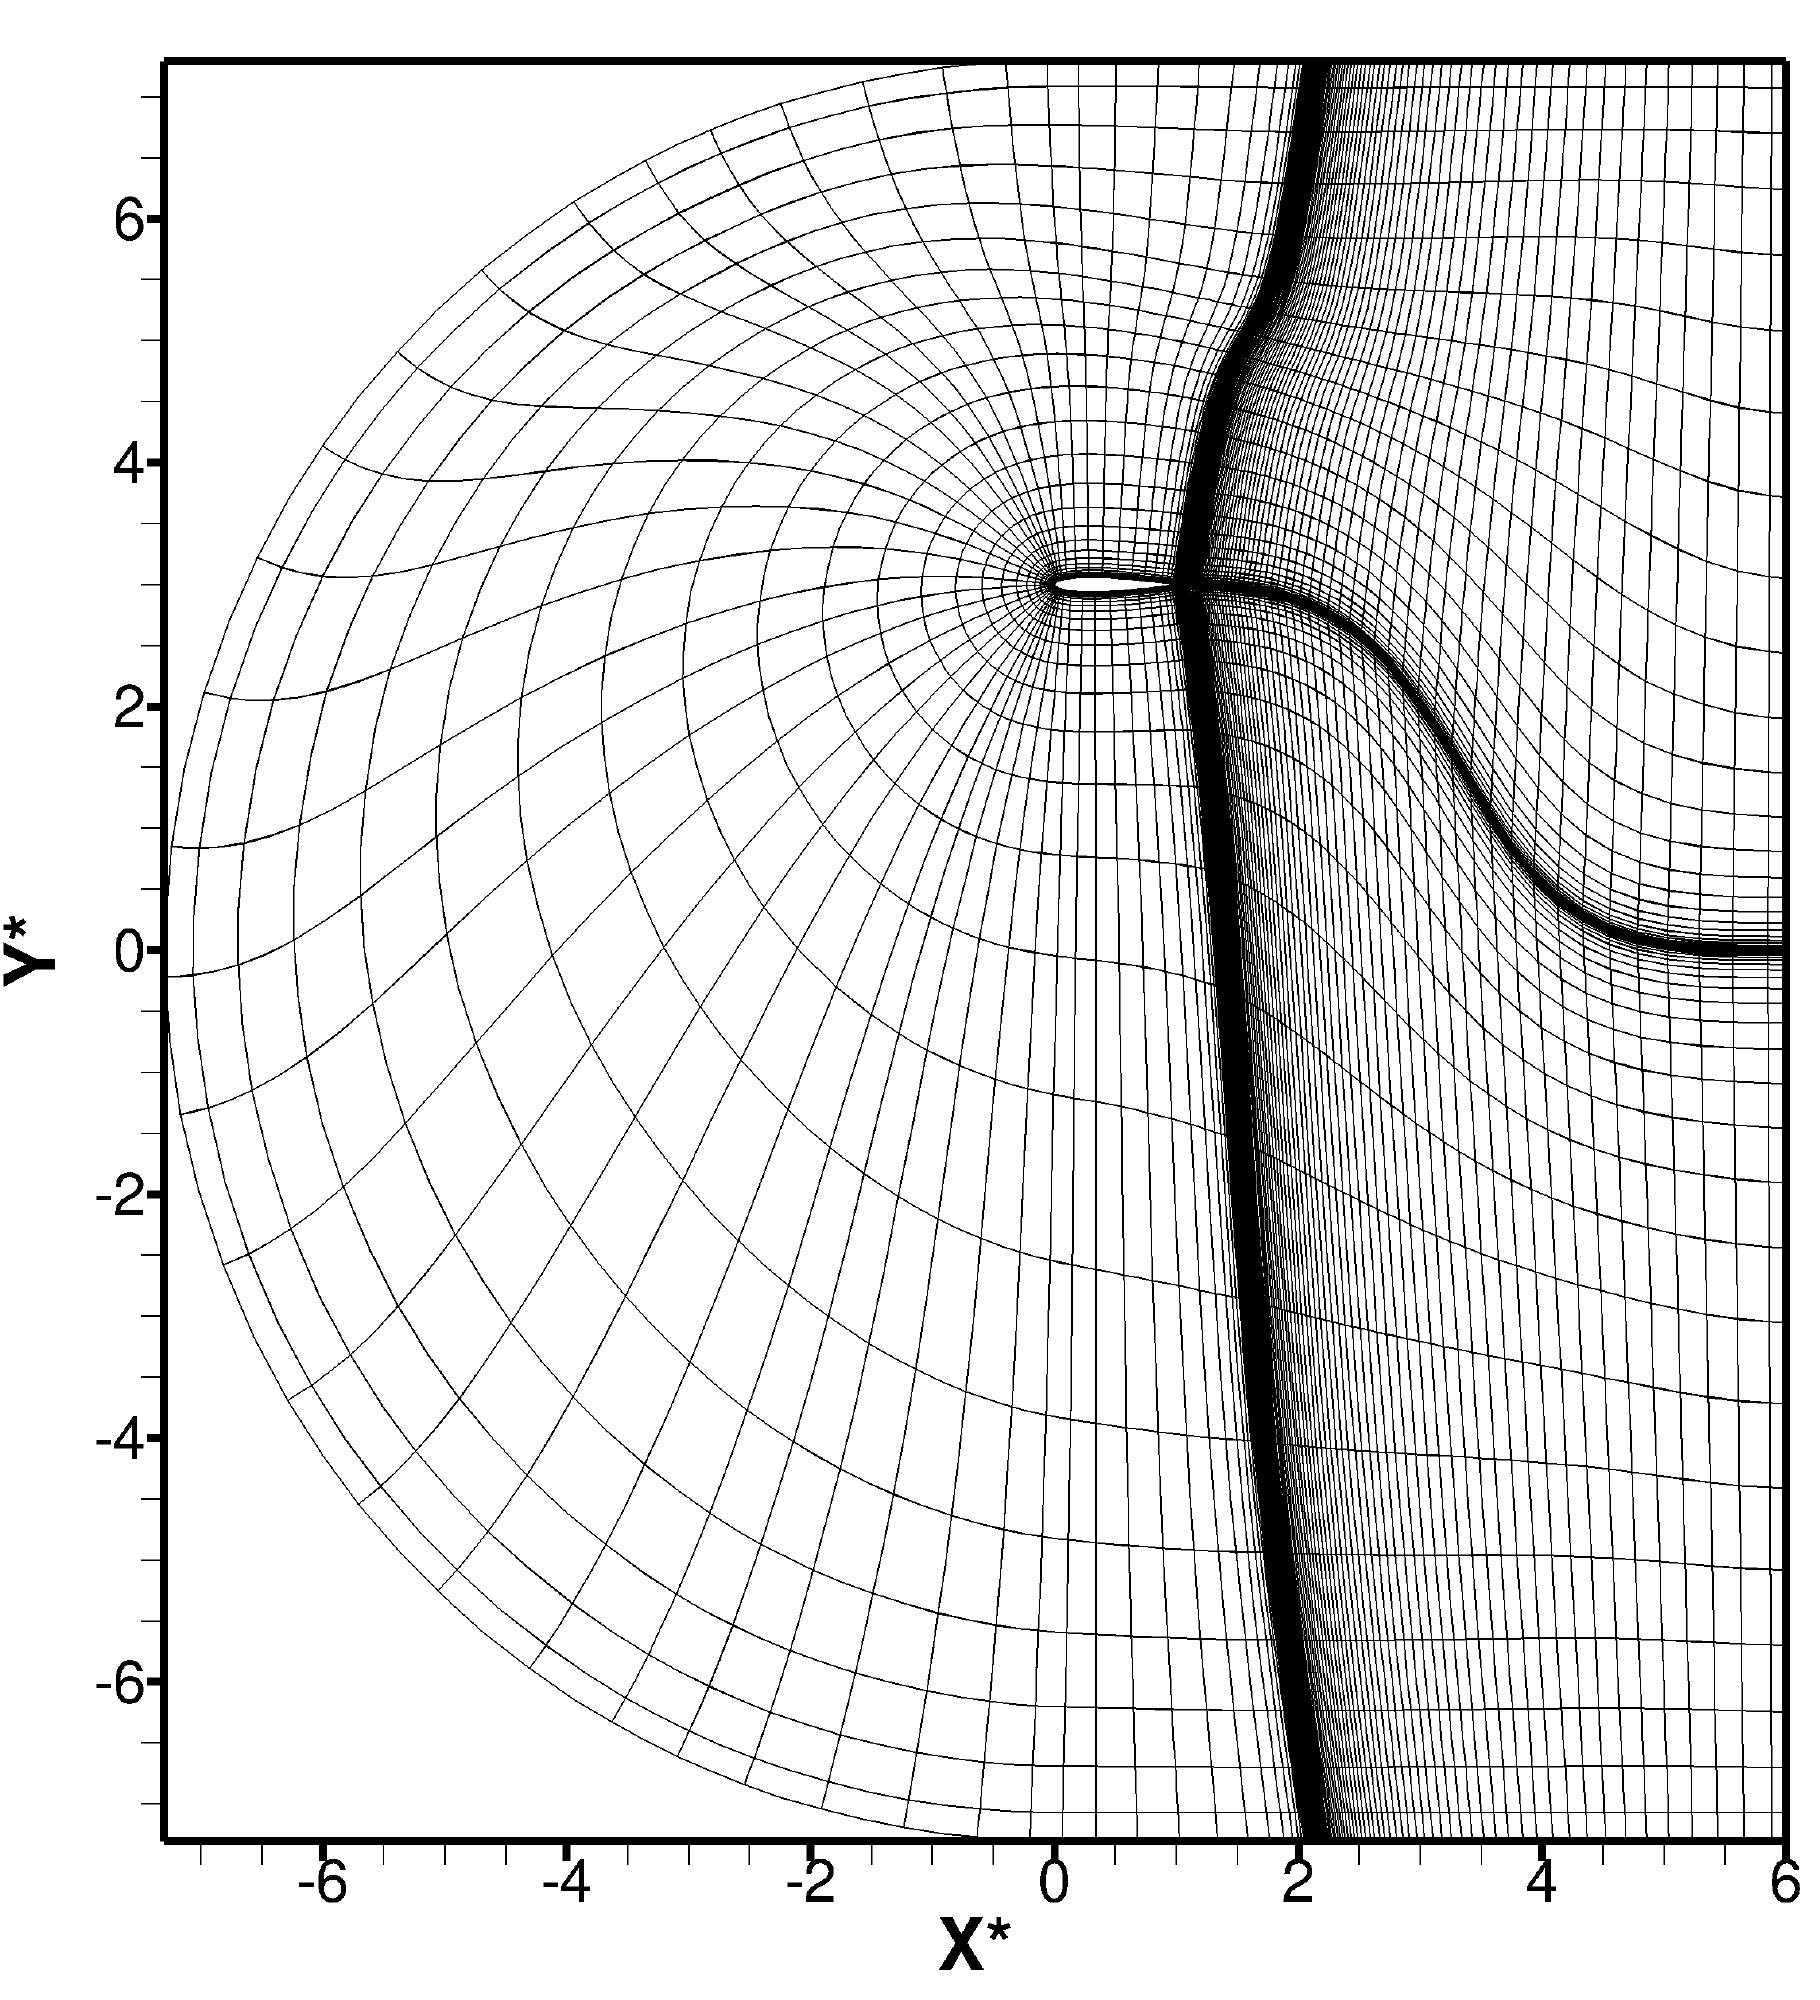} \label{fig:mesh_overall_idw_tfi_re-meshing}}\hfill
	\subfigure[Adapted mesh: Focus on the trailing edge.]{\includegraphics[width=0.49\textwidth]{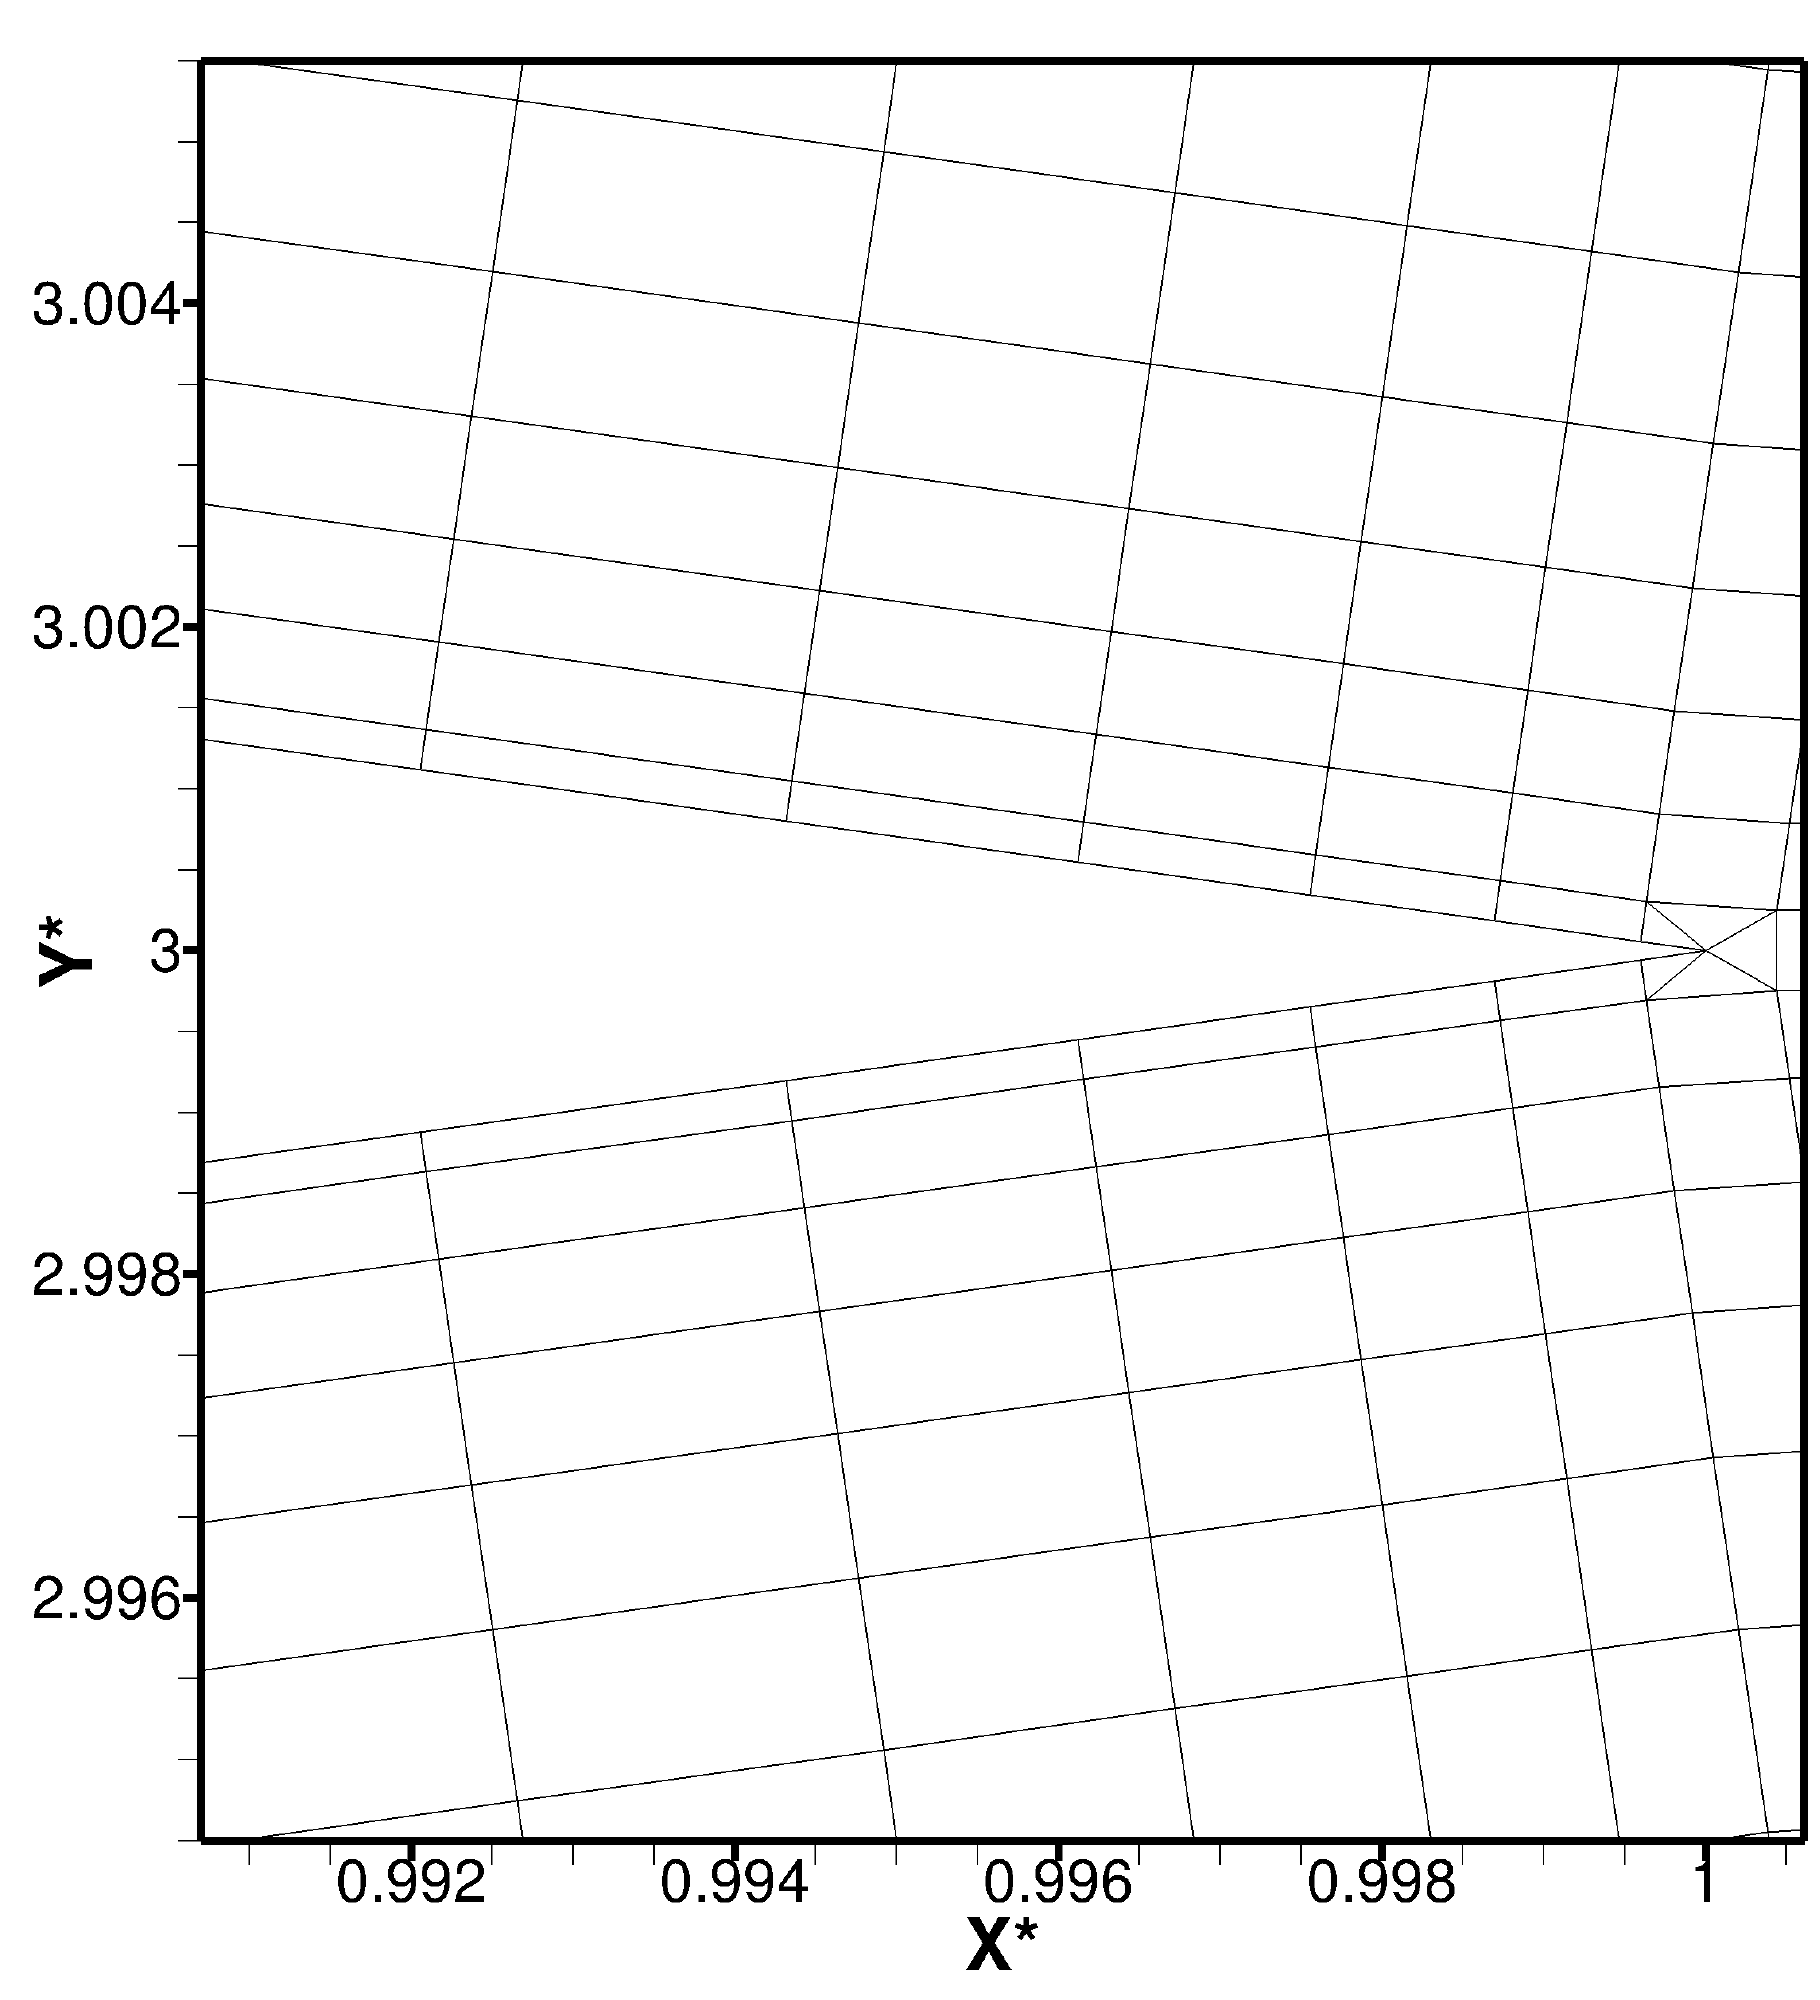}\label{fig:mesh_trailing_edge_idw_tfi_re_meshing}}\hfill
	\caption{Hybrid IDW-TFI algorithm with $\alpha_{fxd}=\alpha_{mv}=0.1$: Mesh adaption considering a translational displacement of $X_2=0.3\,m$.}
	\label{fig:mesh_idw_tfi_re_meshing}
\end{figure}
\par The problems generated by the TFI algorithm are overcome through the utilization of this method, i$.$e$.$, no degenerated cells are created at the trailing edge, as well as the first cell height is maintained for all cells located on the airfoil surface, enabling the computation with constant time step sizes. Moreover, the required computational time is reasonable considering the one needed by the IDW method. Although the achieved skew metric quality is considerably lower than the one reached with the TFI method, Fig.\ \ref{fig:mesh_skew_idw_tfi_re_meshing} illustrates that the cells with lower quality are located distant from the airfoil, which does not lead to accuracy problems since the critical flow phenomena occur near the airfoil.
\par Due to the thorough investigation of the mesh adaption algorithms, the IDW-TFI method with $\alpha_{fxd}=\alpha_{mv}=0.1$ is chosen to further simulate cases characterized by great airfoil translational and rotational displacements. Although this requires a higher computational time than the TFI method, this does not lead to numerical difficulties due to the maintenance of the height of the cells located on the airfoil surface and therefore can also be utilized for great rotations without the generation of cells with negative volumes. Moreover, the selected parameters provide the best mesh quality considering the orthogonality of the grid.  
\begin{figure}[H]
	\centering
	\centering
	\includegraphics[scale=0.85,draft=\drafttype]{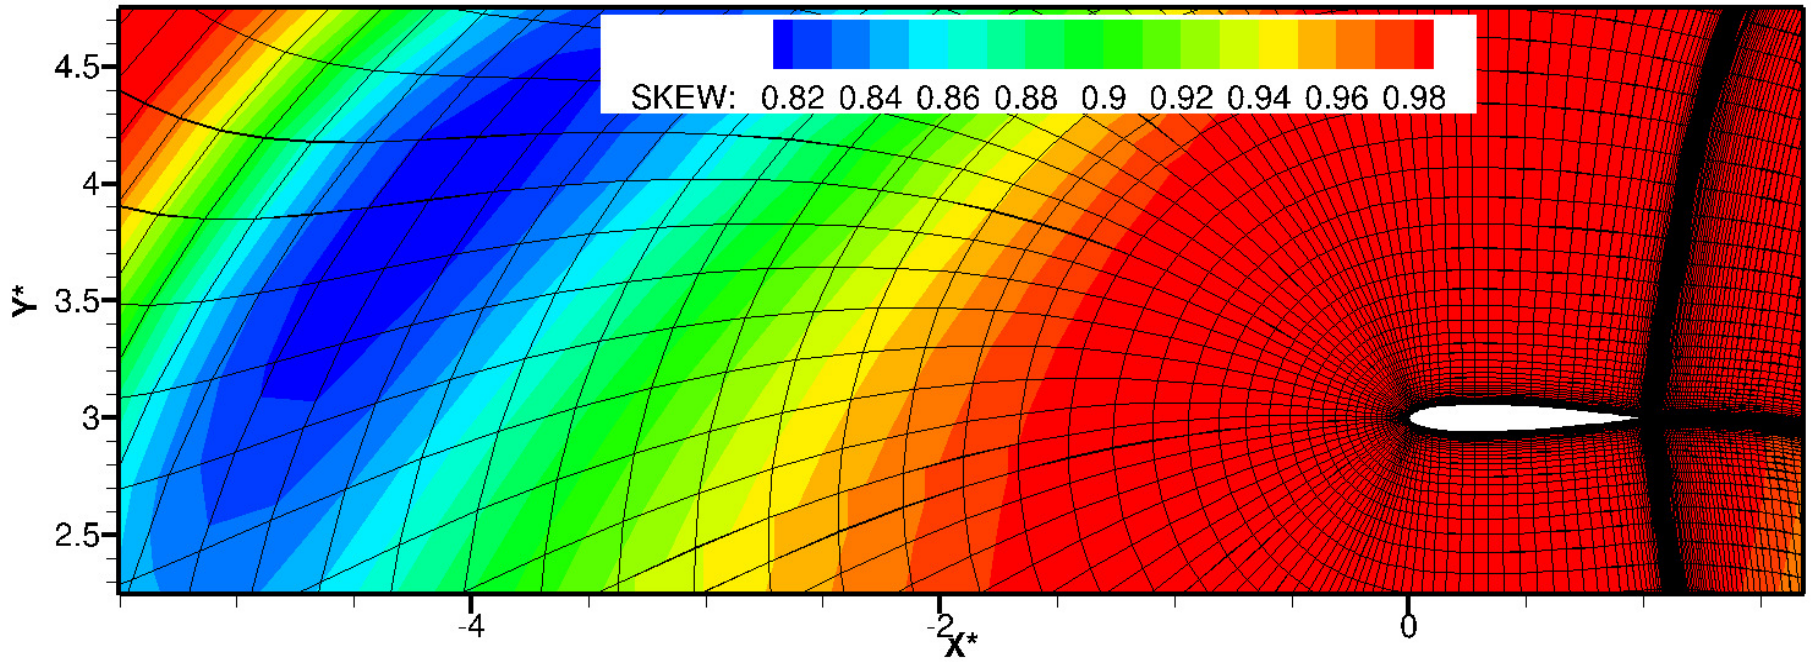}
	\caption{\label{fig:mesh_skew_idw_tfi_re_meshing}Hybrid IDW-TFI algorithm with $\alpha_{fxd}=\alpha_{mv}=0.1$: Mesh quality considering a translational displacement of $X_2=0.3\,m$.}
\end{figure}
