# Supplementary material for: Numerical investigations of the fluid-structure interaction of a NACA0012 airfoil based on large-eddy simulations
Source: arXiv:1807.01574 source file (2018-07-04)
Supplement: Supplementary file 6 [file appendix_tfi_idw_tfi_new.tex]

\par The available mesh adaption algorithms are thoroughly analyzed regarding the maximal displacements achieved by the numerous performed simulations, which are characterized by different system configurations. Since the largest displacements are achieved for the test case characterized by extremely small linear and torsional stiffnesses (see \mbox{Section \ref{subsec:inv_great_airfoil_disp})}, the investigations are based on the maximal airfoil response achieved by this computation.
\par Various simulations utilizing distinct mesh adaption algorithms, as well as various re-meshing parameters are performed in order to establish the method that provides the better quality of the mesh while requiring the smallest computational time. These test cases are simulated considering only a translational displacement of $X_2=0.3\,\text{m}$, which is slightly greater than the maximal translational displacement achieved by the coupled simulation with the TFI re-meshing algorithm (see Section \ref{subsec:inv_great_airfoil_disp}), since the rotational displacement is not considered. The latter is not thoroughly studied, since the cause of the numerical difficulties for angles up to $\varphi_3=49.42^\circ$ is actually the maintenance of the height of the cells located on the airfoil surface and not the preservation of the mesh orthogonality (see Section \ref{subsec:inv_great_airfoil_disp}).
\par The translational displacement of $X_2=0.3\,\text{m}$ is gradually applied as a boundary condition according to Eq.\ (\ref{eq:disp_func}), regarding that $A=0.3\,m$. This procedure must be undertaken, since the IDW and hybrid IDW-TFI algorithms adapt the mesh also in relation to the last time step. A total of $n=1{,}000$ time steps are computed with a time step size of \mbox{$\Delta t=1{\cdot}10^{-3}\,\text{s}$}. The fluid domain is not solved and therefore the required computational time represents only the time needed to adapt the mesh in relation to the new boundaries.  
\begin{equation}
\label{eq:disp_func}
X_{2,\,mesh\,adapt.}=A\,t
\end{equation}
\par The results achieved for all test cases are summarized in Table \ref{table:comp_re_meshing_algorithms}, regarding that the TFI, IDW and hybrid IDW-TFI re-meshing algorithms are examined and that the first cell height $\Delta y^{first\,cell}$ is indicated as $H$ for the sake of simplicity. Although the former algorithm is not applicable for this test case (see \mbox{Section \ref{subsec:inv_great_airfoil_disp})}, this is also computed in order to enable a comparison of the required computational time and the mesh quality. The weighting function utilized to realize the interpolation of the IDW and IDW-TFI methods (see Section \ref{subsubsec:idw_tfi}), can be adapted according to the parameters $\alpha_{fxd}$ and $\alpha_{mv}$, regarding that their increase lead to a stiffer mesh adaption (see \mbox{Sen et al.\ \cite{Sen_2017})}. The former describes the adaption of the fixed boundaries, i$.$e$.$, inlet, outlet, symmetry and periodic while the latter describes the adaption of the moving boundaries, that is, the airfoil wall boundary submitted to the fluid-structure interaction.
\begin{table}[H]
	\centering
	\begin{tabular}{p{3cm} p{3cm} p{3.5cm} p{3.5cm}}
		\hline
		\multicolumn{2}{c}{\bf{Re-meshing}} & \multicolumn{1}{c}{\multirow{2}{3cm}{\centering{\bf{Computational time (h)}}}} & \multicolumn{1}{c}{\multirow{2}{2.5cm}{\centering{\bf{First cell height (m)}}}} \tabularnewline\cline{1-2}
		\centering{\bf{Method}} & \centering{\bf{Parameters}} & & \tabularnewline \hline
		\multicolumn{1}{c}{\multirow{2}{*}{\centering{TFI}}} & \multicolumn{1}{c}{\multirow{2}{*}{\centering{-}}} & \multicolumn{1}{c}{\multirow{2}{*}{\centering{0.020}}} & \centering{$H\geq2.8{\cdot}10^{-5}$ $H\leq 7.0{\cdot}10^{-5}$} \tabularnewline
		\multicolumn{1}{c}{\multirow{2}{*}{\centering{IDW}}} & \centering{$\alpha_{fxd}=0.1$ $\alpha_{mv}=0.3$} & \multicolumn{1}{c}{\multirow{2}{*}{\centering{9.639}}} & \multicolumn{1}{c}{\multirow{2}{*}{\centering{$H=5.0{\cdot}10^{-5}$}}} \tabularnewline
		\multicolumn{1}{c}{\multirow{2}{*}{\centering{IDW-TFI}}} & \centering{$\alpha_{fxd}=0.05$ $\alpha_{mv}=0.3$} & \multicolumn{1}{c}{\multirow{2}{*}{\centering{3.035}}} & \multicolumn{1}{c}{\multirow{2}{*}{\centering{$H=5.0{\cdot}10^{-5}$}}} \tabularnewline
		\multicolumn{1}{c}{\multirow{2}{*}{\centering{IDW-TFI}}} & \centering{$\alpha_{fxd}=0.1$ $\alpha_{mv}=0.3$} & \multicolumn{1}{c}{\multirow{2}{*}{\centering{3.030}}} & \multicolumn{1}{c}{\multirow{2}{*}{\centering{$H=5.0{\cdot}10^{-5}$}}} \tabularnewline
		\multicolumn{1}{c}{\multirow{2}{*}{\centering{IDW-TFI}}} & \centering{$\alpha_{fxd}=0.13$ $\alpha_{mv}=0.3$} & \multicolumn{1}{c}{\multirow{2}{*}{\centering{3.031}}} & \multicolumn{1}{c}{\multirow{2}{*}{\centering{$H=5.0{\cdot}10^{-5}$}}} \tabularnewline
		\multicolumn{1}{c}{\multirow{2}{*}{\centering{IDW-TFI}}} & \centering{$\alpha_{fxd}=0.15$ $\alpha_{mv}=0.3$} & \multicolumn{1}{c}{\multirow{2}{*}{\centering{3.053}}} & \multicolumn{1}{c}{\multirow{2}{*}{\centering{$H=5.0{\cdot}10^{-5}$}}} \tabularnewline
		\multicolumn{1}{c}{\multirow{2}{*}{\centering{IDW-TFI}}} & \centering{$\alpha_{fxd}=0.2$ $\alpha_{mv}=0.3$} & \multicolumn{1}{c}{\multirow{2}{*}{\centering{3.034}}} & \multicolumn{1}{c}{\multirow{2}{*}{\centering{$H=5.0{\cdot}10^{-5}$}}} \tabularnewline
%	\end{tabular}
%\end{table}	
%\begin{table}[H]
%	\centering
%	\begin{tabular}{p{2.3cm} p{2.3cm} p{3cm} p{3cm} p{2.5cm}}
		\multicolumn{1}{c}{\multirow{2}{2.3cm}{\centering{IDW-TFI}}} & \centering{$\alpha_{fxd}=0.5$ $\alpha_{mv}=0.3$} & \multicolumn{1}{c}{\multirow{2}{3cm}{\centering{3.032}}} & \multicolumn{1}{c}{\multirow{2}{2.5cm}{\centering{$H=5.0{\cdot}10^{-5}$}}} \tabularnewline
		\multicolumn{1}{c}{\multirow{2}{*}{\centering{IDW-TFI}}} & \centering{$\alpha_{fxd}=0.1$ $\alpha_{mv}=0.1$} & \multicolumn{1}{c}{\multirow{2}{*}{\centering{3.033}}} & \multicolumn{1}{c}{\multirow{2}{*}{\centering{$H=5.0{\cdot}10^{-5}$}}} \tabularnewline
		\multicolumn{1}{c}{\multirow{2}{*}{\centering{IDW-TFI}}} & \centering{$\alpha_{fxd}=0.13$ $\alpha_{mv}=0.1$} & \multicolumn{1}{c}{\multirow{2}{*}{\centering{3.069}}} & \multicolumn{1}{c}{\multirow{2}{*}{\centering{$H=5.0{\cdot}10^{-5}$}}} \tabularnewline
		\multicolumn{1}{c}{\multirow{2}{*}{\centering{IDW-TFI}}} & \centering{$\alpha_{fxd}=0.13$ $\alpha_{mv}=0.5$} & \multicolumn{1}{c}{\multirow{2}{*}{\centering{3.031}}} & \multicolumn{1}{c}{\multirow{2}{*}{\centering{$H=5.0{\cdot}10^{-5}$}}} \tabularnewline
		\hline
	\end{tabular}
	\caption{\label{table:comp_re_meshing_algorithms}Comparison of the re-meshing algorithms: Translational displacement of \mbox{$X_2=0.3\,m$}.}
\end{table}
\par The smallest computational time is achieved utilizing the TFI algorithm, which adapted mesh is illustrated in Fig.\ \ref{fig:mesh_tfi_re_meshing} for the considered displacement, regarding that one out ot two mesh lines is displayed for both the $\xi$-axis on the front domain and the $\eta$-axis on the whole fluid domain. The mesh orthogonality is only not deeply affected due to the fact that no airfoil rotation is present. The first cell height is not maintained, varying between $2.8{\cdot}10^{-5}\,\text{m}\leq \Delta y^{first\,cell}\leq 7.0{\cdot}10^{-5}\,\text{m}$ for the control volumes located on the airfoil surface,\break regarding a initial value of $\Delta y^{first\,cell}= 5.0{\cdot}10^{-5}\,m$. The cell height is also not maintained at the fixed boundaries, i$.$e$.$, the control volumes located at the bottom of the fluid domain are larger than the ones located at the top. Moreover, degenerated cells are created at the\break trailing edge. Therefore, the utilization of this adaptation method always leads to numerical difficulties if large displacements are observed, even if no rotation is present.
\begin{figure}[H]
	\centering
	\subfigure[Adapted mesh - Overall view.]{\includegraphics[width=0.48\textwidth]{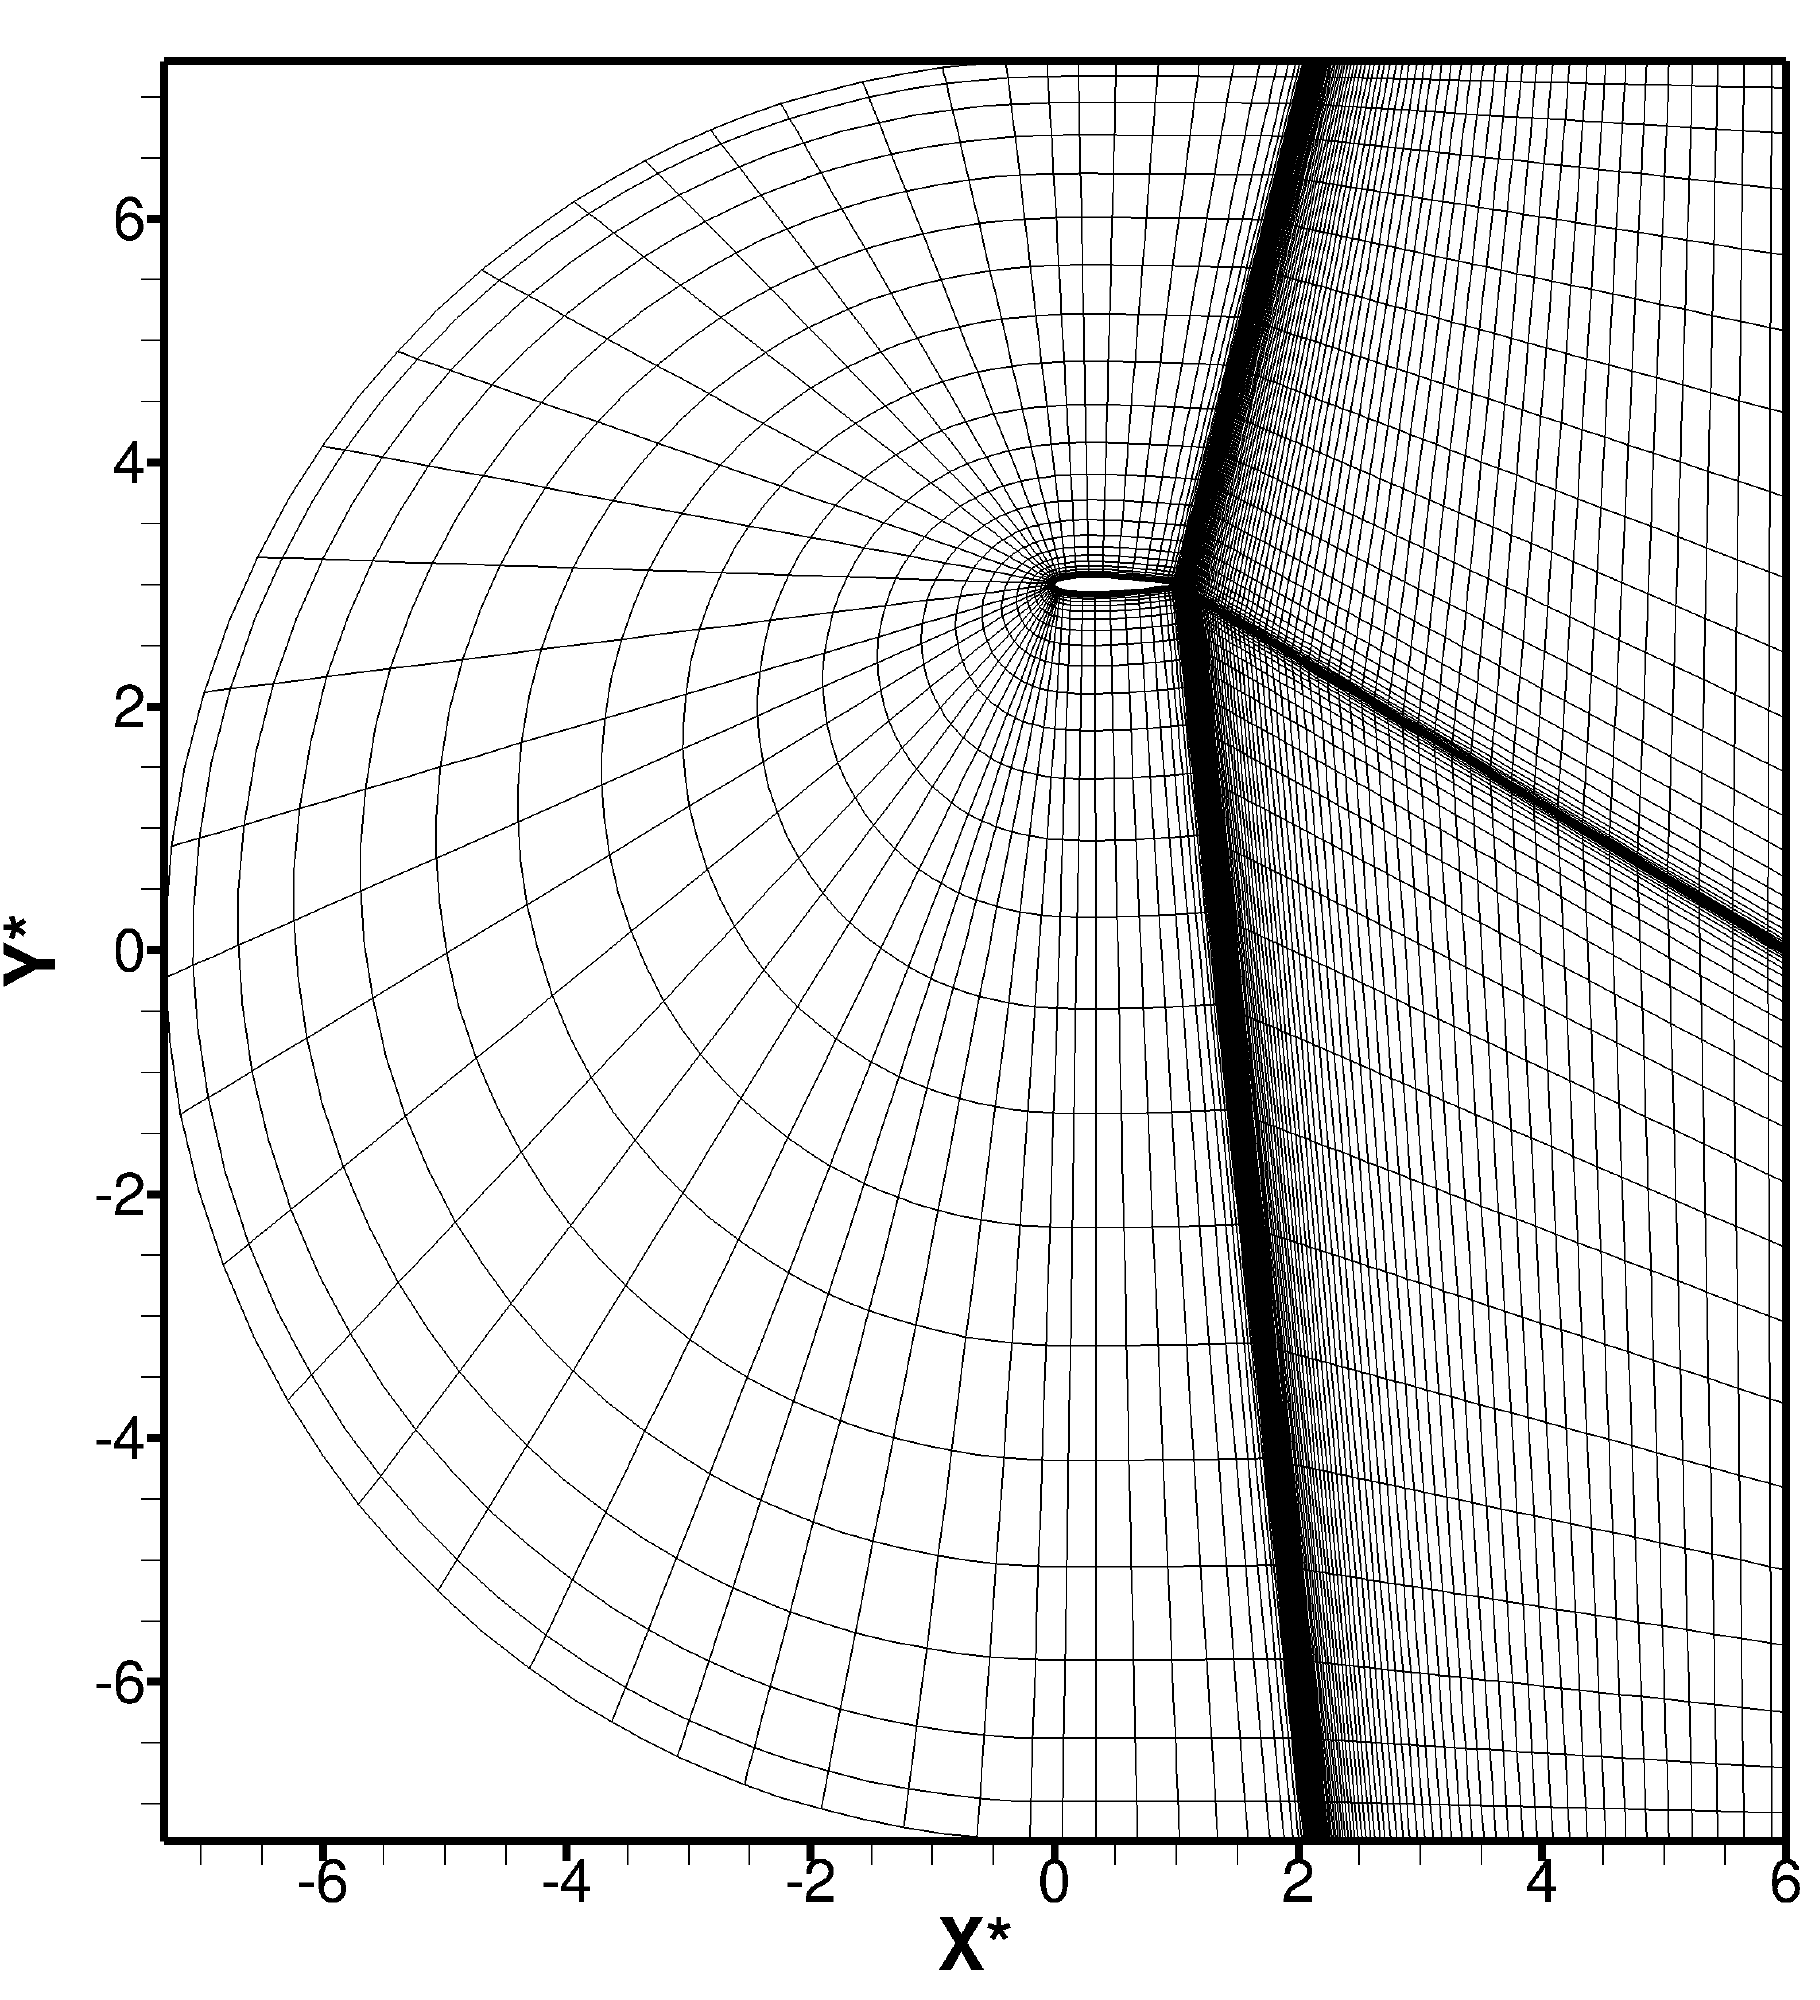} \label{fig:mesh_overall_tfi_re_meshing}}\hfill
	\subfigure[Adapted mesh - Focus on the trailing edge.]{\includegraphics[width=0.48\textwidth]{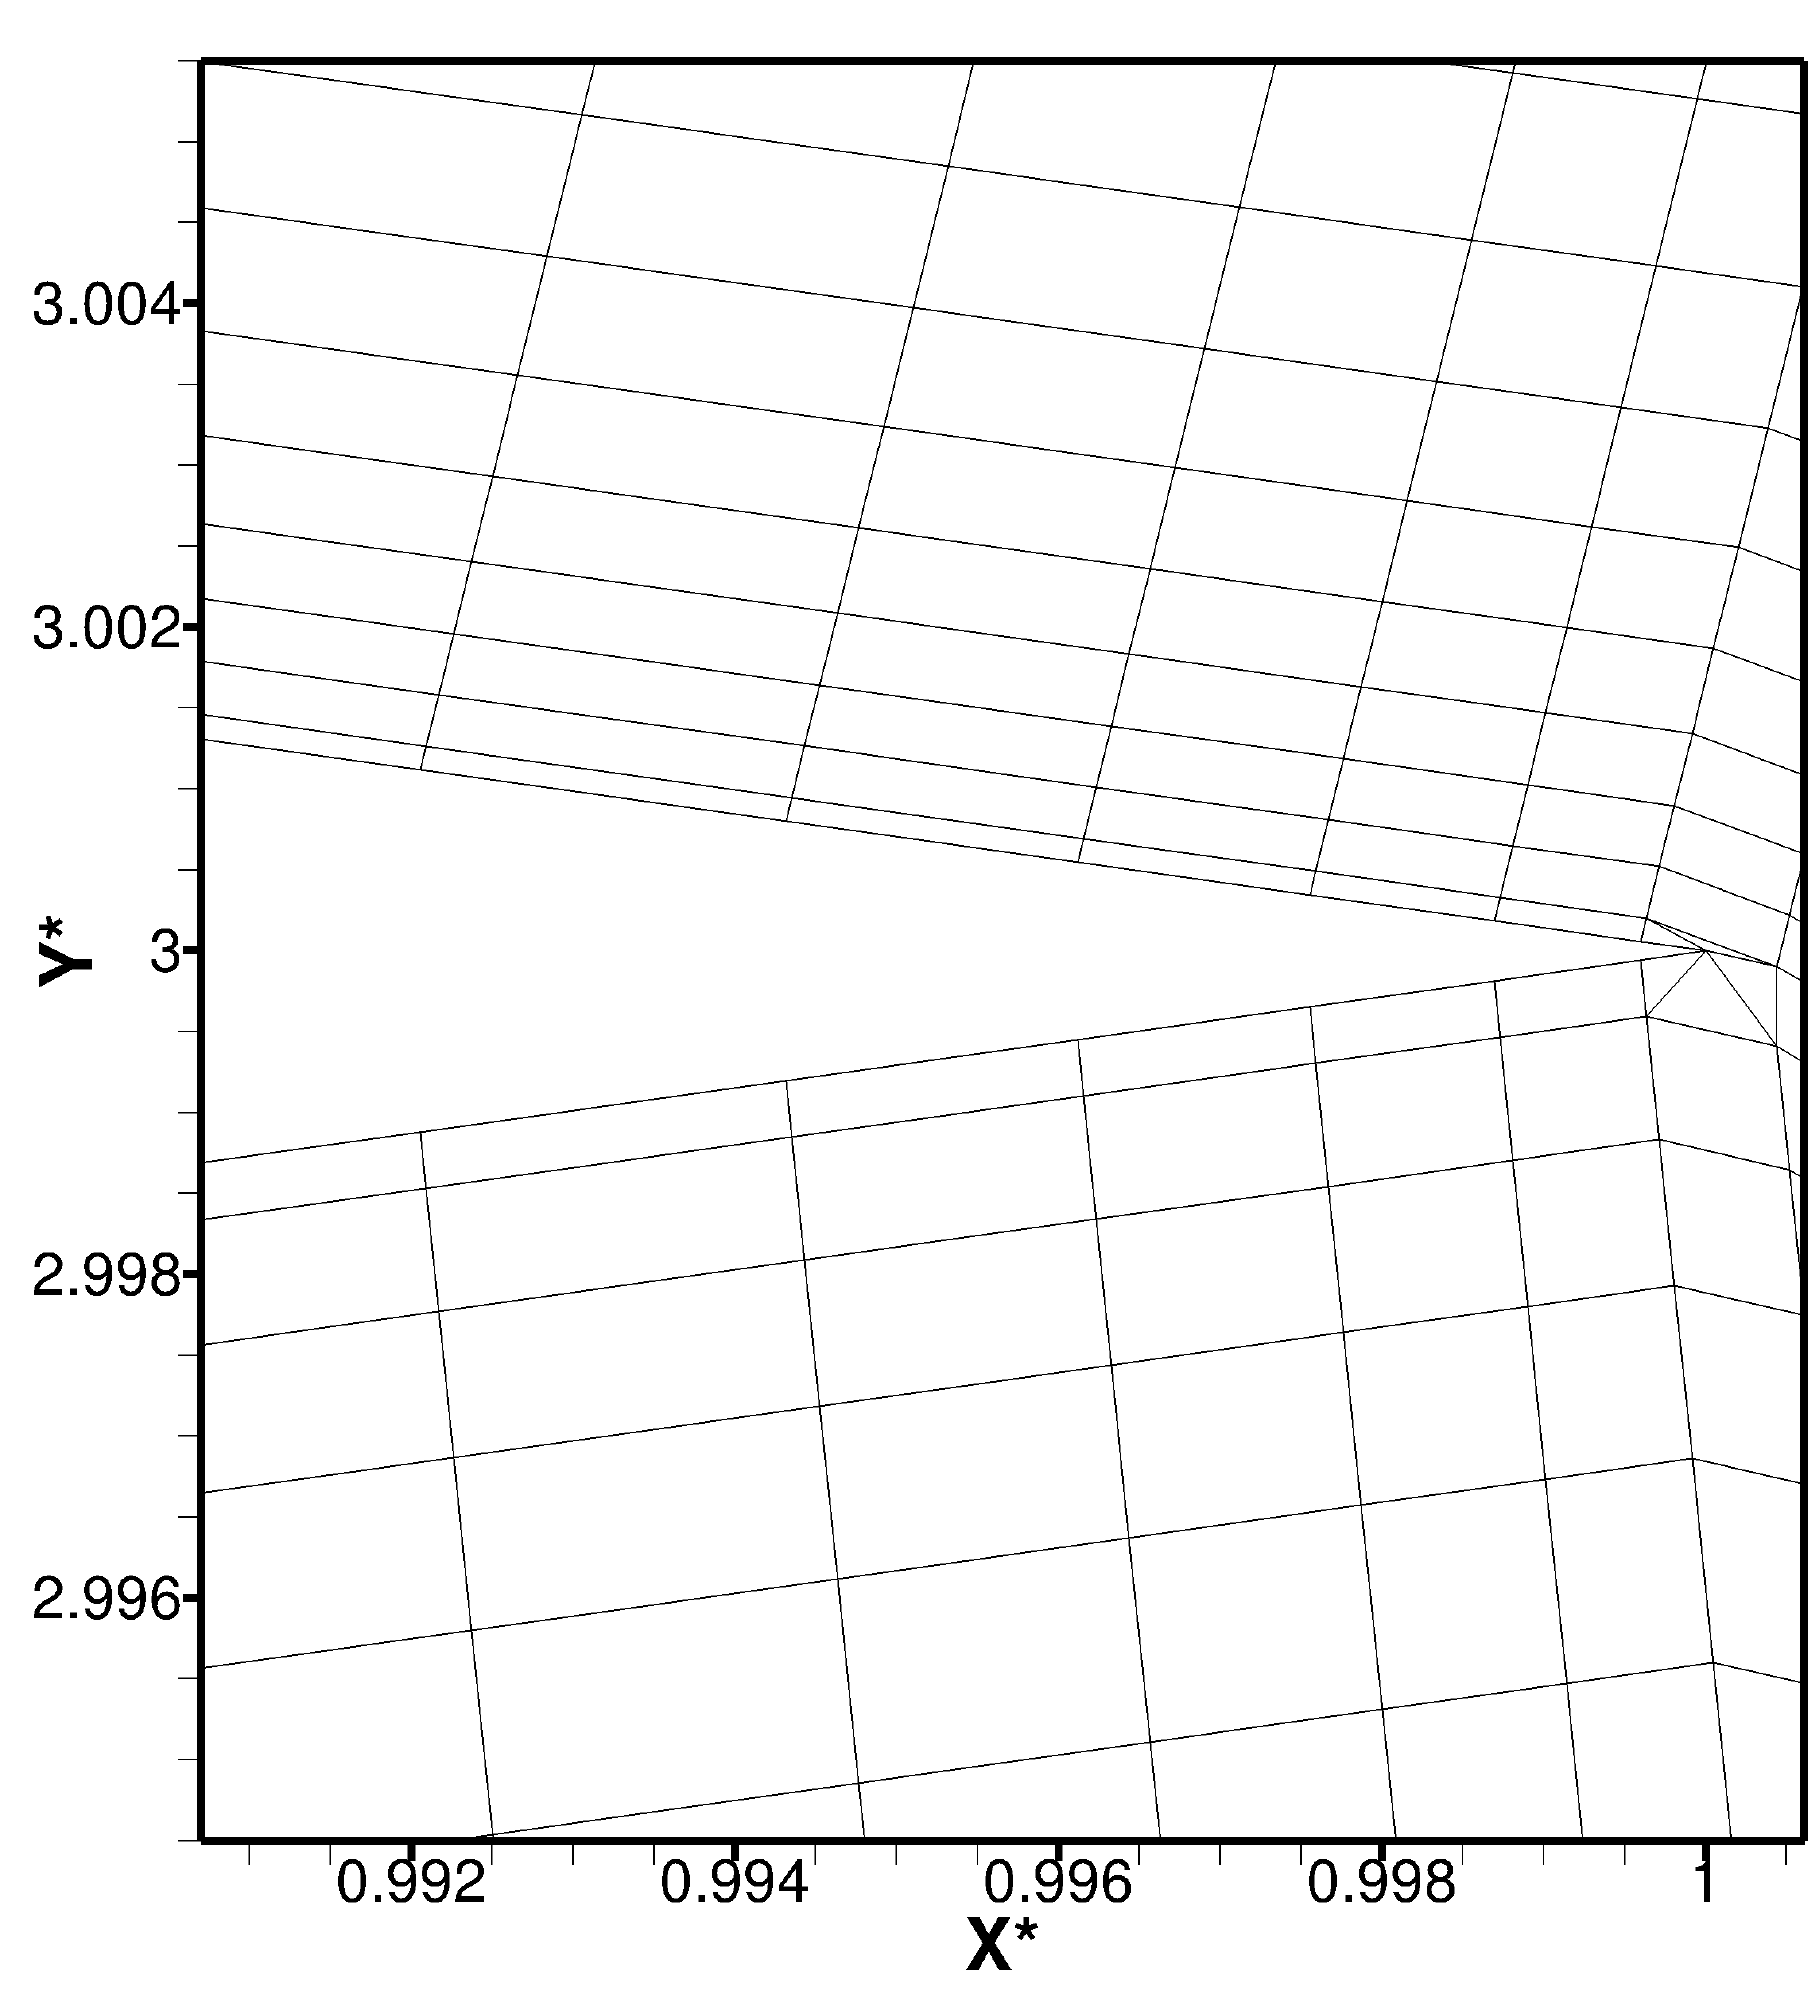} \label{fig:mesh_trailing_edge_tfi_re_meshing}}\hfill
	\caption{TFI algorithm: Mesh adaption considering a translational displacement of \mbox{$X_2=0.3\,\text{m}$}.}
	\label{fig:mesh_tfi_re_meshing}
\end{figure}
\par The IDW  and hybrid IDW-TFI methods are characterized by the maintenance of the first cell height, i$.$e$.$, $\Delta y^{first\,cell}=5{\cdot}10^{-5}\,\text{m}$. Since the required computational time of the former method is about 3.2 and 481.9 times higher than the hybrid IDW-TFI and TFI algorithms while the achieved mesh quality is exactly the same of the hybrid method, the IDW scheme is not considered for further studies.
\par Nine different combinations of the parameters that determine the weighting function of the fixed and the movable boundaries, i$.$e$.$, $\alpha_{fxd}$ and $\alpha_{mv}$, are investigated for the hybrid IDW-TFI algorithm. Since the best mesh quality is achieved for the parameters $\alpha_{fxd}=\alpha_{mv}=0.1$, the mesh adapted utilizing them is illustrated in Fig.\ \ref{fig:mesh_idw_tfi_re_meshing}.
\par The problems generated by the TFI algorithm are overcome through the utilization of this method, i$.$e$.$, no degenerated cells are created at the trailing edge, as well as the first cell height is maintained for all cells located on the airfoil surface, enabling the computation with constant time step sizes. Moreover, the required computational time is reasonable considering the one needed by the IDW method. Although the achieved skew metric quality is low, i$.$e$.$, $f_{skew}\geq0.599$, Fig.\ \ref{fig:mesh_skew_idw_tfi_re_meshing} illustrates that the cells with lower quality are located distant from the airfoil, which does not lead to accuracy problems since the critical flow phenomena occur near the airfoil.
\par Due to the thorough investigation of the mesh adaption algorithms, the IDW-TFI method with $\alpha_{fxd}=\alpha_{mv}=0.1$ is chosen to further simulate cases characterized by large airfoil translational and rotational displacements. Although this requires a higher computational time than the TFI method, this does not lead to numerical difficulties due to the maintenance of the height of the cells located on the airfoil surface and therefore can also be utilized for large rotations without the generation of cells with negative volumes. Moreover, the selected parameters provide the best mesh quality considering the orthogonality of the grid.  
\begin{figure}[H]
	\centering
	\subfigure[Adapted mesh - Overall view.]{\includegraphics[width=0.48\textwidth]{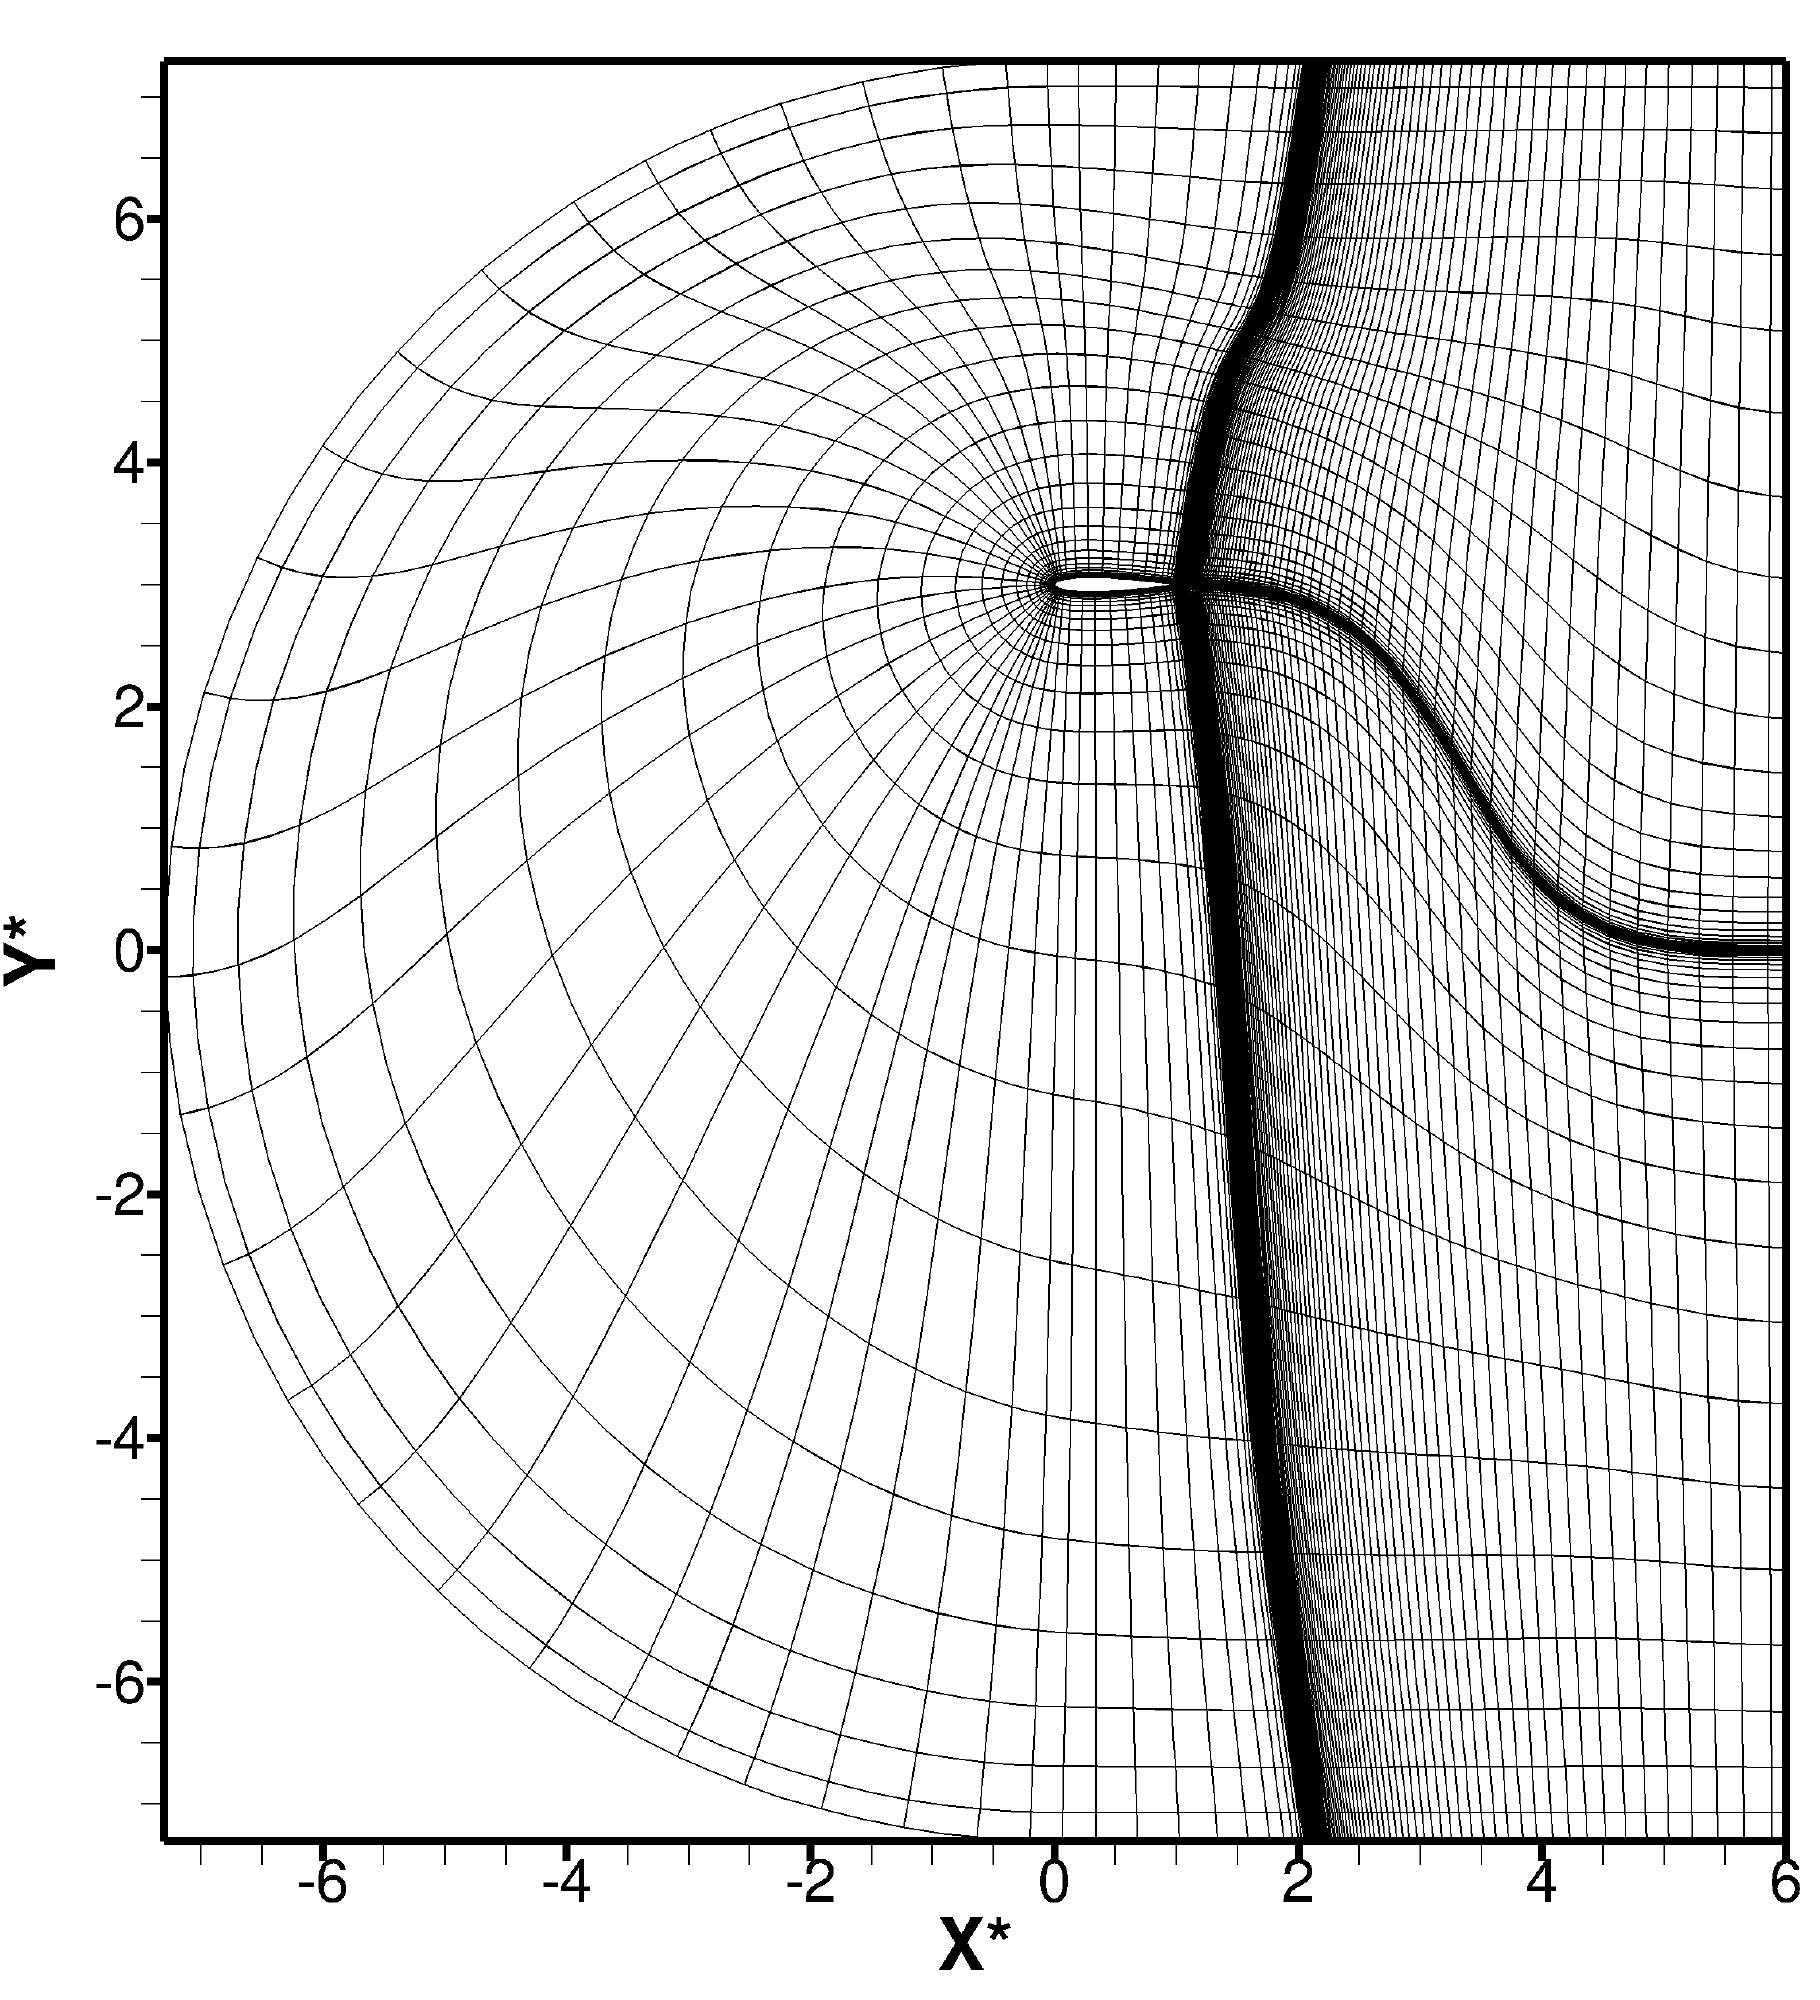} \label{fig:mesh_overall_idw_tfi_re-meshing}}\hfill
	\subfigure[Adapted mesh: Focus on the trailing edge.]{\includegraphics[width=0.48\textwidth]{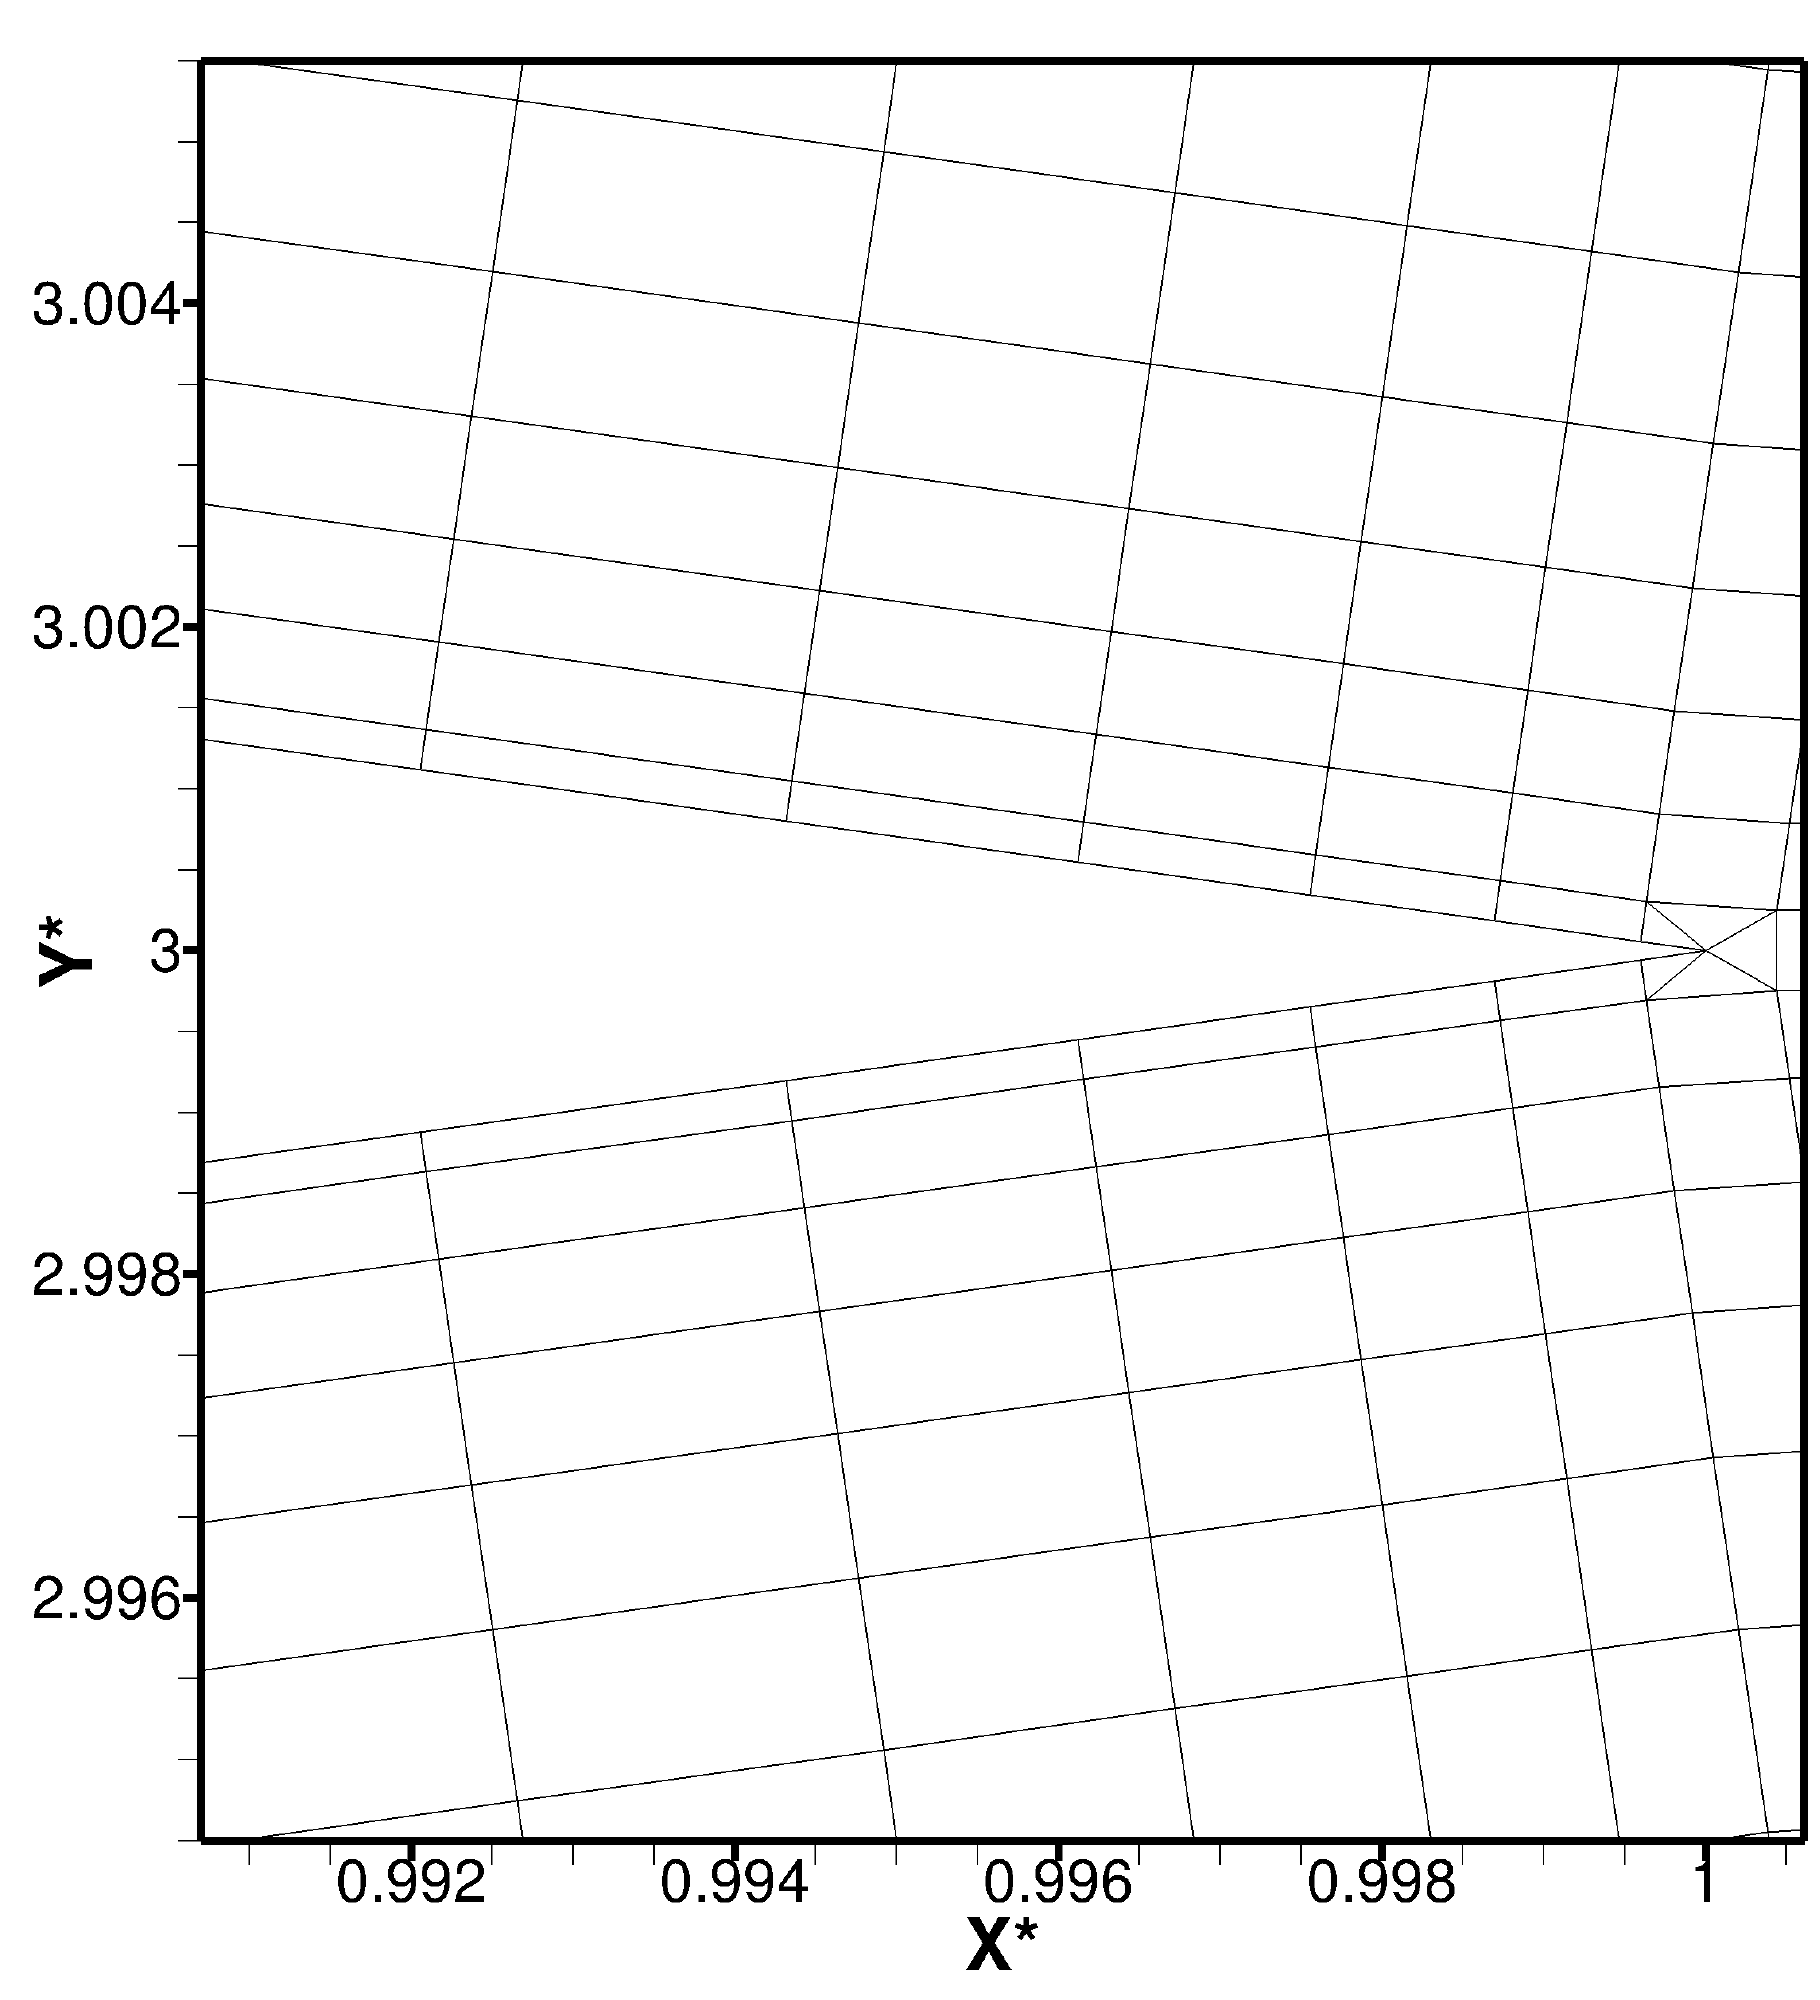}\label{fig:mesh_trailing_edge_idw_tfi_re_meshing}}\hfill
	\caption{Hybrid IDW-TFI algorithm with $\alpha_{fxd}=\alpha_{mv}=0.1$: Mesh adaption considering a translational displacement of $X_2=0.3\,\text{m}$.}
	\label{fig:mesh_idw_tfi_re_meshing}
\end{figure}
\begin{figure}[H]
	\centering
	\centering
	\includegraphics[scale=0.85,draft=\drafttype]{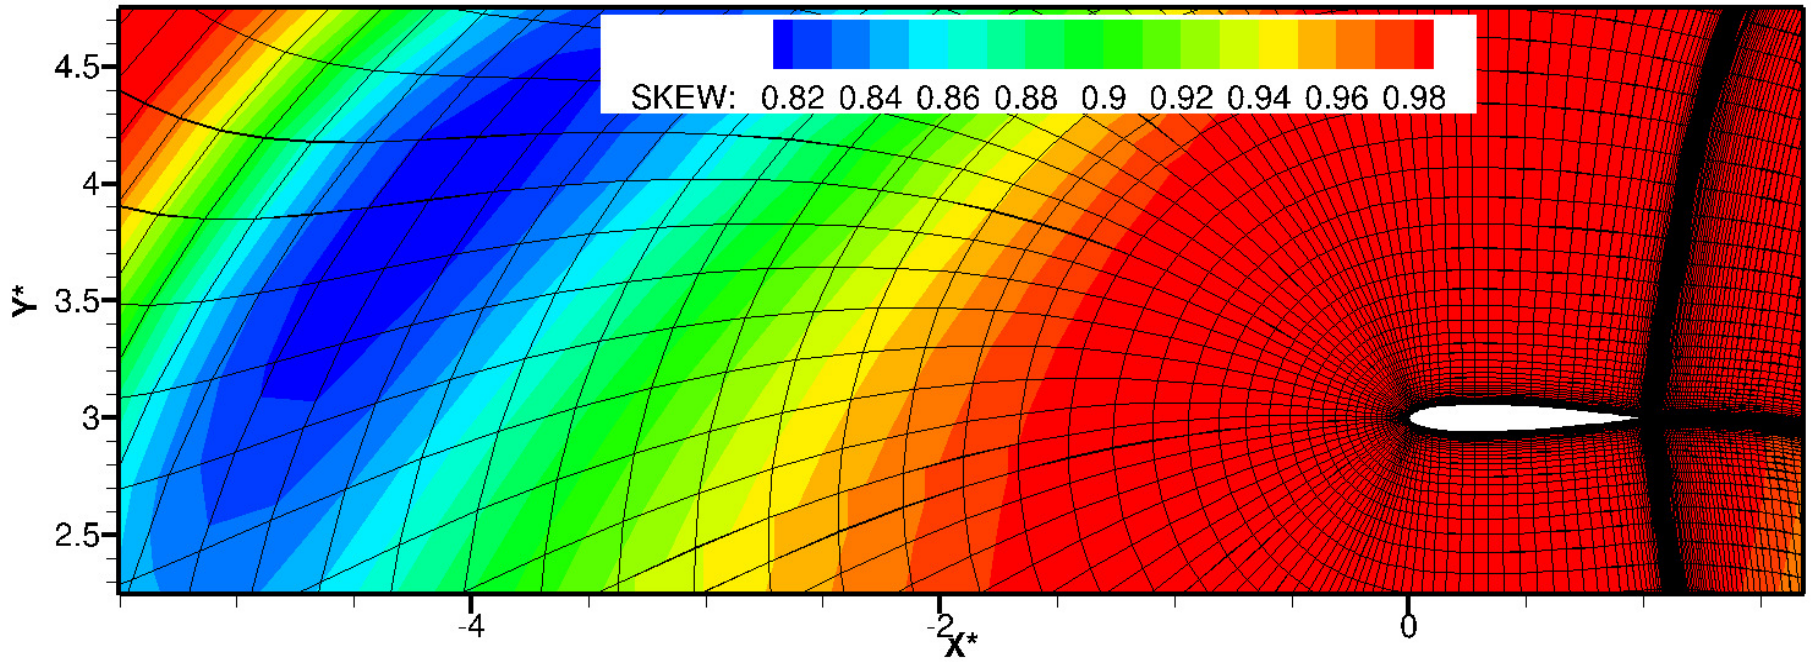}
	\caption{\label{fig:mesh_skew_idw_tfi_re_meshing}Hybrid IDW-TFI algorithm with $\alpha_{fxd}=\alpha_{mv}=0.1$: Mesh quality considering a translational displacement of $X_2=0.3\,\text{m}$.}
\end{figure}
